# Supplementary material for: Adaptive Data-Resilient Multi-Modal Hierarchical Multi-Label Book Genre Identification
Source: arXiv:2505.03839 source file (2025-10-18)
Supplement: Supplementary file 1 [file 7appendix.tex]

\newpage

%less moderate adequate complex

\balance
\appendices

\counterwithin{figure}{section}
\counterwithin{table}{section}
\section{Genre Co-occurrence matrix}
\label{app:cooccurrence}

\begin{figure*}[!t]
    \centering
    (a) \includegraphics[width=0.45\linewidth]{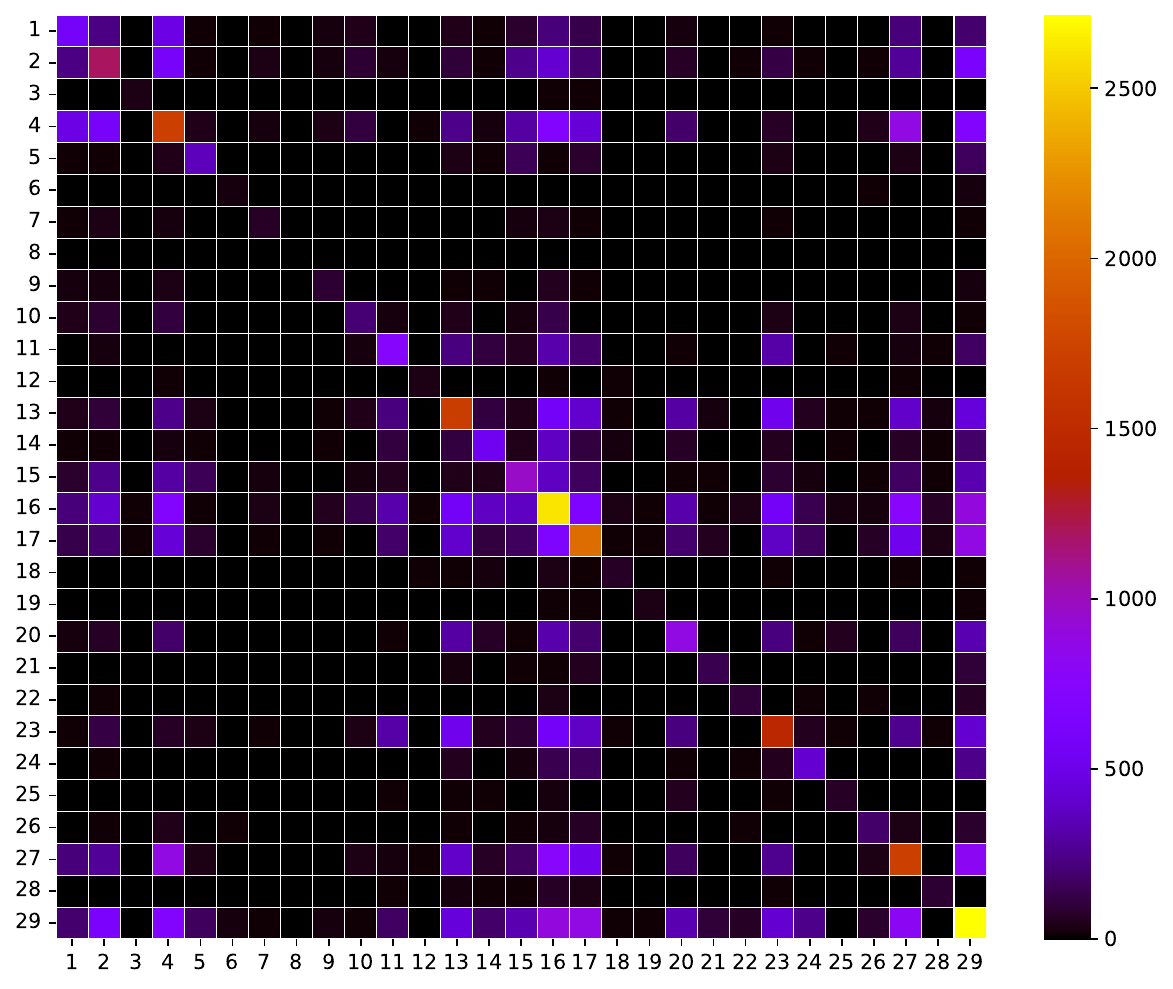}
    (b) \includegraphics[width=0.45\linewidth]{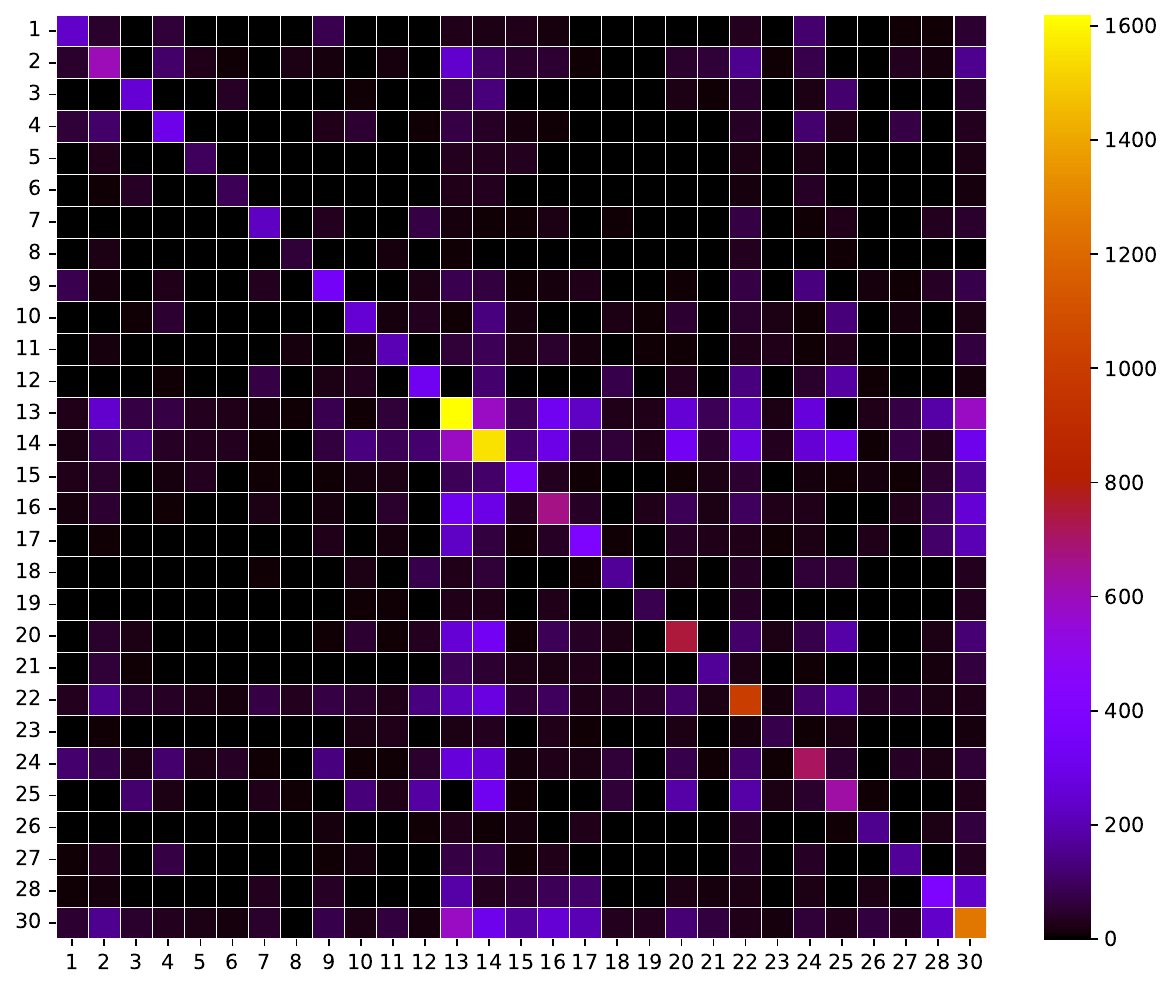}
    \caption{Co-occurrence matrices for book genres: (a) \textit{fiction}, (b) \textit{non-fiction}}
    \label{fig:f_nf_cooccurrence}
\end{figure*}

\noindent 
Fig.s \ref{fig:f_nf_cooccurrence}: (a), (b) visually depict the relationships and co-occurrence patterns among book \textit{fiction} and \textit{non-fiction} genres.

% \begin{figure}[!h]
%     \centering
%     \includegraphics[width=1\linewidth]{figs/co_occurrence_matrix/fiction_heatmap.pdf}
%     \caption{Co-occurrence matrix for book \textit{fiction} genre}
%     \label{fig:fiction_cooccurrence}
% \end{figure}

% \begin{figure}[!h]
%     \centering
%     \includegraphics[width=1\linewidth]{figs/co_occurrence_matrix/nonfiction_heatmap.pdf}
%     \caption{Co-occurrence matrix for book \textit{non-fiction} genre}
%     \label{fig:non_fiction_cooccurrence}
% \end{figure}

\section{Dataset Collection \& Design}
\label{app:dataset_creation}

\noindent 
This section discusses on the collected book data, e.g., coverpage, blurb, metadata, followed by genre labeling.

\section{Dataset Challenges} 
\label{app:dataset_challenge}

\begin{figure*}[t]
\centering
\footnotesize
\makebox[\textwidth][c]{
\begin{adjustbox}{width=\linewidth}
\begin{tabular}{c|c|c|c || c|c|c|c}
%%%%%%%%%%%%%%%
\hline 
&&& &&&&  \\[\dimexpr-\normalbaselineskip+1.5pt]
\includegraphics[width=0.1\linewidth, height=0.145\linewidth]{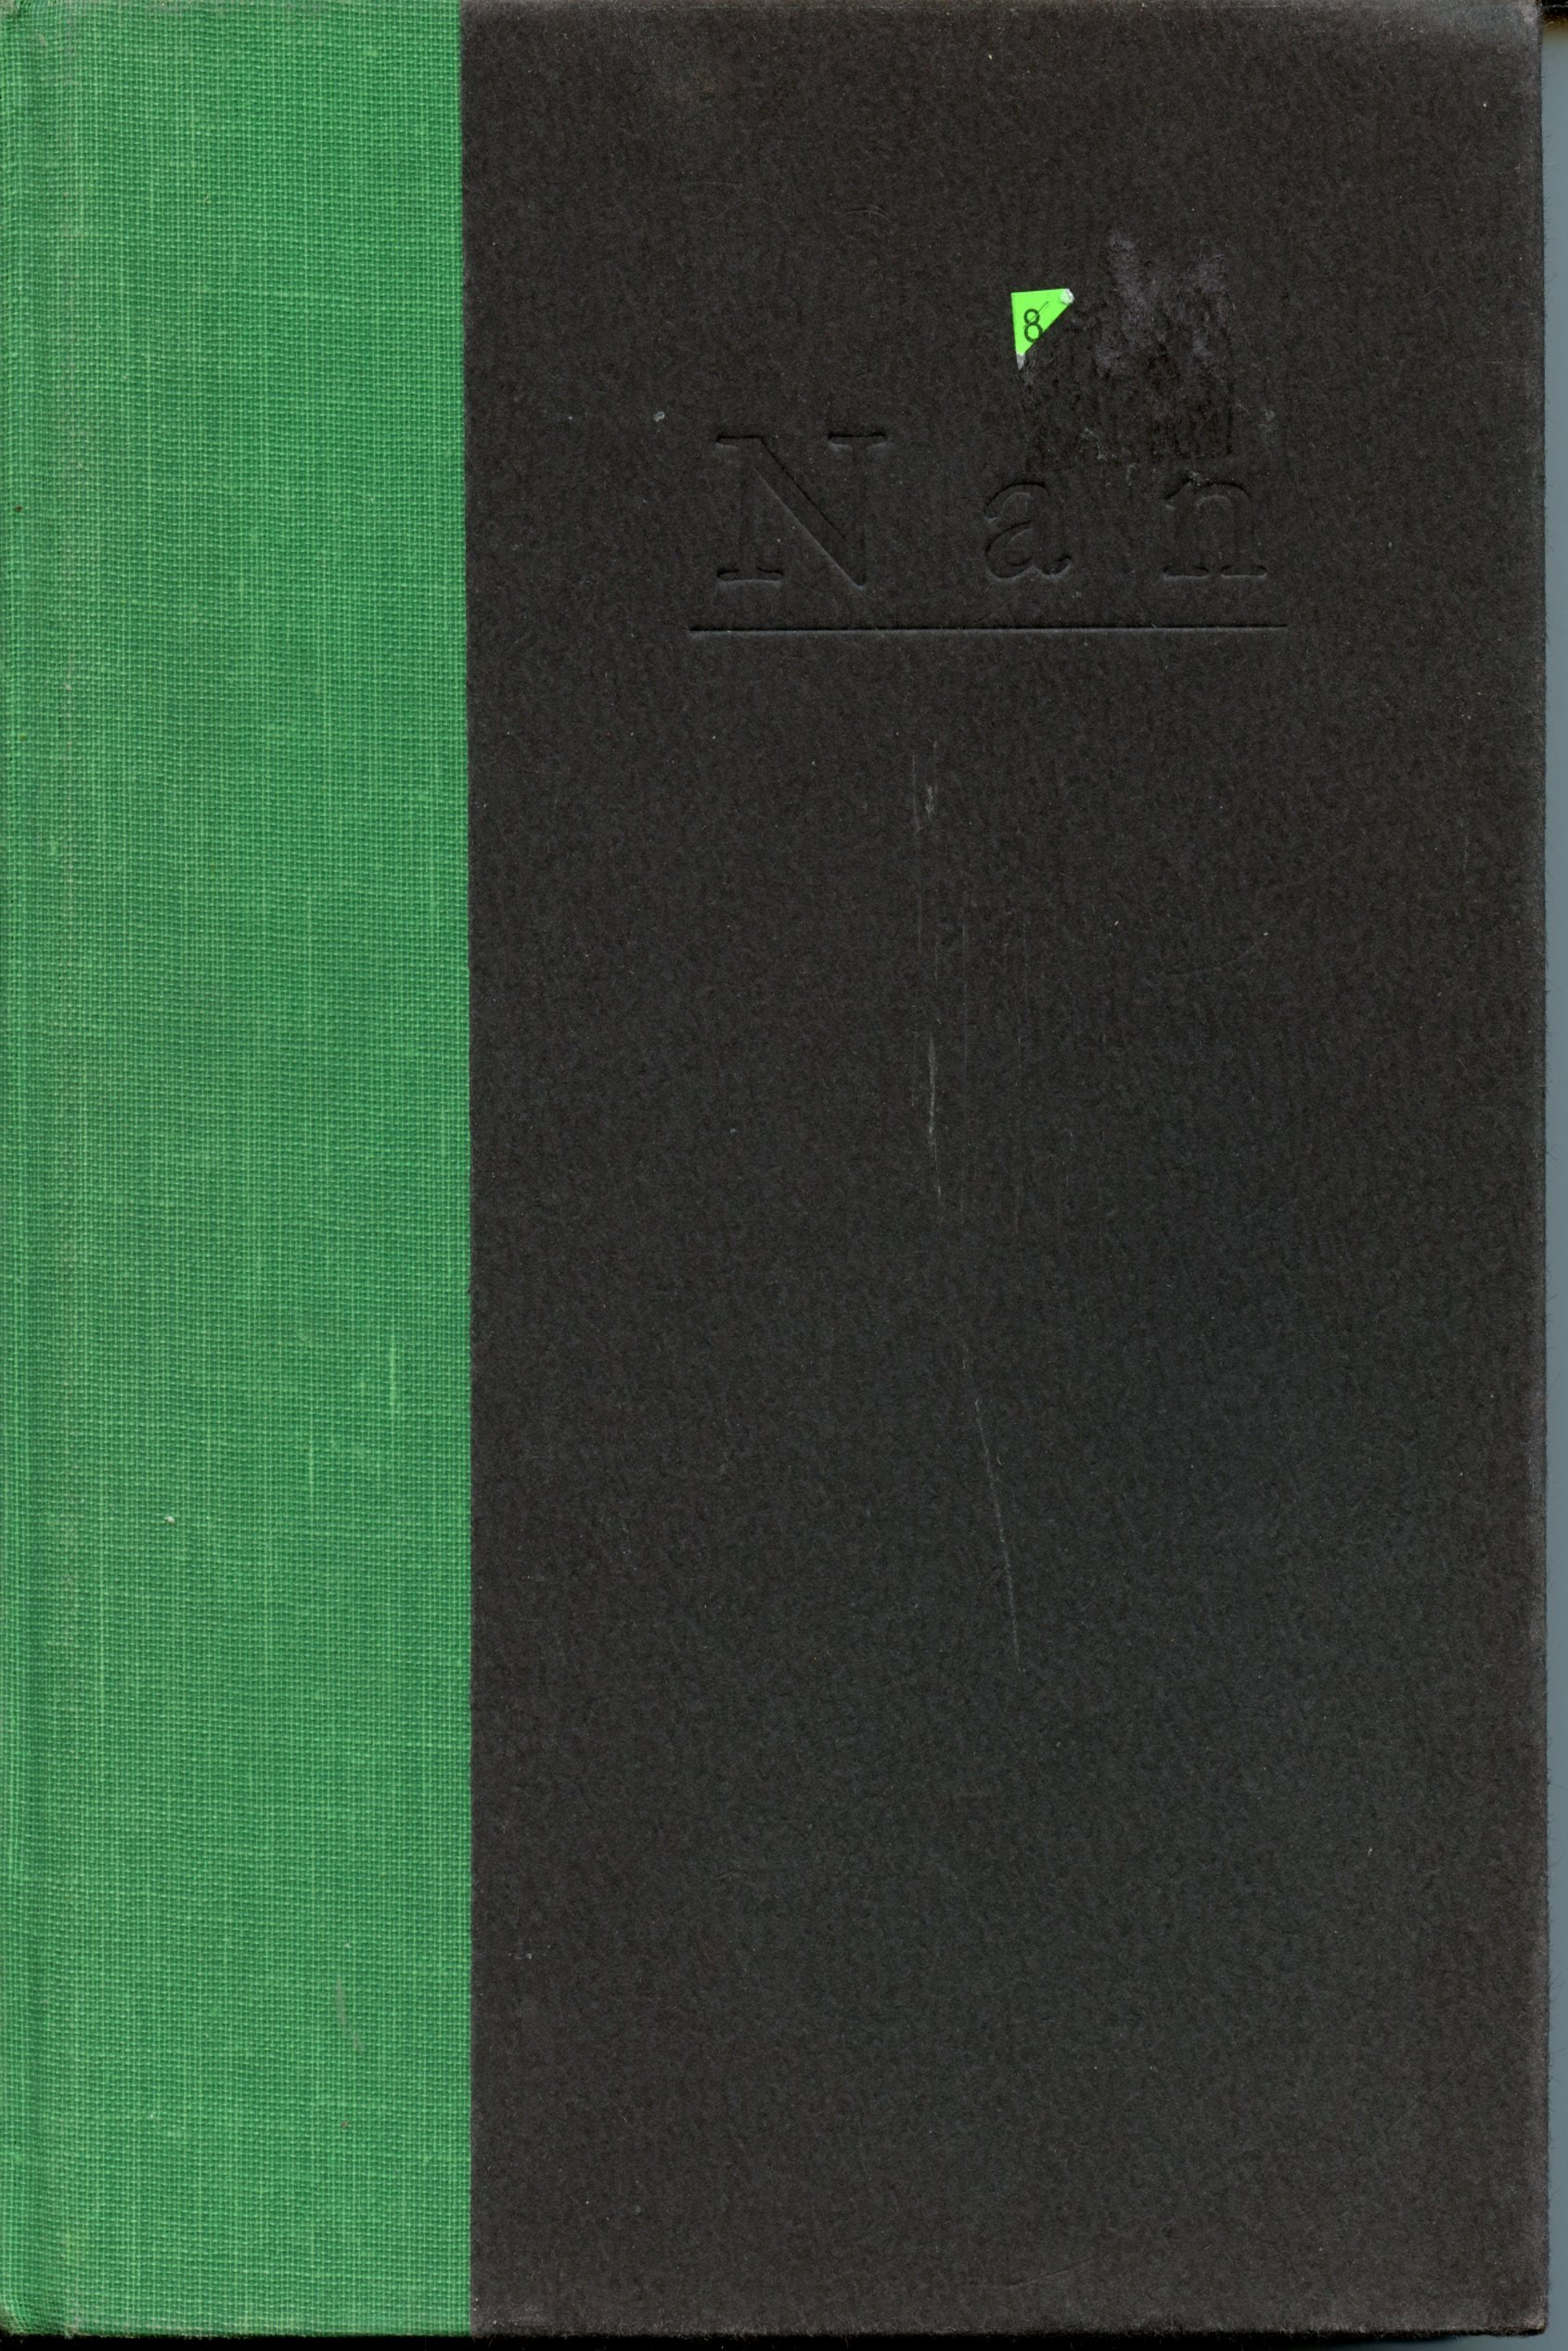} & 
\includegraphics[width=0.1\linewidth, height=0.145\linewidth]{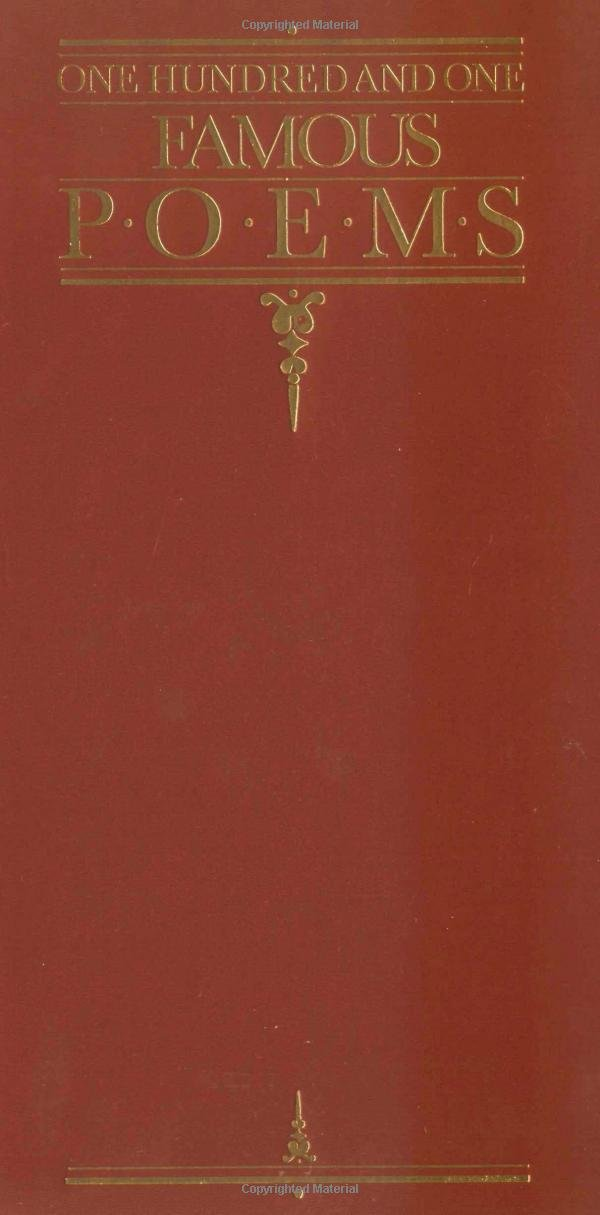} & 
\includegraphics[width=0.1\linewidth, height=0.145\linewidth]{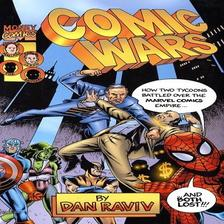} & 
\includegraphics[width=0.1\linewidth, height=0.145\linewidth]{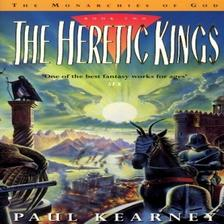} &
\includegraphics[width=0.1\linewidth, height=0.145\linewidth]{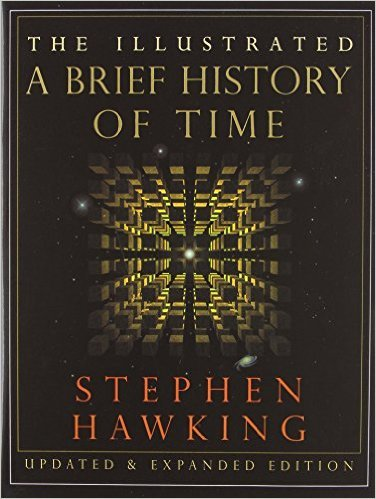} & 
\includegraphics[width=0.1\linewidth, height=0.145\linewidth]{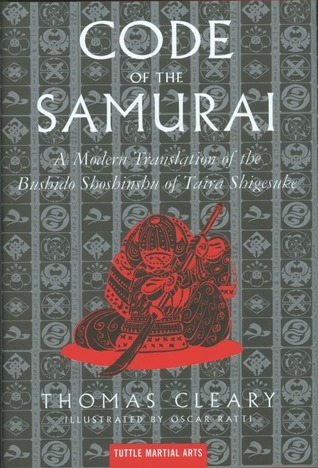} &
\includegraphics[width=0.1\linewidth, height=0.145\linewidth]{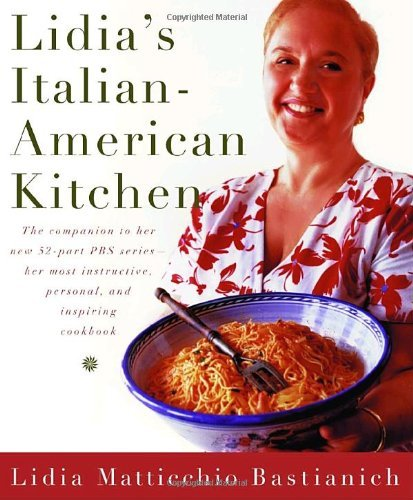} & 
\includegraphics[width=0.1\linewidth, height=0.145\linewidth]{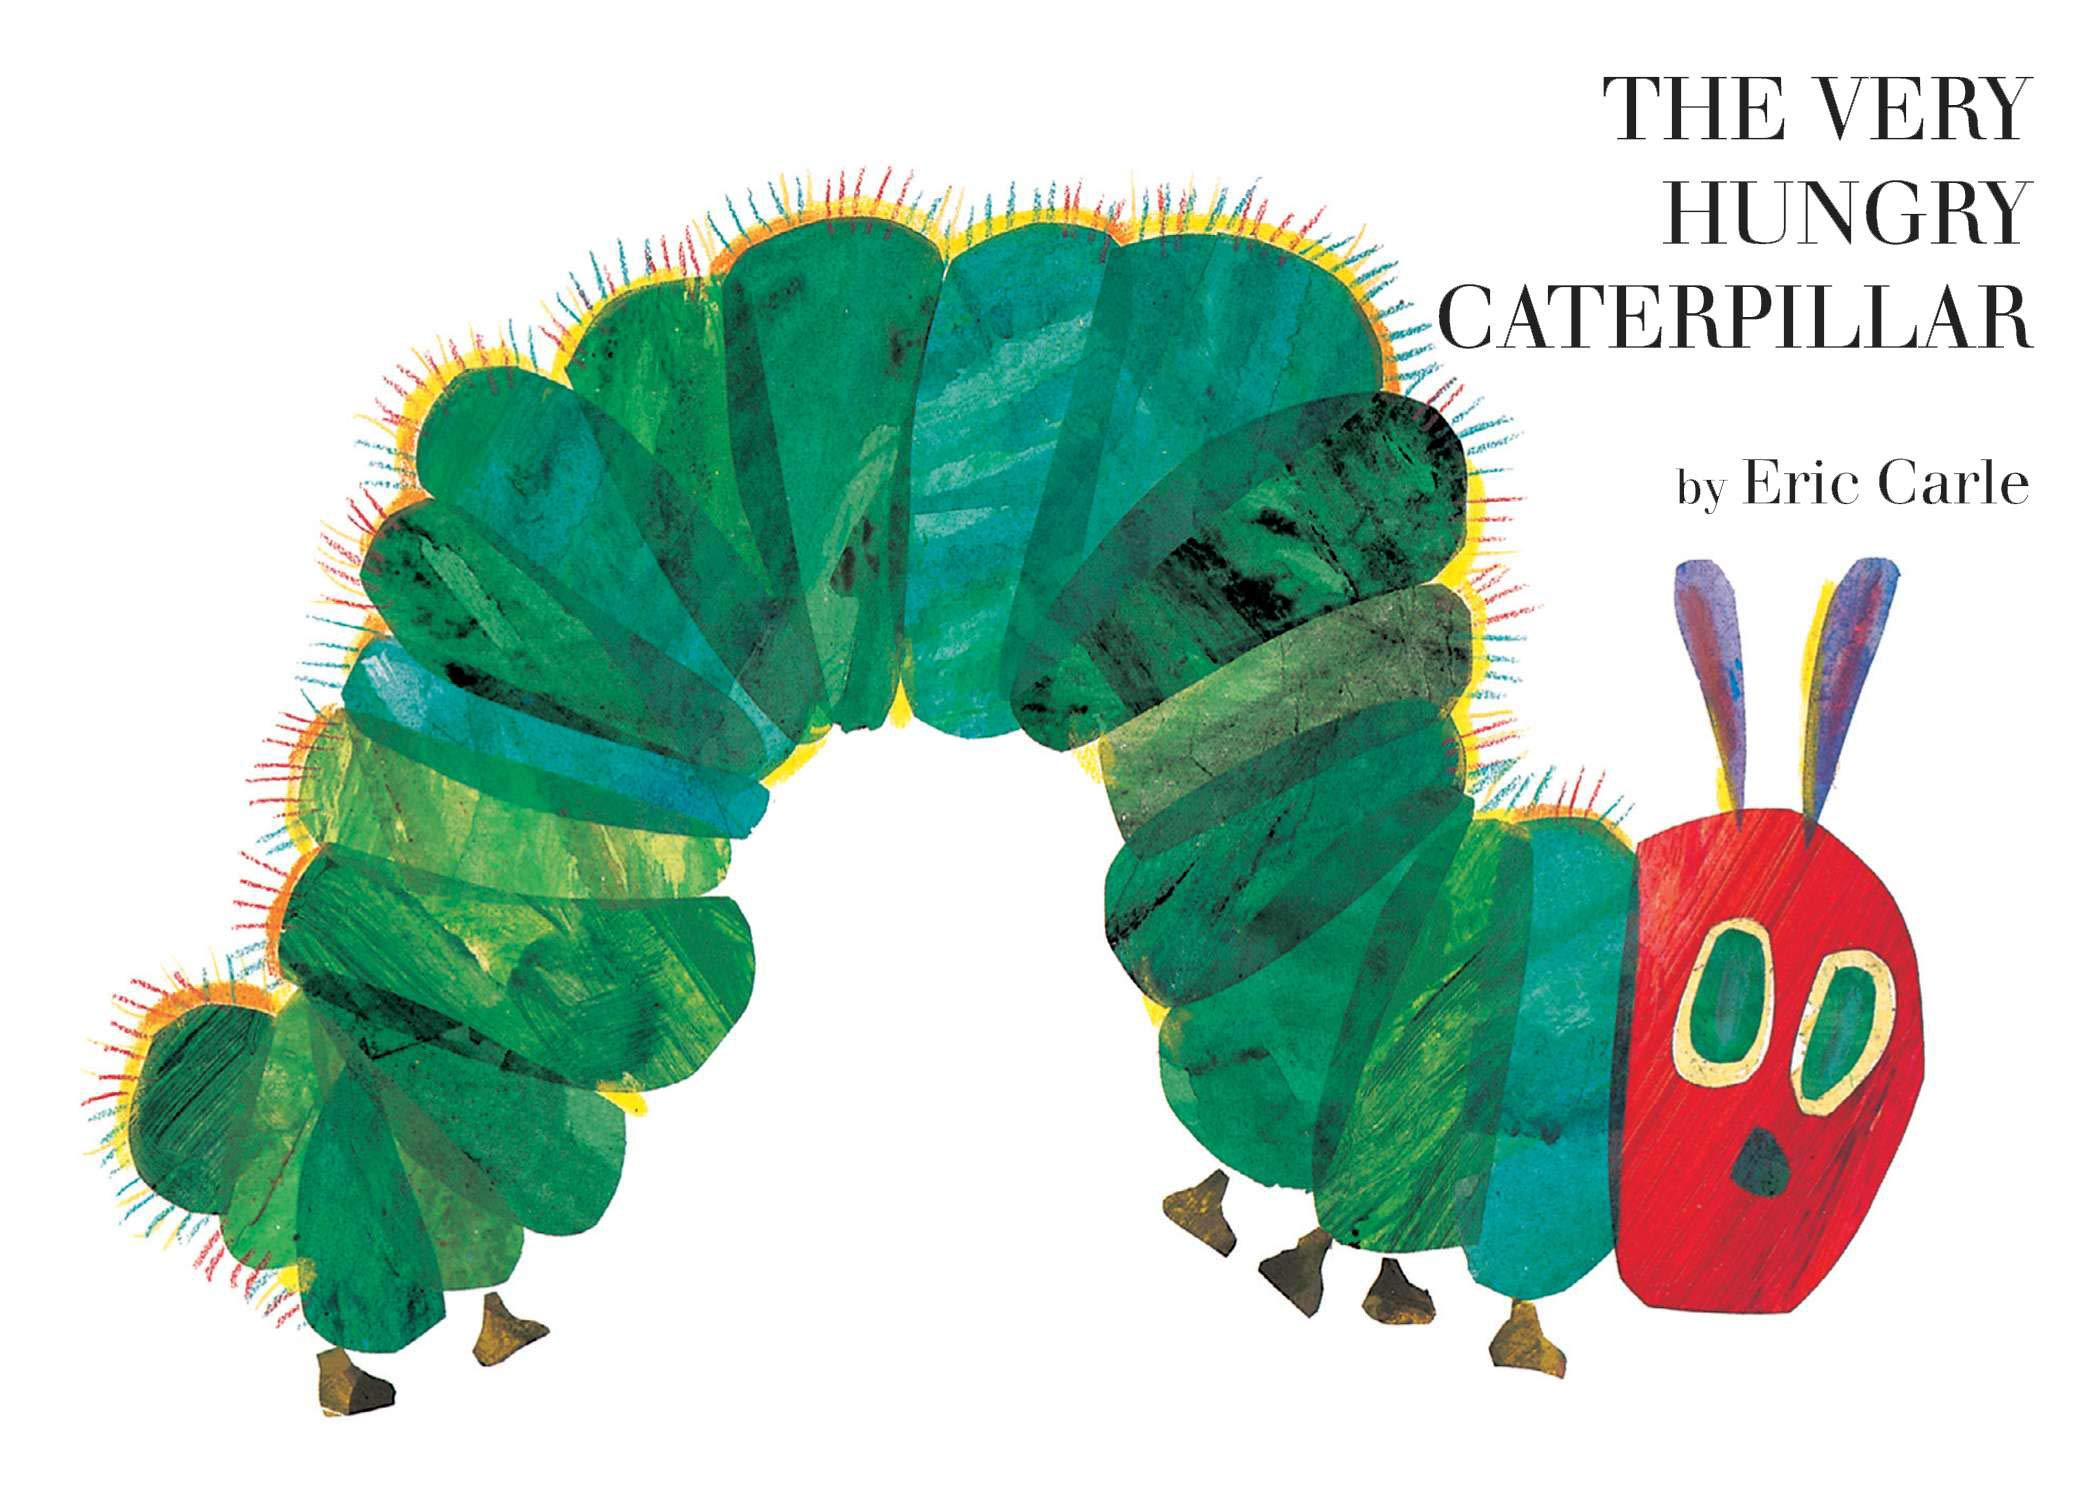} 
\\ 
\textcolor{blue}{\emph{i.}} F : (13, 14, 28, 30) & \textcolor{blue}{\emph{ii.}}  NF : (16, 22, 24) & 
\textcolor{blue}{\emph{iii.}}  NF : (3, 5, 13) & \textcolor{blue}{\emph{iv.}}  F : (16, 29) & 
\textcolor{blue}{\emph{v.}}  NF : (13, 14, 16, 24) & \textcolor{blue}{\emph{vi.}}  NF : (2, 13, 14) & 
\textcolor{blue}{\emph{vii.}}  NF : (7, 16, 22) & \textcolor{blue}{\emph{viii.}}  F : (1, 2, 4, 7)   \\ 
\multicolumn{2}{c|}{Limited visual cues} & \multicolumn{2}{c||}{Complex background} & \multicolumn{4}{c}{Moderate info} \\
%%%%%%%%%%%%%%%
\hline 
&&& &&&&  \\[\dimexpr-\normalbaselineskip+1.5pt]
\includegraphics[width=0.1\linewidth, height=0.145\linewidth]{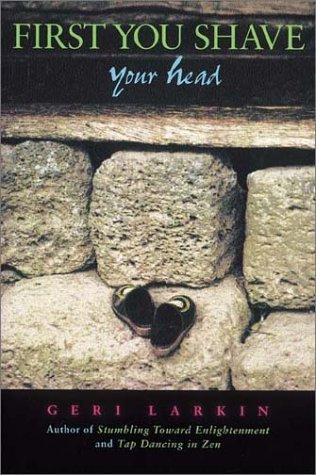} & 
\includegraphics[width=0.1\linewidth, height=0.145\linewidth]{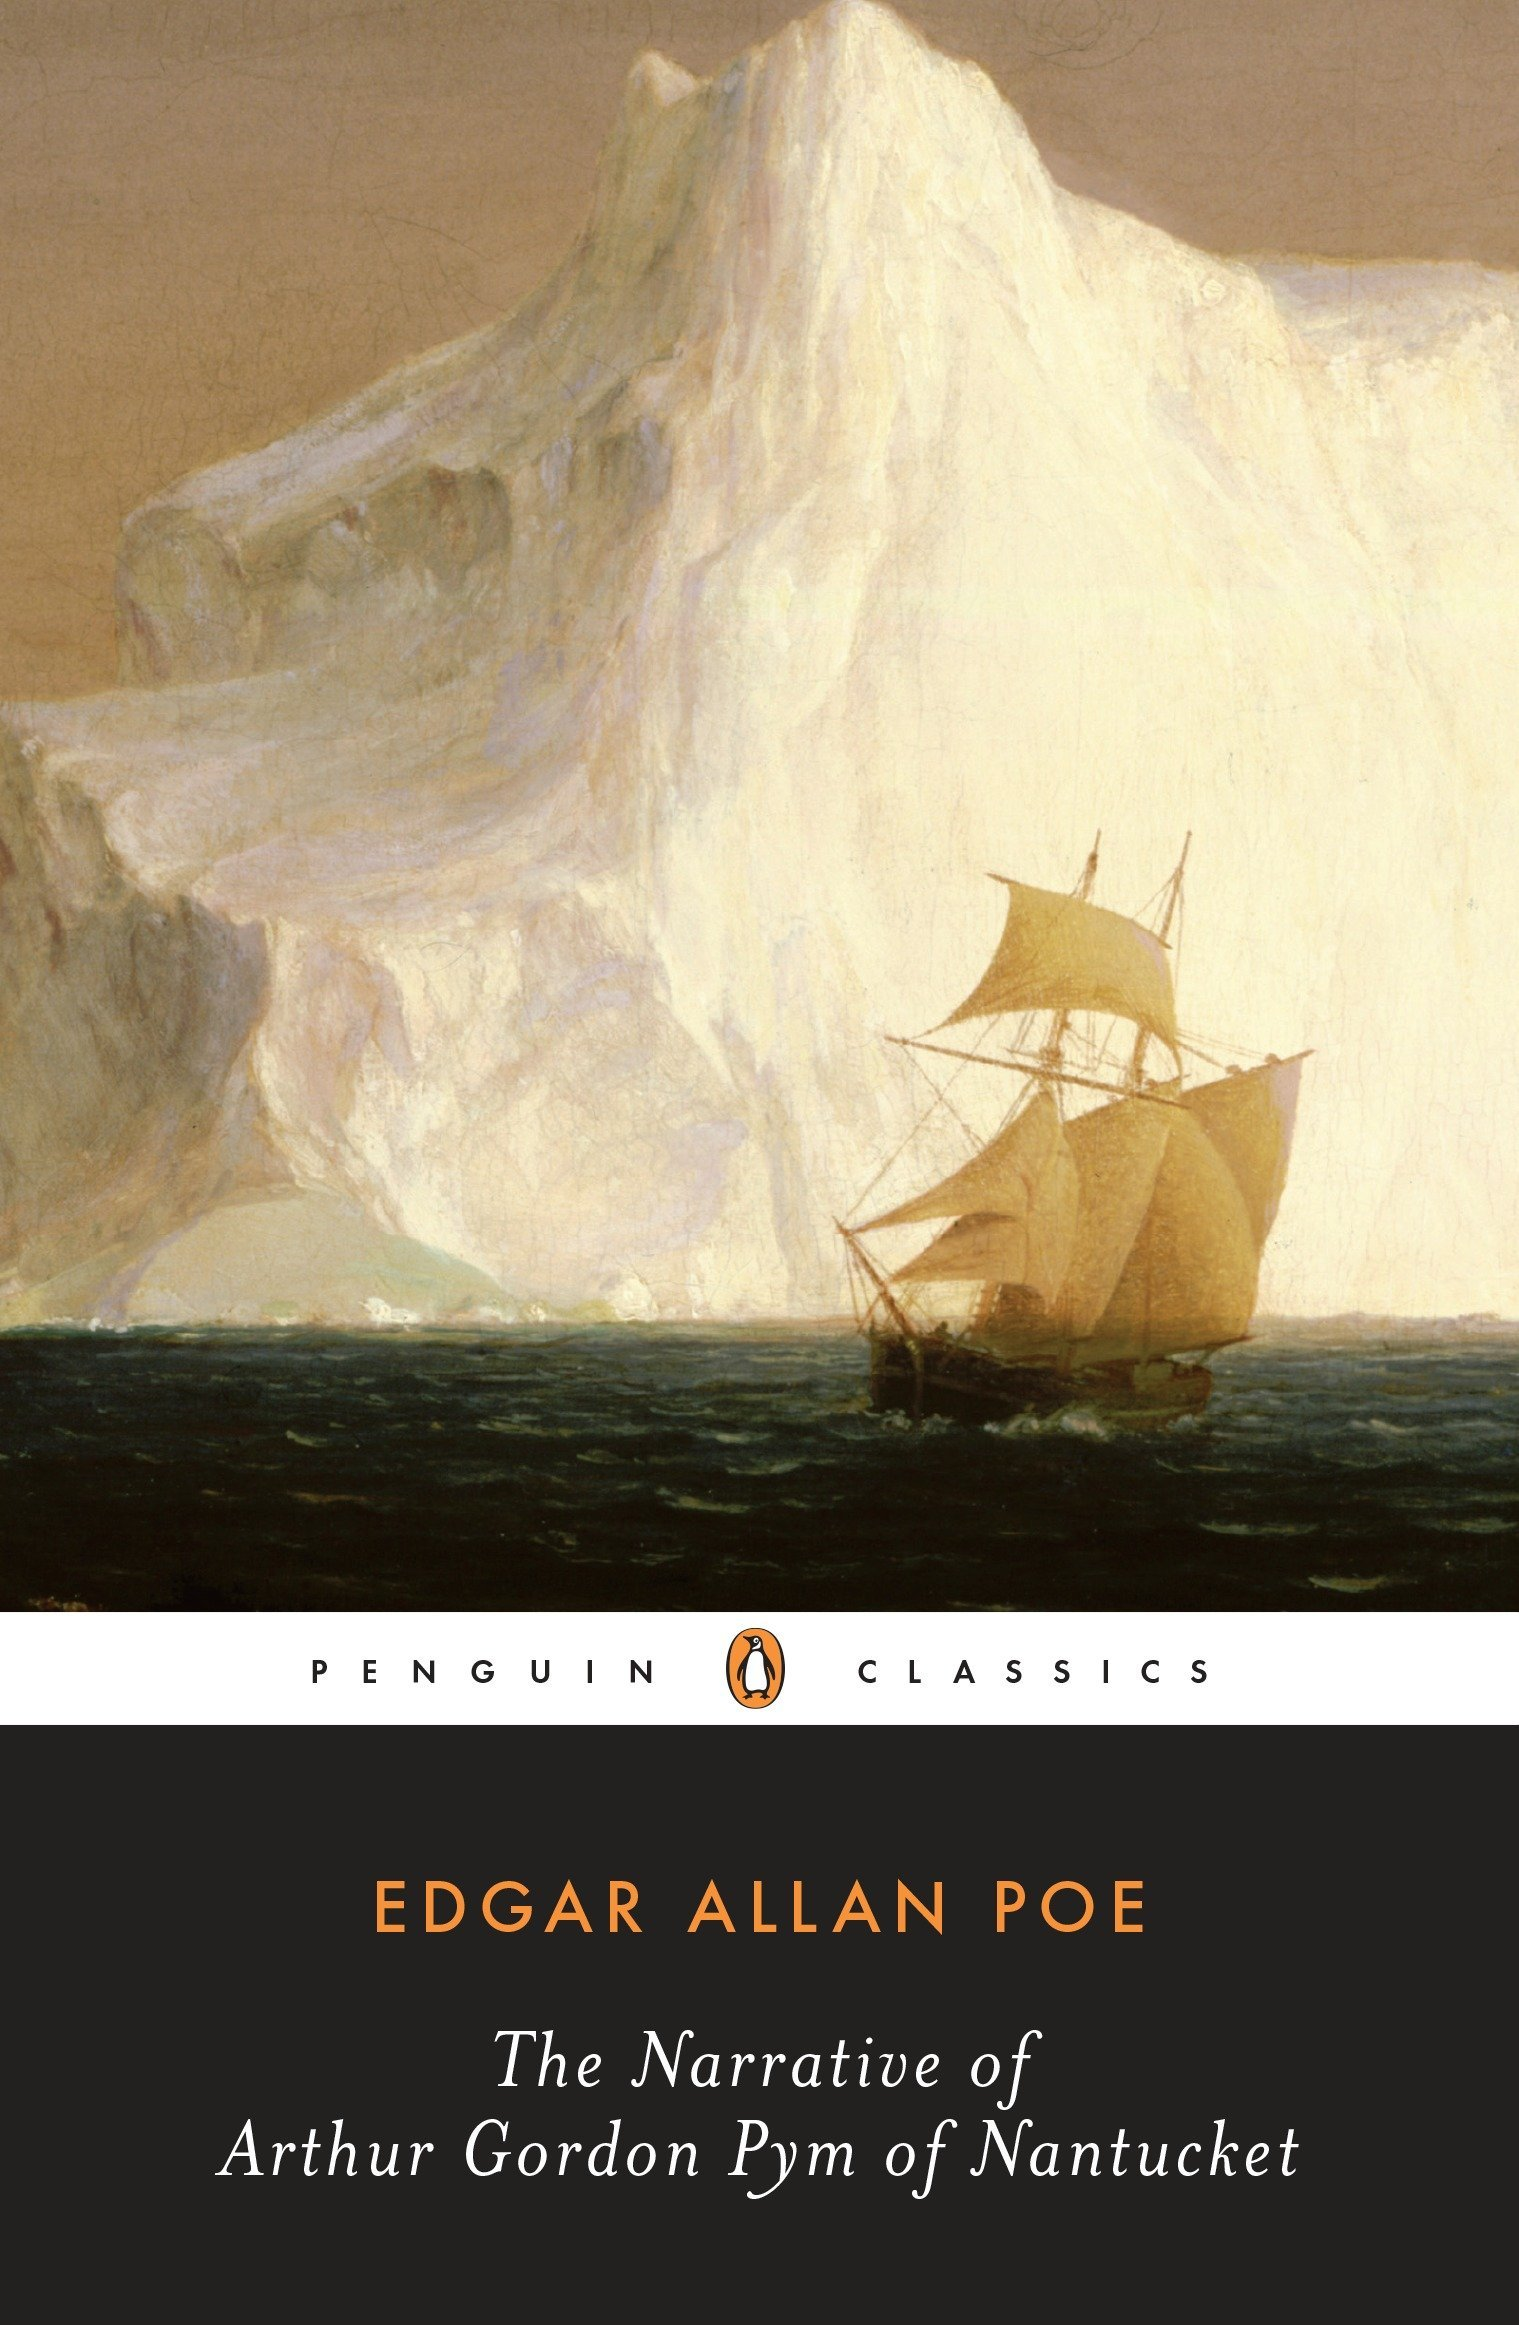} & 
\includegraphics[width=0.1\linewidth, height=0.145\linewidth]{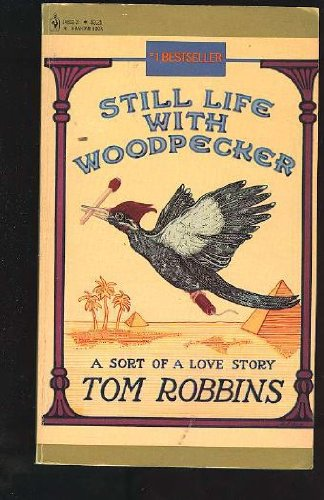} & 
\includegraphics[width=0.1\linewidth, height=0.145\linewidth]{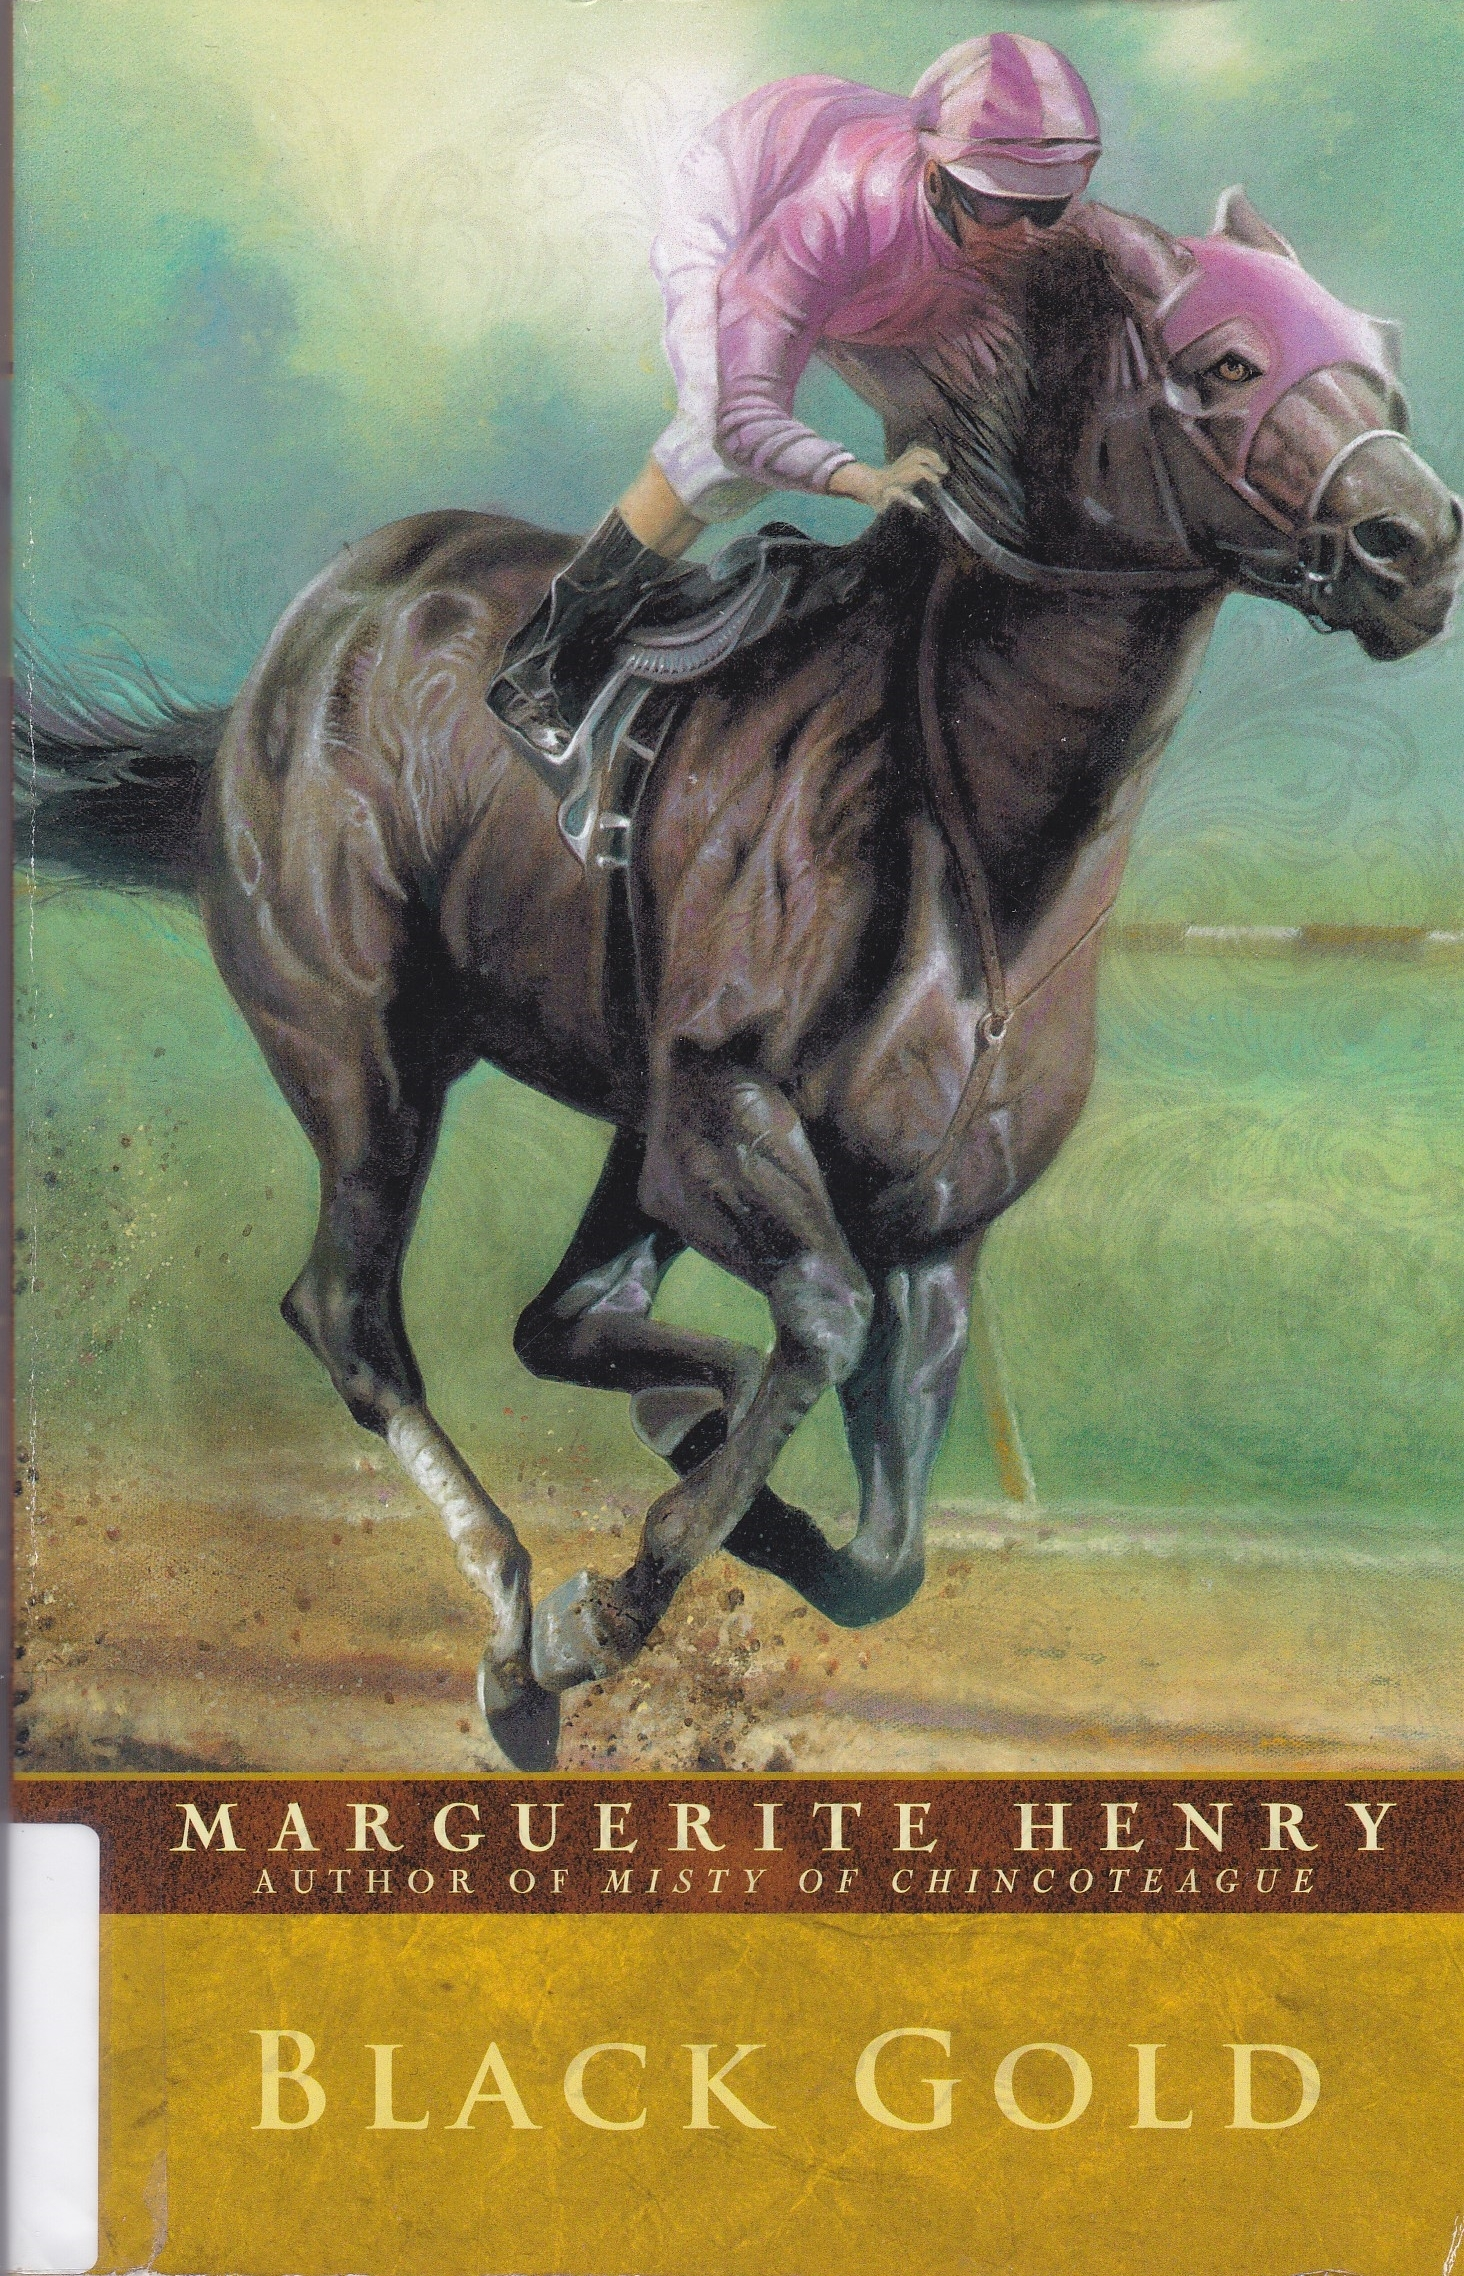} &
\includegraphics[width=0.1\linewidth, height=0.145\linewidth]{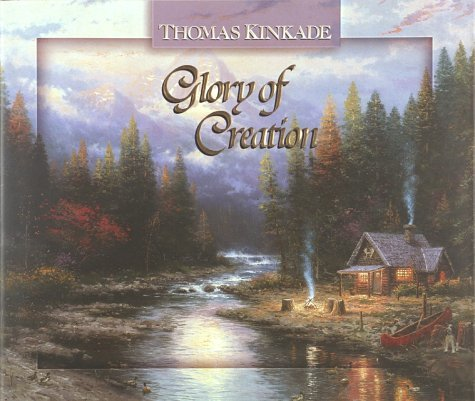} & 
\includegraphics[width=0.1\linewidth, height=0.145\linewidth]{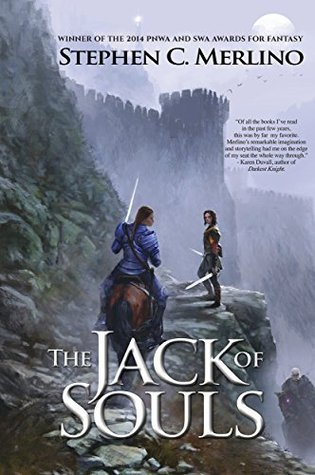} & 
\includegraphics[width=0.1\linewidth, height=0.145\linewidth]{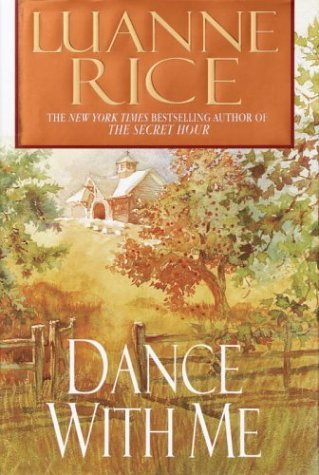} & 
\includegraphics[width=0.1\linewidth, height=0.145\linewidth]{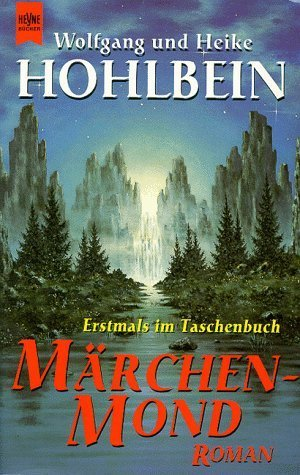} 
\\ 
\textcolor{blue}{\emph{ix.}} NF : (20, 28) & \textcolor{blue}{\emph{x.}}  F : (16, 17, 23, 29) & \textcolor{blue}{\emph{xi.}}  F : (2, 15, 16) & \textcolor{blue}{\emph{xii.}}  F : (9, 14) & 
\textcolor{blue}{\emph{xiii.}}  NF : (2) & \textcolor{blue}{\emph{xiv.}}  F : (29, 23, 27, 17) & \textcolor{blue}{\emph{xv.}}  F : (10, 11, 23) & \textcolor{blue}{\emph{xvi.}} F : (4, 29, 27)  \\ 
\multicolumn{2}{c|}{Non-living element} & \multicolumn{2}{c||}{living element} & \multicolumn{4}{c|}{Scene image}\\
%%%%%%%%%%%%%%%
\hline 
&&& &&&&  \\[\dimexpr-\normalbaselineskip+1.5pt]
\includegraphics[width=0.1\linewidth, height=0.145\linewidth]{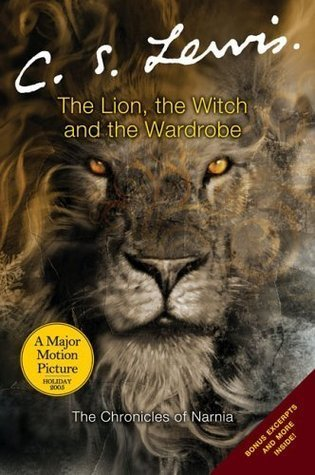} & 
\includegraphics[width=0.1\linewidth, height=0.145\linewidth]{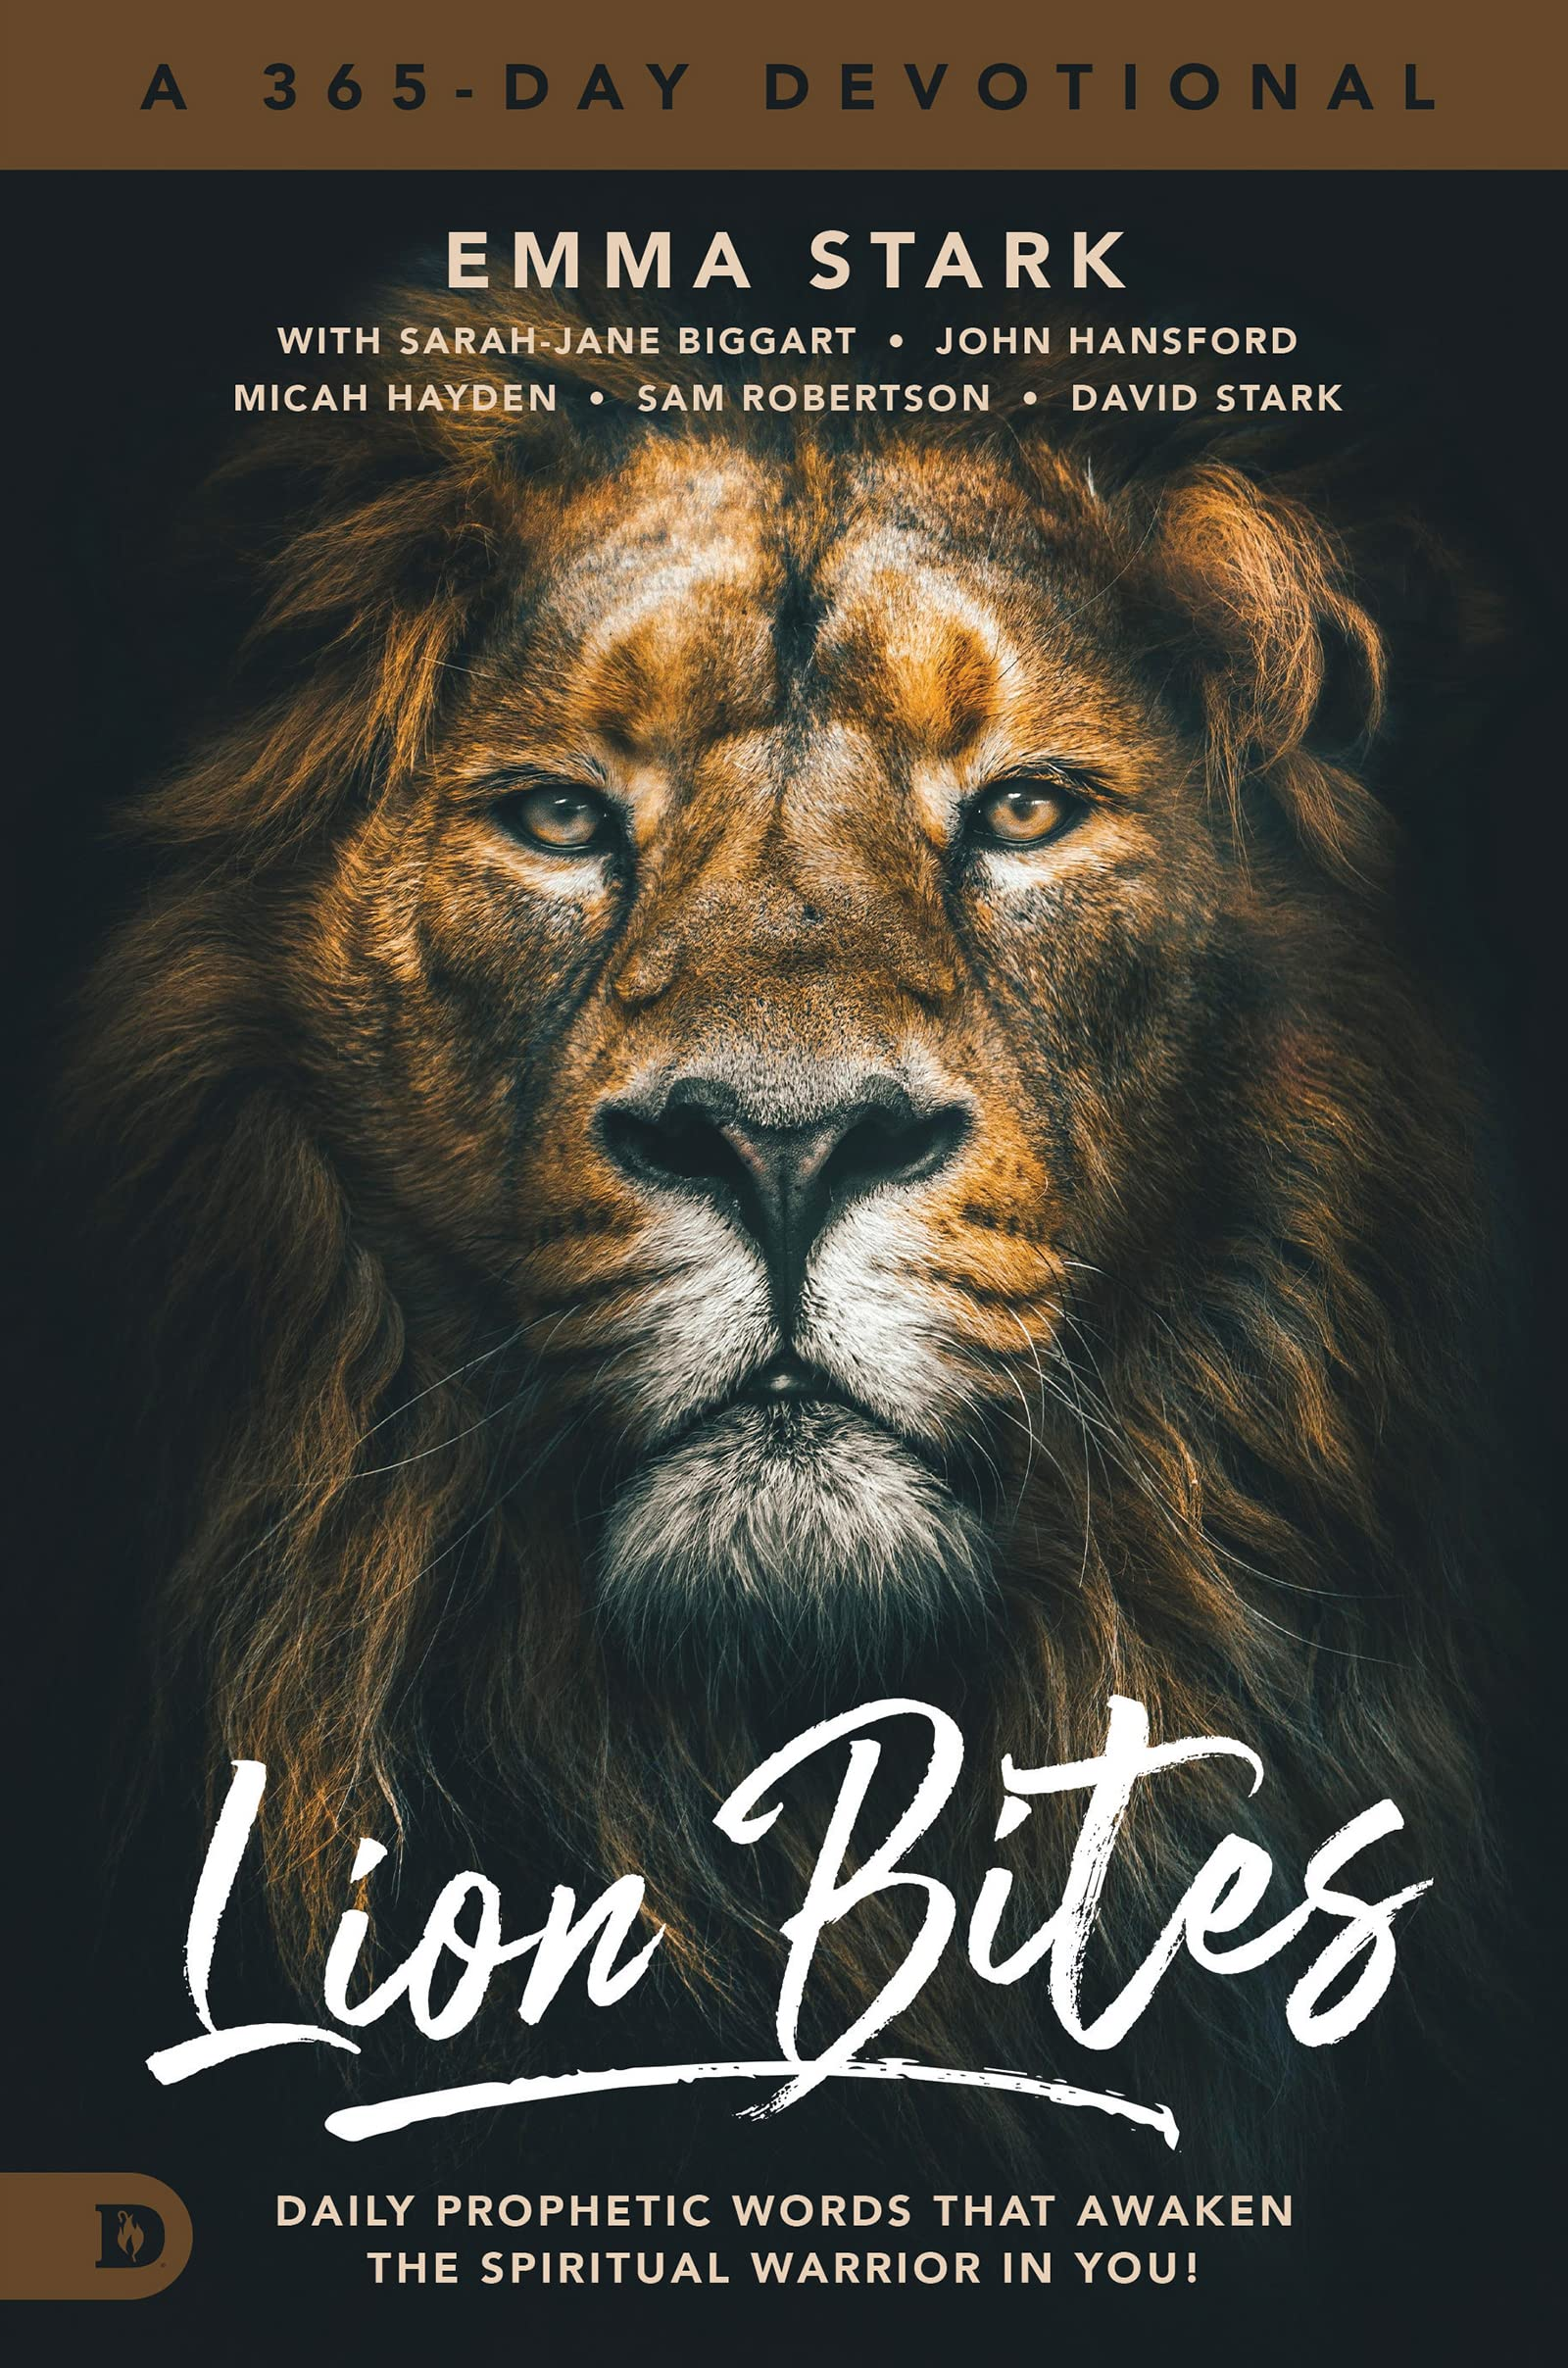} & 
\includegraphics[width=0.1\linewidth, height=0.145\linewidth]{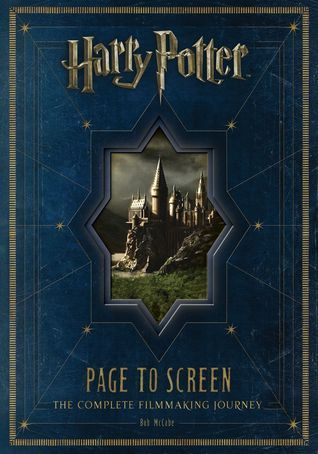} & 
\includegraphics[width=0.1\linewidth, height=0.145\linewidth]{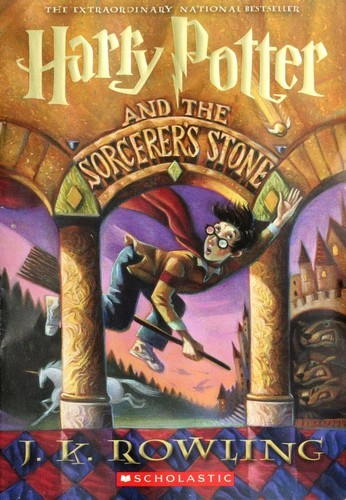} &
\includegraphics[width=0.1\linewidth, height=0.145\linewidth]{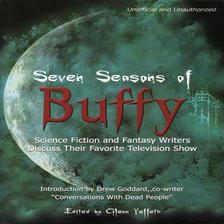} & 
\includegraphics[width=0.1\linewidth, height=0.145\linewidth]{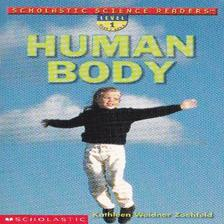} & 
\includegraphics[width=0.1\linewidth, height=0.145\linewidth]{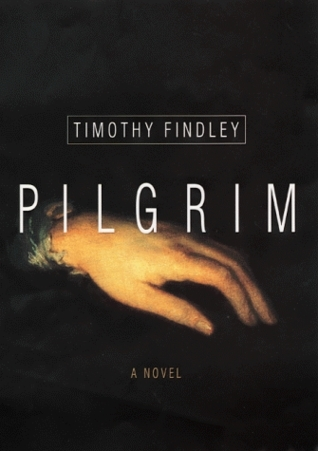} & 
\includegraphics[width=0.1\linewidth, height=0.145\linewidth]{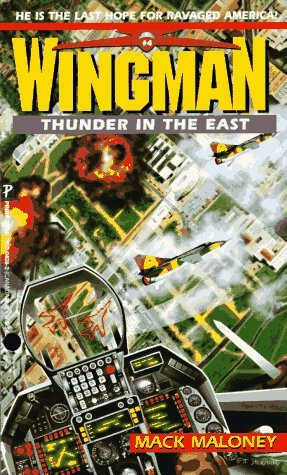} \\ 
\textcolor{blue}{\emph{xvii.}} F : (29, 27, 4) & \textcolor{blue}{\emph{xviii.}}  NF : (20) & \textcolor{blue}{\emph{xix.}}  NF : (22, 19, 27) & \textcolor{blue}{\emph{xx.}}  F : (2, 4, 16, 27) & 
\textcolor{blue}{\emph{xxi.}}  NF : (2, 24) & \textcolor{blue}{\emph{xxii.}}  NF : (2, 24) & \textcolor{blue}{\emph{xxiii.}}  F : (13, 14, 16, 29) & \textcolor{blue}{\emph{xxiv.}}  F : (13, 14, 16, 19)  \\ 
\multicolumn{2}{c|}{Inter-variation} & \multicolumn{2}{c||}{Inter-variation} & \multicolumn{2}{c|}{Intra-variation} & \multicolumn{2}{c}{Intra-variation}\\ 
%%%%%%%%%%%%%%%
\hline 
&&& &&&&  \\[\dimexpr-\normalbaselineskip+1.5pt]
\includegraphics[width=0.1\linewidth, height=0.145\linewidth]{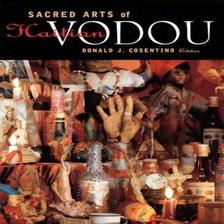} & 
\includegraphics[width=0.1\linewidth, height=0.145\linewidth]{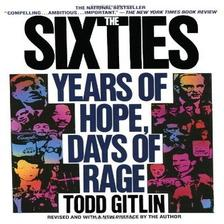} & 
\includegraphics[width=0.1\linewidth, height=0.145\linewidth]{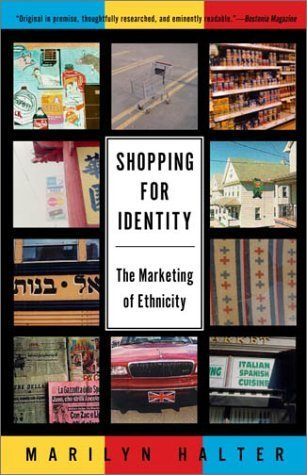} & 
\includegraphics[width=0.1\linewidth, height=0.145\linewidth]{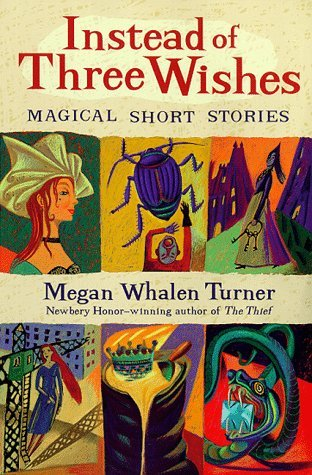} &
\includegraphics[width=0.1\linewidth, height=0.145\linewidth]{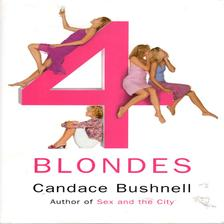} & 
\includegraphics[width=0.1\linewidth, height=0.145\linewidth]{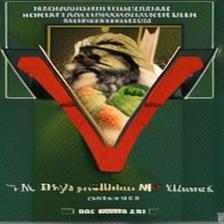} & 
\includegraphics[width=0.1\linewidth, height=0.145\linewidth]{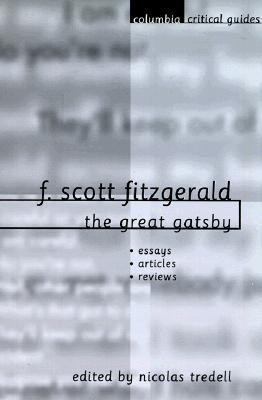} & 
\includegraphics[width=0.1\linewidth, height=0.145\linewidth]{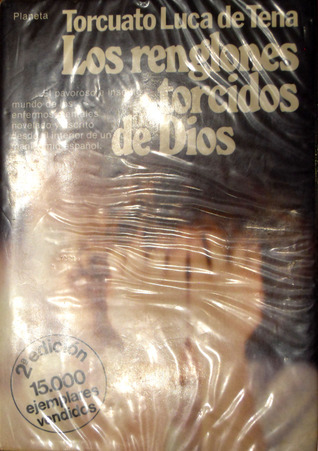} \\ 
\textcolor{blue}{\emph{xxv.}} NF : (2, 13, 20) & \textcolor{blue}{\emph{xxvi.}}  NF : (2, 13, 14) & \textcolor{blue}{\emph{xxvii.}}  NF : (3, 13, 14) & \textcolor{blue}{\emph{xxviii.}}  F : (4, 29, 27) & 
\textcolor{blue}{\emph{xxix.}}  F : (11, 16, 23) & \textcolor{blue}{\emph{xxx.}}  F : (21, 29) & \textcolor{blue}{\emph{xxxi.}} F : (16, 27, 13) & \textcolor{blue}{\emph{xxxii.}}  F : (14, 16, 17) \\ 
\multicolumn{4}{c||}{Collage} & \multicolumn{2}{c|}{Number/ letter as image} & \multicolumn{2}{c}{Unclear image}\\
%%%%%%%%%%%%%%%
\hline
\end{tabular}
\end{adjustbox}
}
\caption{Examples of some challenging book cover images with mentioned issues}
\label{fig:challenge}
\end{figure*}

\begin{figure*}[t]
\centering
\footnotesize
\resizebox{\textwidth}{!}{
\begin{tabular}{c|c|c|c || c|c|c|c}
%%%%%%%%%%%%%%%
\hline 
&&& &&&&  \\[\dimexpr-\normalbaselineskip+1.5pt]
\includegraphics[width=0.1\linewidth, height=0.145\linewidth]{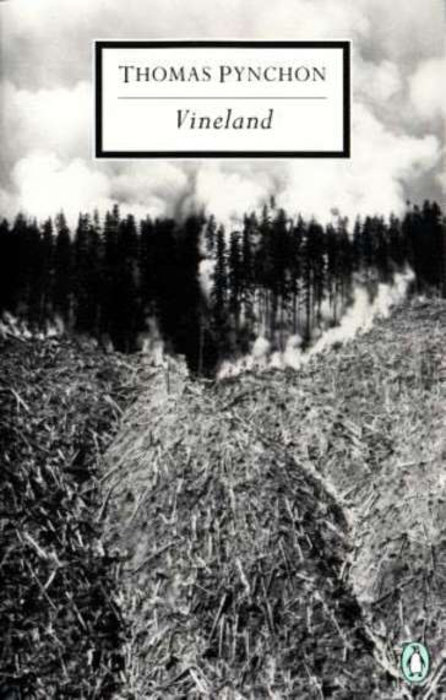} & 
\includegraphics[width=0.1\linewidth, height=0.145\linewidth]{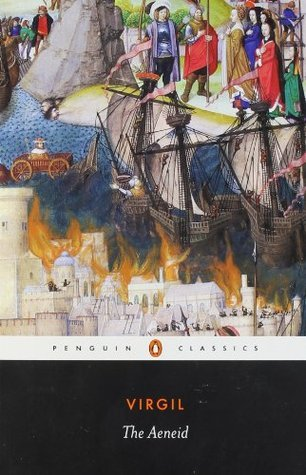} & 
\includegraphics[width=0.1\linewidth, height=0.145\linewidth]{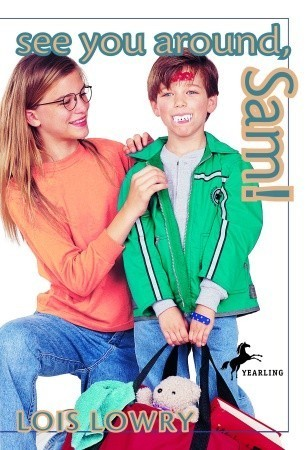} & 
\includegraphics[width=0.1\linewidth, height=0.145\linewidth]{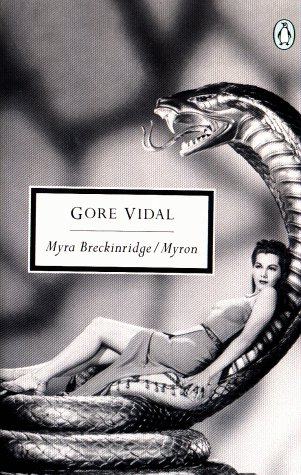} &
\includegraphics[width=0.1\linewidth, height=0.145\linewidth]{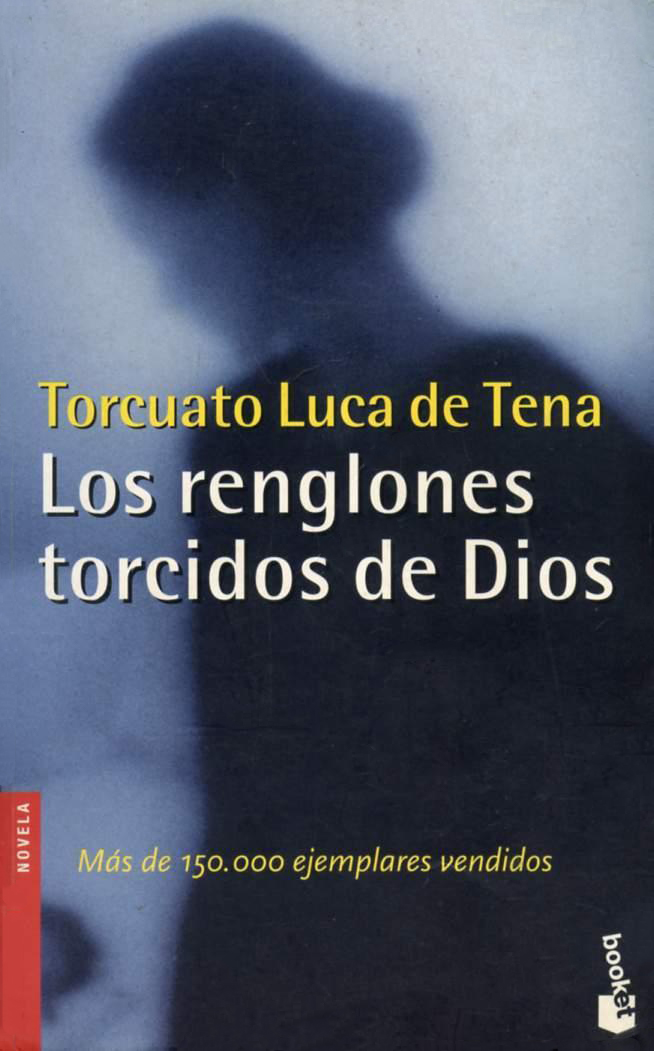} & 
\includegraphics[width=0.1\linewidth, height=0.145\linewidth]{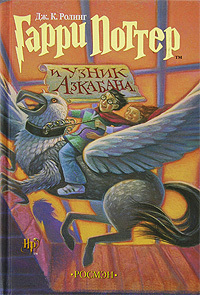} & 
\includegraphics[width=0.1\linewidth, height=0.145\linewidth]{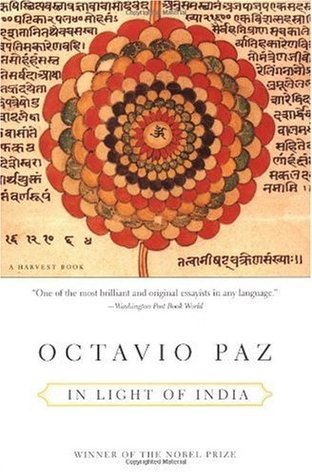} &
\includegraphics[width=0.1\linewidth, height=0.145\linewidth]{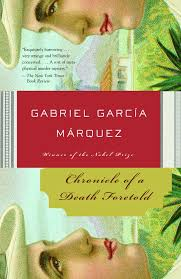}\\
\textcolor{blue}{\emph{i.}} F : (16) & \textcolor{blue}{\emph{ii.}}  F : (16, 20, 29, 27) & \textcolor{blue}{\emph{iii.}}  F : (4, 27) & \textcolor{blue}{\emph{iv.}}  F : (11, 14, 16) & 
\textcolor{blue}{\emph{v.}}  F : (13, 16, 28) & \textcolor{blue}{\emph{vi.}}  F : (2, 4, 29, 27) & \textcolor{blue}{\emph{vii.}} NF : (13, 16, 28) & \textcolor{blue}{\emph{viii.}}  F : (22, 29) \\ 
\multicolumn{4}{c||}{Limited information} & \multicolumn{4}{c}{Non-English cover text}\\
%%%%%%%%%%%%%%%

%%%%%%%%%%%%%%%
\hline 
&&& &&&&  \\[\dimexpr-\normalbaselineskip+1.5pt]
\includegraphics[width=0.1\linewidth, height=0.145\linewidth]{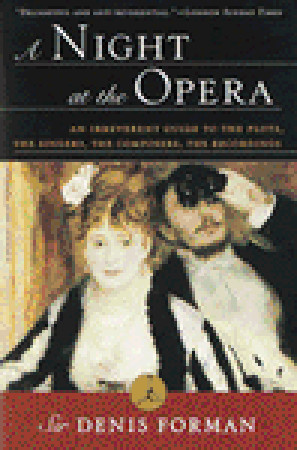} & 
\includegraphics[width=0.1\linewidth, height=0.145\linewidth]{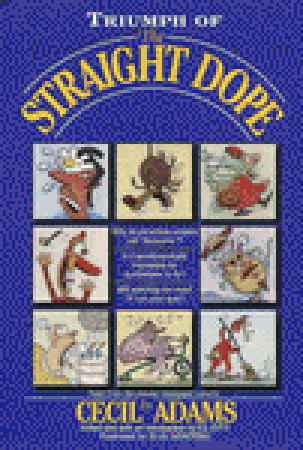} & 
\includegraphics[width=0.1\linewidth, height=0.145\linewidth]{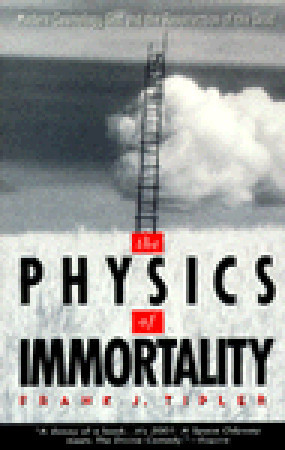} & 
\includegraphics[width=0.1\linewidth, height=0.145\linewidth]{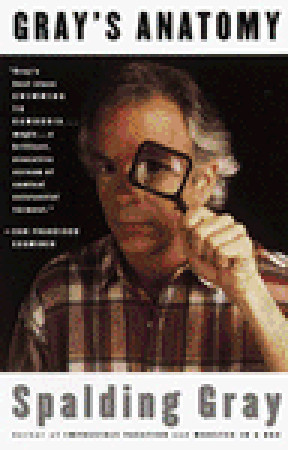} &
\includegraphics[width=0.1\linewidth, height=0.145\linewidth]{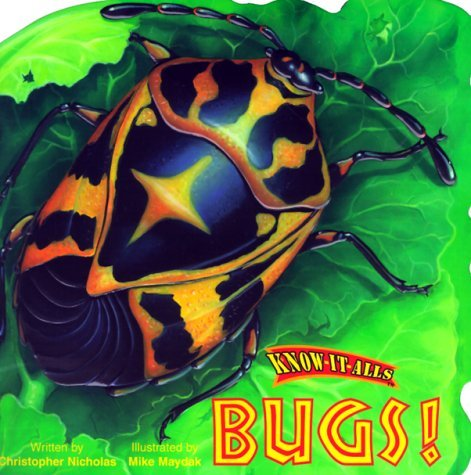} & 
\includegraphics[width=0.1\linewidth, height=0.145\linewidth]{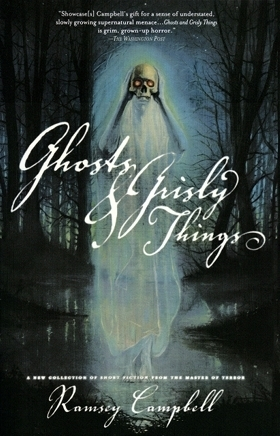} & 
\includegraphics[width=0.1\linewidth, height=0.145\linewidth]{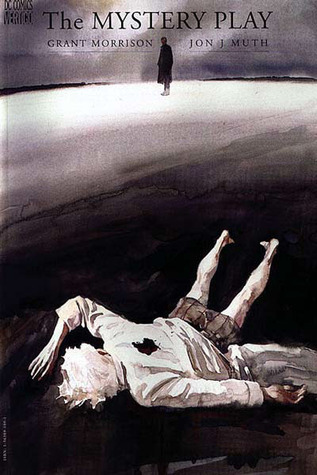} & 
\includegraphics[width=0.1\linewidth, height=0.145\linewidth]{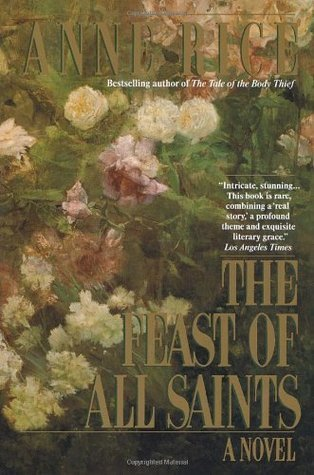}\\ 

\textcolor{blue}{\emph{ix.}} NF : (2, 13, 22) & \textcolor{blue}{\emph{x.}}  NF : (15, 22) & \textcolor{blue}{\emph{xi.}}  NF : (14, 20, 24) & \textcolor{blue}{\emph{xii.}}  NF : (13, 14, 24) & 
\textcolor{blue}{\emph{xiii.}}  NF : (1, 2, 4) & \textcolor{blue}{\emph{xiv.}}  F : (17,24, 29) & \textcolor{blue}{\emph{xv.}} F : (5, 17) & \textcolor{blue}{\emph{xvi.}}  F : (13, 17, 29) \\ 
\multicolumn{4}{c||}{Low resolution cover images} & \multicolumn{4}{c}{Complex background}\\
%%%%%%%%%%%%%%%
\hline
\end{tabular}
}
% \caption{Some challenges of extracting OCR from book cover page}
% \caption{Some challenges of extracted text from cover page}
\caption{Examples of some challenging cases involving text on cover page}
\label{fig:challenge_ocr}
\end{figure*}

% Examples of complex cases involving text elements on book covers.
% involving text on book covers

%%%%
   %%         1->'Animals & Wild life & Pets',
   %%		   2->'Arts & Photography',
   %%	       3->'Business & Money',
   %%	   4->'Childrens Book',
   %%	   5->'Comics & Graphic',
   %%		6->'Computers & Technology',
   %%		7->'Cookbooks & Food & Wine',
   %%		8->'Crafts & Hobbies & Home',
   %%		9->'Environment & Plant',
   %%		10->'Family & Parenting & Relationships',
   %%		11->'Fashion & Lifestyle',
   %%		12->'Health & Fitness & Dieting',
   %%		13->'History',
   %%		14->'Humanities',
   %%		15->'Humor & Entertainment',
   %%		16->'Literature',
   %%		17->'Mystery & Thriller & Suspense & Horror',
   %%		18->'Medical',
   %%		19->'Meta Text', 
   %%		20->'Mythology & Religion & Spirituality',
   %%		21->'Press & Media',
   %%		22->'Reference & Language',
   %%		23->'Romance',
   %%		24->'Science & Math & Mathematics',
   %%		25->'Self-Help & Motivation',
   %%		26->'Sports & Outdoors',
   %%		27->'Teen & Young Adult',
   %%		28->'Travel',
   %%		29->'Science Fiction & Fantasy'

  %%

\noindent
We identified several key challenges within each modality of our dataset, which are outlined below. 

%================================================
\subsection{Challenges in Cover Image}
\noindent
The complexity of book cover images poses challenges in accurately identifying book genres. 

\subsubsection{Background}
Book cover image background plays a crucial role in setting the tone or mood, sparking interest, and assisting readers in determining whether the book aligns with their tastes and preferences.
For instance, \emph{sci-fi \& fantasy} book covers frequently showcase detailed background elements, featuring enchanting landscapes and vivid colors, designed to captivate readers with a sense of wonder and adventure (Fig. \ref{fig:challenge}: \emph{viii}). 
Based on the visual cues available in the background of the cover image, we can group it as follows:

\paragraph{Limited Visual Cues} Sometimes, the cover page provides minimal or no visual information, containing only text in standard fonts, making genre identification challenging (Fig.s \ref{fig:challenge}: \emph{i-ii}).

\paragraph{Moderate Information} 
The cover page often includes moderate visual features to represent some of its genres but may fail to capture others due to the multi-label nature of genres (Fig.s \ref{fig:challenge}: \emph{v-viii}).

\paragraph{Complex Background} In some instances, the background of a book cover image becomes convoluted due to the presence of extensive or composite visual effects or elements (Fig.s \ref{fig:challenge}: \emph{iii-iv}).

%================================================

\subsubsection{Foreground}
The foreground of a book cover image plays a vital role in capturing reader attention. 
However, foreground images on book covers pose challenges for genre identification due to ambiguity, cross-genre similarities, abstract designs, stylistic variations, cultural influences, evolving trends, and marketing-driven misrepresentations. 

\paragraph{Living/ Non-living Element} 
The foreground image can effectively communicate the book theme or atmosphere by strategically placing engaging foreground elements. 
Some non-living elements (e.g., mountain, sea, etc.) are typically associated with genres like \emph{travel}. 
However, in some cases (Fig. \ref{fig:challenge}: \emph{x}), such elements are used to represent genres like 
\emph{literature}, 
\emph{mystery \& thriller \& suspense \& horror \& adventure}, 
\emph{romance}, and
\emph{sci-fi \& fantasy}, 
which creates a disconnect and makes genre identification challenging. 
Similarly, living objects contribute to this ambiguity. 
For example, while an animal on the cover often implies a connection to genres like \emph{animals \& wildlife \& pets}, 
there are instances (Fig. \ref{fig:challenge}: \emph{xi-xii}) 
where this association does not hold, making genre identification more challenging.

\paragraph{Scene Image} 
Scene-based images on book covers further complicate genre prediction due to their intricate visual details, clutter, and lack of a cohesive composition (Fig.s \ref{fig:challenge}: \emph{xiii-xvi}). Unlike single-object covers, scene-based images often contain multiple elements—characters, landscapes, objects, or action sequences—that may belong to different genres. This complexity increases ambiguity, as the dominant visual theme may not be immediately apparent. 
Additionally, certain scenes may be common across multiple genres, making classification more challenging. 
Variations in artistic styles, lighting, and color palettes further contribute to genre ambiguity. 

%================================================

\subsubsection{Inter-Variation}
Sometimes, books from different genres may contain similar visual information (Fig.s  \ref{fig:challenge}: \emph{xvii-xviii}, and Fig.s  \ref{fig:challenge}: \emph{xix-xx}). This may be intentional to challenge reader expectations, create intrigue, or highlight genre blends.
For example, cover image of Fig. \ref{fig:challenge}: \emph{xvii} comprises genres  
\emph{childrens' book}, 
\emph{comics \& graphics}, 
\emph{sci-fi \& fantasy}, 
\emph{teen \& young adult}, but another book's cover image (Fig \ref{fig:challenge}: \emph{xviii}) with similar visual cues belongs to \emph{arts \& photography}.

%================================================

\subsubsection{Intra-Variation}
The visual styles and design elements used in cover images within a specific genre can vary widely. 
This variation is often influenced by the author/artist's unique vision and the intended mood of the book, resulting in diverse interpretations of the same genre. 
Additionally, publishers frequently adhere to specific house styles or branding guidelines, incorporating consistent visual elements or color schemes across their catalog. 
While this ensures some level of uniformity within a publisher's collection, the broader diversity in design choices makes genre identification more challenging 
(Fig.s \ref{fig:challenge}: \emph{xxi-xxii}, and Fig.s \ref{fig:challenge}: \emph{xxiii-xxiv}).

%====================================

\subsubsection{Collage}
In some cases, book covers integrate multiple aforementioned background and foreground elements, forming a collage of numerous smaller images. This visual complexity often leads to information overload, making it challenging to accurately determine the book’s genre (Fig.s \ref{fig:challenge}: \emph{xxv-xxviii}).

%====================================
\subsubsection{Number/ Letter as Image}
Occasionally, book covers feature numbers or letters stylized as visual elements. This artistic choice is often intended to emphasize a theme, establish a distinctive style, or highlight key information related to the book’s content. However, such designs pose a unique challenge for genre identification, as the graphical representation of text or numbers can obscure their intended meaning, making interpretation more difficult (Fig.s \ref{fig:challenge}: \emph{xxix-xxx}).

%====================================
\subsubsection{Unclear Image}
Sometimes, book covers feature images that are blurry, hazy, or of low resolution. Extracting meaningful features from such images becomes difficult, making accurate genre identification challenging (Fig.s \ref{fig:challenge}: \emph{xxxi-xxxii}).

%====================================

%====================================

\subsection{Challenges in Cover Text}
\noindent
We extracted text from book cover images using an OCR (Optical Character Recognition) engine. However, these extracted texts present additional challenges, which we summarize below.

%====================================
\subsubsection{Limited Text}
Some book covers feature only minimal text, such as the author name, or the book title, without supplementary elements like subtitles, or descriptive taglines. These additional details often play a crucial role in genre identification. The absence of such details forces the OCR system to rely solely on sparse information, significantly increasing the risk of misclassification (Fig.s \ref{fig:challenge_ocr}: \emph{i-iv}).

%====================================
\subsubsection{Linguistic Issues}
OCR systems are often designed with a primary focus on specific languages, e.g., English. When book covers feature text in non-English languages, these systems may face difficulties in accurately recognizing and processing the characters. Errors in language detection or character recognition can lead to misinterpretations, further complicating text-based genre classification (Fig. \ref{fig:challenge_ocr}: \emph{v-viii}).

%====================================
\subsubsection{Low Resolution Cover Page}
Low-quality and glossy book covers present significant challenges for accurate text extraction using OCR. Glossy surfaces can create glare and reflections when photographed or scanned, interfering with character recognition. Additionally, low-resolution images often result in blurred text, making it difficult to distinguish individual characters. These factors contribute to errors in text extraction and misinterpretation (Fig.s \ref{fig:challenge_ocr}: \emph{ix-xii}).

%====================================
\subsubsection{Complex background}
Colorful or busy backgrounds on book covers present a significant challenge for OCR systems. These complex backgrounds can interfere with the OCR process in several ways:

        \paragraph{Visual Clutter}
        A busy background with multiple colors, patterns, or images can create visual clutter. This clutter makes it difficult for the OCR system to distinguish the text from the background. The presence of various elements can cause the OCR algorithm to misidentify parts of the background as text or fail to recognize the text altogether (Fig.s \ref{fig:challenge_ocr}: \emph{xiii-xvi}).
        
        \paragraph{Color Contrast}
        Text on colorful backgrounds might not have sufficient contrast. When the text color closely matches the background colors, the OCR system struggles to differentiate between them. High contrast between text and background is crucial for accurate OCR, and colorful backgrounds often fail to provide this (Fig.s \ref{fig:challenge_ocr}: \emph{xiii-xvi}).

%====================================

%====================================
\subsection{Challenges in Blurb}

\noindent
The blurb often contains genre-related textual information. However, there are difficulties in accurately identifying genres based on the blurb text. These challenges are briefly outlined below: 

%====================================
\subsubsection{Insufficient Information}
There are several books containing blurb, often lacked the necessary detail to determine the book’s genre accurately. 
For example: 
The book \emph{Peter Pan} (ISBN-13: \emph{9780881011111}) has the blurb \textquotedblleft Book by J.M. Barrie\textquotedblright. Now, from just the information about the author, it is hard to determine the book genres.

%====================================
\subsubsection{Irrelevant Information}
% \emph {\textbf{(b) Irrelevant information}}: 
We encounter many books containing irrelevant information in the blurb. These blurbs frequently consist of vague or generic statements, contributing little to the genre's understanding, making genre identification difficult. 
For instance:
\begin{itemize}[---]
\item The book titles \emph{Pedagogy of the Oppressed} (ISBN-13: \emph{9780826400475}) has the blurb \textquotedblleft SIGNED COPY BY THE AUTHOR\textquotedblright. This information is very irrelevant to identifying book genres.
\end{itemize}

%====================================
\subsubsection{Multilinguality}
% \emph{\textbf{(c) Multilinguality}}:
Blurb texts are available in various languages, each with its own script and sentence structure. This lack of uniformity makes it difficult to build a framework that can effectively understand and process multiple languages. 
%Each language uses different scripts and sentence structures cause different handling. The lack of uniformity in language led to challenges in building a framework that understands multiple languages.

\begin{itemize}[---]
    \item The book \emph{Michelangelo} (ISBN-13: \emph{9783499222290}) has the blurb in the German -  \textquotedblleft In dem vor Vitalität berstenden Stadtstaat Florenz des 16. Jahrhunderts kämpfte eines der universalen Genies der Menschheitsgeschichte wie ein Titan gegen Kardinäle, Fürsten und Päpste. Rivalitäten mit berühmten Zeitgenossen wie Leonardo da Vinci und Raffael machten ihm das Leben ebenso schwer wie seine eigene dämonische Natur. In den Wirren einer zwischen üppigem Prunk und ständigen Kriegen zerrissenen Zeit schuf Michelangelo, "Gottes eigenes Kind", sein unsterbliches Werk.\textquotedblright
\end{itemize}

%====================================

%====================================
\subsection{Challenges of Metadata}
\noindent
There are several challenges for identifying book genres using book metadata information. We summarized those challenges as follows.

%==========================
\subsubsection{Surface-Level Information}
% \emph{\textbf{(a) Surface-Level Information}}: 
Metadata doesn't reveal a user's deeper interests, reading level, or genre preferences. One author writes books on different genres. So, someone who enjoys a particular author might not like all of their books.

%====================================
%====================================

\subsection{Challenges of Ground-Truthing}
\noindent
Establishing reliable ground-truth genre labels presented significant challenges due to the inherent subjectivity and complexity of the task. 

\subsubsection{Partial Understanding by Human Annotators} 
Since it is often impractical for annotators to read an entire book, the ground-truthing process primarily relied on linguistic experts who assigned genre labels based on limited content—such as publisher blurbs, user reviews (e.g., from Goodreads), and selected excerpts. This partial exposure may lead to a superficial or incomplete understanding of the book’s thematic nuances, thereby impacting the accuracy of genre labeling.

\subsubsection{Subjectivity and Inconsistency in Genre Interpretation} 
Genre classification is often influenced by subjective interpretation. Annotators might interpret the same book differently based on the emphasis placed on particular elements. For instance, a book that blends psychological drama and crime might be labeled as \emph{thriller} by one expert, and as \emph{mystery} or \emph{drama} by another, depending on their reading perspective.

\subsubsection{Fiction vs. Non-fiction Ambiguities}
Differentiating between fiction and non-fiction genres was particularly challenging for works related to well-known fictional universes. For example, while a “\emph{Harry Potter}” novel is clearly fiction, a companion book like "\emph{Harry Potter \--- Page to Screen: The Complete Filmmaking Journey}" is non-fiction, despite sharing the same universe and characters. Such genre-conflicting edge cases complicated the labeling process, requiring careful contextual analysis.

\subsubsection{Multi-Label Overlaps and Unclear Boundaries} 
Many books span multiple genres, making it difficult to determine which labels are most appropriate and at what level of the hierarchy. 
% For example, a book might simultaneously belong to “Fantasy,” “Young Adult,” and “Adventure,” but experts may vary in how broadly or narrowly they assign labels, especially without formal guidelines.

\subsubsection{Lack of Standardized Taxonomy} 
Genre taxonomies vary significantly across publishers, retailers, and literary databases, resulting in inconsistent ground-truth references. Aligning expert annotations with a unified genre hierarchy was non-trivial and often required manual reconciliation.

% Reviewer Bias in Indirect Labeling:
% When annotations were based on user reviews or crowdsourced content, they were susceptible to bias or misinterpretation. Reviewers may focus on personal opinions or plot elements irrelevant to genre classification, leading to noise in genre inference.

%====================================

\subsection{Challenges of Overall Dataset}
\noindent
In preparing a high-quality dataset for hierarchical multi-label book genre classification, several overarching challenges emerged, particularly due to the multi-label nature of the task and the complexity of real-world genre distributions.

\subsubsection{Label Imbalance in Multi-Label Context} 
The dataset exhibits significant class imbalance, with certain genres being highly represented, while others appear far less frequently. However, unlike single-label classification, this imbalance cannot be easily corrected through traditional resampling techniques because books often belong to multiple genres simultaneously. Balancing one under-represented genre could unintentionally disrupt the co-occurrence patterns with more frequent genre.

\subsubsection{Constraints in Data Augmentation} 
Augmentation techniques commonly used to balance datasets pose unique risks in the multi-label setting. When augmenting samples from a genre with few examples, the co-occurring genres in the original sample—many of which may already be overrepresented—also get replicated. This reinforces existing imbalance and biases, making it difficult to selectively boost specific genre classes without inadvertently inflating others.}

\subsubsection{Sparse Label Combinations} 
The multi-label setting also leads to a large number of unique label combinations, many of which appear very infrequently. This sparsity in the label space challenges the model’s ability to generalize well to unseen or rare combinations and limits the effectiveness of frequency-based heuristics.

\subsubsection{Dependency Between Genre Labels} 
Usually genre labels are not mutually independent; the presence of one genre may often influence the likelihood of another. Modeling these dependencies becomes increasingly difficult as the number of labels grows, especially under imbalance and sparsity, and it further complicates synthetic balancing or sampling strategies.

%====================================
% \subsection{Challenges of Multi-Class Labeling}
% \noindent
% Multi-labeling of book genres presents several challenges, including:

% \textbullet~ \emph{Visual ambiguity}: Book covers often contain elements that are relevant to multiple genres, making it difficult to assign distinct labels.

% \textbullet~ \emph{Feature overlap}: Certain visual and textual features may be common across different genres, leading to misclassification.

% \textbullet~\emph{Sparse representation}: Some genres may have limited representation in the dataset, making it harder for models to learn their distinguishing features.

% \textbullet~\emph{Inter-genre dependencies}: Some genres frequently co-occur (e.g., Fantasy and Adventure), requiring models to capture complex relationships between labels.

% \textbullet~\emph{Minimal visual cues}: Some book covers lack strong genre-specific visual elements, relying more on textual information, which may not always be available.

% \textbullet~\emph{Subjective labeling}: Genre classification can be subjective, as the same book may be perceived differently by different annotators.

% \textbullet~ \emph{Scalability issues}: As the number of genres increases, assigning multiple labels accurately becomes more computationally intensive.
\section{Data Processing}
\label{app:data_processing}

\noindent
Below we discuss data augmentation followed by data preprocessing.

\subsection{{Data Augmentation}} 
\noindent
We observed that some specific genres within both fiction and non-fiction had insufficient samples. While these genres did not have enough samples to be removed, the limited information in these samples hindered the effective training of our models. We utilized data augmentation methods to generate new samples for these genres. We discuss data augmentation methods below in detail:

\subsubsection{Visual Data Augmentation}
% \emph{\textbf{(a) Visual Data Augmentation}}: 
To enhance the diversity of the dataset, we employed \textquoteleft{Stable-diffusion-xl-refiner-1.0'} \cite{stable-diffusion-xl-refiner-1.0} for coverpage data augmentation. The diffusion model generates high-quality synthetic data by progressively adding noise to the original data and then learning to reverse this process.

\subsubsection{Textual Data Augmentation}
% \emph{\textbf{(b) Textual Data Augmentation}}: 
To augment description text, we used GEMINI \cite{gemini} a large language model to generate additional description text from the existing one. Through prompt engineering techniques, we ensured that the generated content accurately retained the contextual meaning and relevance of the original data.

\subsection{{Data Preprocessing}}
\noindent
Data preprocessing is the initial step in data analysis, where raw data is transformed into a suitable format for further analysis. We resized coverpage ${\cal{I}}$ into $3 \times 224 \times 224$. Description text ${\cal{T}}$ and cover text ${\cal{C}}$ went through multiple preprocessing steps. First, we remove stop words of the english language and the articles (a, an, the), then we remove string punctuation from them.

% \clearpage

% Additional content starting from a new page
% For example:

\section{Statistical Information}

%Hierarchical Genrewise

%Visual (Resolution, Size)

%Description (word count, processed w/o stopwords)
%\begin{enumerate}

In Table \ref{tab:dataset_table}, we present the hierarchical analysis of book counts by genre. The dataset includes 30 genres. This table provides counts for fiction and nonfiction books separately within each genre. In the table, we can observe overlapping counts across genres due to some books are associated with multiple genres.
The dataset was split up into training (${\cal{D}}_{train}$), validation (${\cal{D}}_{val}$), and testing (${\cal{D}}_{test}$) disjoint sets with an approximate ratio of 8:1:1 considering the presence of all genres in each set equivalently.
Additionally, we employ data augmentation techniques for the cover page images and descriptions to enhance the number of available samples. 
%Before data augmentation, training, validation, and testing sets contained 8972, 1152, and 1178 samples. After data augmentation, training, validation, and testing sets contained 22340, 2804, and 2809 samples.  

Table \ref{tab:all_stats} presents the statistical analysis of each modality before and after augmentation. We have used minimum, maximum, mean ($\mu$), median, and standard deviation ($\sigma$) for statistical analysis. We are measuring the dataset based on the image area for the cover page image, the number of words for the description text and cover text, and the number of books written/published by the author/publisher for metadata.

We also provide the distribution of each modality before and after augmentation. Table \ref{tab:stats_coverpage} shows the area-wise distribution of cover page images. In Fig. \ref{tab:stats_description}, we demonstrate word count-wise distribution of description text. Fig. \ref{tab:stats_cover_text} presents word count-wise distribution of cover text and Fig. \ref{tab:stats_metadata} provides a breakdown of the number of books authored within specific
ranges and the corresponding count of authors who fall into that range, similarly the number of books published within ranges and the number of publishers associated with that range. This analysis provides valuable insights into the dataset.

\begin{table}[!hbt]
 \centering
 \caption{Statistical analysis}
 %\vspace{1em} % Adjust the vertical space here
 \begin{adjustbox}{width=0.47\textwidth}
 \begin{tabular}{c|c|c|c|c|c|c}
\hline
   \textbf{Input} & 
   
& \textbf{Minimum} & \textbf{Maximum} & \textbf{Mean ($\mu$)} & \textbf{Median} & \textbf{SD ($\sigma$)}\\ \hline

& Image area before & \multirow{2}{*}{20460} & \multirow{2}{*}{16301712} & \multirow{2}{*}{435282.41} & \multirow{2}{*}{146775} & \multirow{2}{*}{1125224.73}\\

\textbf{Cover page} & augmentation & & & & & \\
\cline{2-7}
\textbf{images} & Image area after & \multirow{2}{*}{20460} & \multirow{2}{*}{16301712} & \multirow{2}{*}{325205.84} & \multirow{2}{*}{135850} & \multirow{2}{*}{980565.34}\\ 
& augmentation & & & & & \\
\hline

& No. of words before & \multirow{2}{*}{0} & \multirow{2}{*}{1786} & \multirow{2}{*}{120.52} & \multirow{2}{*}{98} & \multirow{2}{*}{102.37}\\ 
   
\textbf{Description} & augmentation & & & & & \\
\cline{2-7}

\textbf{text} & No. of words after & \multirow{2}{*}{0} & \multirow{2}{*}{1953} & \multirow{2}{*}{110.01} & \multirow{2}{*}{96} & \multirow{2}{*}{80.89}\\ 

& augmentation & & & & & \\
\hline

\multirow{4}{*}{\textbf{Cover text}} & No. of words  & \multirow{3}{*}{1} & \multirow{3}{*}{944} & \multirow{3}{*}{20.67} & \multirow{3}{*}{15} & \multirow{3}{*}{27.69}\\

& before augmentation & & & & & \\ \cline{2-7}

 & No. of words  & \multirow{3}{*}{1} & \multirow{3}{*}{944} & \multirow{3}{*}{21.61} & \multirow{3}{*}{16} & \multirow{3}{*}{25.89}\\
& after augmentation & & & & & \\
   
\hline

& No. of books  & \multirow{2}{*}{1} & \multirow{2}{*}{43} & \multirow{2}{*}{1.57} & \multirow{2}{*}{1} & \multirow{2}{*}{1.91}\\ 

\textbf{Metadata} & written by an author & & & & & \\

\cline{2-7}
& No. of books  & \multirow{2}{*}{1} & \multirow{2}{*}{268} & \multirow{2}{*}{5.80} & \multirow{2}{*}{1} & \multirow{2}{*}{16.64}\\ 
   
& published by a publisher & & & & & \\

\hline

   \multicolumn{7}{r}{SD: Standard Deviation}
 \end{tabular}
\end{adjustbox}
\label{tab:all_stats}
 \end{table}

\begin{table}[!hbt]
\centering  
% \footnotesize
% \caption{ Image area-wise distribution  before and after augmentation} 
% \caption{Statistics analysis of cover page images}
\caption{Image area-wise distribution of cover page}
\begin{adjustbox}{width=0.47\textwidth}
\begin{tabular}{c|c|c}%{p{2.5cm}|p{2.5cm}|p{2.5cm}}
\hline
Image area range  & Number of samples before & Number of samples after\\
(10000 pixel$^2$) & augmentation & augmentation \\
\hline 
< 5 & 20 & 50\\
5 \--- 10 & 264 & 9847\\
10 \--- 15 & 7039 & 11104\\
15 \--- 20 & 2194 & 3895\\
20 \--- 25 & 275 & 574\\
25 \--- 30 & 120 & 243\\
30 \--- 35 & 51 & 86\\
35 \--- 40 & 41 & 63\\
> 40 & 1298 & 2091\\
 \hline
\end{tabular}
\end{adjustbox}
\label{tab:stats_coverpage}
\end{table}

\begin{figure}[!hbt]
    \centering
    \begin{subfigure}{0.24\textwidth}
        \begin{tikzpicture}[scale=0.48]
        \begin{axis}[
        ybar,
        ymin=0,
        ymax=7000,
        ylabel={No. of samples},
        xlabel={Word count range},
        symbolic x coords={0 -- 100,101 -- 200,201 -- 300,301 -- 400,>400},
        xtick=data,
        ytick={1000,2000,3000,4000,5000,6000},
        nodes near coords,
        every node near coord/.append style={font=\large, yshift=5pt, color=black},
        tick label style={font=\large},
        label style={font=\Large},
        enlarge x limits=0.15,
        ymajorgrids=true,
        xmajorgrids=false,
        xticklabel style={rotate=90, anchor=east},
        ]
        \addplot+[fill=red, color=red]  coordinates {(0 -- 100,5788) (101 -- 200,3524) (201 -- 300,1370) (301 -- 400,422) (>400,187)};
        \end{axis}
    \end{tikzpicture}
    \caption{before augmentation}
    \end{subfigure}
    \hfill
     \begin{subfigure}{0.24\textwidth}
        \begin{tikzpicture}[scale=0.48]
        \begin{axis}[
        ybar,
        ymin=0,
        ymax=17500,
        ylabel={No. of samples},
        xlabel={Word count range},
        symbolic x coords={0 -- 100,101 -- 200,201 -- 300,301 -- 400,>400},
        xtick=data,
        ytick={2500,5000,7500,10000,12500,15000},
        nodes near coords,
        every node near coord/.append style={font=\large, yshift=5pt, color=black},
        tick label style={font=\large},
        label style={font=\Large},
        enlarge x limits=0.15,
        ymajorgrids=true,
        xmajorgrids=false,
        xticklabel style={rotate=90, anchor=east},
        ]
        \addplot+[fill=blue, color=blue]  coordinates {(0 -- 100,14710) (101 -- 200,10222) (201 -- 300,2257) (301 -- 400,553) (>400,200)};
        \end{axis}
    \end{tikzpicture}
    \caption{after augmentation}
    \end{subfigure}
    \caption{(a)  Word count-wise distribution of description across sample}
    \label{tab:stats_description}
\end{figure}

\begin{figure}[!hbt]
    \centering
    \begin{subfigure}{0.24\textwidth}
        \begin{tikzpicture}[scale=0.48]
        \begin{axis}[
        ybar,
        ymin=0,
        ymax=8400,
        ylabel={No. of samples},
        xlabel={Word count range},
        symbolic x coords={0 -- 20,21 -- 40,41 -- 60,61 -- 80,81 -- 100,>100},
        xtick=data,
        ytick={1200,2400,3600,4800,6000,7200},
        nodes near coords,
        every node near coord/.append style={font=\large, yshift=5pt, color=black},
        tick label style={font=\large},
        label style={font=\Large},
        enlarge x limits=0.15,
        ymajorgrids=true,
        xmajorgrids=false,
        xticklabel style={rotate=90, anchor=east},
        ]
        \addplot+[fill=red, color=red]  coordinates {(0 -- 20,7421) (21 -- 40,2880) (41 -- 60,740) (61 -- 80,146) (81 -- 100,38) (>100,74) };
        \end{axis}
    \end{tikzpicture}
    \caption{before augmentation}
    \end{subfigure}
    % \hfill
     \begin{subfigure}{0.24\textwidth}
        \begin{tikzpicture}[scale=0.48]
        \begin{axis}[
        ybar,
        ymin=0,
        ymax=21000,
        ylabel={No. of samples},
        xlabel={Word count range},
        symbolic x coords={0 -- 20,21 -- 40,41 -- 60,61 -- 80,81 -- 100,>100},
        xtick=data,
        ytick={3000,6000,9000,12000,15000,18000},
        nodes near coords,
        every node near coord/.append style={font=\large, yshift=5pt, color=black},
        tick label style={font=\large},
        label style={font=\Large},
        enlarge x limits=0.15,
        ymajorgrids=true,
        xmajorgrids=false,
        xticklabel style={rotate=90, anchor=east},
        ]
        \addplot+[fill=blue, color=blue]  coordinates {(0 -- 20,17646) (21 -- 40,7476) (41 -- 60,2013) (61 -- 80,491) (81 -- 100,128)  (>100,199)};
        \end{axis}
    \end{tikzpicture}
    \caption{after augmentation}
    \end{subfigure}
    \caption{(a)  Word count-wise distribution of cover text across sample}
    \label{tab:stats_cover_text}
\end{figure}

\begin{figure}[!hbt]
    \centering
    % \begin{subfigure}{0.24\textwidth}
        \begin{tikzpicture}[scale=0.55]
        \begin{axis}[
        ybar,
        ymin=0,
        ymax=8000,
        ylabel={No. of authors},
        xlabel={No. of samples},
        symbolic x coords={0 -- 10,11 -- 20,21 -- 30,31 -- 40, >40},
        xtick=data,
        ytick={1000,2000,3000,4000,5000,6000, 7000},
        nodes near coords,
        every node near coord/.append style={font=\large, yshift=5pt, color=black},
        tick label style={font=\large},
        label style={font=\Large},
        enlarge x limits=0.15,
        ymajorgrids=true,
        xmajorgrids=false,
        xticklabel style={rotate=90, anchor=east},
        ]
        \addplot+[fill=red, color=red]  coordinates {(0 -- 10,7122) (11 -- 20,42) (21 -- 30,6) (31 -- 40,5) (>40,1)};
        \end{axis}
    \end{tikzpicture}
    % \caption{\footnotesize}
    % \end{subfigure}
    % \hfill
    %  \begin{subfigure}{0.24\textwidth}
    %     \begin{tikzpicture}[scale=0.48]
    %     \begin{axis}[
    %     ybar,
    %     ymin=0,
    %     ymax=2000,
    %     ylabel={No. of publisher},
    %     xlabel={No. of samples},
    %     symbolic x coords={0 -- 10,11 -- 20,21 -- 30,31 -- 40,41 -- 50, >50},
    %     xtick=data,
    %     ytick={250,500,750,1000,1250,1500, 1750},
    %     nodes near coords,
    %     every node near coord/.append style={font=\large, yshift=5pt, color=black},
    %     tick label style={font=\large},
    %     label style={font=\Large},
    %     enlarge x limits=0.15,
    %     ymajorgrids=true,
    %     xmajorgrids=false,
    %     xticklabel style={rotate=90, anchor=east},
    %     ]
    %     \addplot+[fill=blue, color=blue]  coordinates {(0 -- 10,1735) (11 -- 20,99) (21 -- 30,34) (31 -- 40,28) (41 -- 50,15) (>50,35)};
    %     \end{axis}
    % \end{tikzpicture}
    % \caption{\footnotesize No. of samples-wise distribution of publishers}
    % \end{subfigure}
    \caption{No. of samples-wise distribution of authors}
    \label{tab:stats_metadata}
\end{figure}

\section{Experimental Settings}
\label{app:experimental_settings}
\noindent
Table \ref{tab:settings} provides detailed experimental settings for each training stage. 
\begin{table}[!hbt]
\centering

\caption{Experimental settings details}
\begin{adjustbox}{width=0.4\textwidth} 
\begin{tabular}{c|l}
% \hline
% \multicolumn{2}{c}{System settings} \\ \hline

% Operating system & Ubuntu 20.04.4 LTS \\
% Processor & Intel(R) Xeon(R) W-1270 (3.40GHz, 16 cores) \\
% Ram & 128 GB \\
% GPU & NVIDIA RTX A5000 (24GB) \\
% Environment & Python 3.10.14, PyTorch 2.1.0 \\

\hline
\multicolumn{2}{c}{Knowledge graph embedding settings} \\
\hline

Tool & OpenKE Toolkit \\
No. of epochs & 500 \\
Batch size & 100 \\
Learning rate & $10^{-3}$ \\
Optimizer & Adam \\

\hline
\multicolumn{2}{c}{Level-1 and Level-2 classification settings} \\
\hline

No. of epochs (Level-1 classification) & 50 \\
No. of epochs (Level-2 classification) & 100 \\
Batch size & 16 \\
Learning rate & $10^{-5}$ \\
Weight decay & $10^{-2}$ \\
Exponential decay rates & $\beta_1$ = 0.9, $\beta_2$ = 0.999 \\
Zero-denominator avoidance parameter & $10^{-8}$ \\
Optimizer & AdamW \\
Patience & 5 \\

\hline
\multicolumn{2}{c}{Classifier selector settings} \\
\hline

No. of epochs & 100 \\
Batch size & 16 \\
Learning rate & $10^{-3}$ \\
Weight decay & $10^{-2}$ \\
Exponential decay rates & $\beta_1$ = 0.9, $\beta_2$ = 0.999 \\
Zero-denominator avoidance parameter & $10^{-8}$ \\
Optimizer & AdamW \\
Patience & 5 \\
\hline
\end{tabular}
\label{tab:settings}
\end{adjustbox}
\end{table}
\section{Heatmap for Correct Classification}

\noindent
Table \ref{tab:heatmap_samples} presents 10 selected data samples, and Fig. \ref{tab:heatmap} provides a qualitative evaluation of IMaGINe performance through heatmap encodings for them. These grayscale heatmaps visualize the ground-truth and IMaGINe-predicted genre labels, with white representing positive and black indicating negative genres.

\begin{table*}[!hbt]
\centering
\caption{Data samples for heatmap}
\begin{adjustbox}{width=0.88\textwidth}
% \begin{adjustbox}{angle=90, height=1\textheight}
% \footnotesize
\begin{tabular}{c|ll}%p{0.9\textwidth}}
% \multicolumn{3}{c}{(a) Samples for heatmap analysis}\\
\hline %\hline
% \multicolumn{1}{c}{} & \multicolumn{1}{c}{} & \\[\dimexpr -\normalbaselineskip+1.5pt]

\rowcolor[HTML]{D9D9D9}
\multicolumn{3}{c}{\textcolor{blue}{\emph{(a)}} \textbf{9780060223595: Bread and Jam for Frances; Author: Russell Hoban; Publisher: HarperCollins Publishers}}\\
\hline %\hline
% & \\ [\dimexpr-\normalbaselineskip+1.5pt]

\multirow{5}{*}{\includegraphics[width=0.04\linewidth, height=0.05\linewidth]{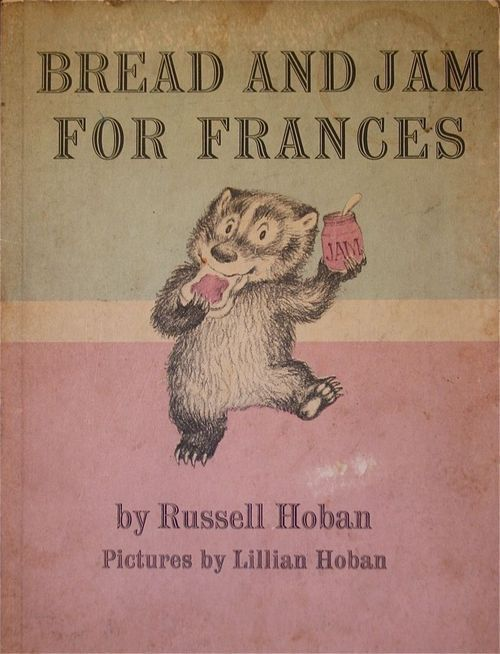}} & \multirow{4}{*}{\textbf{Blurb}:} & The classic funny story about a stubborn little badger with very particular tastes in food. Frances is a fussy eater. In fact, the only thing she likes is bread and jam. She won't  \\
& & touch her squishy soft-boiled egg. She trades away her chicken-salad sandwich at lunch. She turns up her nose at boring veal cutlets. Unless her parents can come up with a \\
& &    plan, Frances just might go on eating bread and jam forever! Join the generations of families that have laughed along as Frances sings "Jam on biscuits, jam on bread,\\
& &   Jam is the thing I like most, Jam is sticky, jam is sweet, Jam is tasty, jam’s a treat—raspberry, strawberry, gooseberry, I’m very FOND…OF…JAM!"\\ \cline{2-3}
% & ${\cal{M}}$ & \{"author":"Russell Hoban","publisher":"HarperCollins Publishers"\}\\ \hline
& \multicolumn{1}{l}{\textbf{Actual Genre}:} & (Fiction, \{Animals \& Wildlife \& Pets, Arts \& Photography, {Childrens\textquoteright} Book, Cookbooks \& Food \& Wine, Family \& Parenting \& Relationships, Literature\})\\ 

\hline \hline

\rowcolor[HTML]{D9D9D9}
\multicolumn{3}{c}{\textcolor{blue}{\emph{(b)}} \textbf{9782723423014: Sailor Moon, tome 14 : Le royaume Elusion; Author: Naoko Takeuchi; Publisher: GLÉNAT}}\\
\hline 

\multirow{3}{*}{\includegraphics[width=0.04\linewidth, height=0.05\linewidth]{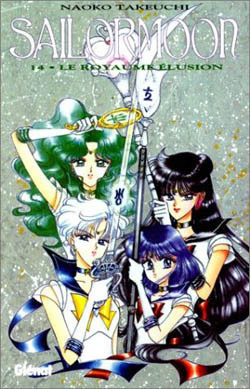}} & \multirow{2}{*}{\textbf{Blurb}:} & A graphic novel offers the continuing adventures of Serena and her friends, who use the power of the moon and the planets, as the superhero Sailor Moon and her comrades, \\
& &  to battle the forces of evil. \\ \cline{2-3}

% & ${\cal{M}}$ & \{"author":"Naoko Takeuchi","publisher":"GLÉNAT"\}\\ \hline
& \multicolumn{1}{l}{\textbf{Actual Genre}:} & (Fiction, \{Comics \& Graphic, Romance, Science Fiction \& Fantasy\})\\

\hline \hline
\rowcolor[HTML]{D9D9D9}
\multicolumn{3}{c}{\textcolor{blue}{\emph{(c)}} \textbf{9780895297273: Prescription for Nutritional Healing: A Practical A-Z Reference to Drug-Free Remedies Using Vitamins, Minerals, Herbs \& Food Supplements;}}\\
\rowcolor[HTML]{D9D9D9}
\multicolumn{3}{c}{ \textbf{
Author: James F. Balch; Publisher: Avery Publishing Group}} \\
\hline 
\multirow{3}{*}{\includegraphics[width=0.04\linewidth, height=0.05\linewidth]{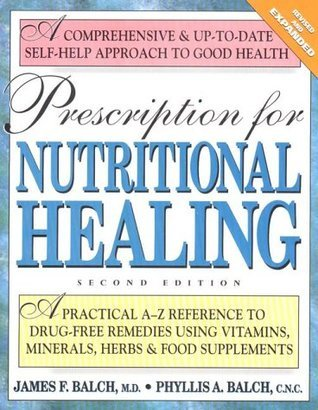}} & \multirow{2}{*}{\textbf{Blurb}:} & An alphabetical encyclopedia of nutritional treatments for a wide range of common ailments explains how to use vitamins, herbs, minerals, and food supplements to promote \\
& &  healing and wellness.\\ \cline{2-3}
% & ${\cal{M}}$ & \{"author":"James F.,Md. Balch","publisher":"Avery Publishing Group"\}\\ \hline
& \multicolumn{1}{l}{\textbf{Actual Genre}:} & (Non-fiction, \{Cookbooks \& Food \& Wine, Health \& Fitness \& Dieting, Medical, Reference \& Language, Self-Help \& Motivation\})\\

\hline \hline
\rowcolor[HTML]{D9D9D9}
\multicolumn{3}{c}{\textcolor{blue}{\emph{(d)}} \textbf{9780060172732: The Dog Who Rescues Cats: The True Story of Ginny; Author: Philip Gonzalez; Publisher: Harpercollins}}\\
\hline 
\multirow{3}{*}{\includegraphics[width=0.04\linewidth, height=0.05\linewidth]{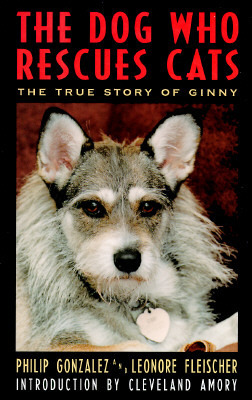}} & \multirow{2}{*}{\textbf{Blurb}:} & The true story of Ginny, an abused dog with an affinity for rescuing cats in trouble, describes Ginny's part in the saving of such handicapped felines as the one-eyed Revlon, \\
& &  deaf Madam, and the paralyzed Topsy. \\ \cline{2-3}

% & ${\cal{M}}$ & \{"author":"Philip Gonzalez","publisher":"Harpercollins"\}\\ \hline
& \multicolumn{1}{l}{\textbf{Actual Genre}:} & (Non-fiction, \{Animals \& Wildlife \& Pets, Biographies \& Memoir\})\\

\hline \hline
\rowcolor[HTML]{D9D9D9}
\multicolumn{3}{c}{\textcolor{blue}{\emph{(e)}} \textbf{9780671668365: MAGIC OF CONFLICT; Author: Thomas Crum; Publisher: Touchstone}}\\
\hline 
\multirow{3}{*}{\includegraphics[width=0.04\linewidth, height=0.05\linewidth]{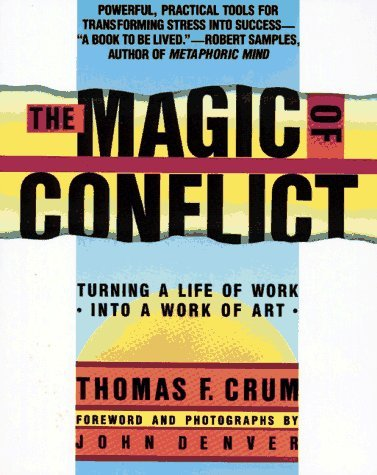}} & \multirow{2}{*}{\textbf{Blurb}:} & Gives techniques for transforming conflict into an opportunity for choice and change and how to grow beyond the striving competitiveness, and pressure of personal and \\
& &  professional life. \\ \cline{2-3}

% & ${\cal{M}}$ & \{"author":"Thomas Crum","publisher":"Touchstone"\}\\
% \hline

& \multicolumn{1}{l}{\textbf{Actual Genre}:} & (Non-fiction, \{Business \& Money, Humanities, Mythology \& Religion \& Spirituality, Self-Help \& Motivation\})\\

\hline \hline
\rowcolor[HTML]{D9D9D9}
\multicolumn{3}{c}{\textcolor{blue}{\emph{(f)}} \textbf{9780963235930: Beyond Backpacking: Ray Jardines Guide to Lightweight Hiking; Author: Ray Jardine; Publisher: Adventurelore Press}}\\
\hline

\multirow{3}{*}{\includegraphics[width=0.04\linewidth, height=0.05\linewidth]{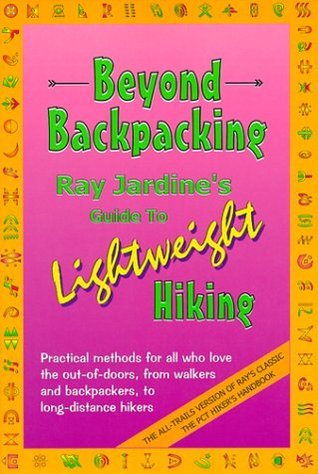}} & \multirow{2}{*}{\textbf{Blurb}:} & Beyond Backpacking has 517 pages of "practical methods for all who love the out-of-doors". Chapters include Equipment, Hiking Considerations, Obstacles, Longer  \\
& & Journeys and Back to Basics.  \\
\cline{2-3}
% & ${\cal{M}}$ & \{"author":"Ray Jardine","publisher":"Adventurelore Press"\}\\
% \hline
& \multicolumn{1}{l}{\textbf{Actual Genre}:} & (Non-fiction, \{Environment \& Plant, Mystery \& Thriller \& Suspense \& Horror, Reference \& Language, Sports \& Outdoors, Travel\})\\

\hline \hline
\rowcolor[HTML]{D9D9D9}
\multicolumn{3}{c}{\textcolor{blue}{\emph{(g)}} \textbf{9780380773527: Dreaming of You; Author: Lisa Kleypas; Publisher: Avon}}\\
\hline 
\multirow{7}{*}{\includegraphics[width=0.04\linewidth, height=0.05\linewidth]{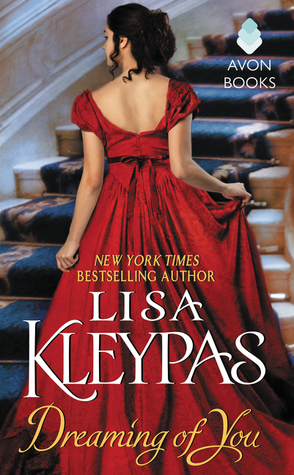}} & \multirow{6}{*}{\textbf{Blurb}:} & She stood at danger's threshold—then love beckoned her in.A prim, well-bred gentlewoman, Sara Fielding is a writer who puts pen to paper to create dreams. But now\\
& &   curiosity is luring her from the shelter of her country cottage into the dangerous world of Derek Craven—handsome, tough, and tenacious—and the most exciting man Sara \\
& &  has ever met. Derek rose from poverty to become the wealthy lord of London’s most exclusive gambling house. And now duty demands that he allow Sara Fielding to \\
& &  enter his perilous realm of ever-shifting fortunes—with her impeccable manners and her infuriating innocence. But there is a hidden strength and sensuality to the lady that\\
& &    captivates him beyond  his better judgment.And in this world, where danger lurks behind every shadow, even a proper “mouse” can be transformed into a breathtaking \\
& &  enchantress—and a cynical gambler can be shaken to his core by the power of passion and the promise of love.\\
\cline{2-3}
& \multicolumn{1}{l}{\textbf{Actual Genre}:} & (Fiction, \{Fashion \& Lifestyle, History, Romance\})\\

\hline \hline

\rowcolor[HTML]{D9D9D9}
\multicolumn{3}{c}{\textbf{{\emph{(h).}} 9780679602613: The Soul of a New Machine; Author: TRACY KIDDER; Publisher: Modern Library}}\\
\hline \hline

\multirow{13}{*}{\includegraphics[width=0.04\linewidth, height=0.05\linewidth]{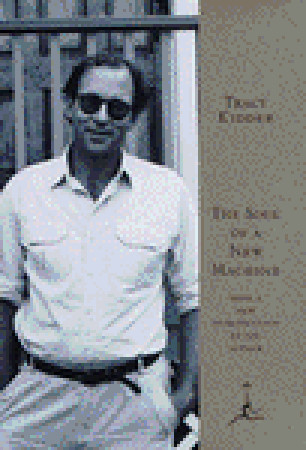}} & \multirow{12}{*}{\textbf{Blurb}:} & Winner of the Pulitzer Prize and the American Book Award, The Soul of a New Machine was a bestseller on its first publication in 1981. With the touch of an expert thriller\\
& &    writer, Tracy Kidder recounts the feverish efforts of a team of Data General researchers to create a new 32-bit superminicomputer. A compelling account of individual sacrifice \\
& &    and human ingenuity, The Soul of a New Machine endures as the classic chronicle of the computer age and the masterminds behind its technological advances. "A superb \\
& &   book," said Robert Pirsig, author of Zen and the Art of Motorcycle Maintenance. "All the incredible complexity and chaos and exploitation and loneliness and strange,\\
& &     half-mad beauty of this field are honestly and correctly drawn." The Washington Post Book World said, "Kidder has created compelling entertainment.  He offers a fast,\\
& &    painless, enjoyable means to an initial understanding of computers, allowing us to understand the complexity of machines  we could only marvel at before, and to appreciate\\

& &   the skills of the people who create them."The Modern Library has played a significant role in American cultural  life for the better part of a century. The series was founded\\
& &   in 1917 by the publishers Boni and Liveright and eight years later acquired by Bennett Cerf and Donald Klopfer. It provided the foundation for their next publishing venture,\\

& &   Random House. The Modern Library has been a staple of the American book trade, providing readers with affordable hardbound editions of important works of literature and \\
& & thought. For the Modern Library's seventy-fifth anniversary, Random House redesigned the series, restoring as its emblem the running torch-bearer created by Lucian Bernhard \\

&  & in 1925 and refurbishing jackets, bindings, and type, as well as inaugurating a new program of selecting titles. The Modern Library continues to provide the world's best \\

& & books, at the best prices. Tracy Kidder has written a new Introduction to this Modern Library edition.\\ \cline{2-3}

 % & ${\cal{M}} $ & \{"author":"TRACY KIDDER","publisher":"Modern Library"\}\\ \hline
& \multicolumn{1}{c}{\textbf{Actual Genre}:} & (Non-fiction, {Business \& Money, Computers \& Technology, History, Science \& Math })\\

\hline \hline
\rowcolor[HTML]{D9D9D9}
\multicolumn{3}{c}{\textcolor{blue}{\emph{(i)}} \textbf{9780803716988: Library Lil; Author: Suzanne Williams; Publisher: Dial Books}}\\
\hline 

\multirow{3}{*}{\includegraphics[width=0.04\linewidth, height=0.05\linewidth]{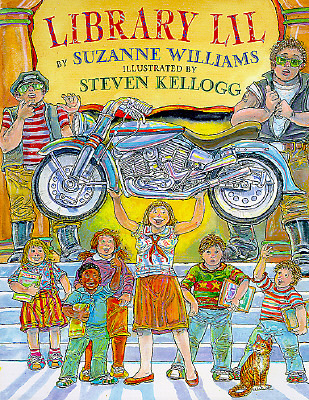}} & \multirow{2}{*}{\textbf{Blurb}:} & A formidable librarian makes readers not only out of the once resistant residents of her small town, but out of a tough-talking, television-watching motorcycle gang as well. \\
& & \\
\cline{2-3}
% & ${\cal{M}}$ & \{"author":"Suzanne Williams","publisher":"Dial Books"\}\\

% \hline
& \multicolumn{1}{l}{\textbf{Actual Genre}:} & (Fiction, \{Arts \& Photography, {Childrens\textquoteright} Book, Humor \& Entertainment, Meta Text, Sci-Fi\})\\

\hline \hline
\rowcolor[HTML]{D9D9D9}
\multicolumn{3}{c}{\textcolor{blue}{\emph{(j)}} \textbf{9780130255792: Understanding Movies; Author: Louis D. Giannetti; Publisher: Prentice Hall}}\\
\hline 
\multirow{5}{*}{\includegraphics[width=0.04\linewidth, height=0.05\linewidth]{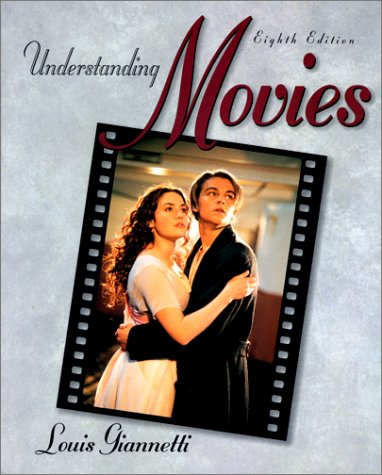}} & \multirow{4}{*}{\textbf{Blurb}:} & Designed to help movie watchers analyze films with precision and technical sophistication, this book focuses on formalism how the forms of the film (e.g., camera work, \\
& &  editing, photography, etc.) create meaning. It sheds light on how television and movies communicate, and the complex network of language systems they use. Chapter topics\\

& &    cover recent developments from all aspects of cinema, contemporary films, personalities in the field, photography, movement, editing, sound, acting, drama, story writing, and   \\ 

& & theory. For movie critics and fans alike.\\
\cline{2-3}

& \multicolumn{1}{l}{\textbf{Actual Genre}:} & (Non-fiction, \{Arts \& Photography, Press \& Media, Reference \& Language, Teen \& Young Adult\}) \\
\hline

\end{tabular}
\end{adjustbox}

\label{tab:heatmap_samples}

\end{table*}
\begin{figure*}[!hbt]
\centering

% \begin{adjustbox}{angle=90, height=1\textheight}
\begin{adjustbox}{width=0.88\textwidth} 
\begin{tabular}{cc|c|c|c|c|c|c|c|c|c|c|c|c|c|c|c|c|c|c|c|c|c|c|c|c|c|c|c|c|c|c|c|c}
\hline

\multicolumn{1}{c}{} & \multicolumn{1}{c|}{} & 
\multicolumn{2}{c|}{Level-1} & \multicolumn{30}{c}{Level-2 Classification} \\
\cline{3-34} 
%%%%%% Actual
\multicolumn{1}{c}{} & \multicolumn{1}{c|}{Class ID}  & NF & F & 1 & 2& 3 & 4& 5& 6 & 7 & 8 & 9 & 10 & 11 & 12 & 13 & 14 & 15 & 16 & 17 & 18 & 19 & 20 & 21 & 22 & 23 & 24 & 25 & 26 & 27 & 28 & 29 & 30 \\ 
% \cline{2-34} 
\hline \hline 

\multirow{10}{*}{\textbf{\rotatebox{90}{\underline{Ground-truth}}}} & \textcolor{blue}{\emph{(a)}} & \cellcolor[gray]{0} & \cellcolor[gray]{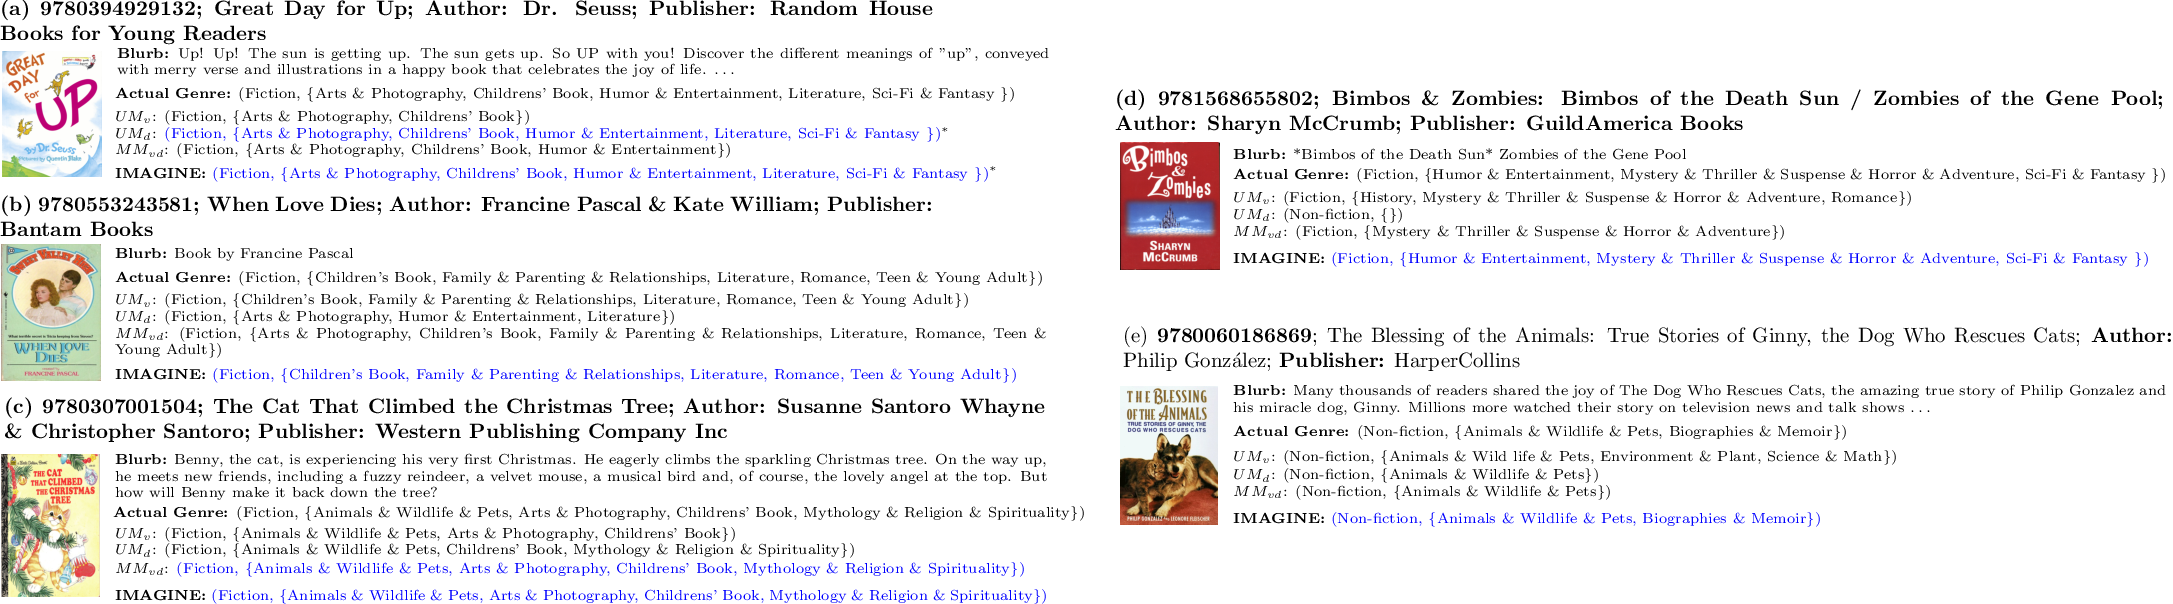} & \cellcolor[gray]{1.00000} & \cellcolor[gray]{1.00000} & \cellcolor[gray]{0.00000} & \cellcolor[gray]{1.00000} & \cellcolor[gray]{0.00000} & \cellcolor[gray]{0.00000} & \cellcolor[gray]{1.00000} & \cellcolor[gray]{0.00000} & \cellcolor[gray]{0.00000} & \cellcolor[gray]{1.00000} & \cellcolor[gray]{0.00000} & \cellcolor[gray]{0.00000} & \cellcolor[gray]{0.00000} & \cellcolor[gray]{0.00000} & \cellcolor[gray]{0.00000} & \cellcolor[gray]{1.00000} & \cellcolor[gray]{0.00000} & \cellcolor[gray]{0.00000} & \cellcolor[gray]{0.00000} & \cellcolor[gray]{0.00000} & \cellcolor[gray]{0.00000} & \cellcolor[gray]{0.00000} & \cellcolor[gray]{0.00000} & \cellcolor[gray]{0.00000} & \cellcolor[gray]{0.00000} & \cellcolor[gray]{0.00000} & \cellcolor[gray]{0.00000} & \cellcolor[gray]{0.00000} & \cellcolor[gray]{0.00000} & \cellcolor[gray]{0.00000} \\ \cline{2-34} 

 & \textcolor{blue}{\emph{(b)}} & \cellcolor[gray]{0} & \cellcolor[gray]{1} & \cellcolor[gray]{0.00000} & \cellcolor[gray]{0.00000} & \cellcolor[gray]{0.00000} & \cellcolor[gray]{0.00000} & \cellcolor[gray]{1.00000} & \cellcolor[gray]{0.00000} & \cellcolor[gray]{0.00000} & \cellcolor[gray]{0.00000} & \cellcolor[gray]{0.00000} & \cellcolor[gray]{0.00000} & \cellcolor[gray]{0.00000} & \cellcolor[gray]{0.00000} & \cellcolor[gray]{0.00000} & \cellcolor[gray]{0.00000} & \cellcolor[gray]{0.00000} & \cellcolor[gray]{0.00000} & \cellcolor[gray]{0.00000} & \cellcolor[gray]{0.00000} & \cellcolor[gray]{0.00000} & \cellcolor[gray]{0.00000} & \cellcolor[gray]{0.00000} & \cellcolor[gray]{0.00000} & \cellcolor[gray]{1.00000} & \cellcolor[gray]{0.00000} & \cellcolor[gray]{0.00000} & \cellcolor[gray]{0.00000} & \cellcolor[gray]{0.00000} & \cellcolor[gray]{0.00000} & \cellcolor[gray]{1.00000} & \cellcolor[gray]{0.00000} \\ \cline{2-34} 
 
 & \textcolor{blue}{\emph{(c)}} & \cellcolor[gray]{1} & \cellcolor[gray]{0} & \cellcolor[gray]{0.00000} & \cellcolor[gray]{0.00000} & \cellcolor[gray]{0.00000} & \cellcolor[gray]{0.00000} & \cellcolor[gray]{0.00000} & \cellcolor[gray]{0.00000} & \cellcolor[gray]{1.00000} & \cellcolor[gray]{0.00000} & \cellcolor[gray]{0.00000} & \cellcolor[gray]{0.00000} & \cellcolor[gray]{0.00000} & \cellcolor[gray]{1.00000} & \cellcolor[gray]{0.00000} & \cellcolor[gray]{0.00000} & \cellcolor[gray]{0.00000} & \cellcolor[gray]{0.00000} & \cellcolor[gray]{0.00000} & \cellcolor[gray]{1.00000} & \cellcolor[gray]{0.00000} & \cellcolor[gray]{0.00000} & \cellcolor[gray]{0.00000} & \cellcolor[gray]{1.00000} & \cellcolor[gray]{0.00000} & \cellcolor[gray]{0.00000} & \cellcolor[gray]{1.00000} & \cellcolor[gray]{0.00000} & \cellcolor[gray]{0.00000} & \cellcolor[gray]{0.00000} & \cellcolor[gray]{0.00000} & \cellcolor[gray]{0.00000} \\ \cline{2-34} 
 
 & \textcolor{blue}{\emph{(d)}} & \cellcolor[gray]{1} & \cellcolor[gray]{0} & \cellcolor[gray]{1.00000} & \cellcolor[gray]{0.00000} & \cellcolor[gray]{0.00000} & \cellcolor[gray]{0.00000} & \cellcolor[gray]{0.00000} & \cellcolor[gray]{0.00000} & \cellcolor[gray]{0.00000} & \cellcolor[gray]{0.00000} & \cellcolor[gray]{0.00000} & \cellcolor[gray]{0.00000} & \cellcolor[gray]{0.00000} & \cellcolor[gray]{0.00000} & \cellcolor[gray]{0.00000} & \cellcolor[gray]{0.00000} & \cellcolor[gray]{0.00000} & \cellcolor[gray]{0.00000} & \cellcolor[gray]{0.00000} & \cellcolor[gray]{0.00000} & \cellcolor[gray]{0.00000} & \cellcolor[gray]{0.00000} & \cellcolor[gray]{0.00000} & \cellcolor[gray]{0.00000} & \cellcolor[gray]{0.00000} & \cellcolor[gray]{0.00000} & \cellcolor[gray]{0.00000} & \cellcolor[gray]{0.00000} & \cellcolor[gray]{0.00000} & \cellcolor[gray]{0.00000} & \cellcolor[gray]{0.00000} & \cellcolor[gray]{1.00000} \\ \cline{2-34} 
 
 & \textcolor{blue}{\emph{(e)}} & \cellcolor[gray]{1} & \cellcolor[gray]{0} & \cellcolor[gray]{0.00000} & \cellcolor[gray]{0.00000} & \cellcolor[gray]{1.00000} & \cellcolor[gray]{0.00000} & \cellcolor[gray]{0.00000} & \cellcolor[gray]{0.00000} & \cellcolor[gray]{0.00000} & \cellcolor[gray]{0.00000} & \cellcolor[gray]{0.00000} & \cellcolor[gray]{0.00000} & \cellcolor[gray]{0.00000} & \cellcolor[gray]{0.00000} & \cellcolor[gray]{0.00000} & \cellcolor[gray]{1.00000} & \cellcolor[gray]{0.00000} & \cellcolor[gray]{0.00000} & \cellcolor[gray]{0.00000} & \cellcolor[gray]{0.00000} & \cellcolor[gray]{0.00000} & \cellcolor[gray]{1.00000} & \cellcolor[gray]{0.00000} & \cellcolor[gray]{0.00000} & \cellcolor[gray]{0.00000} & \cellcolor[gray]{0.00000} & \cellcolor[gray]{1.00000} & \cellcolor[gray]{0.00000} & \cellcolor[gray]{0.00000} & \cellcolor[gray]{0.00000} & \cellcolor[gray]{0.00000} & \cellcolor[gray]{0.00000} \\ \cline{2-34}
 
 & \textcolor{blue}{\emph{(f)}} & \cellcolor[gray]{1} & \cellcolor[gray]{0} & \cellcolor[gray]{0.00000} & \cellcolor[gray]{0.00000} & \cellcolor[gray]{0.00000} & \cellcolor[gray]{0.00000} & \cellcolor[gray]{0.00000} & \cellcolor[gray]{0.00000} & \cellcolor[gray]{0.00000} & \cellcolor[gray]{0.00000} & \cellcolor[gray]{1.00000} & \cellcolor[gray]{0.00000} & \cellcolor[gray]{0.00000} & \cellcolor[gray]{0.00000} & \cellcolor[gray]{0.00000} & \cellcolor[gray]{0.00000} & \cellcolor[gray]{0.00000} & \cellcolor[gray]{0.00000} & \cellcolor[gray]{1.00000} & \cellcolor[gray]{0.00000} & \cellcolor[gray]{0.00000} & \cellcolor[gray]{0.00000} & \cellcolor[gray]{0.00000} & \cellcolor[gray]{1.00000} & \cellcolor[gray]{0.00000} & \cellcolor[gray]{0.00000} & \cellcolor[gray]{0.00000} & \cellcolor[gray]{1.00000} & \cellcolor[gray]{0.00000} & \cellcolor[gray]{1.00000} & \cellcolor[gray]{0.00000} & \cellcolor[gray]{0.00000} \\ \cline{2-34} 
 
 & \textcolor{blue}{\emph{(g)}} & \cellcolor[gray]{0} & \cellcolor[gray]{1} & \cellcolor[gray]{0.00000} & \cellcolor[gray]{0.00000} & \cellcolor[gray]{0.00000} & \cellcolor[gray]{0.00000} & \cellcolor[gray]{0.00000} & \cellcolor[gray]{0.00000} & \cellcolor[gray]{0.00000} & \cellcolor[gray]{0.00000} & \cellcolor[gray]{0.00000} & \cellcolor[gray]{0.00000} & \cellcolor[gray]{1.00000} & \cellcolor[gray]{0.00000} & \cellcolor[gray]{1.00000} & \cellcolor[gray]{0.00000} & \cellcolor[gray]{0.00000} & \cellcolor[gray]{0.00000} & \cellcolor[gray]{0.00000} & \cellcolor[gray]{0.00000} & \cellcolor[gray]{0.00000} & \cellcolor[gray]{0.00000} & \cellcolor[gray]{0.00000} & \cellcolor[gray]{0.00000} & \cellcolor[gray]{1.00000} & \cellcolor[gray]{0.00000} & \cellcolor[gray]{0.00000} & \cellcolor[gray]{0.00000} & \cellcolor[gray]{0.00000} & \cellcolor[gray]{0.00000} & \cellcolor[gray]{0.00000} & \cellcolor[gray]{0.00000} \\ \cline{2-34} 
 
 &\textcolor{blue}{\emph{(h)}} & \cellcolor[gray]{1} & \cellcolor[gray]{0} & \cellcolor[gray]{0.00000} & \cellcolor[gray]{0.00000} & \cellcolor[gray]{1.00000} & \cellcolor[gray]{0.00000} & \cellcolor[gray]{0.00000} & \cellcolor[gray]{1.00000} & \cellcolor[gray]{0.00000} & \cellcolor[gray]{0.00000} & \cellcolor[gray]{0.00000} & \cellcolor[gray]{0.00000} & \cellcolor[gray]{0.00000} & \cellcolor[gray]{0.00000} & \cellcolor[gray]{1.00000} & \cellcolor[gray]{0.00000} & \cellcolor[gray]{0.00000} & \cellcolor[gray]{0.00000} & \cellcolor[gray]{0.00000} & \cellcolor[gray]{0.00000} & \cellcolor[gray]{0.00000} & \cellcolor[gray]{0.00000} & \cellcolor[gray]{0.00000} & \cellcolor[gray]{0.00000} & \cellcolor[gray]{0.00000} & \cellcolor[gray]{1.00000} & \cellcolor[gray]{0.00000} & \cellcolor[gray]{0.00000} & \cellcolor[gray]{0.00000} & \cellcolor[gray]{0.00000} & \cellcolor[gray]{0.00000} & \cellcolor[gray]{0.00000} \\ \cline{2-34} 
 & \textcolor{blue}{\emph{(i)}} & \cellcolor[gray]{0} & \cellcolor[gray]{1} & \cellcolor[gray]{0.00000} & \cellcolor[gray]{1.00000} & \cellcolor[gray]{0.00000} & \cellcolor[gray]{1.00000} & \cellcolor[gray]{0.00000} & \cellcolor[gray]{0.00000} & \cellcolor[gray]{0.00000} & \cellcolor[gray]{0.00000} & \cellcolor[gray]{0.00000} & \cellcolor[gray]{0.00000} & \cellcolor[gray]{0.00000} & \cellcolor[gray]{0.00000} & \cellcolor[gray]{0.00000} & \cellcolor[gray]{0.00000} & \cellcolor[gray]{1.00000} & \cellcolor[gray]{0.00000} & \cellcolor[gray]{0.00000} & \cellcolor[gray]{0.00000} & \cellcolor[gray]{1.00000} & \cellcolor[gray]{0.00000} & \cellcolor[gray]{0.00000} & \cellcolor[gray]{0.00000} & \cellcolor[gray]{0.00000} & \cellcolor[gray]{0.00000} & \cellcolor[gray]{0.00000} & \cellcolor[gray]{0.00000} & \cellcolor[gray]{0.00000} & \cellcolor[gray]{0.00000} & \cellcolor[gray]{1.00000} & \cellcolor[gray]{0.00000} \\ \cline{2-34} 
 & \textcolor{blue}{\emph{(j)}} & \cellcolor[gray]{1} & \cellcolor[gray]{0} & \cellcolor[gray]{0.00000} & \cellcolor[gray]{1.00000} & \cellcolor[gray]{0.00000} & \cellcolor[gray]{0.00000} & \cellcolor[gray]{0.00000} & \cellcolor[gray]{0.00000} & \cellcolor[gray]{0.00000} & \cellcolor[gray]{0.00000} & \cellcolor[gray]{0.00000} & \cellcolor[gray]{0.00000} & \cellcolor[gray]{0.00000} & \cellcolor[gray]{0.00000} & \cellcolor[gray]{0.00000} & \cellcolor[gray]{0.00000} & \cellcolor[gray]{0.00000} & \cellcolor[gray]{0.00000} & \cellcolor[gray]{0.00000} & \cellcolor[gray]{0.00000} & \cellcolor[gray]{0.00000} & \cellcolor[gray]{0.00000} & \cellcolor[gray]{1.00000} & \cellcolor[gray]{1.00000} & \cellcolor[gray]{0.00000} & \cellcolor[gray]{0.00000} & \cellcolor[gray]{0.00000} & \cellcolor[gray]{0.00000} & \cellcolor[gray]{1.00000} & \cellcolor[gray]{0.00000} & \cellcolor[gray]{0.00000} & \cellcolor[gray]{0.00000} \\ 
 \hline \hline

%%%%%%%% Predicted

\multirow{10}{*}{\textbf{\rotatebox{90}{\underline{Predicted score}}}} & \textcolor{blue}{\emph{(a)}} & \cellcolor[gray]{0.00044} & \cellcolor[gray]{0.99956} & \cellcolor[gray]{0.99476} & \cellcolor[gray]{0.99909} & \cellcolor[gray]{0.00001} & \cellcolor[gray]{0.99997} & \cellcolor[gray]{0.00083} & \cellcolor[gray]{0.00002} & \cellcolor[gray]{0.94047} & \cellcolor[gray]{0.00000} & \cellcolor[gray]{0.00563} & \cellcolor[gray]{0.99830} & \cellcolor[gray]{0.00000} & \cellcolor[gray]{0.00056} & \cellcolor[gray]{0.00066} & \cellcolor[gray]{0.00122} & \cellcolor[gray]{0.03674} & \cellcolor[gray]{0.99246} & \cellcolor[gray]{0.00000} & \cellcolor[gray]{0.00550} & \cellcolor[gray]{0.00044} & \cellcolor[gray]{0.00000} & \cellcolor[gray]{0.00014} & \cellcolor[gray]{0.00006} & \cellcolor[gray]{0.00023} & \cellcolor[gray]{0.00008} & \cellcolor[gray]{0.00006} & \cellcolor[gray]{0.00002} & \cellcolor[gray]{0.00533} & \cellcolor[gray]{0.00015} & \cellcolor[gray]{0.03099} & \cellcolor[gray]{0.00000} \\ \cline{2-34} 

 & \textcolor{blue}{\emph{(b)}} & \cellcolor[gray]{0.00016} & \cellcolor[gray]{0.99984} & \cellcolor[gray]{0.00133} & \cellcolor[gray]{0.01118} & \cellcolor[gray]{0.00027} & \cellcolor[gray]{0.00066} & \cellcolor[gray]{0.99569} & \cellcolor[gray]{0.04551} & \cellcolor[gray]{0.00032} & \cellcolor[gray]{0.00000} & \cellcolor[gray]{0.00000} & \cellcolor[gray]{0.00001} & \cellcolor[gray]{0.00002} & \cellcolor[gray]{0.00000} & \cellcolor[gray]{0.03169} & \cellcolor[gray]{0.00016} & \cellcolor[gray]{0.02745} & \cellcolor[gray]{0.00027} & \cellcolor[gray]{0.00545} & \cellcolor[gray]{0.00022} & \cellcolor[gray]{0.00001} & \cellcolor[gray]{0.00010} & \cellcolor[gray]{0.00255} & \cellcolor[gray]{0.00001} & \cellcolor[gray]{0.99160} & \cellcolor[gray]{0.00353} & \cellcolor[gray]{0.00000} & \cellcolor[gray]{0.00004} & \cellcolor[gray]{0.10041} & \cellcolor[gray]{0.00222} & \cellcolor[gray]{0.97165} & \cellcolor[gray]{0.00000} \\ \cline{2-34} 
 
 & \textcolor{blue}{\emph{(c)}} & \cellcolor[gray]{0.99994} & \cellcolor[gray]{0.00006} & \cellcolor[gray]{0.00007} & \cellcolor[gray]{0.00004} & \cellcolor[gray]{0.00007} & \cellcolor[gray]{0.03481} & \cellcolor[gray]{0.00017} & \cellcolor[gray]{0.00009} & \cellcolor[gray]{0.97895} & \cellcolor[gray]{0.00046} & \cellcolor[gray]{0.00542} & \cellcolor[gray]{0.01889} & \cellcolor[gray]{0.00044} & \cellcolor[gray]{0.99680} & \cellcolor[gray]{0.00002} & \cellcolor[gray]{0.00266} & \cellcolor[gray]{0.00002} & \cellcolor[gray]{0.00476} & \cellcolor[gray]{0.01359} & \cellcolor[gray]{0.82687} & \cellcolor[gray]{0.00702} & \cellcolor[gray]{0.00038} & \cellcolor[gray]{0.00001} & \cellcolor[gray]{0.99791} & \cellcolor[gray]{0.00092} & \cellcolor[gray]{0.00011} & \cellcolor[gray]{0.99844} & \cellcolor[gray]{0.00979} & \cellcolor[gray]{0.00001} & \cellcolor[gray]{0.00032} & \cellcolor[gray]{0.00000} & \cellcolor[gray]{0.00001} \\ \cline{2-34} 
 
 & \textcolor{blue}{\emph{(d)}} & \cellcolor[gray]{0.99635} & \cellcolor[gray]{0.00365} & \cellcolor[gray]{0.99472} & \cellcolor[gray]{0.00016} & \cellcolor[gray]{0.00009} & \cellcolor[gray]{0.00001} & \cellcolor[gray]{0.00002} & \cellcolor[gray]{0.00004} & \cellcolor[gray]{0.00303} & \cellcolor[gray]{0.00000} & \cellcolor[gray]{0.00361} & \cellcolor[gray]{0.00086} & \cellcolor[gray]{0.00008} & \cellcolor[gray]{0.00000} & \cellcolor[gray]{0.00635} & \cellcolor[gray]{0.00004} & \cellcolor[gray]{0.00166} & \cellcolor[gray]{0.00040} & \cellcolor[gray]{0.00005} & \cellcolor[gray]{0.00005} & \cellcolor[gray]{0.01653} & \cellcolor[gray]{0.00047} & \cellcolor[gray]{0.00008} & \cellcolor[gray]{0.00086} & \cellcolor[gray]{0.00274} & \cellcolor[gray]{0.00353} & \cellcolor[gray]{0.00000} & \cellcolor[gray]{0.00002} & \cellcolor[gray]{0.00000} & \cellcolor[gray]{0.00001} & \cellcolor[gray]{0.00000} & \cellcolor[gray]{0.99131} \\ \cline{2-34} 
 
 & \textcolor{blue}{\emph{(e)}} & \cellcolor[gray]{0.99991} & \cellcolor[gray]{0.00009} & \cellcolor[gray]{0.00002} & \cellcolor[gray]{0.00099} & \cellcolor[gray]{0.99969} & \cellcolor[gray]{0.00000} & \cellcolor[gray]{0.00419} & \cellcolor[gray]{0.01303} & \cellcolor[gray]{0.00000} & \cellcolor[gray]{0.00003} & \cellcolor[gray]{0.00002} & \cellcolor[gray]{0.04246} & \cellcolor[gray]{0.00810} & \cellcolor[gray]{0.00004} & \cellcolor[gray]{0.00268} & \cellcolor[gray]{0.98886} & \cellcolor[gray]{0.00000} & \cellcolor[gray]{0.00006} & \cellcolor[gray]{0.00004} & \cellcolor[gray]{0.00378} & \cellcolor[gray]{0.00823} & \cellcolor[gray]{0.90046} & \cellcolor[gray]{0.00000} & \cellcolor[gray]{0.00545} & \cellcolor[gray]{0.00357} & \cellcolor[gray]{0.00013} & \cellcolor[gray]{0.99689} & \cellcolor[gray]{0.00008} & \cellcolor[gray]{0.00005} & \cellcolor[gray]{0.00000} & \cellcolor[gray]{0.00000} & \cellcolor[gray]{0.00358} \\ \cline{2-34} 
 
 & \textcolor{blue}{\emph{(f)}} & \cellcolor[gray]{0.99993} & \cellcolor[gray]{0.00007} & \cellcolor[gray]{0.00021} & \cellcolor[gray]{0.00002} & \cellcolor[gray]{0.00009} & \cellcolor[gray]{0.00027} & \cellcolor[gray]{0.00241} & \cellcolor[gray]{0.00001} & \cellcolor[gray]{0.02858} & \cellcolor[gray]{0.01158} & \cellcolor[gray]{0.93981} & \cellcolor[gray]{0.00048} & \cellcolor[gray]{0.00162} & \cellcolor[gray]{0.03215} & \cellcolor[gray]{0.00400} & \cellcolor[gray]{0.00079} & \cellcolor[gray]{0.00082} & \cellcolor[gray]{0.00392} & \cellcolor[gray]{0.91136} & \cellcolor[gray]{0.00001} & \cellcolor[gray]{0.00181} & \cellcolor[gray]{0.00202} & \cellcolor[gray]{0.00007} & \cellcolor[gray]{0.99415} & \cellcolor[gray]{0.00998} & \cellcolor[gray]{0.00002} & \cellcolor[gray]{0.00505} & \cellcolor[gray]{0.99881} & \cellcolor[gray]{0.01750} & \cellcolor[gray]{0.97146} & \cellcolor[gray]{0.00000} & \cellcolor[gray]{0.11416} \\ \cline{2-34} 
 
 & \textcolor{blue}{\emph{(g)}} & \cellcolor[gray]{0.00008} & \cellcolor[gray]{0.99992} & \cellcolor[gray]{0.00213} & \cellcolor[gray]{0.04993} & \cellcolor[gray]{0.00258} & \cellcolor[gray]{0.00845} & \cellcolor[gray]{0.00705} & \cellcolor[gray]{0.00096} & \cellcolor[gray]{0.00517} & \cellcolor[gray]{0.00225} & \cellcolor[gray]{0.00287} & \cellcolor[gray]{0.42612} & \cellcolor[gray]{0.71277} & \cellcolor[gray]{0.01147} & \cellcolor[gray]{0.92822} & \cellcolor[gray]{0.00258} & \cellcolor[gray]{0.17138} & \cellcolor[gray]{0.07084} & \cellcolor[gray]{0.00624} & \cellcolor[gray]{0.04806} & \cellcolor[gray]{0.03481} & \cellcolor[gray]{0.04279} & \cellcolor[gray]{0.01641} & \cellcolor[gray]{0.00774} & \cellcolor[gray]{0.85877} & \cellcolor[gray]{0.11464} & \cellcolor[gray]{0.00673} & \cellcolor[gray]{0.00154} & \cellcolor[gray]{0.05980} & \cellcolor[gray]{0.00338} & \cellcolor[gray]{0.01469} & \cellcolor[gray]{0.00000} \\ \cline{2-34} 
 & \textcolor{blue}{\emph{(h)}} & \cellcolor[gray]{0.99975} & \cellcolor[gray]{0.00025} & \cellcolor[gray]{0.00133} & \cellcolor[gray]{0.00295} & \cellcolor[gray]{0.92140} & \cellcolor[gray]{0.01267} & \cellcolor[gray]{0.01531} & \cellcolor[gray]{0.87444} & \cellcolor[gray]{0.04635} & \cellcolor[gray]{0.00045} & \cellcolor[gray]{0.00879} & \cellcolor[gray]{0.00264} & \cellcolor[gray]{0.01290} & \cellcolor[gray]{0.00145} & \cellcolor[gray]{0.98127} & \cellcolor[gray]{0.33684} & \cellcolor[gray]{0.00039} & \cellcolor[gray]{0.05179} & \cellcolor[gray]{0.00029} & \cellcolor[gray]{0.05201} & \cellcolor[gray]{0.01190} & \cellcolor[gray]{0.00225} & \cellcolor[gray]{0.06651} & \cellcolor[gray]{0.00788} & \cellcolor[gray]{0.00283} & \cellcolor[gray]{0.82674} & \cellcolor[gray]{0.00126} & \cellcolor[gray]{0.00023} & \cellcolor[gray]{0.24525} & \cellcolor[gray]{0.03039} & \cellcolor[gray]{0.00000} & \cellcolor[gray]{0.18526} \\ \cline{2-34} 
 & \textcolor{blue}{\emph{(i)}} & \cellcolor[gray]{0.00315} & \cellcolor[gray]{0.99685} & \cellcolor[gray]{0.00671} & \cellcolor[gray]{0.80333} & \cellcolor[gray]{0.00000} & \cellcolor[gray]{0.85072} & \cellcolor[gray]{0.00034} & \cellcolor[gray]{0.00014} & \cellcolor[gray]{0.00026} & \cellcolor[gray]{0.00000} & \cellcolor[gray]{0.00001} & \cellcolor[gray]{0.00009} & \cellcolor[gray]{0.00004} & \cellcolor[gray]{0.00500} & \cellcolor[gray]{0.00000} & \cellcolor[gray]{0.00001} & \cellcolor[gray]{0.99992} & \cellcolor[gray]{0.00002} & \cellcolor[gray]{0.03822} & \cellcolor[gray]{0.00001} & \cellcolor[gray]{0.99222} & \cellcolor[gray]{0.00018} & \cellcolor[gray]{0.00008} & \cellcolor[gray]{0.00030} & \cellcolor[gray]{0.00001} & \cellcolor[gray]{0.00000} & \cellcolor[gray]{0.00000} & \cellcolor[gray]{0.01542} & \cellcolor[gray]{0.04668} & \cellcolor[gray]{0.00000} & \cellcolor[gray]{0.99957} & \cellcolor[gray]{0.00000} \\ \cline{2-34} 
 & \textcolor{blue}{\emph{(j)}} & \cellcolor[gray]{0.99802} & \cellcolor[gray]{0.00198} & \cellcolor[gray]{0.01750} & \cellcolor[gray]{0.97278} & \cellcolor[gray]{0.05179} & \cellcolor[gray]{0.17395} & \cellcolor[gray]{0.00997} & \cellcolor[gray]{0.05670} & \cellcolor[gray]{0.00747} & \cellcolor[gray]{0.13790} & \cellcolor[gray]{0.00693} & \cellcolor[gray]{0.00516} & \cellcolor[gray]{0.07648} & \cellcolor[gray]{0.00456} & \cellcolor[gray]{0.07431} & \cellcolor[gray]{0.08559} & \cellcolor[gray]{0.14760} & \cellcolor[gray]{0.01880} & \cellcolor[gray]{0.00740} & \cellcolor[gray]{0.01624} & \cellcolor[gray]{0.01769} & \cellcolor[gray]{0.00190} & \cellcolor[gray]{0.66830} & \cellcolor[gray]{0.96815} & \cellcolor[gray]{0.07242} & \cellcolor[gray]{0.15810} & \cellcolor[gray]{0.13284} & \cellcolor[gray]{0.00079} & \cellcolor[gray]{0.68137} & \cellcolor[gray]{0.00128} & \cellcolor[gray]{0.00000} & \cellcolor[gray]{0.00036} \\ 
 \hline

 \multicolumn{34}{r}{L-1: Level-1 classification, NF: \textit{non-fiction}, F: \textit{fiction}}
\end{tabular}
\end{adjustbox}
\caption{Ground-truth and IMaGINe-predicted confidence score heat-map encodings in gray color code}
\label{tab:heatmap}
\end{figure*}

\clearpage

\section{Performance Stagnation Analysis of IMAGINE}

\noindent
In this section, we first explore the quantitative analysis for genre indistinguishability and then the qualitative analysis for misprediction by IMAGINE.

\subsection{Qualitative Analysis for Misprediction due to insufficient information on samples:}
\noindent
Our analysis of misprediction indicates that insufficient information on some samples is the one potential cause of these errors. Even human evaluators may find it challenging to determine genres from some samples accurately. Table \ref{tab:misprediction_sample} presents examples of IMAGINE's misprediction.
It is notable that some of the samples can easily misinterpreted in terms of actual genre due to insufficient information on description text and misleading coverage images (e.g., Table \ref{tab:misprediction_sample}: \emph{(a), (b), (c), (d)}).

Based on the above analysis, we recommend providing detailed blurb and redesigning the cover page of these books to better reflect their true genres. These will help to prevent misunderstandings, attract the right audience, and ensure that viewers engage with content that aligns with their interests.

\begin{table}[!hbt]
\centering
\caption{Misprediction due to insufficient information on samples}
\begin{adjustbox}{width=0.5\textwidth}
% \begin{adjustbox}{angle=90, height=1\textheight}
% \footnotesize
\begin{tabular}{c|ll}%p{0.9\textwidth}}
% \multicolumn{3}{c}{(a) Samples for heatmap analysis}\\
\hline \hline

\hline \hline
\rowcolor[HTML]{D9D9D9}
\multicolumn{3}{c}{\textbf{{\emph{(a)}} 9780760705902: The awakening; Author: Kate Chopin; Publisher: Barnes \& Noble Books}}\\
\hline \hline
& \\ [\dimexpr-\normalbaselineskip+1.5pt]

\multirow{6}{*}{\includegraphics[width=0.15\linewidth]{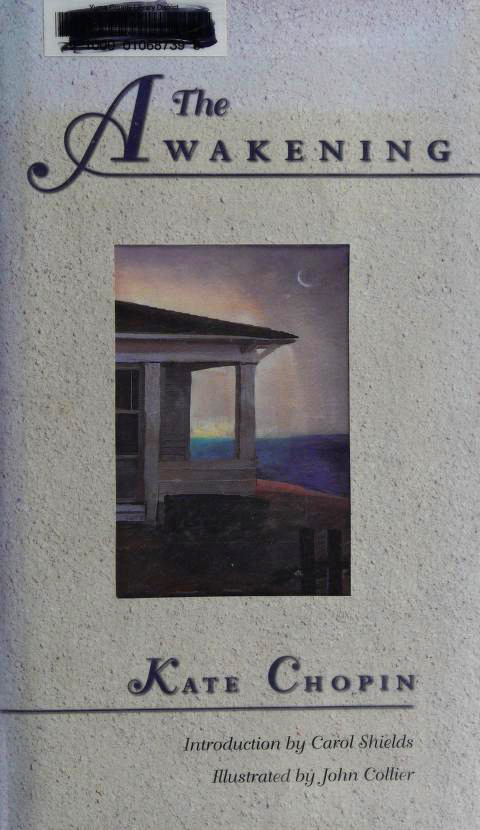}} & \multirow{2}{*}{\textbf{Blurb}:} & \multirow{2}{*}{The Awakening}\\ %\cline{2-3}
& & \\ \cline{2-3}
% & ${\cal{M}}$ & \{"author":"Kate Chopin","publisher":"Barnes \& Noble Books"\}\\ \hline
& \multirow{2}{*}{\textbf{Actual Genre}:} & \multirow{2}{*}{(Fiction, \{History, Humanities, Literature, Teen \& Young Adult\})}\\ %\cline{2-3}
& & \\ \cline{2-3}
& \multirow{2}{*}{\textbf{Predicted Genre}:} & \multirow{2}{*}{(Fiction, \{Arts \& Photography, Environment \& Plant, Literature\})}\\
& & \\

\hline \hline
\rowcolor[HTML]{D9D9D9}
\multicolumn{3}{c}{\textbf{{\emph{(b)}} 9780826400475: Pedagogy of the oppressed; Author: Paulo Freire; Publisher: Continuum}}\\
\hline \hline
& \\ [\dimexpr-\normalbaselineskip+1.5pt]

\multirow{6}{*}{\includegraphics[width=0.15\linewidth]{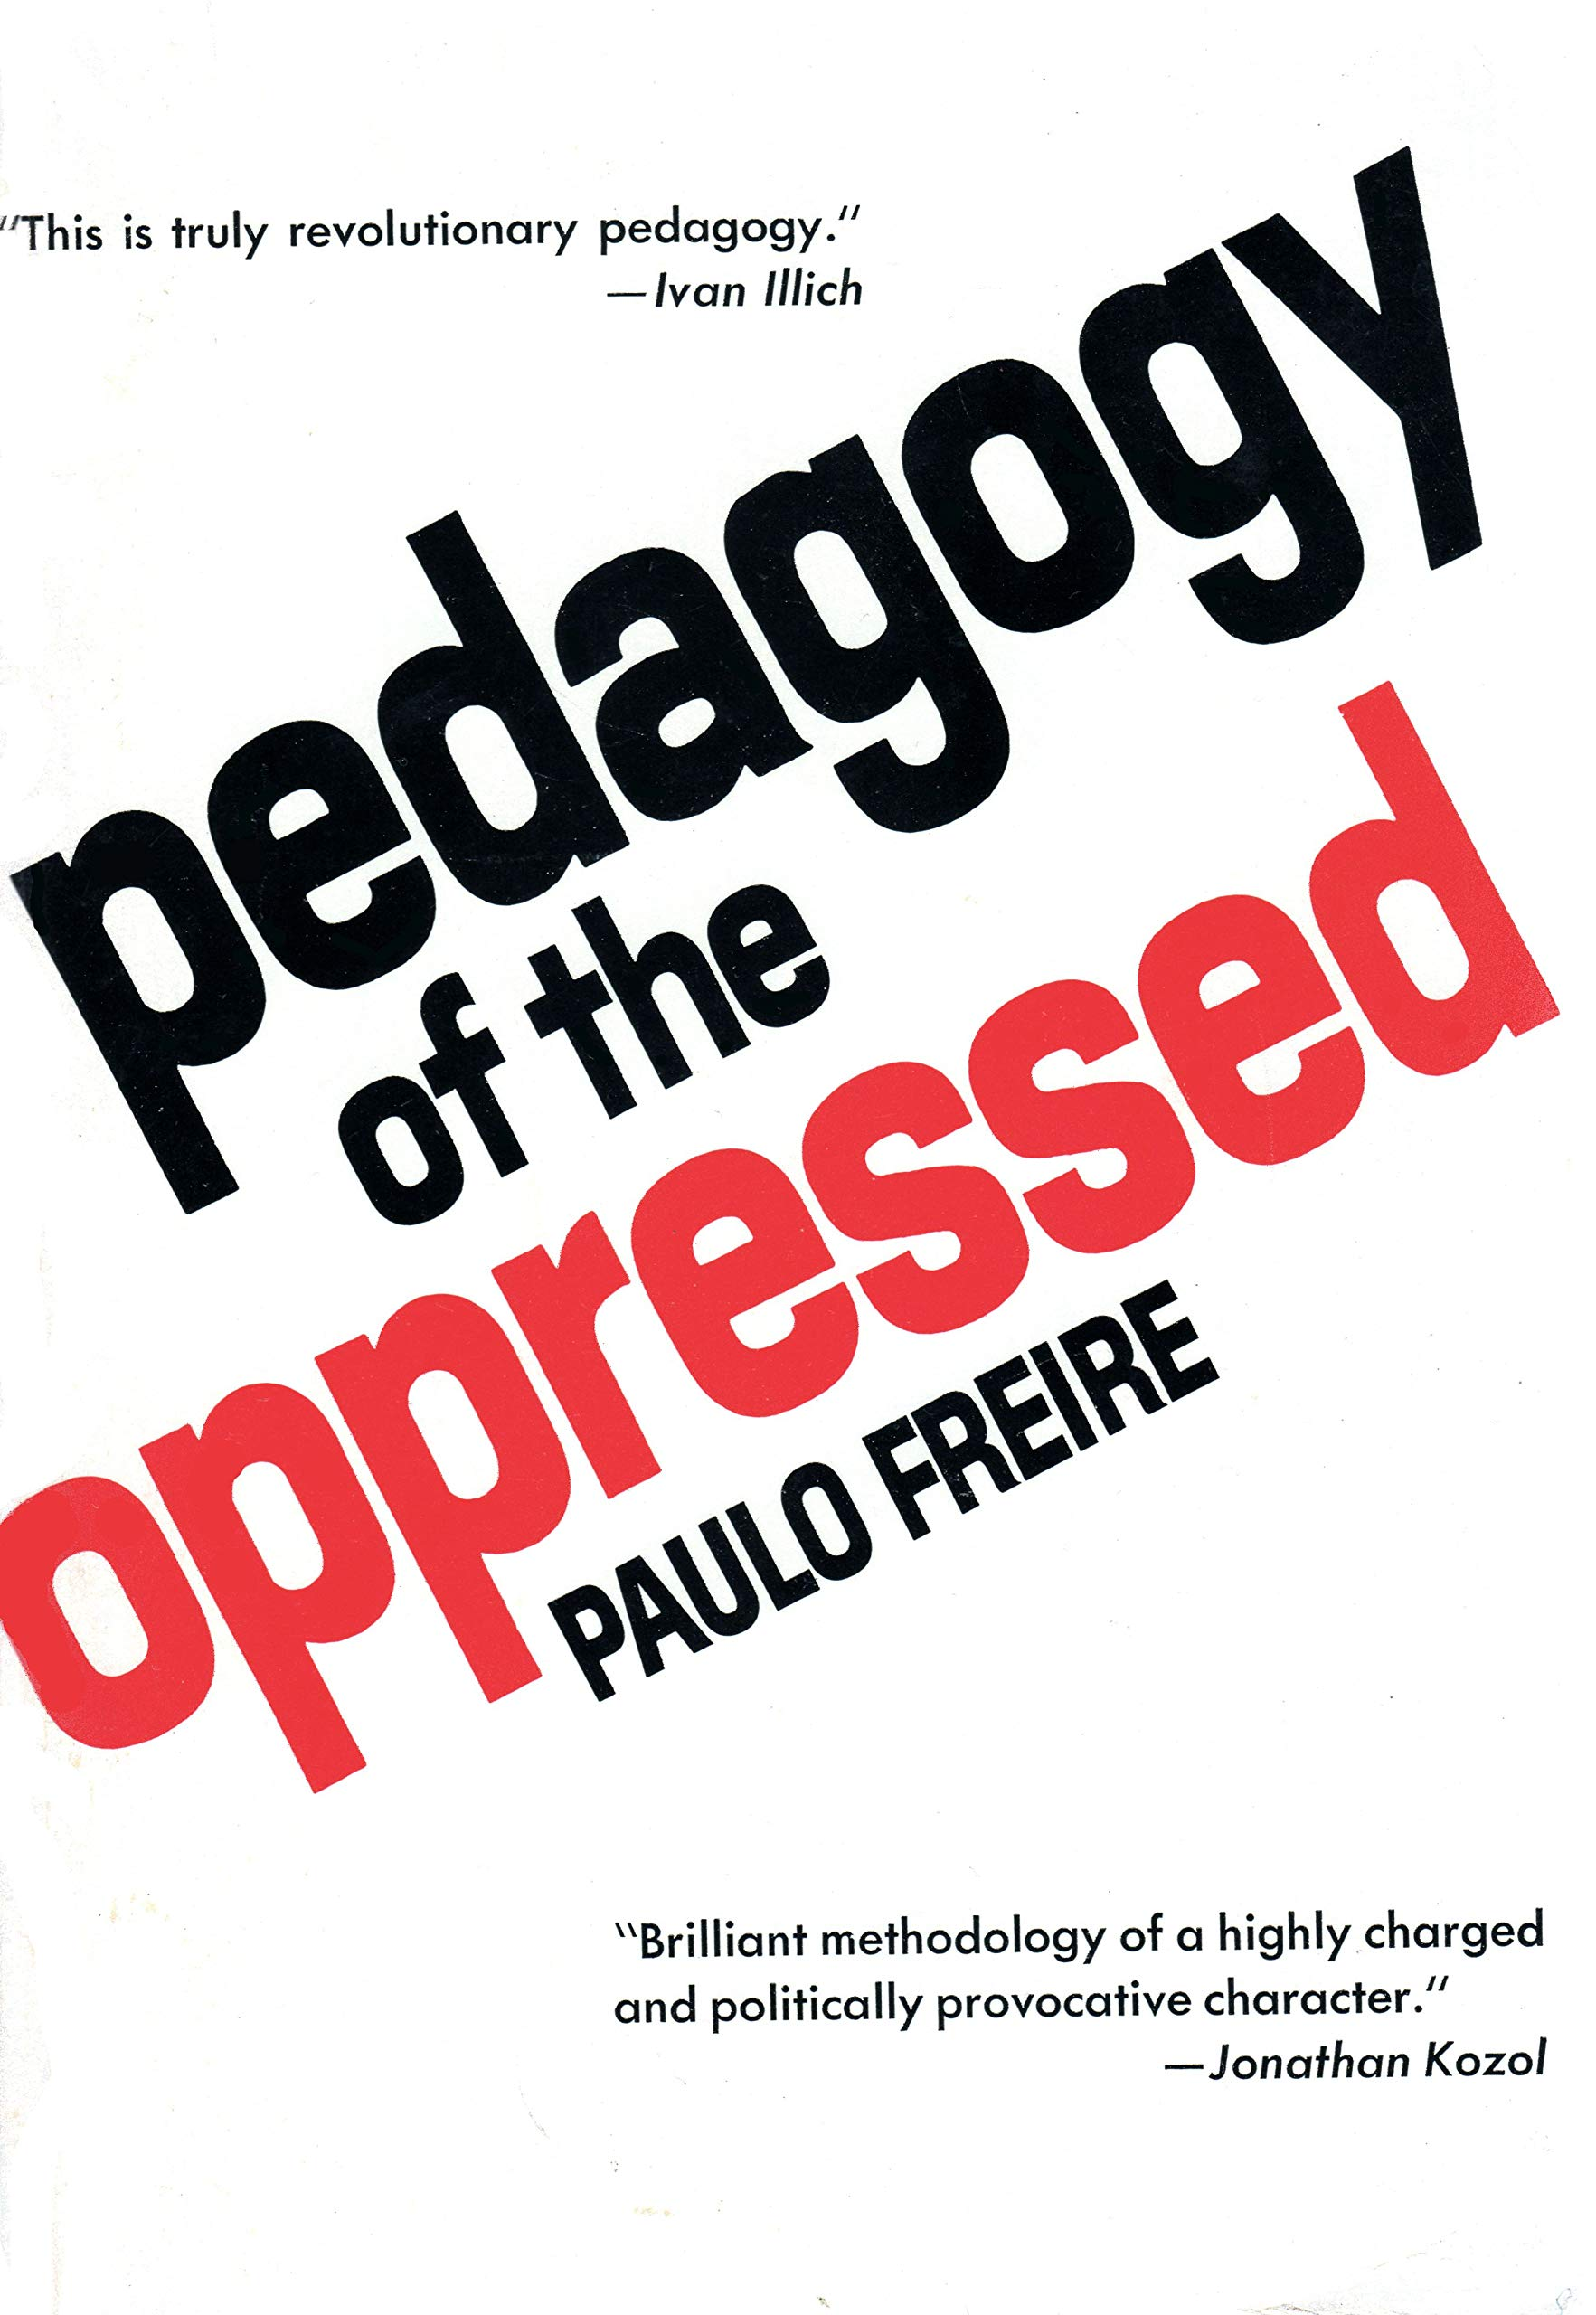}} & \multirow{2}{*}{\textbf{Blurb}:} & \multirow{2}{*}{TSIGNED COPY BY THE AUTHOR} \\ 
& & \\
\cline{2-3}

%& ${\cal{M}}$ & \{"author":"Paulo Freire","publisher":"Continuum"\}\\ \hline
& \multirow{2}{*}{\textbf{Actual Genre}:} & \multirow{2}{*}{(Non-fiction, \{Humanities\})}\\ 
& & \\
\cline{2-3}
& \multirow{2}{*}{\textbf{Predicted Genre}:} & \multirow{2}{*}{(Non-fiction, \{Science \& Math \& Mathematics\})} \\
& & \\

\hline \hline
\rowcolor[HTML]{D9D9D9}
\multicolumn{3}{c}{\textbf{{\emph{(c)}} 9788420478722: LA Caverna De Las Ideas; Author: Jose Carlos Somoza; Publisher: Alfaguara}}\\
\hline \hline

\multirow{6}{*}{\includegraphics[width=0.15\linewidth]{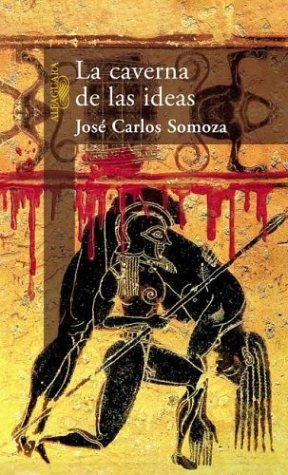}} & \multirow{2}{*}{\textbf{Blurb}:} & \multirow{2}{*}{Book by Jose Carlos Somoza} \\
& &  \\ \cline{2-3}

% & ${\cal{M}}$ & \{"author":"Jose Carlos Somoza","publisher":"Aguilar"\}\\
% \hline

& \multirow{2}{*}{\textbf{Actual Genre}:} & \multirow{2}{*}{(Fiction, \{History, Humanities, Literature, Mystery \& Thriller \& Suspense \& Horror\})}\\
& &  \\ \cline{2-3}
& \multirow{2}{*}{\textbf{Predicted Genre}:} & \multirow{2}{*}{(Fiction, \{Arts \& Photography, Literature, Reference \& Language, Sci-Fi\})} \\
& &  \\

\hline \hline
\rowcolor[HTML]{D9D9D9}
\multicolumn{3}{c}{\textbf{{\emph{(d)}} 9781571740601: Gooberz; Author: Linda Goodman; Publisher: Hampton Roads Publishing Company}}\\
\hline \hline

\multirow{6}{*}{\includegraphics[width=0.15\linewidth]{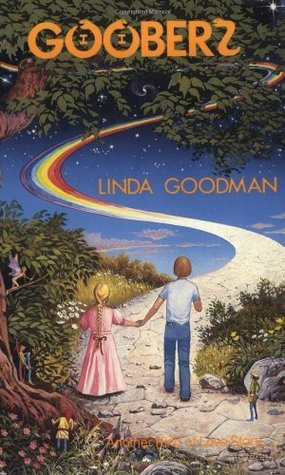}} & \multirow{2}{*}{\textbf{Blurb}:} & \multirow{2}{*}{Paperback} \\
& & \\
\cline{2-3}
% & ${\cal{M}}$ & \{"author":"Linda Goodman","publisher":"Hampton Roads Publishing Company"\}\\
% \hline
& \multirow{2}{*}{\textbf{Actual Genre}:} & \multirow{2}{*}{(Fiction, \{Literature, Mythology \& Religion \& Spirituality\})}\\
& & \\
\cline{2-3}
& \multirow{2}{*}{\textbf{Predicted Genre}:} & \multirow{2}{*}{(Fiction, \{Arts \& Photography, Literature, Sci-Fi\})}\\
& & \\

\hline

% \multicolumn{3}{r}{${\cal{I}}$: Coverpage Image, ${\cal{T}}$: Description Text, ${\cal{M}}$: Metadata}
\end{tabular}
\end{adjustbox}

\label{tab:misprediction_sample}

\end{table}

\begin{table*}[]
\centering
\caption{Fiction genre indistinguishability analysis}

% \begin{adjustbox}{angle=90, height=0.87\textheight}
\begin{adjustbox}{width=1\textwidth} 
\begin{tabular}{c|c|c|c|c|c|c|c|c|c|c|c|c|c|c|c|c|c|c|c|c|c|c|c|c|c|c|c|c|c|c}
\hline
& Class ID $\downarrow\rightarrow$  & 1 & 2 & 3 & 4 & 5 & 6 & 7 & 8 & 9 & 10 & 11 & 12 & 13 & 14 & 15 & 16 & 17 & 18 & 19 & 20 & 21 & 22 & 23 & 24 & 25 & 26 & 27 & 28 & 29 \\

%%%%%%%%%%%%%%%%%%%%%%%%%%%%%%%%%%%%%%%%%%%
% Sample Count
%%%%%%%%%%%%%%%%%%%%%%%%%%%%%%%%%%%%%%%%%%%
\hline \hline
\rowcolor[HTML]{D9D9D9}
\multicolumn{31}{c}{(a) \textbf{Sample Count}}\\
\hline \hline

 \multirow{29}{*}{\rotatebox{90}{Actual Class ID $\downarrow$}} & 1 & 1002 & 539 & 0 & 817 & 23 & 0 & 153 & 0 & 206 & 143 & 0 & 102 & 41 & 38 & 190 & 362 & 38 & 45 & 158 & 52 & 0 & 0 & 16 & 33 & 27 & 0 & 248 & 0 & 304 \\
 & 2 & 539 & 2024 & 12 & 1279 & 32 & 68 & 308 & 44 & 206 & 319 & 24 & 141 & 129 & 54 & 435 & 716 & 46 & 81 & 204 & 137 & 23 & 102 & 154 & 44 & 71 & 53 & 327 & 39 & 882 \\
 & 3 & 0 & 12 & 510 & 0 & 28 & 18 & 0 & 0 & 0 & 0 & 0 & 0 & 154 & 109 & 44 & 160 & 0 & 0 & 213 & 30 & 14 & 0 & 0 & 0 & 106 & 0 & 0 & 14 & 69 \\
 & 4 & 817 & 1279 & 0 & 2575 & 104 & 69 & 291 & 44 & 262 & 387 & 0 & 174 & 273 & 72 & 449 & 997 & 70 & 109 & 484 & 242 & 14 & 51 & 74 & 25 & 83 & 189 & 979 & 19 & 876 \\
 & 5 & 23 & 32 & 28 & 104 & 643 & 19 & 9 & 0 & 0 & 0 & 0 & 0 & 62 & 32 & 270 & 32 & 0 & 0 & 137 & 0 & 9 & 19 & 69 & 17 & 0 & 19 & 56 & 0 & 299 \\
 & 6 & 0 & 68 & 18 & 69 & 19 & 473 & 0 & 0 & 0 & 0 & 0 & 0 & 39 & 18 & 54 & 137 & 0 & 0 & 154 & 0 & 0 & 19 & 16 & 18 & 0 & 179 & 16 & 36 & 419 \\
 & 7 & 153 & 308 & 0 & 291 & 9 & 0 & 646 & 0 & 16 & 62 & 38 & 102 & 24 & 40 & 191 & 306 & 16 & 0 & 133 & 16 & 8 & 0 & 92 & 17 & 0 & 0 & 52 & 32 & 103 \\
 & 8 & 0 & 44 & 0 & 44 & 0 & 0 & 0 & 408 & 0 & 0 & 77 & 0 & 103 & 0 & 0 & 191 & 0 & 0 & 268 & 44 & 0 & 52 & 0 & 52 & 0 & 0 & 52 & 0 & 0 \\
 & 9 & 206 & 206 & 0 & 262 & 0 & 0 & 16 & 0 & 713 & 40 & 26 & 0 & 141 & 104 & 40 & 441 & 0 & 0 & 158 & 84 & 0 & 0 & 36 & 48 & 0 & 50 & 76 & 25 & 184 \\
 & 10 & 143 & 319 & 0 & 387 & 0 & 0 & 62 & 0 & 40 & 638 & 80 & 48 & 130 & 0 & 103 & 371 & 31 & 0 & 20 & 48 & 0 & 0 & 97 & 0 & 36 & 0 & 94 & 8 & 28 \\
 & 11 & 0 & 24 & 0 & 0 & 0 & 0 & 38 & 77 & 26 & 80 & 1128 & 96 & 254 & 139 & 99 & 614 & 89 & 54 & 256 & 151 & 0 & 9 & 376 & 0 & 153 & 0 & 18 & 66 & 159 \\
 & 12 & 102 & 141 & 0 & 174 & 0 & 0 & 102 & 0 & 0 & 48 & 96 & 566 & 30 & 200 & 79 & 365 & 257 & 0 & 84 & 21 & 0 & 0 & 9 & 0 & 0 & 0 & 142 & 0 & 76 \\
 & 13 & 41 & 129 & 154 & 273 & 62 & 39 & 24 & 103 & 141 & 130 & 254 & 30 & 2473 & 138 & 70 & 985 & 108 & 155 & 650 & 382 & 73 & 20 & 574 & 77 & 187 & 65 & 400 & 174 & 506 \\
 & 14 & 38 & 54 & 109 & 72 & 32 & 18 & 40 & 0 & 104 & 0 & 139 & 200 & 138 & 1169 & 85 & 693 & 226 & 40 & 256 & 287 & 0 & 34 & 97 & 8 & 229 & 26 & 146 & 86 & 339 \\
 & 15 & 190 & 435 & 44 & 449 & 270 & 54 & 191 & 0 & 40 & 103 & 99 & 79 & 70 & 85 & 1595 & 604 & 25 & 172 & 271 & 38 & 40 & 42 & 100 & 19 & 34 & 40 & 159 & 83 & 454 \\
 & 16 & 362 & 716 & 160 & 997 & 32 & 137 & 306 & 191 & 441 & 371 & 614 & 365 & 985 & 693 & 604 & 4730 & 378 & 218 & 1044 & 496 & 67 & 216 & 803 & 219 & 277 & 88 & 899 & 425 & 1175 \\
 & 17 & 158 & 204 & 213 & 484 & 137 & 154 & 133 & 268 & 158 & 20 & 256 & 84 & 650 & 256 & 271 & 1044 & 200 & 214 & 3371 & 258 & 168 & 0 & 379 & 158 & 90 & 236 & 471 & 242 & 1184 \\
 & 18 & 38 & 46 & 0 & 70 & 0 & 0 & 16 & 0 & 0 & 31 & 89 & 257 & 108 & 226 & 25 & 378 & 752 & 0 & 200 & 29 & 46 & 0 & 117 & 24 & 0 & 8 & 114 & 0 & 144 \\
 & 19 & 45 & 81 & 0 & 109 & 0 & 0 & 0 & 0 & 0 & 0 & 54 & 0 & 155 & 40 & 172 & 218 & 0 & 598 & 214 & 29 & 0 & 64 & 74 & 16 & 0 & 0 & 85 & 0 & 182 \\
 & 20 & 52 & 137 & 30 & 242 & 0 & 0 & 16 & 44 & 84 & 48 & 151 & 21 & 382 & 287 & 38 & 496 & 29 & 29 & 258 & 1517 & 0 & 73 & 352 & 18 & 615 & 0 & 171 & 56 & 427 \\
 & 21 & 0 & 23 & 14 & 14 & 9 & 0 & 8 & 0 & 0 & 0 & 0 & 0 & 73 & 0 & 40 & 67 & 46 & 0 & 168 & 0 & \textbf{396} & 23 & 0 & 16 & 0 & 0 & 0 & 14 & \textbf{264} \\
 & 22 & 0 & 102 & 0 & 51 & 19 & 19 & 0 & 52 & 0 & 0 & 9 & 0 & 20 & 34 & 42 & 216 & 0 & 64 & 0 & 73 & 23 & 560 & 0 & 118 & 0 & 63 & 76 & 11 & 379 \\
 & 23 & 16 & 154 & 0 & 74 & 69 & 16 & 92 & 0 & 36 & 97 & 376 & 9 & 574 & 97 & 100 & 803 & 117 & 74 & 379 & 352 & 0 & 0 & 1778 & 49 & 193 & 12 & 247 & 67 & 423 \\
 & 24 & 33 & 44 & 0 & 25 & 17 & 18 & 17 & 52 & 48 & 0 & 0 & 0 & 77 & 8 & 19 & 219 & 24 & 16 & 158 & 18 & 16 & 118 & 49 & 580 & 0 & 0 & 92 & 0 & 281 \\
 & 25 & 27 & 71 & 106 & 83 & 0 & 0 & 0 & 0 & 0 & 36 & 153 & 0 & 187 & 229 & 34 & 277 & 0 & 0 & 90 & 615 & 0 & 0 & 193 & 0 & 799 & 0 & 51 & 45 & 81 \\
 & 26 & 0 & 53 & 0 & 189 & 19 & 179 & 0 & 0 & 50 & 0 & 0 & 0 & 65 & 26 & 40 & 88 & 8 & 0 & 236 & 0 & 0 & 63 & 12 & 0 & 0 & 657 & 114 & 0 & 366 \\
 & 27 & 248 & 327 & 0 & 979 & 56 & 16 & 52 & 52 & 76 & 94 & 18 & 142 & 400 & 146 & 159 & 899 & 114 & 85 & 471 & 171 & 0 & 76 & 247 & 92 & 51 & 114 & 1973 & 0 & 766 \\
 & 28 & 0 & 39 & 14 & 19 & 0 & 36 & 32 & 0 & 25 & 8 & 66 & 0 & 174 & 86 & 83 & 425 & 0 & 0 & 242 & 56 & 14 & 11 & 67 & 0 & 45 & 0 & 0 & 603 & 94 \\
 & 29 & 304 & 882 & 69 & 876 & 299 & 419 & 103 & 0 & 184 & 28 & 159 & 76 & 506 & 339 & 454 & 1175 & 144 & 182 & 1184 & 427 & \textbf{264} & 379 & 423 & 281 & 81 & 366 & 766 & 94 & \textbf{3980} \\

%%%%%%%%%%%%%%%%%%%%%%%%%%%%%%%%%%%%%%%%%%%
% Cooccurrence
%%%%%%%%%%%%%%%%%%%%%%%%%%%%%%%%%%%%%%%%%%%
\hline \hline
\rowcolor[HTML]{D9D9D9}
\multicolumn{31}{c}{(b) \textbf{Cooccurrence}}\\
\hline \hline

 \multirow{29}{*}{\rotatebox{90}{Actual Class ID $\downarrow$}} & 1 & 1 & 0.27 & 0 & 0.32 & 0.04 & 0 & 0.24 & 0 & 0.29 & 0.22 & 0 & 0.18 & 0.02 & 0.03 & 0.12 & 0.08 & 0.05 & 0.08 & 0.05 & 0.03 & 0 & 0 & 0.01 & 0.06 & 0.03 & 0 & 0.13 & 0 & 0.08 \\
 & 2 & 0.54 & 1 & 0.02 & 0.50 & 0.05 & 0.14 & 0.48 & 0.11 & 0.29 & 0.50 & 0.02 & 0.25 & 0.05 & 0.05 & 0.27 & 0.15 & 0.06 & 0.14 & 0.06 & 0.09 & 0.06 & 0.18 & 0.09 & 0.08 & 0.09 & 0.08 & 0.17 & 0.06 & 0.22 \\
 & 3 & 0 & 0.01 & 1 & 0 & 0.04 & 0.04 & 0 & 0 & 0 & 0 & 0 & 0 & 0.06 & 0.09 & 0.03 & 0.03 & 0 & 0 & 0.06 & 0.02 & 0.04 & 0 & 0 & 0 & 0.13 & 0 & 0 & 0.02 & 0.02 \\
 & 4 & 0.82 & 0.63 & 0 & 1 & 0.16 & 0.15 & 0.45 & 0.11 & 0.37 & 0.61 & 0 & 0.31 & 0.11 & 0.06 & 0.28 & 0.21 & 0.09 & 0.18 & 0.14 & 0.16 & 0.04 & 0.09 & 0.04 & 0.04 & 0.10 & 0.29 & 0.50 & 0.03 & 0.22 \\
 & 5 & 0.02 & 0.02 & 0.05 & 0.04 & 1 & 0.04 & 0.01 & 0 & 0 & 0 & 0 & 0 & 0.03 & 0.03 & 0.17 & 0.01 & 0 & 0 & 0.04 & 0 & 0.02 & 0.03 & 0.04 & 0.03 & 0 & 0.03 & 0.03 & 0 & 0.08 \\
 & 6 & 0 & 0.03 & 0.04 & 0.03 & 0.03 & 1 & 0 & 0 & 0 & 0 & 0 & 0 & 0.02 & 0.02 & 0.03 & 0.03 & 0 & 0 & 0.05 & 0 & 0 & 0.03 & 0.01 & 0.03 & 0 & 0.27 & 0.01 & 0.06 & 0.11 \\
 & 7 & 0.15 & 0.15 & 0 & 0.11 & 0.01 & 0 & 1 & 0 & 0.02 & 0.10 & 0.03 & 0.18 & 0.01 & 0.03 & 0.12 & 0.06 & 0.02 & 0 & 0.04 & 0.01 & 0.02 & 0 & 0.05 & 0.03 & 0 & 0 & 0.03 & 0.05 & 0.03 \\
 & 8 & 0 & 0.02 & 0 & 0.02 & 0 & 0 & 0 & 1 & 0 & 0 & 0.07 & 0 & 0.04 & 0 & 0 & 0.04 & 0 & 0 & 0.08 & 0.03 & 0 & 0.09 & 0 & 0.09 & 0 & 0 & 0.03 & 0 & 0 \\
 & 9 & 0.21 & 0.10 & 0 & 0.10 & 0 & 0 & 0.02 & 0 & 1 & 0.06 & 0.02 & 0 & 0.06 & 0.09 & 0.03 & 0.09 & 0 & 0 & 0.05 & 0.06 & 0 & 0 & 0.02 & 0.08 & 0 & 0.08 & 0.04 & 0.04 & 0.05 \\
 & 10 & 0.14 & 0.16 & 0 & 0.15 & 0 & 0 & 0.10 & 0 & 0.06 & 1 & 0.07 & 0.08 & 0.05 & 0 & 0.06 & 0.08 & 0.04 & 0 & 0.01 & 0.03 & 0 & 0 & 0.05 & 0 & 0.05 & 0 & 0.05 & 0.01 & 0.01 \\
 & 11 & 0 & 0.01 & 0 & 0 & 0 & 0 & 0.06 & 0.19 & 0.04 & 0.13 & 1 & 0.17 & 0.10 & 0.12 & 0.06 & 0.13 & 0.12 & 0.09 & 0.08 & 0.10 & 0 & 0.02 & 0.21 & 0 & 0.19 & 0 & 0.01 & 0.11 & 0.04 \\
 & 12 & 0.10 & 0.07 & 0 & 0.07 & 0 & 0 & 0.16 & 0 & 0 & 0.08 & 0.09 & 1 & 0.01 & 0.17 & 0.05 & 0.08 & 0.34 & 0 & 0.02 & 0.01 & 0 & 0 & 0.01 & 0 & 0 & 0 & 0.07 & 0 & 0.02 \\
 & 13 & 0.04 & 0.06 & 0.30 & 0.11 & 0.10 & 0.08 & 0.04 & 0.25 & 0.20 & 0.20 & 0.23 & 0.05 & 1 & 0.12 & 0.04 & 0.21 & 0.14 & 0.26 & 0.19 & 0.25 & 0.18 & 0.04 & 0.32 & 0.13 & 0.23 & 0.10 & 0.20 & 0.29 & 0.13 \\
 & 14 & 0.04 & 0.03 & 0.21 & 0.03 & 0.05 & 0.04 & 0.06 & 0 & 0.15 & 0 & 0.12 & 0.35 & 0.06 & 1 & 0.05 & 0.15 & 0.30 & 0.07 & 0.08 & 0.19 & 0 & 0.06 & 0.05 & 0.01 & 0.29 & 0.04 & 0.07 & 0.14 & 0.09 \\
 & 15 & 0.19 & 0.21 & 0.09 & 0.17 & 0.42 & 0.11 & 0.30 & 0 & 0.06 & 0.16 & 0.09 & 0.14 & 0.03 & 0.07 & 1 & 0.13 & 0.03 & 0.29 & 0.08 & 0.03 & 0.10 & 0.08 & 0.06 & 0.03 & 0.04 & 0.06 & 0.08 & 0.14 & 0.11 \\
 & 16 & 0.36 & 0.35 & 0.31 & 0.39 & 0.05 & 0.29 & 0.47 & 0.47 & 0.62 & 0.58 & 0.54 & 0.64 & 0.40 & 0.59 & 0.38 & 1 & 0.50 & 0.36 & 0.31 & 0.33 & 0.17 & 0.39 & 0.45 & 0.38 & 0.35 & 0.13 & 0.46 & 0.70 & 0.30 \\
 & 17 & 0.16 & 0.10 & 0.42 & 0.19 & 0.21 & 0.33 & 0.21 & 0.66 & 0.22 & 0.03 & 0.23 & 0.15 & 0.26 & 0.22 & 0.17 & 0.22 & 0.27 & 0.36 & 1 & 0.17 & 0.42 & 0 & 0.21 & 0.27 & 0.11 & 0.36 & 0.24 & 0.40 & 0.30 \\
 & 18 & 0.04 & 0.02 & 0 & 0.03 & 0 & 0 & 0.02 & 0 & 0 & 0.05 & 0.08 & 0.45 & 0.04 & 0.19 & 0.02 & 0.08 & 1 & 0 & 0.06 & 0.02 & 0.12 & 0 & 0.07 & 0.04 & 0 & 0.01 & 0.06 & 0 & 0.04 \\
 & 19 & 0.04 & 0.04 & 0 & 0.04 & 0 & 0 & 0 & 0 & 0 & 0 & 0.05 & 0 & 0.06 & 0.03 & 0.11 & 0.05 & 0 & 1 & 0.06 & 0.02 & 0 & 0.11 & 0.04 & 0.03 & 0 & 0 & 0.04 & 0 & 0.05 \\
 & 20 & 0.05 & 0.07 & 0.06 & 0.09 & 0 & 0 & 0.02 & 0.11 & 0.12 & 0.08 & 0.13 & 0.04 & 0.15 & 0.25 & 0.02 & 0.10 & 0.04 & 0.05 & 0.08 & 1 & 0 & 0.13 & 0.20 & 0.03 & 0.77 & 0 & 0.09 & 0.09 & 0.11 \\
 & 21 & 0 & 0.01 & 0.03 & 0.01 & 0.01 & 0 & 0.01 & 0 & 0 & 0 & 0 & 0 & 0.03 & 0 & 0.03 & 0.01 & 0.06 & 0 & 0.05 & 0 & 1 & 0.04 & 0 & 0.03 & 0 & 0 & 0 & 0.02 & 0.07 \\
 & 22 & 0 & 0.05 & 0 & 0.02 & 0.03 & 0.04 & 0 & 0.13 & 0 & 0 & 0.01 & 0 & 0.01 & 0.03 & 0.03 & 0.05 & 0 & 0.11 & 0 & 0.05 & 0.06 & 1 & 0 & 0.20 & 0 & 0.10 & 0.04 & 0.02 & 0.10 \\
 & 23 & 0.02 & 0.08 & 0 & 0.03 & 0.11 & 0.03 & 0.14 & 0 & 0.05 & 0.15 & 0.33 & 0.02 & 0.23 & 0.08 & 0.06 & 0.17 & 0.16 & 0.12 & 0.11 & 0.23 & 0 & 0 & 1 & 0.08 & 0.24 & 0.02 & 0.13 & 0.11 & 0.11 \\
 & 24 & 0.03 & 0.02 & 0 & 0.01 & 0.03 & 0.04 & 0.03 & 0.13 & 0.07 & 0 & 0 & 0 & 0.03 & 0.01 & 0.01 & 0.05 & 0.03 & 0.03 & 0.05 & 0.01 & 0.04 & 0.21 & 0.03 & 1 & 0 & 0 & 0.05 & 0 & 0.07 \\
 & 25 & 0.03 & 0.04 & 0.21 & 0.03 & 0 & 0 & 0 & 0 & 0 & 0.06 & 0.14 & 0 & 0.08 & 0.20 & 0.02 & 0.06 & 0 & 0 & 0.03 & 0.41 & 0 & 0 & 0.11 & 0 & 1 & 0 & 0.03 & 0.07 & 0.02 \\
 & 26 & 0 & 0.03 & 0 & 0.07 & 0.03 & 0.38 & 0 & 0 & 0.07 & 0 & 0 & 0 & 0.03 & 0.02 & 0.03 & 0.02 & 0.01 & 0 & 0.07 & 0 & 0 & 0.11 & 0.01 & 0 & 0 & 1 & 0.06 & 0 & 0.09 \\
 & 27 & 0.25 & 0.16 & 0 & 0.38 & 0.09 & 0.03 & 0.08 & 0.13 & 0.11 & 0.15 & 0.02 & 0.25 & 0.16 & 0.12 & 0.10 & 0.19 & 0.15 & 0.14 & 0.14 & 0.11 & 0 & 0.14 & 0.14 & 0.16 & 0.06 & 0.17 & 1 & 0 & 0.19 \\
 & 28 & 0 & 0.02 & 0.03 & 0.01 & 0 & 0.08 & 0.05 & 0 & 0.04 & 0.01 & 0.06 & 0 & 0.07 & 0.07 & 0.05 & 0.09 & 0 & 0 & 0.07 & 0.04 & 0.04 & 0.02 & 0.04 & 0 & 0.06 & 0 & 0 & 1 & 0.02 \\
 & 29 & 0.30 & 0.44 & 0.14 & 0.34 & 0.47 & 0.89 & 0.16 & 0 & 0.26 & 0.04 & 0.14 & 0.13 & 0.20 & 0.29 & 0.28 & 0.25 & 0.19 & 0.30 & 0.35 & 0.28 & \textbf{0.67} & 0.68 & 0.24 & 0.48 & 0.10 & 0.56 & 0.39 & 0.16 & 1 \\

%%%%%%%%%%%%%%%%%%%%%%%%%%%%%%%%%%%%%%%%%%%
% Misprediction
%%%%%%%%%%%%%%%%%%%%%%%%%%%%%%%%%%%%%%%%%%%
\hline \hline
\rowcolor[HTML]{D9D9D9}
\multicolumn{31}{c}{(c) \textbf{Misprediction}}\\
\hline \hline

 \multirow{30}{*}{\rotatebox{90}{Predicted Class ID $\downarrow$}} & 1 & 0 & 0.04 & 0 & 0 & 0.01 & 0 & 0.03 & 0 & 0.01 & 0.03 & 0 & 0.02 & 0.02 & 0.01 & 0.04 & 0.01 & 0.01 & 0.01 & 0.02 & 0.02 & 0 & 0 & 0.02 & 0 & 0 & 0.01 & 0.06 & 0 & 0.02 \\
 & 2 & 0.18 & 0 & 0.02 & 0.03 & 0.13 & 0 & 0.09 & 0 & 0.04 & 0.12 & 0.03 & 0.04 & 0.06 & 0.07 & 0.09 & 0.06 & 0.01 & 0.04 & 0.07 & 0.06 & 0.09 & 0.04 & 0.07 & 0.05 & 0.06 & 0.06 & 0.08 & 0.03 & 0.04 \\
 & 3 & 0.01 & 0 & 0 & 0 & 0.01 & 0 & 0 & 0 & 0 & 0 & 0 & 0 & 0.01 & 0.01 & 0 & 0 & 0 & 0 & 0.01 & 0 & 0 & 0 & 0.01 & 0 & 0.01 & 0 & 0 & 0 & 0 \\
 & 4 & 0.64 & 0.19 & 0.02 & 0 & 0.06 & 0 & 0.09 & 0 & 0.03 & 0.18 & 0.01 & 0.04 & 0.05 & 0.03 & 0.08 & 0.06 & 0.01 & 0.01 & 0.08 & 0.07 & 0.02 & 0 & 0.05 & 0.02 & 0.02 & 0.07 & 0.13 & 0.01 & 0.06 \\
 & 5 & 0 & 0.01 & 0 & 0.01 & 0 & 0 & 0 & 0 & 0 & 0 & 0.01 & 0 & 0.01 & 0 & 0 & 0.01 & 0 & 0 & 0.01 & 0 & 0.02 & 0 & 0 & 0 & 0 & 0 & 0.01 & 0 & 0.01 \\
 & 6 & 0 & 0 & 0 & 0.01 & 0 & 0 & 0 & 0 & 0 & 0 & 0 & 0 & 0 & 0 & 0 & 0 & 0 & 0 & 0.01 & 0.01 & 0.02 & 0.03 & 0 & 0 & 0 & 0.03 & 0 & 0 & 0 \\
 & 7 & 0 & 0 & 0 & 0 & 0.01 & 0 & 0 & 0 & 0 & 0 & 0 & 0.02 & 0 & 0 & 0 & 0 & 0 & 0 & 0.01 & 0 & 0 & 0 & 0 & 0 & 0 & 0 & 0 & 0 & 0 \\
 & 8 & 0 & 0 & 0 & 0 & 0 & 0 & 0 & 0 & 0 & 0 & 0 & 0 & 0 & 0 & 0 & 0 & 0 & 0 & 0 & 0.01 & 0 & 0 & 0 & 0 & 0 & 0 & 0 & 0 & 0 \\
 & 9 & 0.02 & 0.01 & 0 & 0.01 & 0.01 & 0 & 0 & 0 & 0 & 0.01 & 0 & 0 & 0.01 & 0.03 & 0.01 & 0 & 0 & 0 & 0.02 & 0.01 & 0.02 & 0 & 0.02 & 0 & 0 & 0.01 & 0.02 & 0.01 & 0.01 \\
 & 10 & 0.03 & 0.01 & 0 & 0 & 0 & 0 & 0.01 & 0 & 0 & 0 & 0.01 & 0 & 0.02 & 0.01 & 0.02 & 0.01 & 0.01 & 0 & 0 & 0.04 & 0 & 0 & 0.03 & 0 & 0 & 0 & 0.03 & 0 & 0 \\
 & 11 & 0.02 & 0.03 & 0 & 0.01 & 0 & 0 & 0 & 0.02 & 0.01 & 0.03 & 0 & 0.02 & 0.02 & 0.03 & 0.03 & 0.02 & 0.02 & 0 & 0.04 & 0.06 & 0 & 0.02 & 0.03 & 0 & 0.01 & 0 & 0.03 & 0 & 0.01 \\
 & 12 & 0 & 0 & 0 & 0 & 0 & 0 & 0.03 & 0 & 0 & 0 & 0 & 0 & 0 & 0.02 & 0 & 0 & 0 & 0 & 0 & 0.01 & 0 & 0 & 0 & 0 & 0.01 & 0 & 0 & 0 & 0 \\
 & 13 & 0.03 & 0.06 & 0.03 & 0.05 & 0.09 & 0 & 0 & 0.05 & 0.04 & 0 & 0.18 & 0 & 0 & 0.09 & 0.05 & 0.07 & 0 & 0.08 & 0.13 & 0.14 & 0.08 & 0 & 0.09 & 0.05 & 0.03 & 0.05 & 0.08 & 0.08 & 0.08 \\
 & 14 & 0.02 & 0.02 & 0.04 & 0.01 & 0.03 & 0 & 0.01 & 0 & 0 & 0.01 & 0.04 & 0.02 & 0.01 & 0 & 0.02 & 0.02 & 0.03 & 0 & 0.03 & 0.02 & 0.07 & 0 & 0.03 & 0.01 & 0.01 & 0.04 & 0.03 & 0.02 & 0.02 \\
 & 15 & 0.01 & 0.03 & 0 & 0.02 & 0.14 & 0 & 0.05 & 0 & 0 & 0.03 & 0.03 & 0.02 & 0.02 & 0.03 & 0 & 0.03 & 0.02 & 0.02 & 0.04 & 0.01 & 0.10 & 0.02 & 0.03 & 0.03 & 0 & 0.03 & 0.03 & 0 & 0.03 \\
 & 16 & 0.16 & 0.11 & 0.10 & 0.10 & 0.16 & 0 & 0.08 & 0.07 & 0.08 & 0.21 & 0.23 & 0.05 & 0.15 & 0.51 & 0.19 & 0 & 0.04 & 0.13 & 0.17 & 0.17 & 0.15 & 0.08 & 0.17 & 0.23 & 0.08 & 0.06 & 0.26 & 0.26 & 0.10 \\
 & 17 & 0.07 & 0.05 & 0.03 & 0.04 & 0.09 & 0.03 & 0.03 & 0.05 & 0.01 & 0.04 & 0.11 & 0.02 & 0.03 & 0.11 & 0.03 & 0.04 & 0 & 0.07 & 0 & 0.04 & 0.12 & 0 & 0.02 & 0.04 & 0.02 & 0.08 & 0.03 & 0.10 & 0.05 \\
 & 18 & 0 & 0.01 & 0.02 & 0 & 0.01 & 0 & 0.03 & 0 & 0 & 0 & 0.04 & 0 & 0.01 & 0.01 & 0 & 0.01 & 0 & 0 & 0.01 & 0.01 & 0.05 & 0.01 & 0.01 & 0 & 0 & 0 & 0 & 0.01 & 0.01 \\
 & 19 & 0 & 0 & 0 & 0 & 0 & 0 & 0 & 0 & 0 & 0 & 0.01 & 0 & 0 & 0.01 & 0 & 0 & 0 & 0 & 0 & 0.01 & 0 & 0 & 0 & 0 & 0 & 0.01 & 0 & 0 & 0 \\
 & 20 & 0.02 & 0.03 & 0.06 & 0.02 & 0.03 & 0 & 0.01 & 0 & 0.04 & 0.03 & 0.04 & 0 & 0.01 & 0.06 & 0.01 & 0.03 & 0 & 0.01 & 0.05 & 0 & 0 & 0.03 & 0.02 & 0.09 & 0.19 & 0.02 & 0.02 & 0.02 & 0.03 \\
 & 21 & 0 & 0 & 0 & 0 & 0.01 & 0 & 0 & 0 & 0 & 0 & 0 & 0 & 0 & 0 & 0 & 0 & 0 & 0 & 0 & 0 & 0 & 0 & 0 & 0.01 & 0 & 0 & 0 & 0 & 0 \\
 & 22 & 0 & 0 & 0 & 0 & 0.03 & 0 & 0 & 0 & 0 & 0 & 0 & 0 & 0 & 0.01 & 0 & 0 & 0 & 0 & 0 & 0.01 & 0.05 & 0 & 0 & 0 & 0 & 0.01 & 0.02 & 0 & 0.01 \\
 & 23 & 0.02 & 0.04 & 0 & 0.03 & 0.03 & 0 & 0 & 0 & 0.03 & 0.03 & 0.15 & 0 & 0.07 & 0.07 & 0.06 & 0.05 & 0.02 & 0.05 & 0.07 & 0.11 & 0 & 0 & 0 & 0.09 & 0.01 & 0.01 & 0.06 & 0.02 & 0.04 \\
 & 24 & 0.01 & 0 & 0 & 0.01 & 0 & 0 & 0 & 0 & 0 & 0 & 0.01 & 0 & 0 & 0 & 0.01 & 0.01 & 0 & 0 & 0.02 & 0.01 & 0 & 0.04 & 0 & 0 & 0.01 & 0 & 0.02 & 0.01 & 0.02 \\
 & 25 & 0 & 0 & 0.07 & 0 & 0 & 0 & 0 & 0 & 0 & 0 & 0 & 0 & 0 & 0 & 0 & 0 & 0.01 & 0 & 0 & 0.01 & 0 & 0 & 0 & 0 & 0 & 0 & 0 & 0 & 0 \\
 & 26 & 0.01 & 0.01 & 0 & 0.01 & 0.03 & 0.03 & 0 & 0 & 0 & 0.01 & 0 & 0 & 0 & 0 & 0 & 0 & 0 & 0 & 0.01 & 0.01 & 0 & 0 & 0.01 & 0 & 0 & 0 & 0 & 0 & 0.01 \\
 & 27 & 0.09 & 0.08 & 0 & 0.12 & 0.04 & 0.02 & 0.03 & 0 & 0 & 0.03 & 0.05 & 0 & 0.05 & 0.04 & 0.05 & 0.07 & 0 & 0.01 & 0.10 & 0.08 & 0 & 0.04 & 0.09 & 0.04 & 0 & 0 & 0 & 0.01 & 0.06 \\
 & 28 & 0.01 & 0 & 0 & 0 & 0.01 & 0 & 0.01 & 0 & 0 & 0 & 0 & 0 & 0 & 0.03 & 0.01 & 0 & 0 & 0.01 & 0.02 & 0.02 & 0 & 0.02 & 0 & 0 & 0.02 & 0.02 & 0 & 0 & 0.01 \\
 & 29 & 0.13 & 0.16 & 0.04 & 0.07 & 0.38 & 0.17 & 0.03 & 0 & 0.04 & 0.03 & 0.07 & 0.02 & 0.07 & 0.13 & 0.10 & 0.07 & 0.01 & 0.02 & 0.22 & 0.12 & \textbf{0.79} & 0.14 & 0.08 & 0.25 & 0.04 & 0.30 & 0.14 & 0 & 0 \\
 & 30 & 0.01 & 0 & 0 & 0 & 0.03 & 0 & 0 & 0 & 0 & 0 & 0.01 & 0 & 0.01 & 0.01 & 0.01 & 0.01 & 0 & 0.01 & 0.01 & 0.01 & 0.02 & 0 & 0 & 0 & 0 & 0.01 & 0.01 & 0 & 0.01 \\
\hline
\end{tabular}
\end{adjustbox}

\label{tab:misclassification_fiction}
\end{table*}

\begin{table*}[]
\centering
\caption{Non-fiction genre indistinguishability analysis}

% \begin{adjustbox}{angle=90, height=0.87\textheight}
\begin{adjustbox}{width=1\textwidth} 
\begin{tabular}{c|c|c|c|c|c|c|c|c|c|c|c|c|c|c|c|c|c|c|c|c|c|c|c|c|c|c|c|c|c|c}
\hline
& Class ID $\downarrow\rightarrow$  & 1 & 2 & 3 & 4 & 5 & 6 & 7 & 8 & 9 & 10 & 11 & 12 & 13 & 14 & 15 & 16 & 17 & 18 & 19 & 20 & 21 & 22 & 23 & 24 & 25 & 26 & 27 & 28 & 30 \\

%%%%%%%%%%%%%%%%%%%%%%%%%%%%%%%%%%%%%%%%%%%
% Sample Count
%%%%%%%%%%%%%%%%%%%%%%%%%%%%%%%%%%%%%%%%%%%
\hline \hline
\rowcolor[HTML]{D9D9D9}
\multicolumn{31}{c}{(a) \textbf{Sample Count}}\\
\hline \hline

\multirow{29}{*}{\rotatebox{90}{Actual Class ID $\downarrow$}} & 1 & 748 & 169 & 0 & 222 & 41 & 0 & 12 & 0 & 306 & 14 & 0 & 12 & 89 & 52 & 97 & 44 & 14 & 10 & 0 & 16 & 0 & 95 & 0 & 369 & 14 & 0 & 65 & 37 & 157 \\
 & 2 & 169 & 1444 & 9 & 331 & 203 & 42 & 0 & 143 & 53 & 34 & 103 & 12 & 512 & 237 & 165 & 109 & 26 & 57 & 58 & 58 & 270 & 408 & 125 & 236 & 14 & 8 & 162 & 28 & 259 \\
 & 3 & 0 & 9 & 614 & 0 & 46 & 197 & 0 & 0 & 0 & 24 & 0 & 0 & 197 & 303 & 38 & 9 & 0 & 0 & 0 & 34 & 44 & 84 & 0 & 58 & 227 & 0 & 8 & 0 & 107 \\
 & 4 & 222 & 331 & 0 & 878 & 41 & 0 & 8 & 28 & 84 & 170 & 0 & 31 & 214 & 140 & 82 & 52 & 37 & 46 & 0 & 9 & 0 & 152 & 0 & 340 & 61 & 9 & 315 & 0 & 109 \\
 & 5 & 41 & 203 & 46 & 41 & 806 & 0 & 0 & 17 & 19 & 10 & 47 & 17 & 308 & 274 & 298 & 50 & 0 & 25 & 24 & 16 & 8 & 216 & 11 & 176 & 19 & 0 & 19 & 16 & 187 \\
 & 6 & 0 & 42 & 197 & 0 & 0 & 483 & 0 & 0 & 11 & 0 & 0 & 0 & 165 & 183 & 11 & 0 & 8 & 12 & 0 & 0 & 0 & 69 & 0 & 201 & 28 & 9 & 0 & 0 & 73 \\
 & 7 & 12 & 0 & 0 & 8 & 0 & 0 & 494 & 0 & 72 & 0 & 9 & 183 & 38 & 26 & 26 & 38 & 41 & 9 & 0 & 11 & 0 & 185 & 12 & 29 & 89 & 0 & 8 & 104 & 111 \\
 & 8 & 0 & 143 & 0 & 28 & 17 & 0 & 0 & 439 & 45 & 0 & 110 & 8 & 52 & 44 & 8 & 19 & 0 & 34 & 0 & 32 & 0 & 290 & 0 & 0 & 47 & 8 & 0 & 0 & 12 \\
 & 9 & 306 & 53 & 0 & 84 & 19 & 11 & 72 & 45 & 846 & 0 & 0 & 66 & 197 & 132 & 37 & 39 & 11 & 0 & 76 & 17 & 9 & 174 & 0 & 361 & 9 & 55 & 41 & 122 & 196 \\
 & 10 & 14 & 34 & 24 & 170 & 10 & 0 & 0 & 0 & 0 & 889 & 119 & 142 & 16 & 521 & 33 & 25 & 149 & 84 & 0 & 193 & 0 & 222 & 225 & 54 & 506 & 9 & 80 & 0 & 57 \\
 & 11 & 0 & 103 & 0 & 0 & 47 & 0 & 9 & 110 & 0 & 119 & 896 & 0 & 210 & 398 & 85 & 216 & 12 & 68 & 47 & 71 & 33 & 223 & 282 & 39 & 133 & 12 & 0 & 9 & 204 \\
 & 12 & 12 & 12 & 0 & 31 & 17 & 0 & 183 & 8 & 66 & 142 & 0 & 949 & 17 & 381 & 0 & 11 & 456 & 0 & 0 & 92 & 0 & 400 & 11 & 221 & 506 & 16 & 0 & 0 & 84 \\
 & 13 & 89 & 512 & 197 & 214 & 308 & 165 & 38 & 52 & 197 & 16 & 210 & 17 & \textbf{3297} & 1016 & 250 & 556 & 128 & 258 & 383 & 249 & 412 & 478 & 198 & 590 & 9 & 84 & \textbf{266} & 369 & 1198 \\
 & 14 & 52 & 237 & 303 & 140 & 274 & 183 & 26 & 44 & 132 & 521 & 398 & 381 & 1016 & 3417 & 295 & 594 & 353 & 254 & 103 & 532 & 241 & 632 & 369 & 597 & 783 & 24 & 255 & 92 & 581 \\
 & 15 & 97 & 165 & 38 & 82 & 298 & 11 & 26 & 8 & 37 & 33 & 85 & 0 & 250 & 295 & 1112 & 97 & 0 & 37 & 39 & 12 & 104 & 149 & 11 & 77 & 33 & 52 & 40 & 147 & 405 \\
 & 16 & 44 & 109 & 9 & 52 & 50 & 0 & 38 & 19 & 39 & 25 & 216 & 11 & 556 & 594 & 97 & 1448 & 34 & 236 & 93 & 126 & 102 & 207 & 265 & 66 & 17 & 0 & 96 & 204 & 575 \\
 & 17 & 0 & 58 & 0 & 0 & 24 & 0 & 0 & 0 & 76 & 0 & 47 & 0 & 383 & 103 & 39 & 93 & 44 & 41 & 744 & 55 & 126 & 103 & 87 & 58 & 9 & 81 & 0 & 221 & 383 \\
 & 18 & 14 & 26 & 0 & 37 & 0 & 8 & 41 & 0 & 11 & 149 & 12 & 456 & 128 & 353 & 0 & 34 & 886 & 0 & 44 & 143 & 9 & 241 & 20 & 318 & 361 & 0 & 0 & 0 & 179 \\
 & 19 & 10 & 57 & 0 & 46 & 25 & 12 & 9 & 34 & 0 & 84 & 68 & 0 & 258 & 254 & 37 & 236 & 0 & 762 & 41 & 52 & 0 & 315 & 0 & 32 & 27 & 0 & 25 & 37 & 289 \\
 & 20 & 16 & 58 & 34 & 9 & 16 & 0 & 11 & 32 & 17 & 193 & 71 & 92 & 249 & 532 & 12 & 126 & 143 & 52 & 55 & 1122 & 0 & 135 & 205 & 93 & 416 & 12 & 0 & 36 & 147 \\
 & 21 & 0 & 270 & 44 & 0 & 8 & 0 & 0 & 0 & 9 & 0 & 33 & 0 & 412 & 241 & 104 & 102 & 9 & 0 & 126 & 0 & 735 & 104 & 42 & 42 & 0 & 11 & 8 & 67 & 278 \\
 & 22 & 95 & 408 & 84 & 152 & 216 & 69 & 185 & 290 & 174 & 222 & 223 & 400 & 478 & 632 & 149 & 207 & 241 & 315 & 103 & 135 & 104 & 2495 & 171 & 327 & 462 & 129 & 149 & 72 & 107 \\
 & 23 & 0 & 125 & 0 & 0 & 11 & 0 & 12 & 0 & 0 & 225 & 282 & 11 & 198 & 369 & 11 & 265 & 20 & 0 & 87 & 205 & 42 & 171 & 877 & 70 & 273 & 12 & 0 & 43 & 162 \\
 & 24 & 369 & 236 & 58 & 340 & 176 & 201 & 29 & 0 & 361 & 54 & 39 & 221 & 590 & 597 & 77 & 66 & 318 & 32 & 58 & 93 & 42 & 327 & 70 & 1809 & 148 & 0 & 188 & 41 & 207 \\
 & 25 & 14 & 14 & 227 & 61 & 19 & 28 & 89 & 47 & 9 & 506 & 133 & 506 & 9 & 783 & 33 & 17 & 361 & 27 & 9 & 416 & 0 & 462 & 273 & 148 & 1519 & 25 & 16 & 9 & 63 \\
 & 26 & 0 & 8 & 0 & 9 & 0 & 9 & 0 & 8 & 55 & 9 & 12 & 16 & 84 & 24 & 52 & 0 & 0 & 0 & 81 & 12 & 11 & 129 & 12 & 0 & 25 & 424 & 0 & 69 & 185 \\
 & 27 & 65 & 162 & 8 & 315 & 19 & 0 & 8 & 0 & 41 & 80 & 0 & 0 & \textbf{266} & 255 & 40 & 96 & 0 & 25 & 0 & 0 & 8 & 149 & 0 & 188 & 16 & 0 & \textbf{659} & 0 & 151 \\
 & 28 & 37 & 28 & 0 & 0 & 16 & 0 & 104 & 0 & 122 & 0 & 9 & 0 & 369 & 92 & 147 & 204 & 0 & 37 & 221 & 36 & 67 & 72 & 43 & 41 & 9 & 69 & 0 & 888 & 543 \\
 & 30 & 157 & 259 & 107 & 109 & 187 & 73 & 111 & 12 & 196 & 57 & 204 & 84 & 1198 & 581 & 405 & 575 & 179 & 289 & 383 & 147 & 278 & 107 & 162 & 207 & 63 & 185 & 151 & 543 & 2802 \\

%%%%%%%%%%%%%%%%%%%%%%%%%%%%%%%%%%%%%%%%%%%
% Cooccurrence
%%%%%%%%%%%%%%%%%%%%%%%%%%%%%%%%%%%%%%%%%%%
\hline \hline
\rowcolor[HTML]{D9D9D9}
\multicolumn{31}{c}{(b) \textbf{Cooccurrence}}\\
\hline \hline

 \multirow{29}{*}{\rotatebox{90}{Actual Class ID $\downarrow$}} & 1 & 1 & 0.12 & 0 & 0.25 & 0.05 & 0 & 0.02 & 0 & 0.36 & 0.02 & 0 & 0.01 & 0.03 & 0.02 & 0.09 & 0.03 & 0.02 & 0.01 & 0 & 0.01 & 0 & 0.04 & 0 & 0.20 & 0.01 & 0 & 0.10 & 0.04 & 0.06 \\
 & 2 & 0.23 & 1 & 0.01 & 0.38 & 0.25 & 0.09 & 0 & 0.33 & 0.06 & 0.04 & 0.11 & 0.01 & 0.16 & 0.07 & 0.15 & 0.08 & 0.03 & 0.07 & 0.08 & 0.05 & 0.37 & 0.16 & 0.14 & 0.13 & 0.01 & 0.02 & 0.25 & 0.03 & 0.09 \\
 & 3 & 0 & 0.01 & 1 & 0 & 0.06 & 0.41 & 0 & 0 & 0 & 0.03 & 0 & 0 & 0.06 & 0.09 & 0.03 & 0.01 & 0 & 0 & 0 & 0.03 & 0.06 & 0.03 & 0 & 0.03 & 0.15 & 0 & 0.01 & 0 & 0.04 \\
 & 4 & 0.30 & 0.23 & 0 & 1 & 0.05 & 0 & 0.02 & 0.06 & 0.10 & 0.19 & 0 & 0.03 & 0.06 & 0.04 & 0.07 & 0.04 & 0.04 & 0.06 & 0 & 0.01 & 0 & 0.06 & 0 & 0.19 & 0.04 & 0.02 & 0.48 & 0 & 0.04 \\
 & 5 & 0.05 & 0.14 & 0.07 & 0.05 & 1 & 0 & 0 & 0.04 & 0.02 & 0.01 & 0.05 & 0.02 & 0.09 & 0.08 & 0.27 & 0.03 & 0 & 0.03 & 0.03 & 0.01 & 0.01 & 0.09 & 0.01 & 0.10 & 0.01 & 0 & 0.03 & 0.02 & 0.07 \\
 & 6 & 0 & 0.03 & 0.32 & 0 & 0 & 1 & 0 & 0 & 0.01 & 0 & 0 & 0 & 0.05 & 0.05 & 0.01 & 0 & 0.01 & 0.02 & 0 & 0 & 0 & 0.03 & 0 & 0.11 & 0.02 & 0.02 & 0 & 0 & 0.03 \\
 & 7 & 0.02 & 0 & 0 & 0.01 & 0 & 0 & 1 & 0 & 0.09 & 0 & 0.01 & 0.19 & 0.01 & 0.01 & 0.02 & 0.03 & 0.05 & 0.01 & 0 & 0.01 & 0 & 0.07 & 0.01 & 0.02 & 0.06 & 0 & 0.01 & 0.12 & 0.04 \\
 & 8 & 0 & 0.10 & 0 & 0.03 & 0.02 & 0 & 0 & 1 & 0.05 & 0 & 0.12 & 0.01 & 0.02 & 0.01 & 0.01 & 0.01 & 0 & 0.04 & 0 & 0.03 & 0 & 0.12 & 0 & 0 & 0.03 & 0.02 & 0 & 0 & 0 \\
 & 9 & 0.41 & 0.04 & 0 & 0.10 & 0.02 & 0.02 & 0.15 & 0.10 & 1 & 0 & 0 & 0.07 & 0.06 & 0.04 & 0.03 & 0.03 & 0.01 & 0 & 0.10 & 0.02 & 0.01 & 0.07 & 0 & 0.20 & 0.01 & 0.13 & 0.06 & 0.14 & 0.07 \\
 & 10 & 0.02 & 0.02 & 0.04 & 0.19 & 0.01 & 0 & 0 & 0 & 0 & 1 & 0.13 & 0.15 & 0 & 0.15 & 0.03 & 0.02 & 0.17 & 0.11 & 0 & 0.17 & 0 & 0.09 & 0.26 & 0.03 & 0.33 & 0.02 & 0.12 & 0 & 0.02 \\
 & 11 & 0 & 0.07 & 0 & 0 & 0.06 & 0 & 0.02 & 0.25 & 0 & 0.13 & 1 & 0 & 0.06 & 0.12 & 0.08 & 0.15 & 0.01 & 0.09 & 0.06 & 0.06 & 0.04 & 0.09 & 0.32 & 0.02 & 0.09 & 0.03 & 0 & 0.01 & 0.07 \\
 & 12 & 0.02 & 0.01 & 0 & 0.04 & 0.02 & 0 & 0.37 & 0.02 & 0.08 & 0.16 & 0 & 1 & 0.01 & 0.11 & 0 & 0.01 & 0.51 & 0 & 0 & 0.08 & 0 & 0.16 & 0.01 & 0.12 & 0.33 & 0.04 & 0 & 0 & 0.03 \\
 & 13 & 0.12 & 0.35 & 0.32 & 0.24 & 0.38 & 0.34 & 0.08 & 0.12 & 0.23 & 0.02 & 0.23 & 0.02 & 1 & 0.30 & 0.22 & 0.38 & 0.14 & 0.34 & 0.51 & 0.22 & 0.56 & 0.19 & 0.23 & 0.33 & 0.01 & 0.20 & \textbf{0.40} & 0.42 & 0.43 \\
 & 14 & 0.07 & 0.16 & 0.49 & 0.16 & 0.34 & 0.38 & 0.05 & 0.10 & 0.16 & 0.59 & 0.44 & 0.40 & 0.31 & 1 & 0.27 & 0.41 & 0.40 & 0.33 & 0.14 & 0.47 & 0.33 & 0.25 & 0.42 & 0.33 & 0.52 & 0.06 & 0.39 & 0.10 & 0.21 \\
 & 15 & 0.13 & 0.11 & 0.06 & 0.09 & 0.37 & 0.02 & 0.05 & 0.02 & 0.04 & 0.04 & 0.09 & 0 & 0.08 & 0.09 & 1 & 0.07 & 0 & 0.05 & 0.05 & 0.01 & 0.14 & 0.06 & 0.01 & 0.04 & 0.02 & 0.12 & 0.06 & 0.17 & 0.14 \\
 & 16 & 0.06 & 0.08 & 0.01 & 0.06 & 0.06 & 0 & 0.08 & 0.04 & 0.05 & 0.03 & 0.24 & 0.01 & 0.17 & 0.17 & 0.09 & 1 & 0.04 & 0.31 & 0.13 & 0.11 & 0.14 & 0.08 & 0.30 & 0.04 & 0.01 & 0 & 0.15 & 0.23 & 0.21 \\
 & 17 & 0 & 0.04 & 0 & 0 & 0.03 & 0 & 0 & 0 & 0.09 & 0 & 0.05 & 0 & 0.12 & 0.03 & 0.04 & 0.06 & 0.05 & 0.05 & 1 & 0.05 & 0.17 & 0.04 & 0.10 & 0.03 & 0.01 & 0.19 & 0 & 0.25 & 0.14 \\
 & 18 & 0.02 & 0.02 & 0 & 0.04 & 0 & 0.02 & 0.08 & 0 & 0.01 & 0.17 & 0.01 & 0.48 & 0.04 & 0.10 & 0 & 0.02 & 1 & 0 & 0.06 & 0.13 & 0.01 & 0.10 & 0.02 & 0.18 & 0.24 & 0 & 0 & 0 & 0.06 \\
 & 19 & 0.01 & 0.04 & 0 & 0.05 & 0.03 & 0.02 & 0.02 & 0.08 & 0 & 0.09 & 0.08 & 0 & 0.08 & 0.07 & 0.03 & 0.16 & 0 & 1 & 0.06 & 0.05 & 0 & 0.13 & 0 & 0.02 & 0.02 & 0 & 0.04 & 0.04 & 0.10 \\
 & 20 & 0.02 & 0.04 & 0.06 & 0.01 & 0.02 & 0 & 0.02 & 0.07 & 0.02 & 0.22 & 0.08 & 0.10 & 0.08 & 0.16 & 0.01 & 0.09 & 0.16 & 0.07 & 0.07 & 1 & 0 & 0.05 & 0.23 & 0.05 & 0.27 & 0.03 & 0 & 0.04 & 0.05 \\
 & 21 & 0 & 0.19 & 0.07 & 0 & 0.01 & 0 & 0 & 0 & 0.01 & 0 & 0.04 & 0 & 0.12 & 0.07 & 0.09 & 0.07 & 0.01 & 0 & 0.17 & 0 & 1 & 0.04 & 0.05 & 0.02 & 0 & 0.03 & 0.01 & 0.08 & 0.10 \\
 & 22 & 0.13 & 0.28 & 0.14 & 0.17 & 0.27 & 0.14 & 0.37 & 0.66 & 0.21 & 0.25 & 0.25 & 0.42 & 0.14 & 0.18 & 0.13 & 0.14 & 0.27 & 0.41 & 0.14 & 0.12 & 0.14 & 1 & 0.19 & 0.18 & 0.30 & 0.30 & 0.23 & 0.08 & 0.04 \\
 & 23 & 0 & 0.09 & 0 & 0 & 0.01 & 0 & 0.02 & 0 & 0 & 0.25 & 0.31 & 0.01 & 0.06 & 0.11 & 0.01 & 0.18 & 0.02 & 0 & 0.12 & 0.18 & 0.06 & 0.07 & 1 & 0.04 & 0.18 & 0.03 & 0 & 0.05 & 0.06 \\
 & 24 & 0.49 & 0.16 & 0.09 & 0.39 & 0.22 & 0.42 & 0.06 & 0 & 0.43 & 0.06 & 0.04 & 0.23 & 0.18 & 0.17 & 0.07 & 0.05 & 0.36 & 0.04 & 0.08 & 0.08 & 0.06 & 0.13 & 0.08 & 1 & 0.10 & 0 & 0.29 & 0.05 & 0.07 \\
 & 25 & 0.02 & 0.01 & 0.37 & 0.07 & 0.02 & 0.06 & 0.18 & 0.11 & 0.01 & 0.57 & 0.15 & 0.53 & 0 & 0.23 & 0.03 & 0.01 & 0.41 & 0.04 & 0.01 & 0.37 & 0 & 0.19 & 0.31 & 0.08 & 1 & 0.06 & 0.02 & 0.01 & 0.02 \\
 & 26 & 0 & 0.01 & 0 & 0.01 & 0 & 0.02 & 0 & 0.02 & 0.07 & 0.01 & 0.01 & 0.02 & 0.03 & 0.01 & 0.05 & 0 & 0 & 0 & 0.11 & 0.01 & 0.01 & 0.05 & 0.01 & 0 & 0.02 & 1 & 0 & 0.08 & 0.07 \\
 & 27 & 0.09 & 0.11 & 0.01 & 0.36 & 0.02 & 0 & 0.02 & 0 & 0.05 & 0.09 & 0 & 0 & 0.08 & 0.07 & 0.04 & 0.07 & 0 & 0.03 & 0 & 0 & 0.01 & 0.06 & 0 & 0.10 & 0.01 & 0 & 1 & 0 & 0.05 \\
 & 28 & 0.05 & 0.02 & 0 & 0 & 0.02 & 0 & 0.21 & 0 & 0.14 & 0 & 0.01 & 0 & 0.11 & 0.03 & 0.13 & 0.14 & 0 & 0.05 & 0.30 & 0.03 & 0.09 & 0.03 & 0.05 & 0.02 & 0.01 & 0.16 & 0 & 1 & 0.19 \\
 & 30 & 0.21 & 0.18 & 0.17 & 0.12 & 0.23 & 0.15 & 0.22 & 0.03 & 0.23 & 0.06 & 0.23 & 0.09 & 0.36 & 0.17 & 0.36 & 0.40 & 0.20 & 0.38 & 0.51 & 0.13 & 0.38 & 0.04 & 0.18 & 0.11 & 0.04 & 0.44 & 0.23 & 0.61 & 1 \\

%%%%%%%%%%%%%%%%%%%%%%%%%%%%%%%%%%%%%%%%%%%
% Misprediction
%%%%%%%%%%%%%%%%%%%%%%%%%%%%%%%%%%%%%%%%%%%
\hline \hline
\rowcolor[HTML]{D9D9D9}
\multicolumn{31}{c}{(c) \textbf{Misprediction}}\\
\hline \hline

 \multirow{30}{*}{\rotatebox{90}{Predicted Class ID $\downarrow$}}
 & 1 & 0 & 0.03 & 0.01 & 0.03 & 0.01 & 0.02 & 0 & 0 & 0.05 & 0 & 0 & 0 & 0.01 & 0.01 & 0.01 & 0.02 & 0 & 0 & 0.01 & 0.01 & 0.01 & 0.01 & 0 & 0.04 & 0 & 0 & 0.06 & 0 & 0 \\
 & 2 & 0.03 & 0 & 0.03 & 0.06 & 0.03 & 0 & 0.02 & 0.03 & 0 & 0.02 & 0.01 & 0 & 0.04 & 0.01 & 0.01 & 0.03 & 0 & 0.01 & 0.02 & 0.01 & 0.09 & 0.02 & 0 & 0.04 & 0 & 0 & 0.10 & 0.02 & 0.05 \\
 & 3 & 0 & 0.01 & 0 & 0 & 0 & 0 & 0 & 0 & 0 & 0.01 & 0 & 0 & 0 & 0.03 & 0 & 0.01 & 0 & 0 & 0 & 0.02 & 0 & 0.02 & 0 & 0 & 0.02 & 0 & 0 & 0 & 0 \\
 & 4 & 0.03 & 0.03 & 0 & 0 & 0 & 0 & 0 & 0 & 0.01 & 0.04 & 0 & 0 & 0.01 & 0.01 & 0.02 & 0.01 & 0.01 & 0 & 0.01 & 0.01 & 0.01 & 0.01 & 0.01 & 0.04 & 0.01 & 0 & 0.17 & 0.01 & 0.01 \\
 & 5 & 0.01 & 0 & 0 & 0 & 0 & 0 & 0 & 0 & 0 & 0 & 0 & 0.01 & 0 & 0 & 0 & 0.01 & 0 & 0 & 0.04 & 0 & 0 & 0 & 0 & 0.01 & 0 & 0 & 0.04 & 0 & 0 \\
 & 6 & 0 & 0.01 & 0.06 & 0.01 & 0 & 0 & 0 & 0 & 0 & 0 & 0.01 & 0 & 0.01 & 0.01 & 0.01 & 0.01 & 0.01 & 0 & 0 & 0 & 0 & 0 & 0 & 0.01 & 0.01 & 0 & 0 & 0 & 0.01 \\
 & 7 & 0 & 0 & 0 & 0 & 0 & 0 & 0 & 0 & 0.01 & 0 & 0 & 0.01 & 0.01 & 0 & 0 & 0.01 & 0.01 & 0 & 0 & 0 & 0 & 0.01 & 0 & 0 & 0 & 0 & 0 & 0.01 & 0.01 \\
 & 8 & 0 & 0 & 0 & 0 & 0 & 0 & 0 & 0 & 0 & 0 & 0.01 & 0 & 0 & 0 & 0 & 0 & 0 & 0.01 & 0 & 0 & 0 & 0.01 & 0 & 0 & 0.01 & 0 & 0 & 0 & 0 \\
 & 9 & 0.07 & 0.02 & 0 & 0.04 & 0 & 0 & 0 & 0 & 0 & 0 & 0 & 0.01 & 0.01 & 0.02 & 0.02 & 0.02 & 0 & 0 & 0 & 0.01 & 0.02 & 0 & 0 & 0.02 & 0.01 & 0 & 0.05 & 0.03 & 0.02 \\
 & 10 & 0 & 0.01 & 0 & 0 & 0 & 0 & 0 & 0 & 0 & 0 & 0 & 0.02 & 0 & 0.03 & 0.01 & 0.01 & 0.01 & 0 & 0 & 0.04 & 0.01 & 0 & 0.01 & 0 & 0.06 & 0 & 0.03 & 0.01 & 0.01 \\
 & 11 & 0.02 & 0.01 & 0 & 0 & 0.01 & 0 & 0.02 & 0 & 0 & 0 & 0 & 0.01 & 0.01 & 0.01 & 0.01 & 0.03 & 0.04 & 0 & 0 & 0.01 & 0.01 & 0 & 0 & 0 & 0.02 & 0 & 0.01 & 0.02 & 0.03 \\
 & 12 & 0.01 & 0 & 0 & 0 & 0 & 0 & 0.09 & 0 & 0 & 0.02 & 0 & 0 & 0 & 0.01 & 0 & 0 & 0 & 0 & 0 & 0.02 & 0 & 0.02 & 0 & 0.02 & 0.01 & 0 & 0 & 0 & 0 \\
 & 13 & 0.03 & 0.06 & 0.16 & 0.09 & 0.10 & 0.03 & 0.02 & 0 & 0.03 & 0 & 0.09 & 0 & 0 & 0.06 & 0.09 & 0.16 & 0.04 & 0.03 & 0.23 & 0.04 & 0.11 & 0.02 & 0.01 & 0.04 & 0.01 & 0.03 & \textbf{0.43} & 0.24 & 0.16 \\
 & 14 & 0 & 0.06 & 0.08 & 0 & 0.05 & 0 & 0 & 0.07 & 0.01 & 0.10 & 0.05 & 0.04 & 0 & 0 & 0.07 & 0.09 & 0.07 & 0.03 & 0.07 & 0.15 & 0.11 & 0.02 & 0.02 & 0.07 & 0.09 & 0.02 & 0.25 & 0.07 & 0.05 \\
 & 15 & 0.03 & 0.01 & 0 & 0.02 & 0.05 & 0 & 0 & 0 & 0 & 0.01 & 0 & 0 & 0.01 & 0 & 0 & 0.02 & 0 & 0.01 & 0.02 & 0 & 0.04 & 0 & 0 & 0.01 & 0 & 0 & 0.05 & 0.05 & 0.02 \\
 & 16 & 0.02 & 0.01 & 0.01 & 0.01 & 0.03 & 0 & 0.02 & 0.02 & 0 & 0.02 & 0.03 & 0.01 & 0.04 & 0.04 & 0 & 0 & 0.02 & 0.09 & 0.04 & 0.04 & 0.01 & 0.01 & 0 & 0.01 & 0.01 & 0.02 & 0.10 & 0.14 & 0.11 \\
 & 17 & 0.01 & 0 & 0.03 & 0 & 0 & 0 & 0 & 0 & 0.01 & 0 & 0.03 & 0 & 0.02 & 0.02 & 0 & 0 & 0.03 & 0.01 & 0 & 0 & 0 & 0.01 & 0 & 0.01 & 0 & 0.02 & 0.03 & 0.07 & 0.04 \\
 & 18 & 0.01 & 0 & 0 & 0 & 0 & 0 & 0.04 & 0 & 0 & 0.02 & 0 & 0 & 0 & 0.01 & 0.02 & 0 & 0 & 0 & 0 & 0.02 & 0 & 0 & 0 & 0.01 & 0.01 & 0 & 0 & 0 & 0 \\
 & 19 & 0 & 0.01 & 0 & 0.01 & 0 & 0 & 0 & 0.06 & 0 & 0.01 & 0.01 & 0 & 0 & 0.01 & 0 & 0.01 & 0 & 0 & 0 & 0.02 & 0 & 0.01 & 0 & 0 & 0 & 0 & 0.01 & 0.01 & 0.01 \\
 & 20 & 0.01 & 0.04 & 0 & 0.02 & 0.02 & 0 & 0 & 0 & 0 & 0.01 & 0.01 & 0.01 & 0.03 & 0.01 & 0 & 0.03 & 0.05 & 0.01 & 0 & 0 & 0.01 & 0.01 & 0 & 0.01 & 0.03 & 0 & 0.04 & 0.02 & 0.03 \\
 & 21 & 0 & 0.01 & 0.07 & 0 & 0 & 0 & 0 & 0 & 0 & 0 & 0.01 & 0 & 0.01 & 0 & 0 & 0 & 0 & 0 & 0.03 & 0 & 0 & 0 & 0 & 0 & 0 & 0 & 0.01 & 0.04 & 0.02 \\
 & 22 & 0.03 & 0.01 & 0.02 & 0.04 & 0.03 & 0.04 & 0.06 & 0.24 & 0.04 & 0.07 & 0 & 0.05 & 0.03 & 0.04 & 0.06 & 0.02 & 0.01 & 0 & 0 & 0.04 & 0 & 0 & 0 & 0.03 & 0.02 & 0.03 & 0.08 & 0.02 & 0.01 \\
 & 23 & 0.02 & 0 & 0 & 0 & 0.02 & 0 & 0 & 0 & 0 & 0 & 0.01 & 0 & 0 & 0.01 & 0.01 & 0.02 & 0.01 & 0 & 0.01 & 0.04 & 0 & 0 & 0 & 0.01 & 0.01 & 0.02 & 0 & 0.02 & 0.03 \\
 & 24 & 0.07 & 0.04 & 0.01 & 0.08 & 0.03 & 0.03 & 0.04 & 0 & 0.06 & 0.03 & 0.01 & 0.03 & 0.02 & 0.03 & 0.03 & 0.03 & 0.08 & 0 & 0.01 & 0.02 & 0.01 & 0.01 & 0 & 0 & 0.03 & 0 & 0.08 & 0 & 0 \\
 & 25 & 0.01 & 0.01 & 0.02 & 0 & 0.02 & 0 & 0.04 & 0.04 & 0.01 & 0.05 & 0.01 & 0.06 & 0.01 & 0.05 & 0.02 & 0.02 & 0.07 & 0 & 0.01 & 0.09 & 0.02 & 0.02 & 0.02 & 0 & 0 & 0 & 0.01 & 0 & 0.01 \\
 & 26 & 0.01 & 0.01 & 0 & 0.01 & 0.01 & 0.02 & 0 & 0 & 0.01 & 0 & 0.01 & 0.01 & 0.01 & 0.01 & 0.03 & 0 & 0 & 0.02 & 0 & 0.02 & 0.01 & 0.01 & 0 & 0 & 0 & 0 & 0.01 & 0.02 & 0.01 \\
 & 27 & 0 & 0.01 & 0 & 0.02 & 0 & 0 & 0 & 0 & 0 & 0.03 & 0 & 0 & 0.01 & 0.01 & 0.02 & 0 & 0 & 0.01 & 0.01 & 0 & 0 & 0 & 0 & 0 & 0.01 & 0 & 0 & 0.01 & 0.02 \\
 & 28 & 0 & 0 & 0.01 & 0 & 0.01 & 0.04 & 0 & 0 & 0.01 & 0 & 0.01 & 0 & 0.01 & 0.02 & 0.02 & 0.01 & 0 & 0 & 0.05 & 0.02 & 0.03 & 0.01 & 0 & 0.02 & 0.01 & 0 & 0 & 0 & 0.01 \\
 & 29 & 0 & 0.01 & 0 & 0.02 & 0.01 & 0 & 0.02 & 0 & 0 & 0 & 0 & 0 & 0.01 & 0.01 & 0.01 & 0.01 & 0 & 0 & 0.01 & 0.02 & 0 & 0.01 & 0 & 0.01 & 0 & 0 & 0 & 0 & 0.02 \\
 & 30 & 0.06 & 0.05 & 0.10 & 0.06 & 0.01 & 0 & 0 & 0 & 0.01 & 0.04 & 0.12 & 0.03 & 0.10 & 0.07 & 0.09 & 0.14 & 0.12 & 0.07 & 0.17 & 0.08 & 0.13 & 0.03 & 0.03 & 0.05 & 0.04 & 0.07 & 0.23 & 0.23 & 0 \\
 \hline
\end{tabular}
\end{adjustbox}
\label{tab:misclassification_non_fiction}
\end{table*}

\begin{table*}[hbt]
\centering
\caption{Example of misclassified data samples due to genre indistinguishability.}
\begin{adjustbox}{width=0.95\textwidth}
% \begin{adjustbox}{angle=90, height=1\textheight}
% \footnotesize
\begin{tabular}{c|ll}%p{0.9\textwidth}}

\hline \hline

\rowcolor[HTML]{D9D9D9}
\multicolumn{3}{c}{\textbf{\emph{(a)} 9780671501075: Dragon's Honor (Star Trek: The Next Generation, No. 38); Author: Kij Johnson; Publisher: Star Trek}}\\
\hline \hline
& \\ [\dimexpr-\normalbaselineskip+1.5pt]

\multirow{8}{*}{\includegraphics[width=0.08\linewidth]{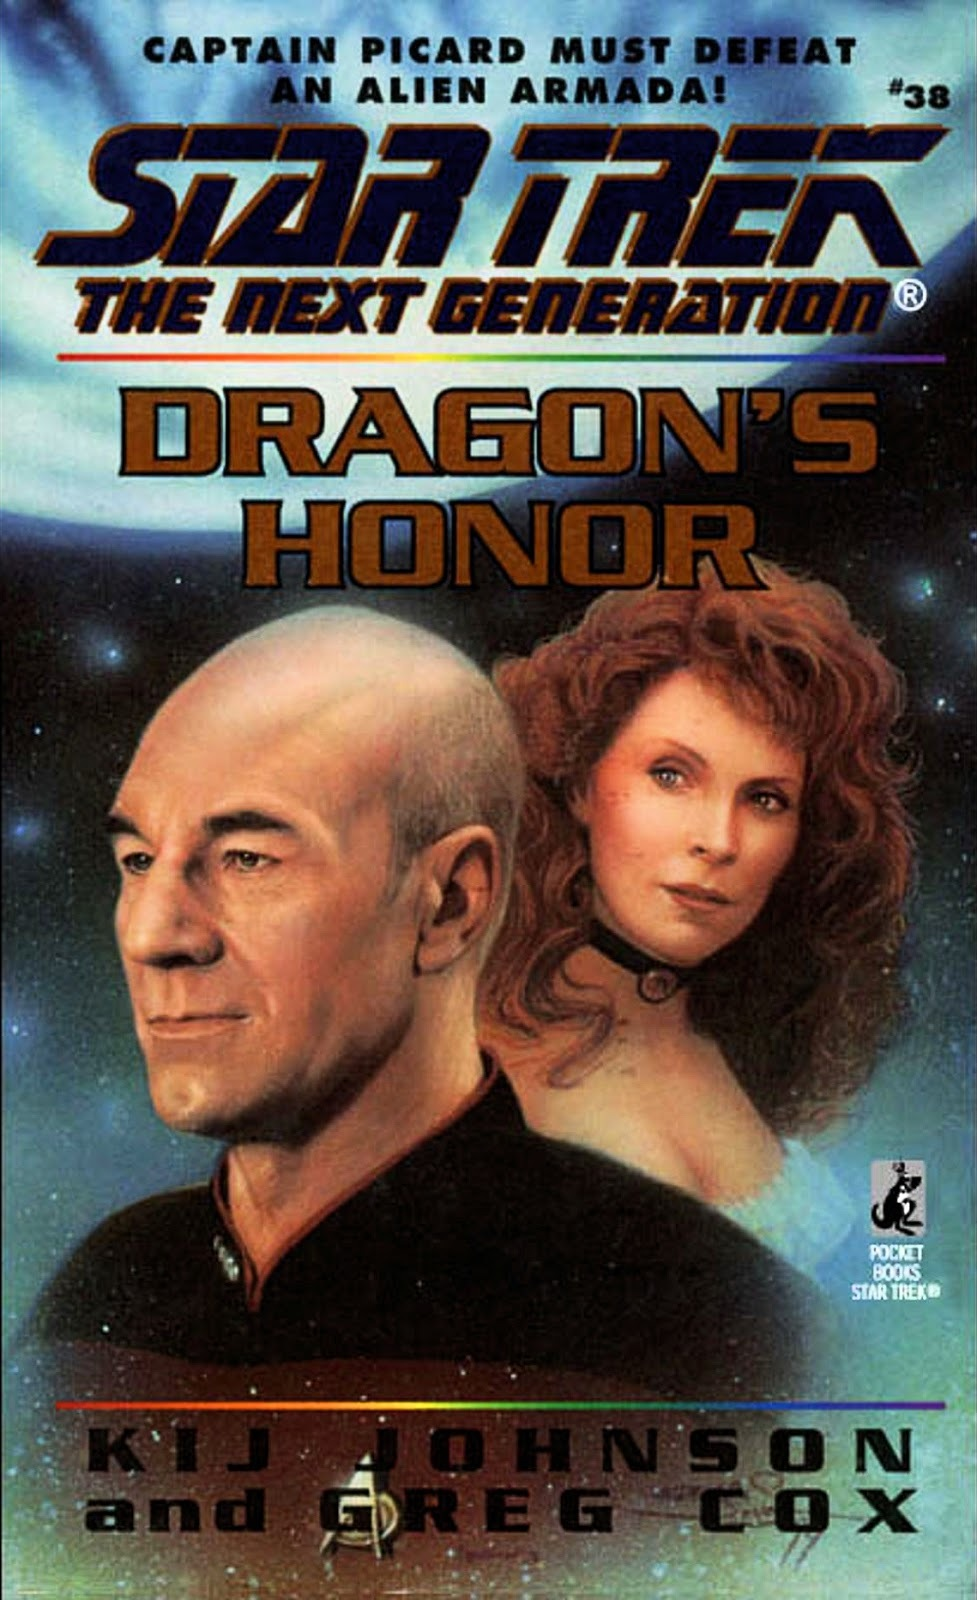}} & \multirow{5}{*}{\textbf{Blurb}:} & Isolated for centuries, the exotic Dragon Empire is finally ready to join the United Federation of Planets. But first the emperor's eldest son must marry the only   \\
 &  & daughter of his oldest enemy, bringing to an end decades of civil war. Without the wedding, there can be no peace -- and no treaty with the Federation.As honored \\
 & & guests of  the  Dragon Empire, Captain Picard and the crew of the "Starship Enterprise" TM must ensure that the royal wedding occurs on schedule, despite the  \\
 & & Empire's complicated and difficult codes of honor. And Dr. Beverly Crusher finds her loyalties torn when she wins the confidence of the unusually reluctant  \\
 & & bride-to-be.  More than just of the Federation. Picard a treaty is at stake, for a vicious race of alien conquerors will stop at nothing, from assassination to invasion,\\
 & &   to keep the Empire out must use all  his skills to save the Empire, and preserve the Dragon's Honor.\\
\cline{2-3}
% & ${\cal{M}}$ & \{"author":"Kij Johnson","publisher":"Star Trek"\}\\ \hline

& \multicolumn{1}{l}{\textbf{Actual Genre}:} & (Fiction, \{Press \& Media, Sci-Fi\})\\ \cline{2-3} %\hline

& \multicolumn{1}{l}{\textbf{Predicted Genre}:} & (Fiction, \{Sci-Fi\})\\

\hline \hline

\rowcolor[HTML]{D9D9D9}
\multicolumn{3}{c}{\textbf{\emph{(b)} 9780380808175: T2: Rising Storm (T2); Author: S.M. Stirling; Publisher: HarperEntertainment}}\\
\hline \hline
& \\ [\dimexpr-\normalbaselineskip+1.5pt]

\multirow{6}{*}{\includegraphics[width=0.08\linewidth]{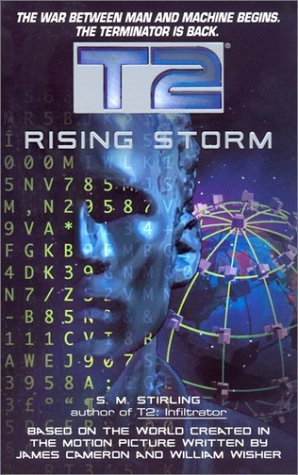}} & \multirow{4}{*}{\textbf{Blurb}:} & \multirow{4}{*}{The war is far from over ... Those who fight for the future face the ultimate challenge ... As the electronic brain behind humanity's destruction comes alive.} \\
 &  & \\
  &  & \\
  &  & \\
\cline{2-3}
% & ${\cal{M}}$ & \{"author":"S.M. Stirling","publisher":"HarperEntertainment"\}\\ \hline

& \multicolumn{1}{l}{\textbf{Actual Genre}:} & (Fiction, \{Mystery \& Thriller \& Suspense \& Horror, Press \& Media, Sci-Fi\})\\ \cline{2-3} %\hline

& \multicolumn{1}{l}{\textbf{Predicted Genre}:} & (Fiction, \{Humanities, Mystery \& Thriller \& Suspense \& Horror, Medical, Sci-Fi\})\\

\hline \hline

\rowcolor[HTML]{D9D9D9}
\multicolumn{3}{c}{\textbf{\emph{(c)} 9781569711293: Star Wars: Battle of the Bounty Hunters; Author: Ryder Windham; Publisher: Dark Horse Comics}}\\
\hline \hline
& \\ [\dimexpr-\normalbaselineskip+1.5pt]

\multirow{6}{*}{\includegraphics[width=0.08\linewidth]{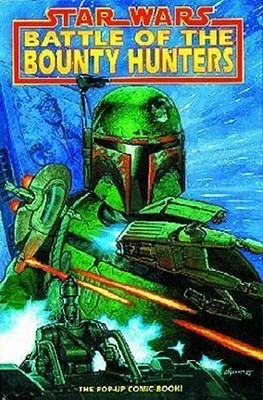}} & \multirow{4}{*}{\textbf{Blurb}:} &  \\
 & & Battle of the Bounty Hunters was a pop-up comic and part of the Star Wars: Shadows of the Empire multimedia campaign. It showed the space battle between \\
 &  &  Boba Fett and IG-88D.\\
 &  &  \\
\cline{2-3}
% & ${\cal{M}}$ & \{"author":"Ryder Windham","publisher":"Dark Horse Comics"\}\\ \hline

& \multicolumn{1}{l}{\textbf{Actual Genre}:} & (Fiction, \{Comics \& Graphic, Press \& Media, Sci-Fi\})\\ \cline{2-3} %\hline

& \multicolumn{1}{l}{\textbf{Predicted Genre}:} & (Fiction, \{Comics \& Graphic, Sci-Fi\})\\ 

\hline \hline

\rowcolor[HTML]{D9D9D9}
\multicolumn{3}{c}{\textbf{\emph{(d)} 9780425051849: 
 Dance of the Tiger; Author: Bjorn Kurten; Publisher: Berkley Publishing Group}}\\
\hline \hline
& \\ [\dimexpr-\normalbaselineskip+1.5pt]

\multirow{6}{*}{\includegraphics[width=0.08\linewidth]{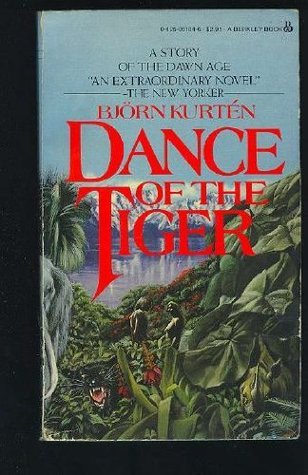}} & \multirow{4}{*}{\textbf{Blurb}:} & \multirow{2}{*}{Björn Kurtén's compelling novel gives the reader a detailed picture of life 35,000 years ago in Western Europe. One of the world's leading scholars of Ice Age}   \\
& & \multirow{2}{*}{fauna, Kurtén fuses extraordinary knowledge and imagination in this vivid evocation of our deepest past. This novel illuminates the lives of the humans who left}    \\ 
& & \multirow{2}{*}{us magnificent paintings in the caves of France and Spain.} \\ 
& & \\ \cline{2-3}

% & ${\cal{M}}$ & \{"author":"Bjorn Kurten","publisher":"Berkley Publishing Group"\}\\ \hline
& \multicolumn{1}{l}{\textbf{Actual Genre}:} & (Fiction, \{History, Humanities, Sci-Fi\})\\ \cline{2-3} %\hline

& \multicolumn{1}{l}{\textbf{Predicted Genre}:} & (Fiction, \{Environment \& Plant, History, Literature, Travel, Sci-Fi\})\\

\hline \hline

\rowcolor[HTML]{D9D9D9}
\multicolumn{3}{c}{\textbf{\emph{(e)} 9780789425225: Voices in the Park; Author: Anthony Browne; Publisher: Dorling Kindersley Publishing}}\\
\hline \hline
& \\ [\dimexpr-\normalbaselineskip+1.5pt]

\multirow{5}{*}{\includegraphics[width=0.08\linewidth]{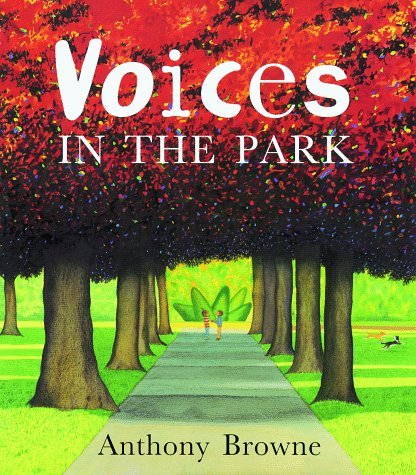}} & \multirow{3}{*}{\textbf{Blurb}:} & \multirow{2}{*}{Four people enter a park and through their eyes young readers see different visions, from the bossy woman and the sad man to the lonely boy and the warm young} \\

 &  &  \multirow{2}{*}{girl, moving from one voice to another and shifting landscapes and seasons.} \\

  &  & \\

\cline{2-3}
% & ${\cal{M}}$ & \{"author":"Anthony Browne","publisher":"Dorling Kindersley Publishing"\}\\ \hline
& \multicolumn{1}{l}{\textbf{Actual Genre}:} & (Fiction, \{Animals \& Wildlife \& Pets, Arts \& Photography, {Childrens\textquoteright} Book, Family \& Parenting \& Relationships, Teen \& Young Adult\})\\ \cline{2-3} %\hline

& \multicolumn{1}{l}{\textbf{Predicted Genre}:} & (Fiction, \{Arts \& Photography, {Childrens\textquoteright} Book, Family \& Parenting \& Relationships, Teen \& Young Adult\})\\ %\hline

\hline \hline

\rowcolor[HTML]{D9D9D9}
\multicolumn{3}{c}{\textbf{\emph{(f)} 9780894712661: The Classic Tale of Velveteen Rabbit or How Toys Become Real; Author: Margery Williams; Publisher: Running Press}}\\
\hline \hline
& \\ [\dimexpr-\normalbaselineskip+1.5pt]

\multirow{5}{*}{\includegraphics[width=0.08\linewidth]{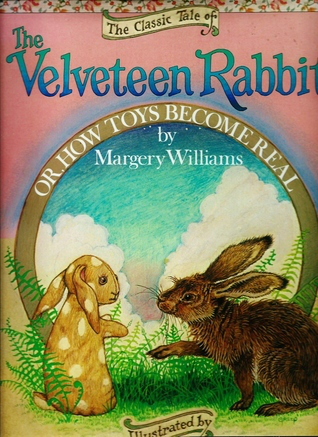}} & \multirow{3}{*}{\textbf{Blurb}:} & \multirow{2}{*}{A beautiful large-format edition of this timeless children's tale, replete with enchanting full-color illustrations. A charming fable with the moral that love can make} \\
& & \multirow{2}{*}{all things real and beautiful. 10" x 13".}\\ 
& & \\ \cline{2-3}

% & ${\cal{M}}$ & \{"author":"Margery Williams","publisher":"Courage Books"\}\\ \hline
& \multicolumn{1}{l}{\textbf{Actual Genre}:} & (Fiction, \{Animals \& Wildlife \& Pets, Arts \& Photography, {Childrens\textquoteright} Book, Literature, Sci-Fi, Teen \& Young Adult\})\\ \cline{2-3} %\hline

& \multicolumn{1}{l}{\textbf{Predicted Genre}:} & (Fiction, \{Arts \& Photography, {Childrens\textquoteright} Book, Literature, Mythology \& Religion \& Spirituality, Teen \& Young Adult, Sci-Fi\})\\
% \hline

\hline \hline

\rowcolor[HTML]{D9D9D9}
\multicolumn{3}{c}{\textbf{\emph{(g)} 9780440436836: Homesick: My Own Story; Author: Jean Fritz; Publisher: Yearling Books}}\\
\hline \hline
& \\ [\dimexpr-\normalbaselineskip+1.5pt]

\multirow{8}{*}{\includegraphics[width=0.08\linewidth]{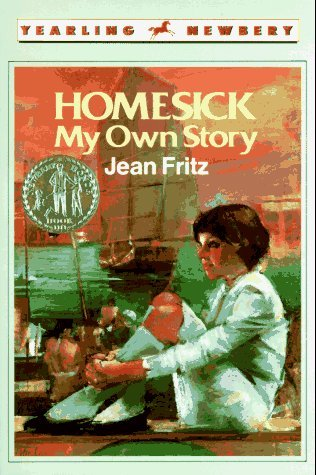}} & \multirow{6}{*}{\textbf{Blurb}:} & Jean Fritz was born in China and lived there until 1927, when she was twelve. Young Jean had spent her entire life in China, but her parents' memories of home  \\
 &  & and letters from relatives in  Pennsylvania made her feel that she was American--and homesick for a place she'd never seen!Family photographs and illustrations   \\
 & &  by Margot Tomes show us the real people behind Jean's vivid and unforgettable stories--memories of picnics on the Great Wall, pranks, holidays in the foreign \\
 & &  compound, rebellious moments at her British school. close ties to Chinese friends, and how it felt to be called a "foreign devil" and spat upon in the streets of \\
 & &  a turbulent China on the eve of revolution. When her family embarks upon its long journey home, Jean is thrilled, but she When she arrives in America at last,  \\
  & & will she fit in after growing up on "the wrong side of the world?" \\
 
\cline{2-3}
% & ${\cal{M}}$ & \{"author":"Jean Fritz","publisher":"Yearling Books"\}\\ \hline
& \multicolumn{1}{l}{\textbf{Actual Genre}:} & (Non-fiction, \{Biographies \& Memoir, {Childrens\textquoteright} Book, History, Teen \& Young Adult\})\\ \cline{2-3} %\hline

& \multicolumn{1}{l}{\textbf{Predicted Genre}:} & (Non-fiction, \{{Childrens\textquoteright} Book, History, Biographies \& Memoir\})\\ %\hline

\hline \hline

\rowcolor[HTML]{D9D9D9}
\multicolumn{3}{c}{\textbf{\emph{(h)} 9780345291363: Elephant Man; Author: Christine Sparks; Publisher: Ballantine Books}}\\
\hline \hline
& \\ [\dimexpr-\normalbaselineskip+1.5pt]

\multirow{7}{*}{\includegraphics[width=0.08\linewidth]{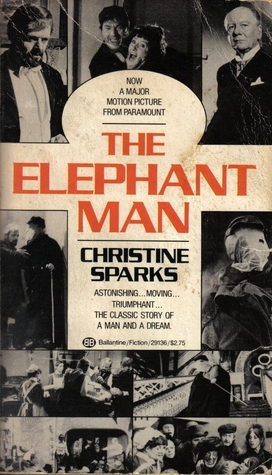}} & \multirow{5}{*}{\textbf{Blurb}:} &  \\
& & John Merrick had lived for more than twenty years imprisoned in a body that condemned him to a miserable life in the workhouse and to humiliation as a circus   \\
 &  & sideshow freak. But beneath  that tragic exterior, within that enormous and deformed head, thrived the soul of a poet, the heart of a dreamer, the longings of a    \\
 & &  man. Based on the extraordinary motion picture that captured the heart of America.\\
  & & \\
 
\cline{2-3}
% & ${\cal{M}}$ & \{"author":"Christine Sparks","publisher":"Ballantine Books"\}\\ \hline
& \multicolumn{1}{l}{\textbf{Actual Genre}:} & (Non-fiction, \{Biographies \& Memoir, History, Literature, Teen \& Young Adult\})\\ \cline{2-3} %\hline

& \multicolumn{1}{l}{\textbf{Predicted Genre}:} & (Non-fiction, \{History, Literature, Biographies \& Memoir\})\\ \hline

\end{tabular}
\end{adjustbox}

\label{tab:indistinguish_sample}

\end{table*}

\begin{table*}[!hbt]
\centering
\caption{Misprediction due to Level-1 classification}
\begin{adjustbox}{width=0.95\textwidth}
% \begin{adjustbox}{angle=90, height=1\textheight}
% \footnotesize
\begin{tabular}{c|ll}%p{0.9\textwidth}}
% \multicolumn{3}{c}{(a) Samples for heatmap analysis}\\

\hline \hline
\rowcolor[HTML]{D9D9D9}
\multicolumn{3}{c}{\textbf{{\emph{(a)}} 9780312266820: Dead Egotistical Morons: A Paul Turner Mystery; Author: Mark Richard Zubro; Publisher: St. Martin's Press}}\\
\hline \hline

\multirow{11}{*}{\includegraphics[width=0.1\linewidth]{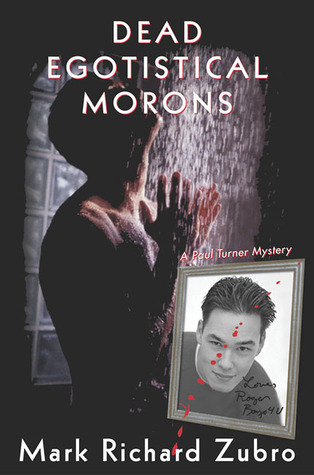}} & \multirow{8}{*}{\textbf{Blurb}:} & Boys4U is the world's most popular singing group - at least among teenaged girls - and they have closed out their sold-out world tour with a series of shows \\
& &   in Chicago's brand new arena. The premier group of the inexplicably popular "boy band" trend, they've just finished their very last concert of the tour. While  \\
& & hundreds of tour members, well-wishers, executives, and various hangers on wait to celebrate another wildly successful tour, the lead singer is found murdered  \\
& &   - shot in the back of the head at close range - in the shower all times, the only other people back there were the other members of the band, and  none of the \\
& &   dozens of people in the next room report having heard a shot. While the international press is engaged of the backstage dressing area. To make matters more    \\
& & distressing, the crime itself was almost impossible - there was tight security on the shower area at in an unprecedented feeding frenzy over the sensationalistic \\
& & murder, Chicago Police Detectives Paul Turner and his partner Buck Fenwick have pulled the unenviable task of investigating the murder But even the initial \\
& &  appearances are deceiving and as they dig deeper into the case, they uncover more disturbing truths beneath the wholesome façade of Boys4U. Now they have \\
& &  untangle an increasingly complex web if they are to stop a determined killer before more victims are claimed. \\
\cline{2-3}

% & ${\cal{M}}$ & \{"author":"Mark Richard Zubro","publisher":"St. Martin's Press"\}\\ \hline

& \multicolumn{1}{l}{\textbf{Actaul Genre}:} & (Fiction, \{Fashion \& Lifestyle, Mystery \& Thriller \& Suspense \& Horror\})\\ \cline{2-3} %\hline
& \multicolumn{1}{l}{\textbf{Predicted Genre}:} & (Non-fiction, \{Arts \& Photography\}) \\

\hline \hline
\rowcolor[HTML]{D9D9D9}
\multicolumn{3}{c}{\textbf{{\emph{(b)}} 9780312979256: Mafia Marriage; Author: Rosalie Bonanno; Publisher: St. Martin's Paperbacks}}\\
\hline \hline

\multirow{9}{*}{\includegraphics[width=0.08\linewidth]{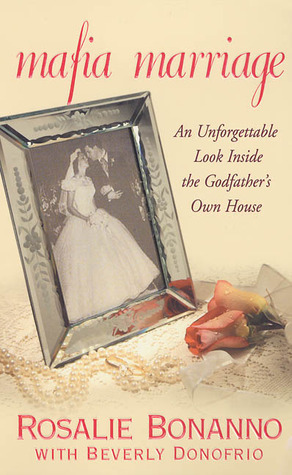}} & \multirow{6}{*}{\textbf{Blurb}:} & An Unforgettable Look Inside the Godfather's Own HouseShe Was A Profaci. He Was A BonannoRosalie Profaci was a Mafia princess. Salvatore "Bill" \\
& &   Bonanno, oldest son of   Mafia Don Joe Bonanno, the real-life model for The Godfather, was organized crime's crown prince. And Bill, deeply involved in his \\
& &   father's "business" of mob schemes thought  pretty Rosalie knew what it meant to be a "Mafia wife." But the convent-raised, deeply devout Rosalie, whose \\
& &   innocence was protected by her doting father, had no idea...Their  Marriage United Two Mafia Dynasties...Mafia Marriage is Rosalie Bonanno's intimate \\
& &  account of life inside the secretive world of the Mafia. Naming names and providing shocking details, she writes about the wild spending sprees, the \\
& &   mysterious absences of her husband, the other women in his-their running from the law, the abductions, and shootings. Above all, Rosalie reveals the passion\\
& &  that kept her virtually a prisoner to love...and her heartbreaking journey of discovering the truth and trying to break free. \\

\cline{2-3}

% & ${\cal{M}}$ & \{"author":"Rosalie Bonanno","publisher":"St. Martin's Paperbacks"\}\\ \hline

& \multicolumn{1}{l}{\textbf{Actaul Genre}:} & (Non-fiction, \{Biographies \& Memoir, Mystery \& Thriller \& Suspense \& Horror\})\\ \cline{2-3} %\hline
& \multicolumn{1}{l}{\textbf{Predicted Genre}:} & (Fiction, \{History, Romance, Teen \& Young Adult\}) \\

\hline

% \multicolumn{3}{r}{${\cal{I}}$: Coverpage Image, ${\cal{T}}$: Description Text, ${\cal{M}}$: Metadata}
\end{tabular}
\end{adjustbox}

\label{tab:model_limitation}

\end{table*}

% \clearpage

\subsection{Quantitative and Qualitative Analysis for Genre Indistinguishability}
\noindent
Our investigation into misclassification suggests that the genre co-occurrence might be a contributing factor. Table \ref{tab:misclassification_fiction}: (a) and \ref{tab:misclassification_non_fiction}: (a) present pair-wise genre sample count for \textit{fiction} and \textit{non-fiction} genre in ${\cal{D}}_{train}$. Each cell in the table represents the number of samples belonging to both the row and column genre class ids. Table \ref{tab:misclassification_fiction}: (b) and \ref{tab:misclassification_non_fiction}: (b) illustrates the co-occurrence ratio between row class ID $i$ in association with column class ID $j$ for \textit{fiction} and \textit{non-fiction} genres respectively. Each cell contains the ratio of samples belonging to both class ids $i$ and $j$ to the total number of training samples associated with class ID $j$. Table \ref{tab:misclassification_fiction}: (c) and \ref{tab:misclassification_non_fiction}: (c) reports the misclassification rate by IMAGINE for \textit{fiction} and \textit{non-fiction} genres, respectively. Here, each cell corresponding to row class ID $i$ and column class ID $j$ represents the ratio between the number of testing samples associated with class ID $j$ but wrongly identified as class ID $i$ and the total number of testing samples associated with class ID $j$ that have been misclassified.

Our analysis of Table \ref{tab:misclassification_fiction} and \ref{tab:misclassification_non_fiction} suggest that the high co-occurrence of the two genres,  coupled with a significant imbalance in the number of training samples associated with one genre without the other, potentially causes the high misclassification rate. For instance, in Table \ref{tab:misclassification_fiction}, 264 out of 396 \textit{Press \& Media} (class ID 21) books are associated with \textit{Sci-Fi} (class ID 29) genre (refer to Table \ref{tab:misclassification_fiction}: (a)). This leaves only 132 samples that are not categorized as \textit{Sci-Fi}. Conversely, there are 3716 \textit{Sci-Fi} books that do not belong to the \textit{Press \& Media} genre, creating imbalance between non-Sci-Fi \textit{Press \& Media} and non-Press \& Media
\textit{Sci-Fi} samples. This leads to \textit{Press \& Media} genre being misclassified as \textit{Sci-Fi} with the misclassification rate of 0.79. Standard data augmentation methods are limited in their ability to address this imbalance issue, as increasing in the number of samples for \textit{Press \& Media} genre, also increases the \textit{Sci-Fi} samples due to inter-genre relation. We observe similar issue between \textit{Humanities} (class ID 14) and \textit{Literature} (class ID 16) (refer Table \ref{tab:misclassification_fiction}),  \textit{Animals \& Wildlife \& Pets} (class ID 1) and \textit{{Childrens\textquoteright} Book} (class ID 4) (refer Table \ref{tab:misclassification_fiction}), and \textit{non-fiction} genres \textit{Teen \& Young Adult} (class ID 27) and \textit{History} (class ID 13) (refer Table \ref{tab:misclassification_non_fiction}). As a result, relatively lower ${\cal{BA}}$ than other genre was observed for \textit{Press \& Media}, \textit{Humanities}, \textit{Animals \& Wildlife \& Pets} in Table \ref{tab:genrewise_analysis}: (a) and \textit{Teen \& Young Adult} in Table \ref{tab:genrewise_analysis}: (b). 

Table \ref{tab:indistinguish_sample} showcases the example of misclassified data samples due to genre indistinguishability. Here, samples [Table \ref{tab:misclassification_fiction}: \emph{(a)-(c)}] contains \textit{Press \& Media} and \textit{Sci-Fi} as actual genre but IMAGINE can only predict \textit{Sci-Fi }. As mentioned above, it is caused by a high imbalance between non-Sci-Fi \textit{Press \& Media} and non-Press \& Media \textit{Sci-Fi}. Similarly, [\ref{tab:misclassification_fiction}: \emph{(d)}], [\ref{tab:misclassification_fiction}: \emph{(e), (f)}] and [\ref{tab:misclassification_fiction}: \emph{(g), (h)}] show the imbalance between [non-Humanities \textit{Literature} and non-Literature \textit{Humanities}], [non-Animals \& Wildlife \& Pets \textit{{Childrens\textquoteright} Book} and non-{Childrens\textquoteright} Book  \textit{Animals \& Wildlife \& Pets}], respectively.

% \emph{(ii) Qualitative Analysis for Genre Indistinguishability:} Table \ref{tab:indistinguish_sample} showcases the example of misclassified data samples due to genre indistinguishability. As mentioned in appendix \ref{app:analysis_misprediction}.\emph{(i)} and Table \ref{tab:misclassification_fiction},   

\subsection{Qualitative Analysis of Model Limitation:} 
Another significant reason for IMAGINE's mispredictions is the inherent limitations of the model. From Table \ref{tab:model_limitation}, we observe genre misprediction in Level-2 classification due to misclassification in Level-1 classification for some samples (e.g., Table \ref{tab:model_limitation}:  \emph{(a)}). This analysis shows the area of improvement in Level-1 classification to enhance the overall performance of the model.
