# Supplementary material for: Adaptive Data-Resilient Multi-Modal Hierarchical Multi-Label Book Genre Identification
Source: arXiv:2505.03839 source file (2025-10-18)
Supplement: Supplementary file 2 [file 7_appendix_experiment_settings.tex]

\section{Experimental Settings}
\label{app:experimental_settings}
\noindent
Table \ref{tab:settings} provides detailed experimental settings for each training stage. 
\begin{table}[!hbt]
\centering

\caption{Experimental settings details}
\begin{adjustbox}{width=0.4\textwidth} 
\begin{tabular}{c|l}
% \hline
% \multicolumn{2}{c}{System settings} \\ \hline

% Operating system & Ubuntu 20.04.4 LTS \\
% Processor & Intel(R) Xeon(R) W-1270 (3.40GHz, 16 cores) \\
% Ram & 128 GB \\
% GPU & NVIDIA RTX A5000 (24GB) \\
% Environment & Python 3.10.14, PyTorch 2.1.0 \\

\hline
\multicolumn{2}{c}{Knowledge graph embedding settings} \\
\hline

Tool & OpenKE Toolkit \\
No. of epochs & 500 \\
Batch size & 100 \\
Learning rate & $10^{-3}$ \\
Optimizer & Adam \\

\hline
\multicolumn{2}{c}{Level-1 and Level-2 classification settings} \\
\hline

No. of epochs (Level-1 classification) & 50 \\
No. of epochs (Level-2 classification) & 100 \\
Batch size & 16 \\
Learning rate & $10^{-5}$ \\
Weight decay & $10^{-2}$ \\
Exponential decay rates & $\beta_1$ = 0.9, $\beta_2$ = 0.999 \\
Zero-denominator avoidance parameter & $10^{-8}$ \\
Optimizer & AdamW \\
Patience & 5 \\

\hline
\multicolumn{2}{c}{Classifier selector settings} \\
\hline

No. of epochs & 100 \\
Batch size & 16 \\
Learning rate & $10^{-3}$ \\
Weight decay & $10^{-2}$ \\
Exponential decay rates & $\beta_1$ = 0.9, $\beta_2$ = 0.999 \\
Zero-denominator avoidance parameter & $10^{-8}$ \\
Optimizer & AdamW \\
Patience & 5 \\
\hline
\end{tabular}
\label{tab:settings}
\end{adjustbox}
\end{table}
