# Supplementary material for: Adaptive Data-Resilient Multi-Modal Hierarchical Multi-Label Book Genre Identification
Source: arXiv:2505.03839 source file (2025-10-18)
Supplement: Supplementary file 3 [file 7appendix_cooccurrence.tex]

\section{Genre Co-occurrence matrix}
\label{app:cooccurrence}

\begin{figure*}[!t]
    \centering
    (a) \includegraphics[width=0.45\linewidth]{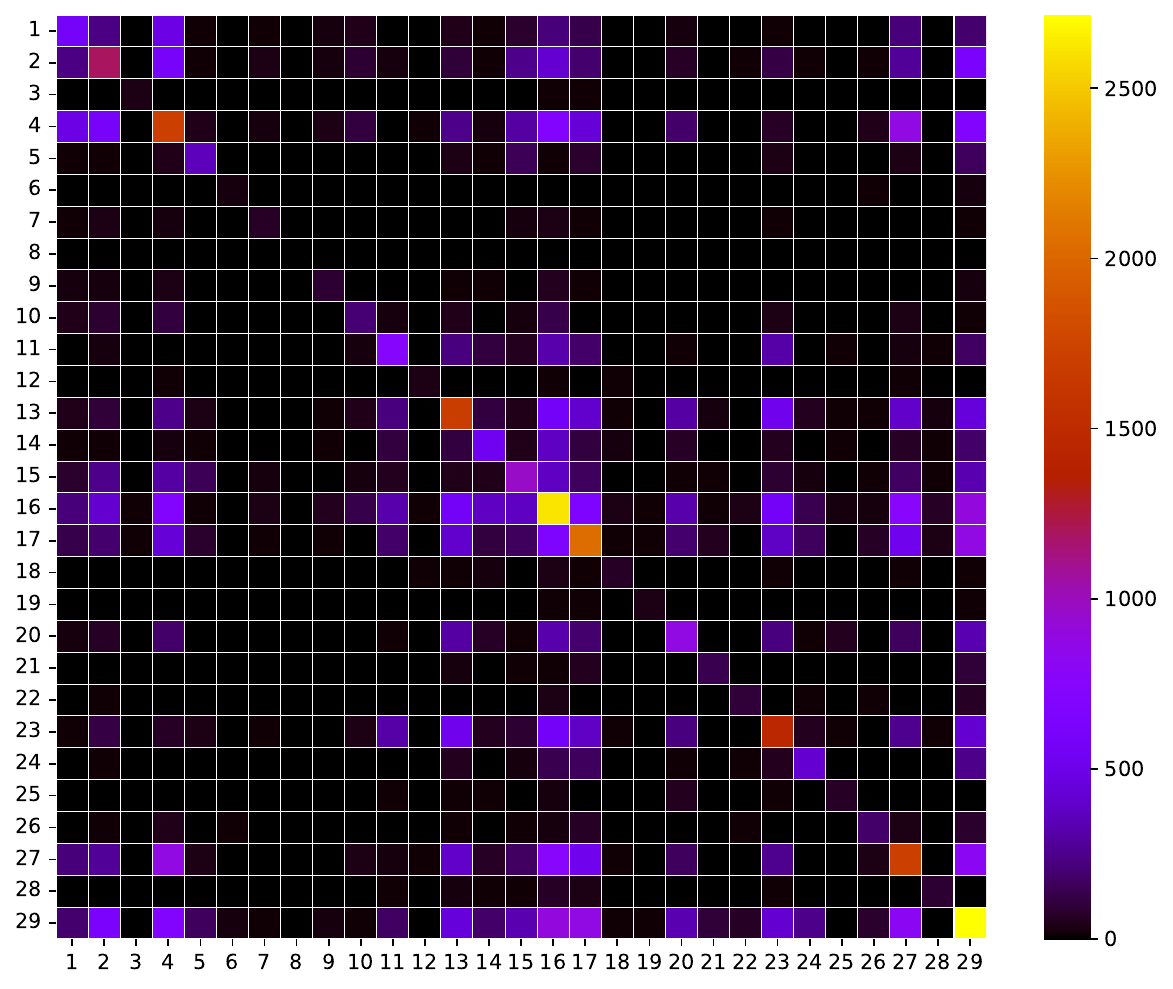}
    (b) \includegraphics[width=0.45\linewidth]{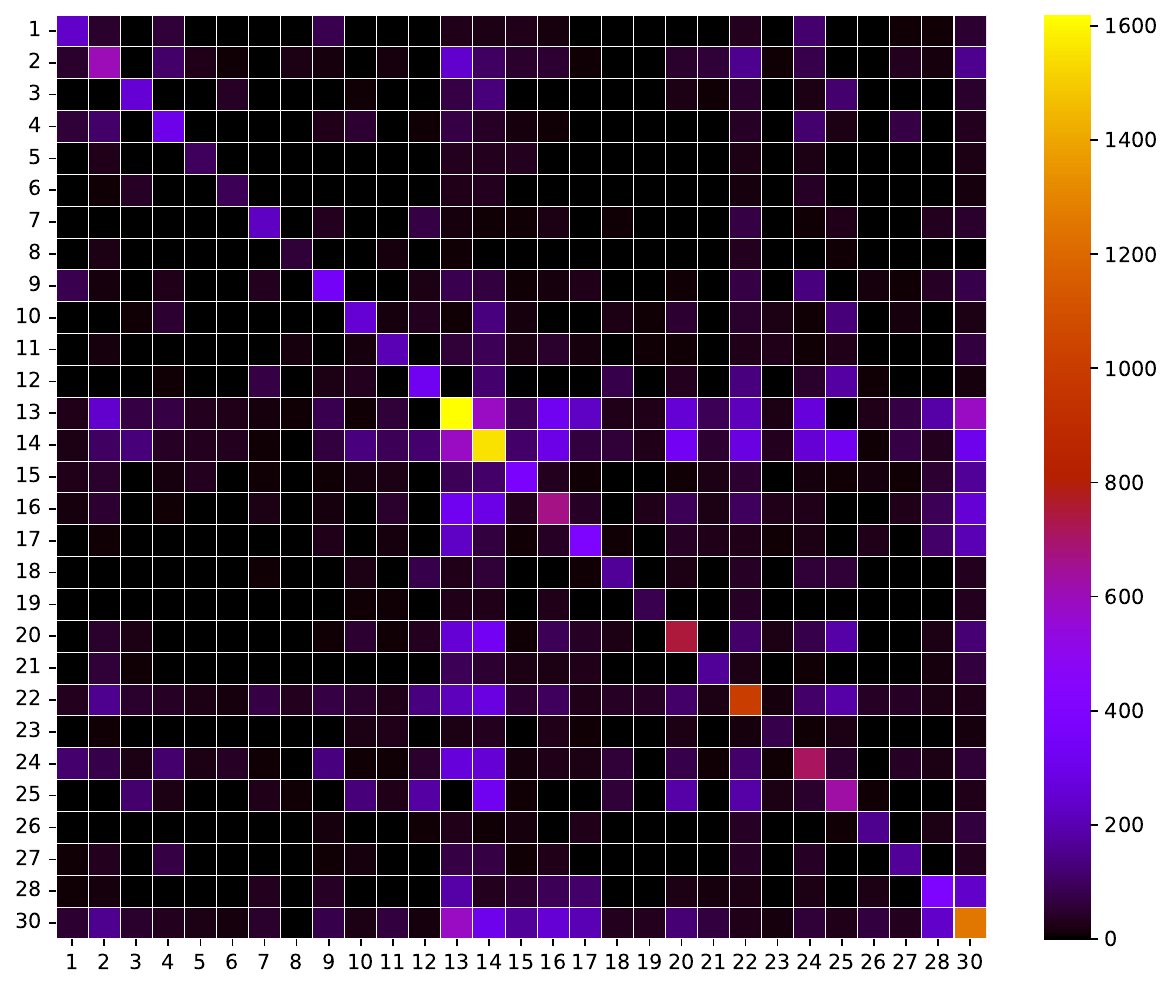}
    \caption{Co-occurrence matrices for book genres: (a) \textit{fiction}, (b) \textit{non-fiction}}
    \label{fig:f_nf_cooccurrence}
\end{figure*}

\noindent 
Fig.s \ref{fig:f_nf_cooccurrence}: (a), (b) visually depict the relationships and co-occurrence patterns among book \textit{fiction} and \textit{non-fiction} genres.

% \begin{figure}[!h]
%     \centering
%     \includegraphics[width=1\linewidth]{figs/co_occurrence_matrix/fiction_heatmap.pdf}
%     \caption{Co-occurrence matrix for book \textit{fiction} genre}
%     \label{fig:fiction_cooccurrence}
% \end{figure}

% \begin{figure}[!h]
%     \centering
%     \includegraphics[width=1\linewidth]{figs/co_occurrence_matrix/nonfiction_heatmap.pdf}
%     \caption{Co-occurrence matrix for book \textit{non-fiction} genre}
%     \label{fig:non_fiction_cooccurrence}
% \end{figure}
