# Supplementary material for: Adaptive Data-Resilient Multi-Modal Hierarchical Multi-Label Book Genre Identification
Source: arXiv:2505.03839 source file (2025-10-18)
Supplement: Supplementary file 4 [file 7appendix_data_challenges.tex]

\section{Dataset Challenges} 
\label{app:dataset_challenge}

\begin{figure*}[t]
\centering
\footnotesize
\makebox[\textwidth][c]{
\begin{adjustbox}{width=\linewidth}
\begin{tabular}{c|c|c|c || c|c|c|c}
%%%%%%%%%%%%%%%
\hline 
&&& &&&&  \\[\dimexpr-\normalbaselineskip+1.5pt]
\includegraphics[width=0.1\linewidth, height=0.145\linewidth]{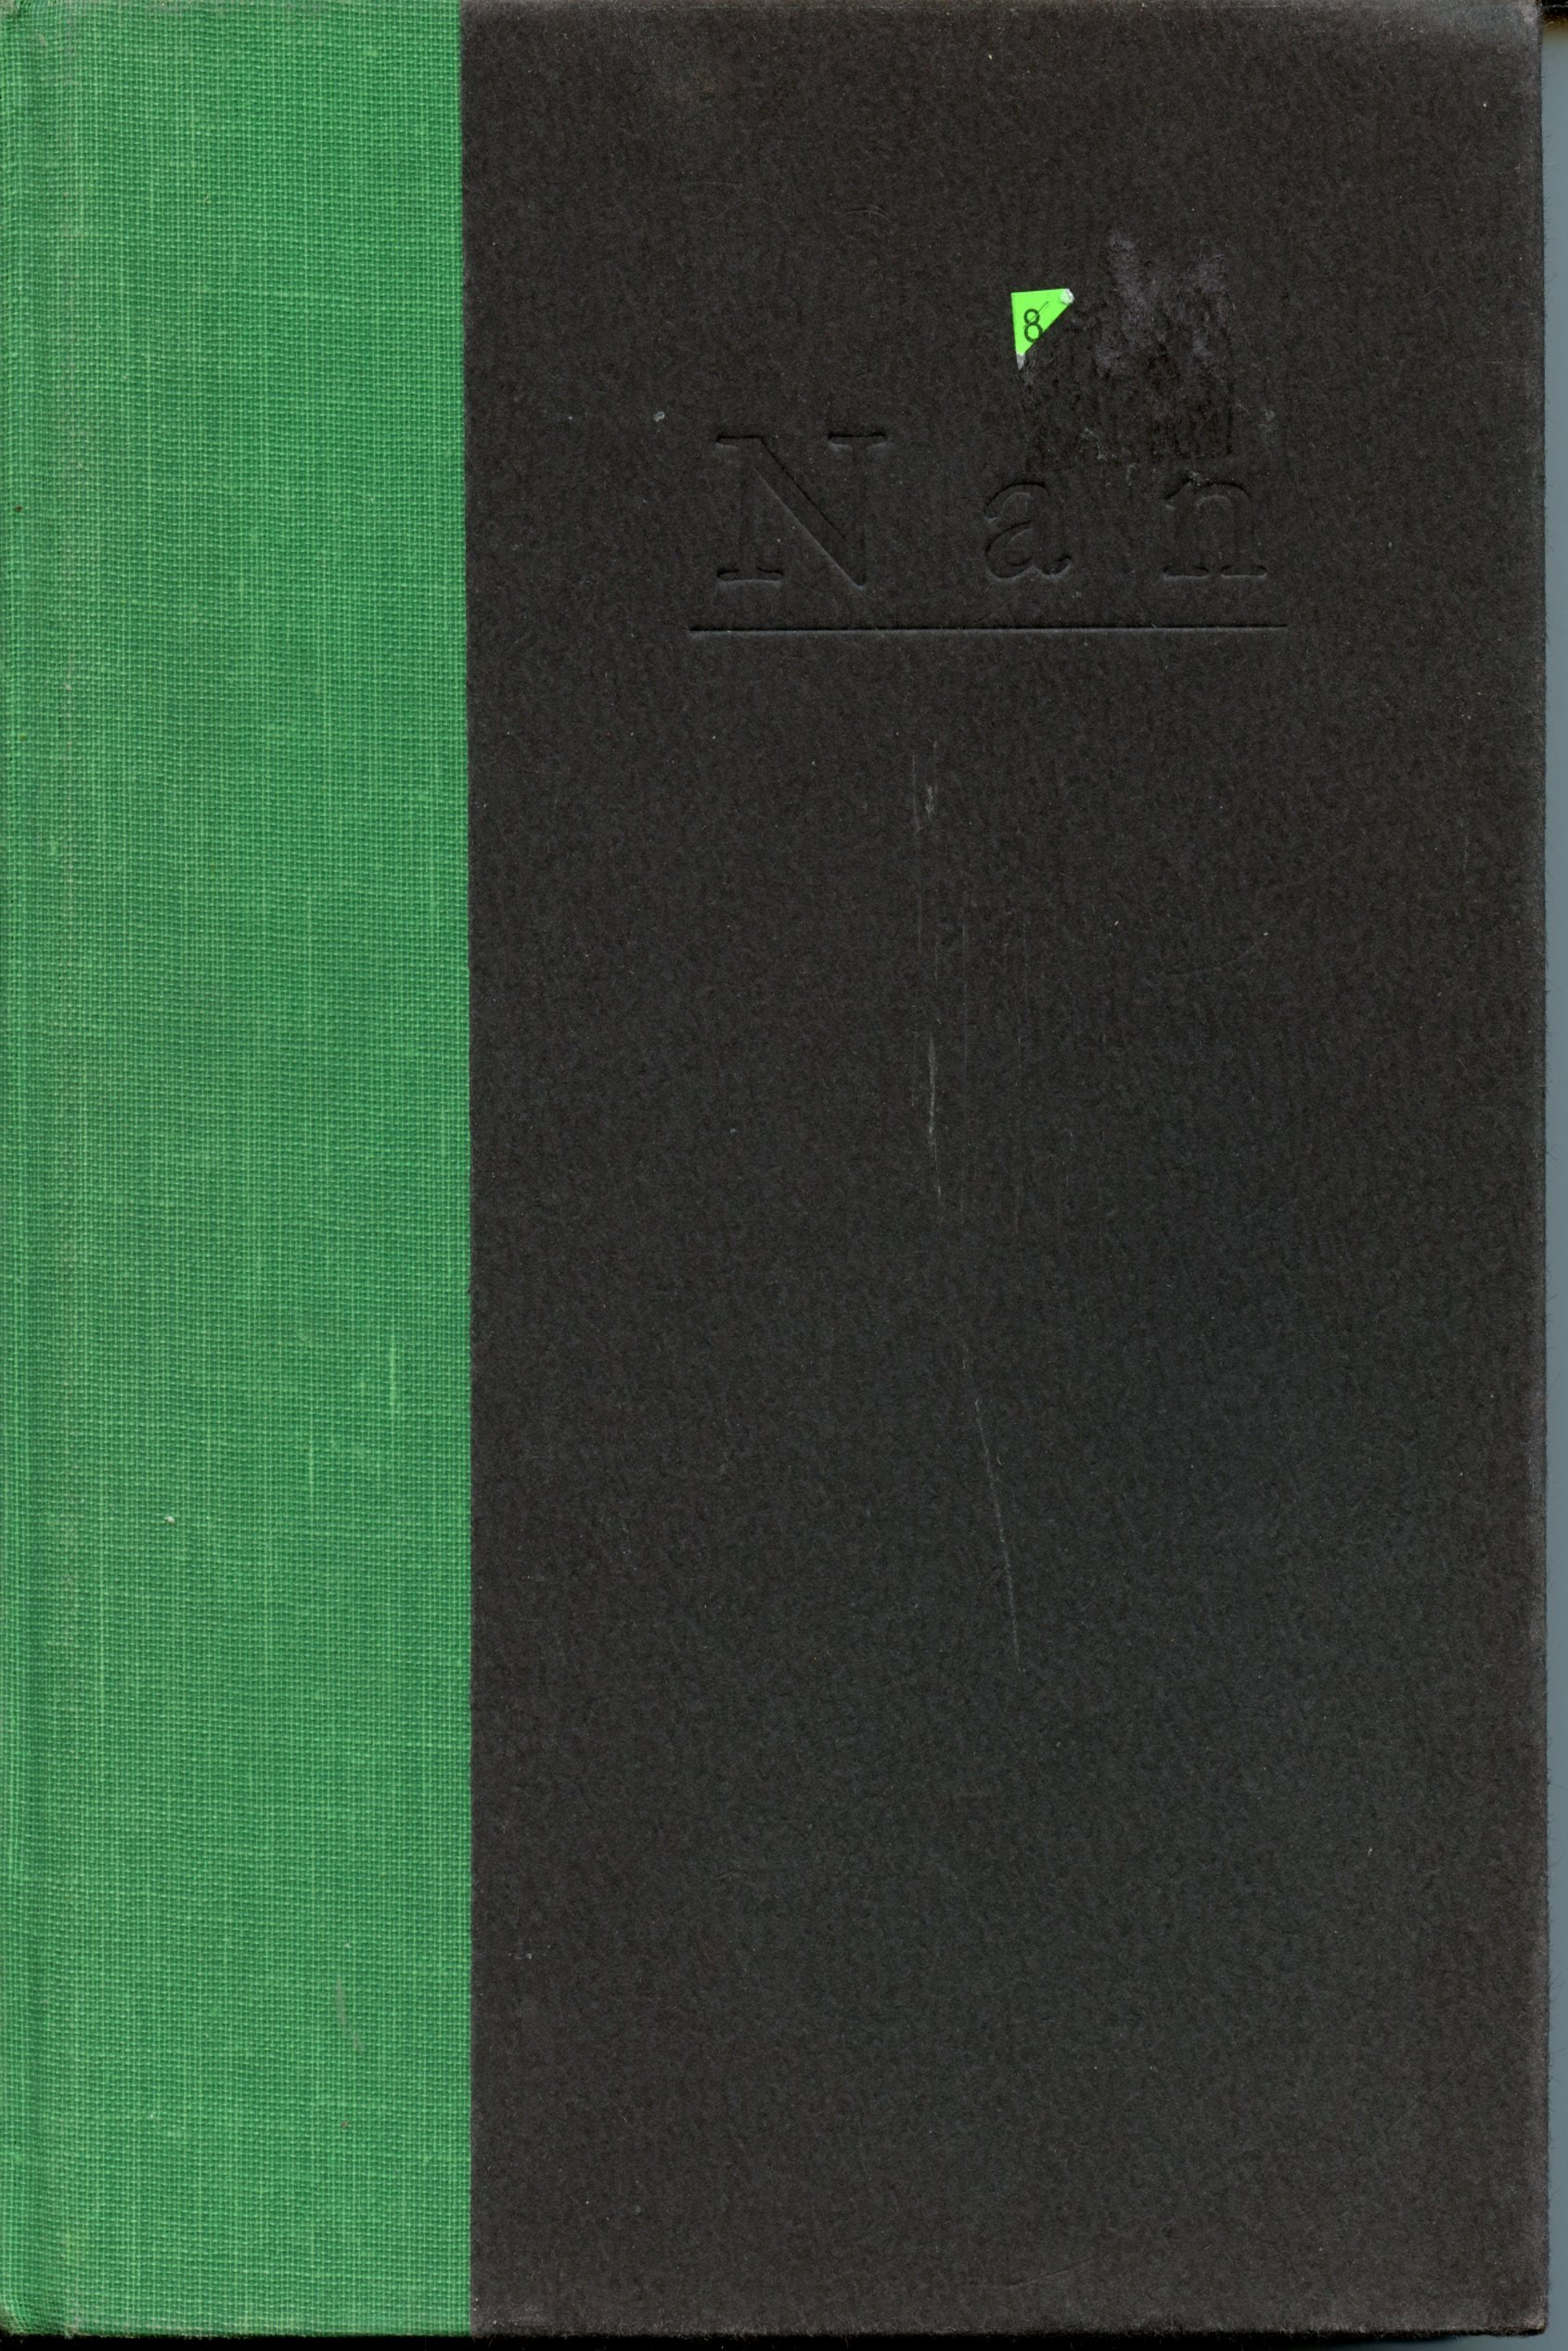} & 
\includegraphics[width=0.1\linewidth, height=0.145\linewidth]{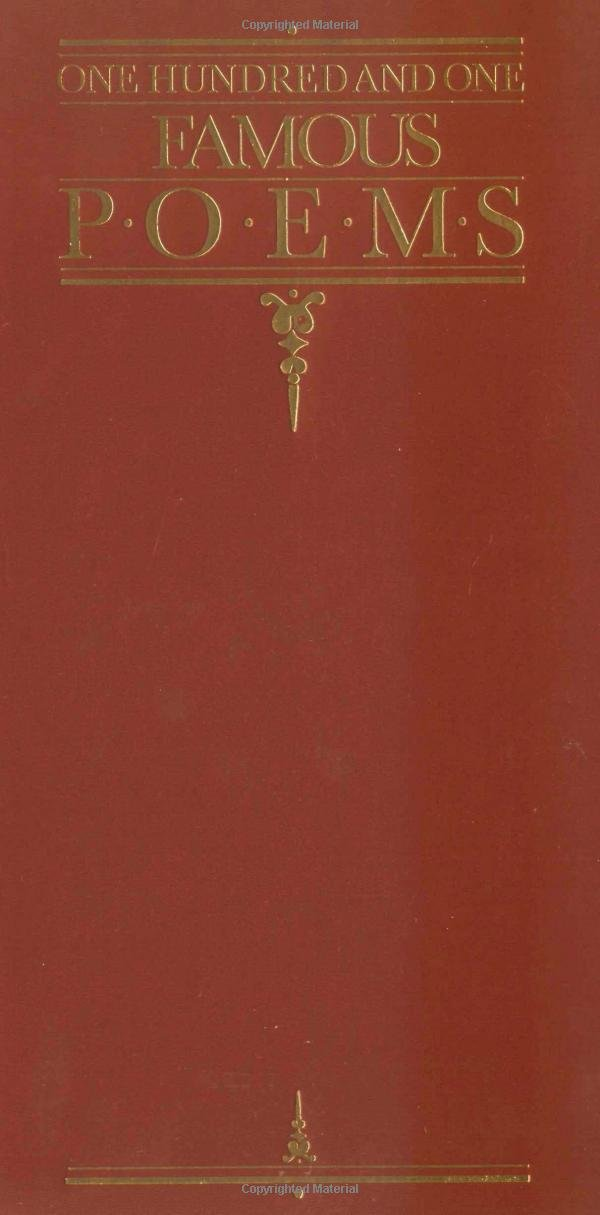} & 
\includegraphics[width=0.1\linewidth, height=0.145\linewidth]{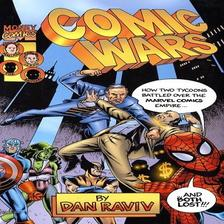} & 
\includegraphics[width=0.1\linewidth, height=0.145\linewidth]{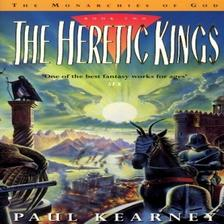} &
\includegraphics[width=0.1\linewidth, height=0.145\linewidth]{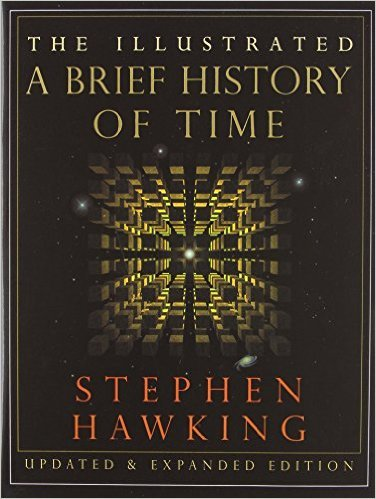} & 
\includegraphics[width=0.1\linewidth, height=0.145\linewidth]{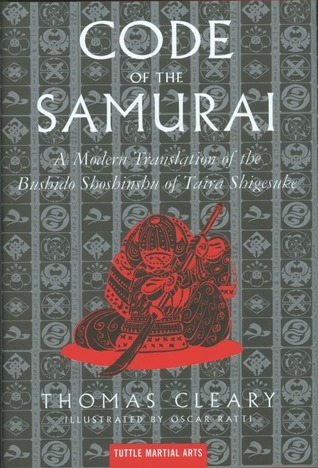} &
\includegraphics[width=0.1\linewidth, height=0.145\linewidth]{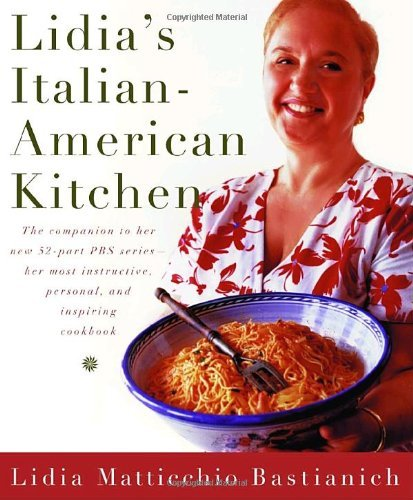} & 
\includegraphics[width=0.1\linewidth, height=0.145\linewidth]{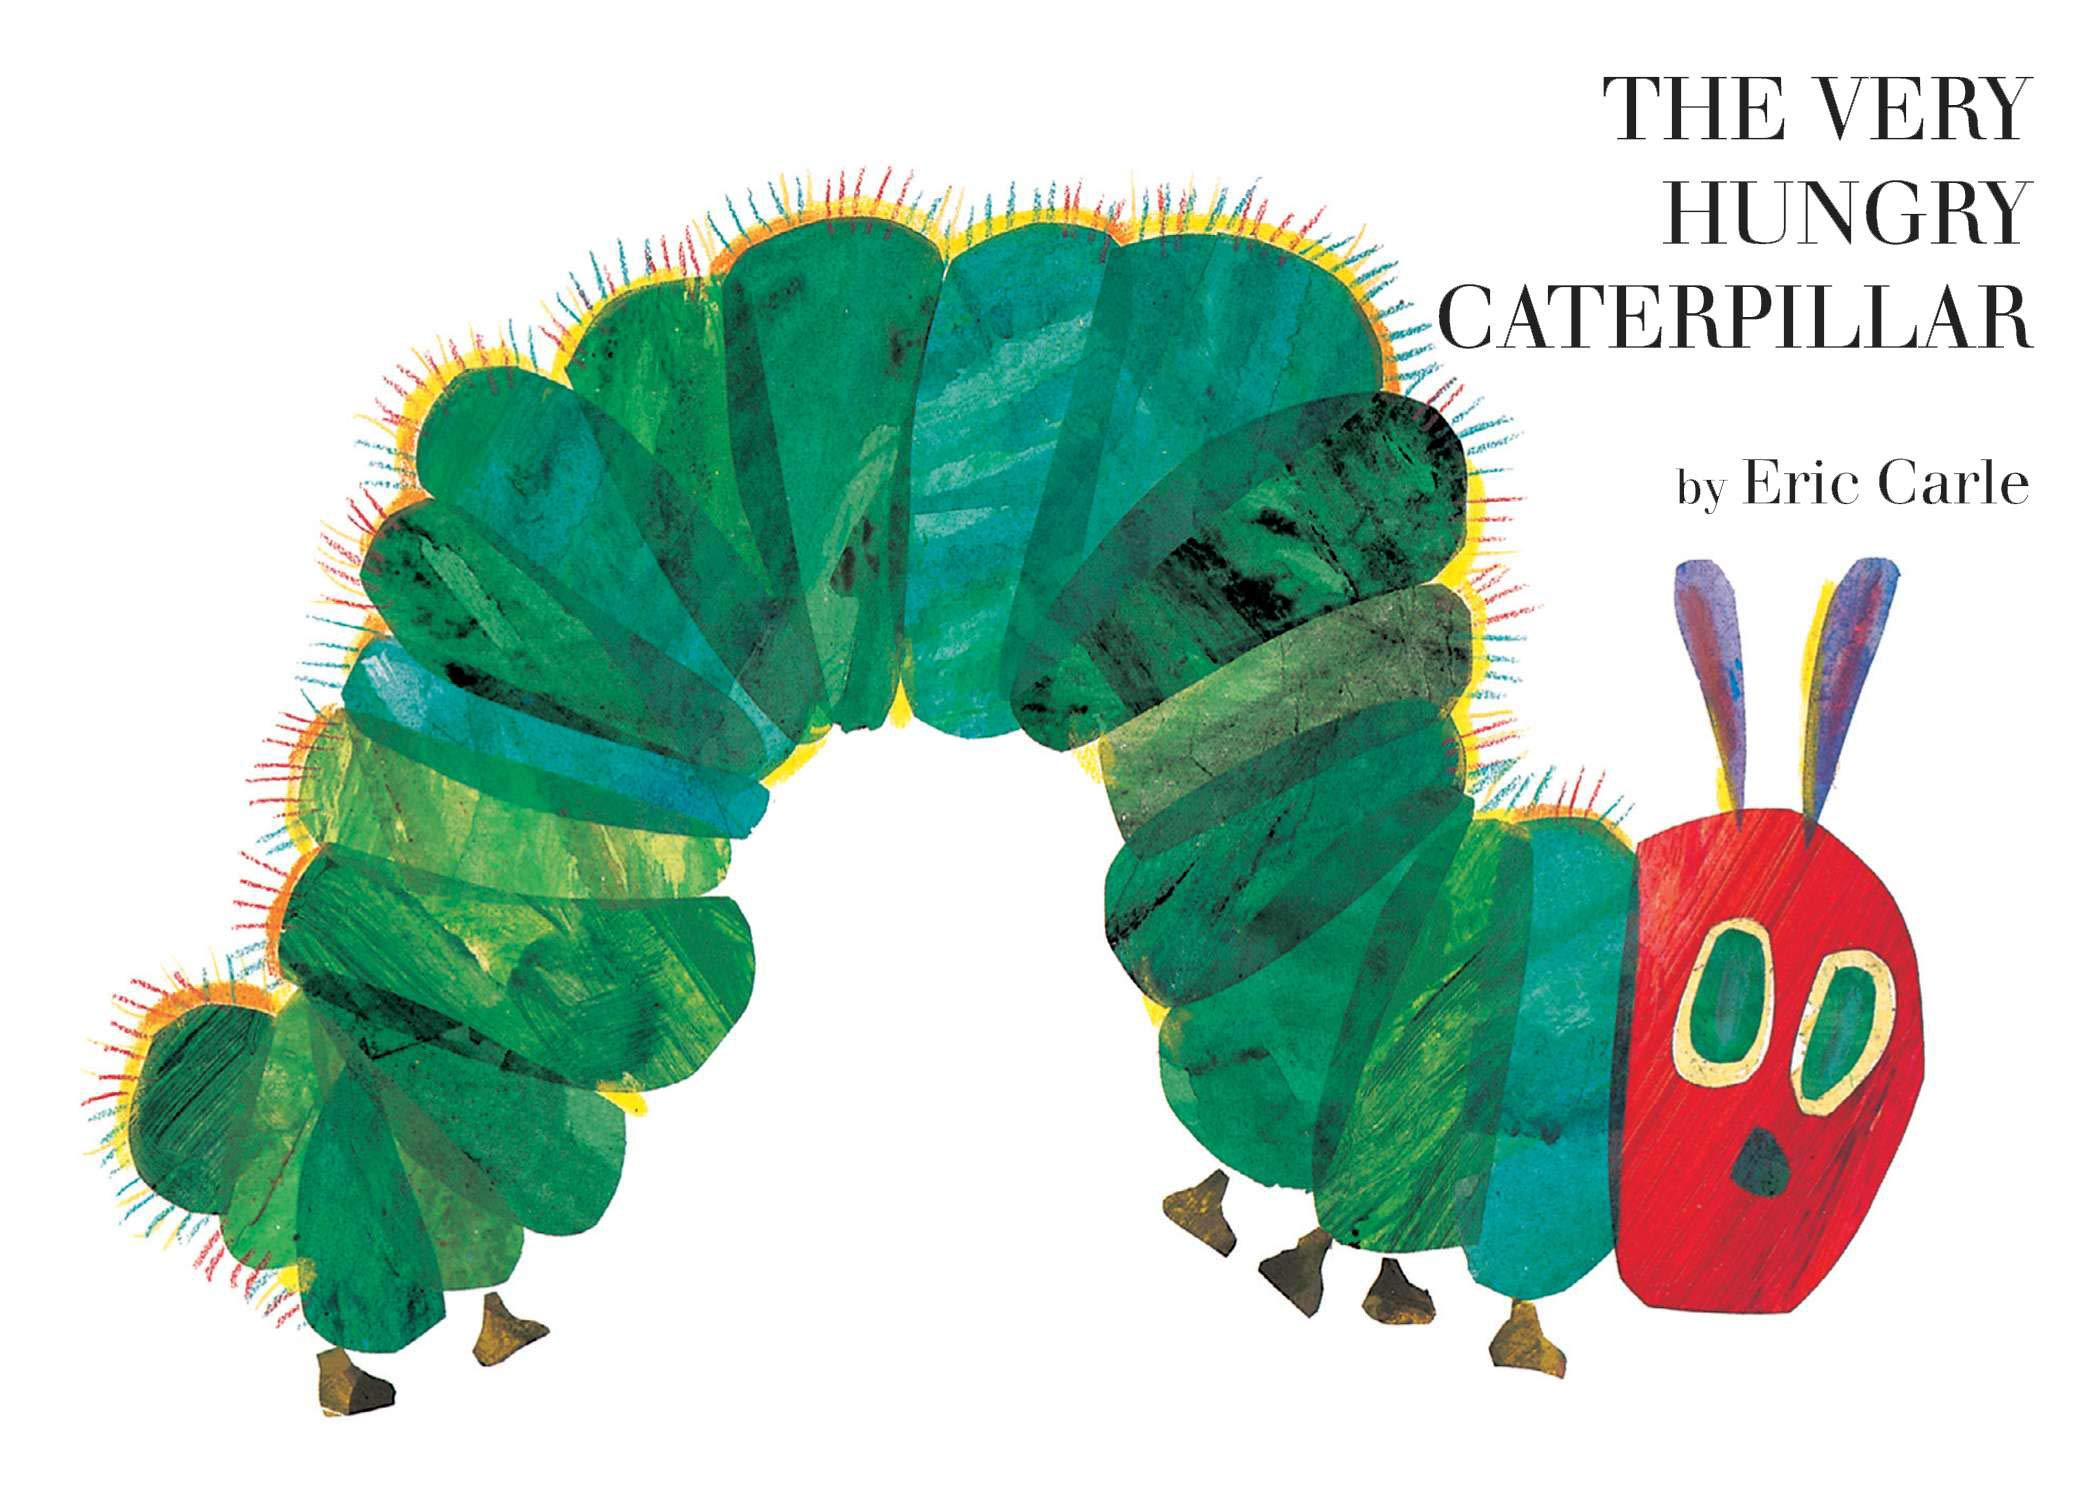} 
\\ 
\textcolor{blue}{\emph{i.}} F : (13, 14, 28, 30) & \textcolor{blue}{\emph{ii.}}  NF : (16, 22, 24) & 
\textcolor{blue}{\emph{iii.}}  NF : (3, 5, 13) & \textcolor{blue}{\emph{iv.}}  F : (16, 29) & 
\textcolor{blue}{\emph{v.}}  NF : (13, 14, 16, 24) & \textcolor{blue}{\emph{vi.}}  NF : (2, 13, 14) & 
\textcolor{blue}{\emph{vii.}}  NF : (7, 16, 22) & \textcolor{blue}{\emph{viii.}}  F : (1, 2, 4, 7)   \\ 
\multicolumn{2}{c|}{Limited visual cues} & \multicolumn{2}{c||}{Complex background} & \multicolumn{4}{c}{Moderate info} \\
%%%%%%%%%%%%%%%
\hline 
&&& &&&&  \\[\dimexpr-\normalbaselineskip+1.5pt]
\includegraphics[width=0.1\linewidth, height=0.145\linewidth]{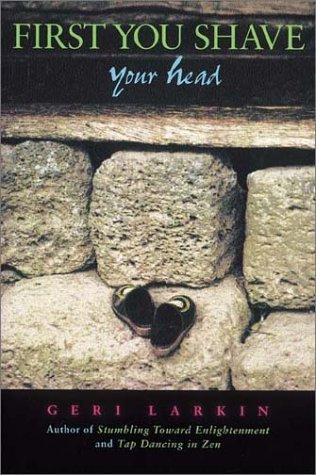} & 
\includegraphics[width=0.1\linewidth, height=0.145\linewidth]{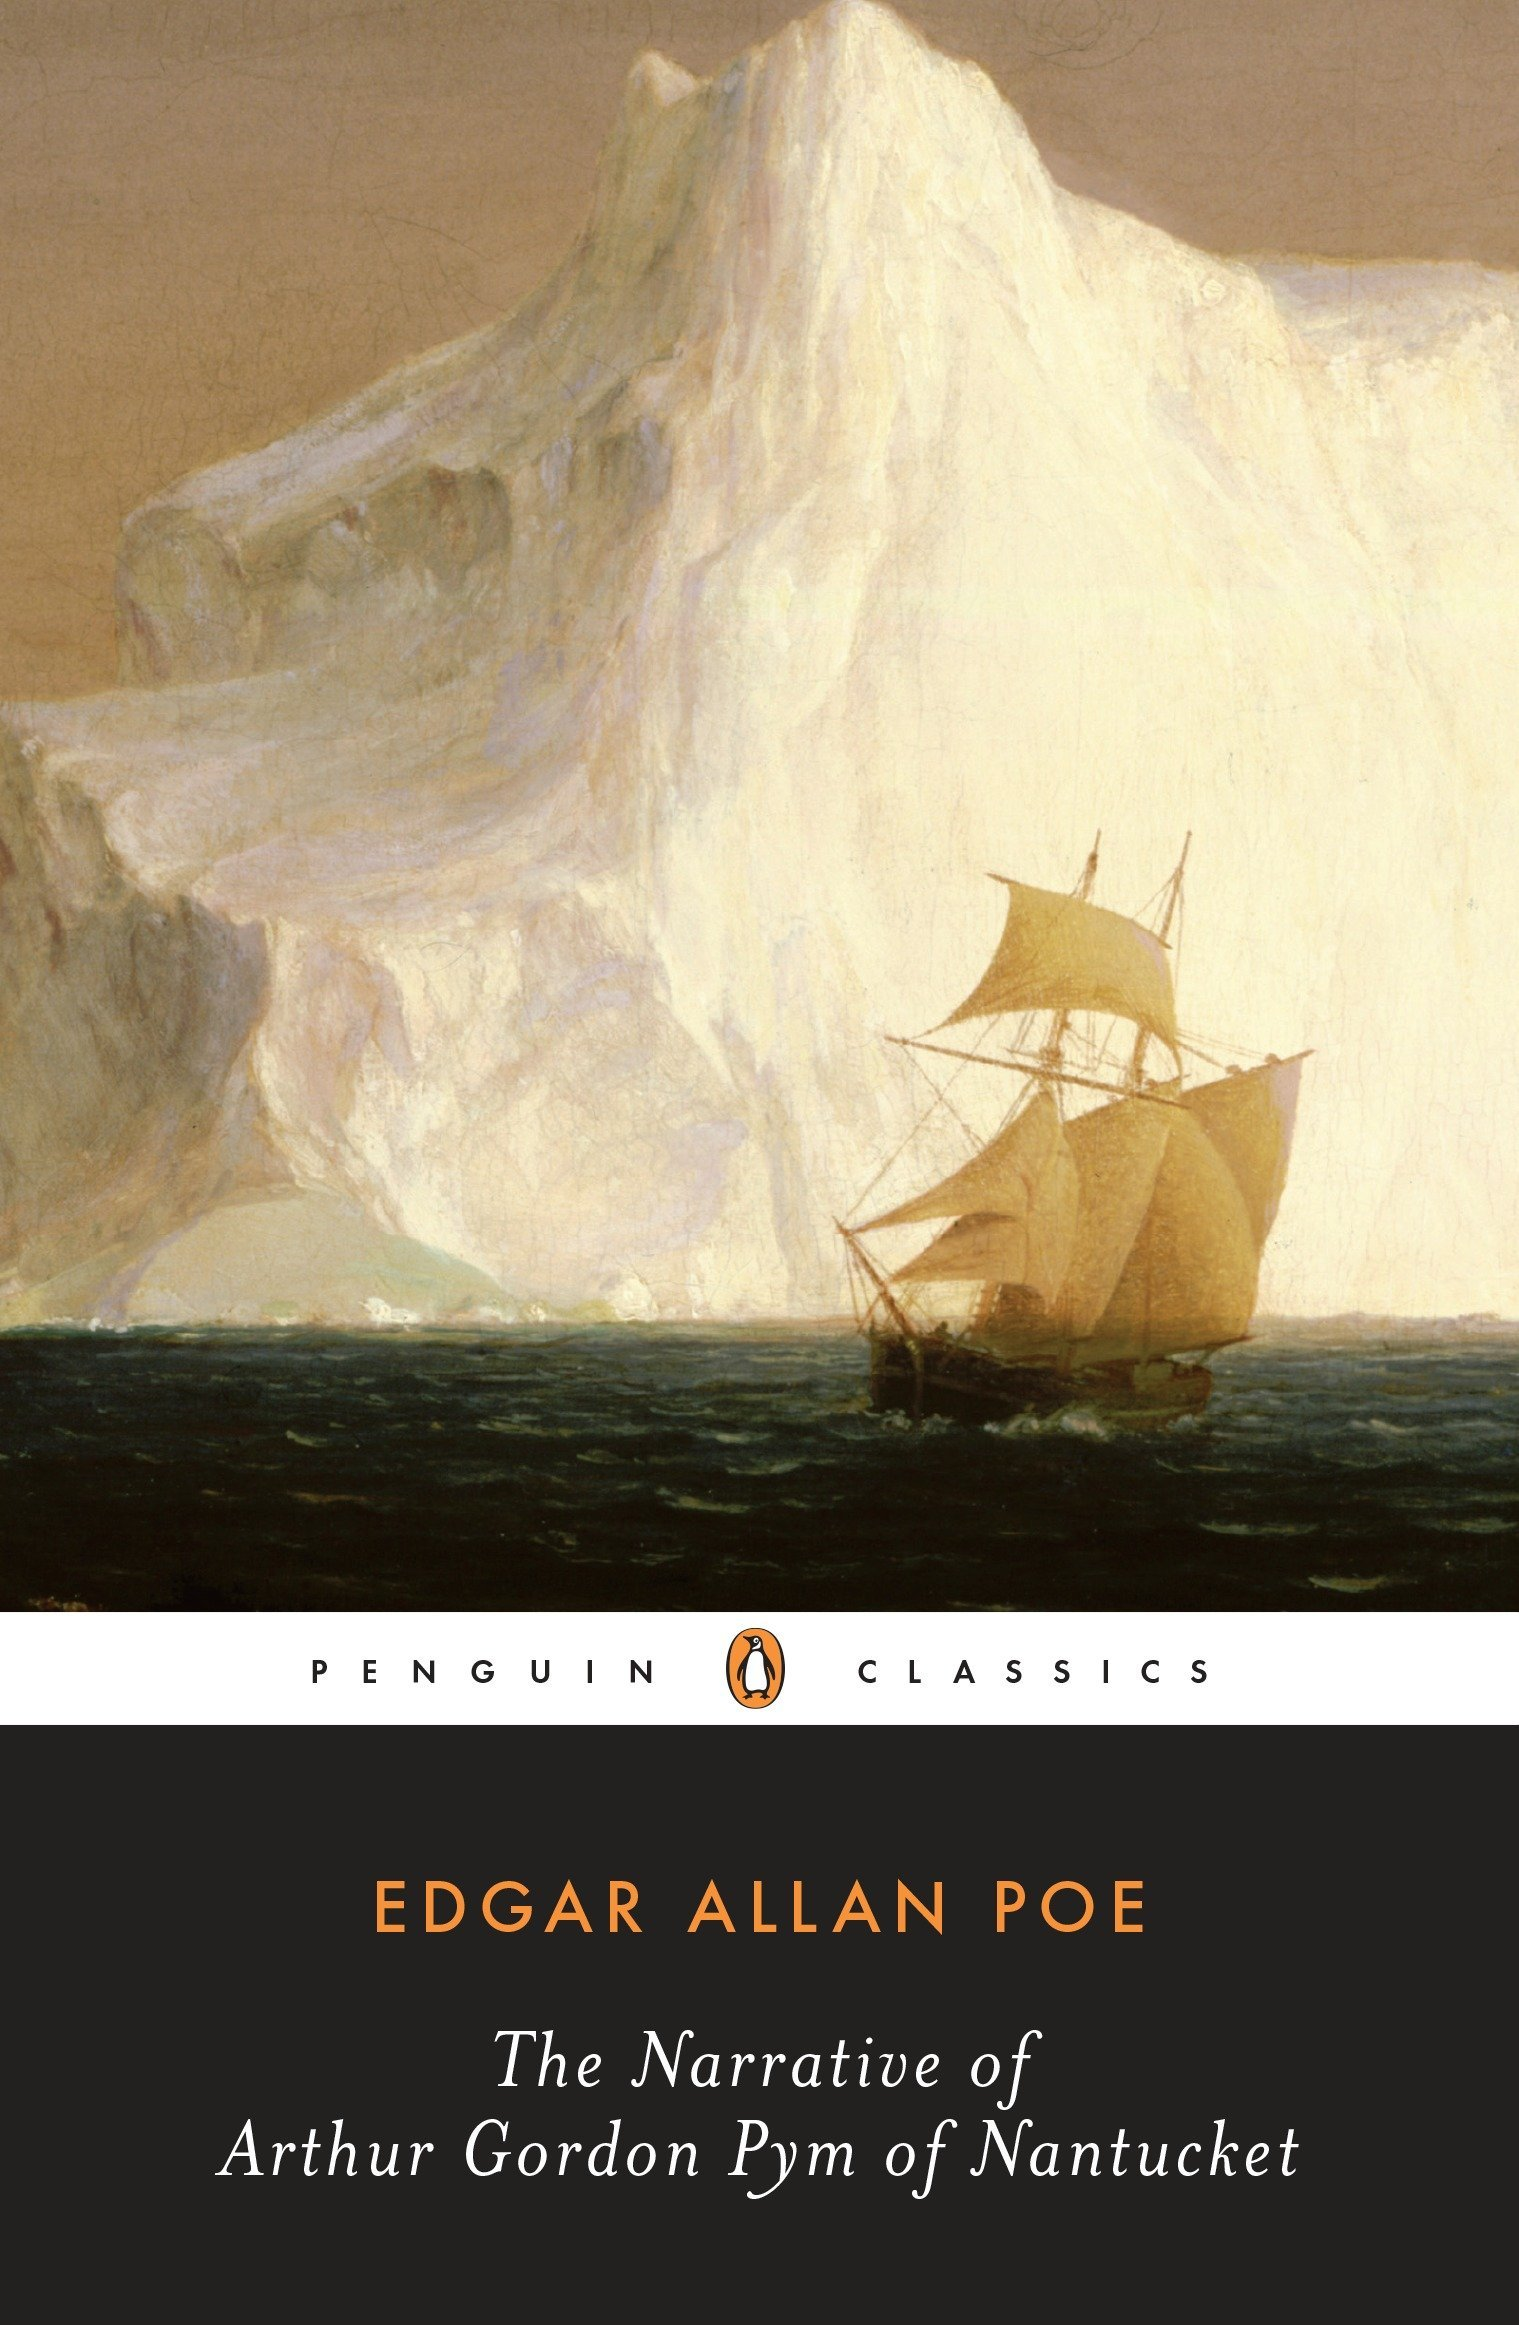} & 
\includegraphics[width=0.1\linewidth, height=0.145\linewidth]{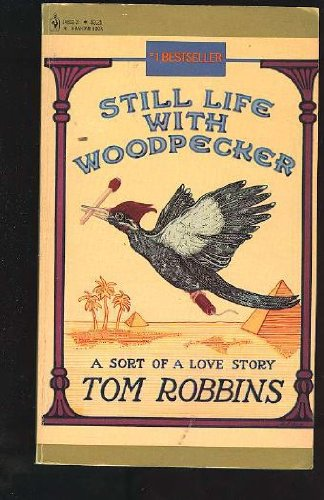} & 
\includegraphics[width=0.1\linewidth, height=0.145\linewidth]{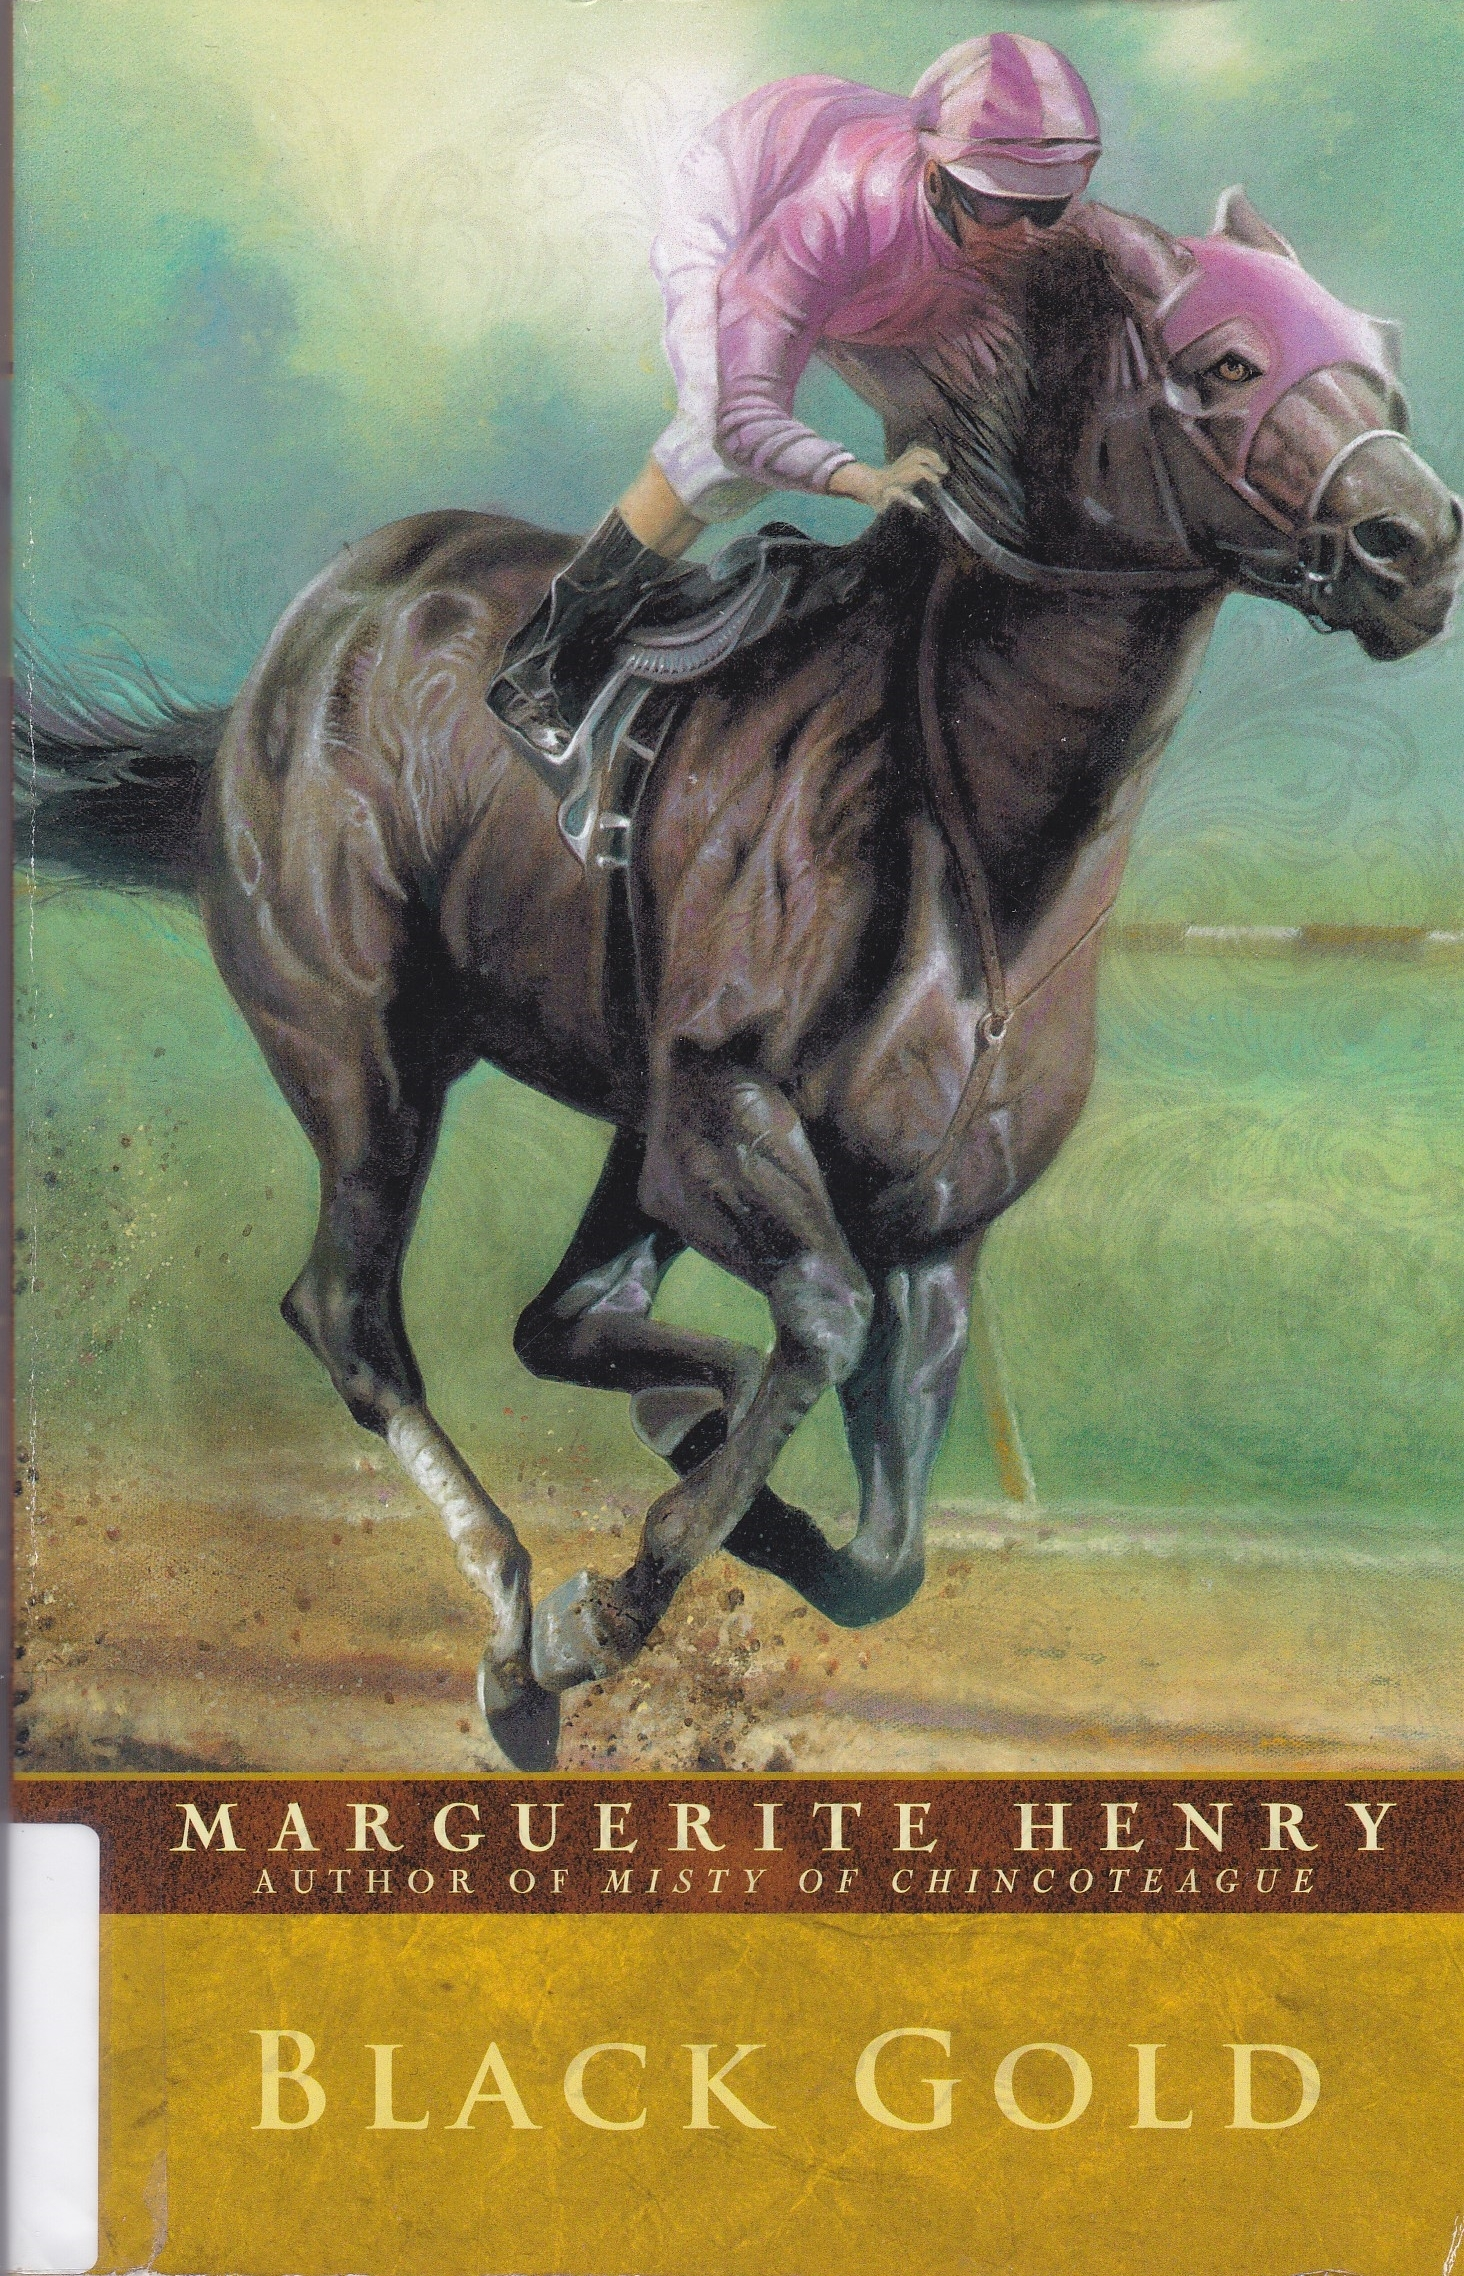} &
\includegraphics[width=0.1\linewidth, height=0.145\linewidth]{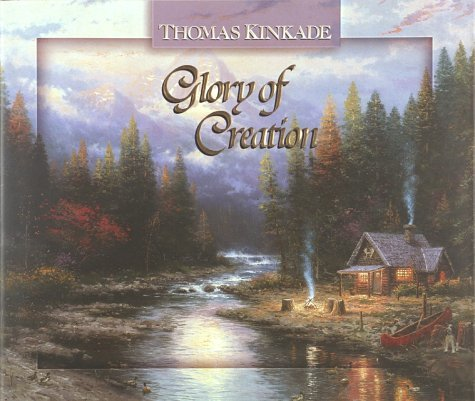} & 
\includegraphics[width=0.1\linewidth, height=0.145\linewidth]{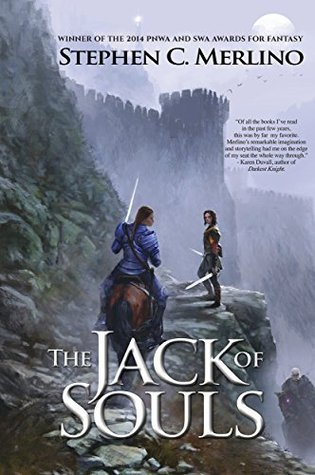} & 
\includegraphics[width=0.1\linewidth, height=0.145\linewidth]{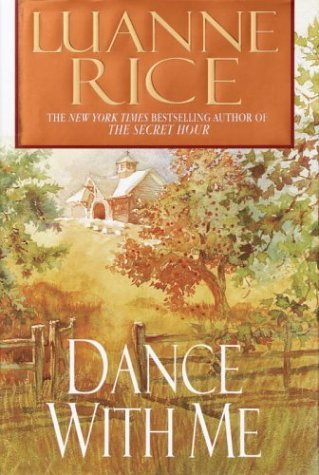} & 
\includegraphics[width=0.1\linewidth, height=0.145\linewidth]{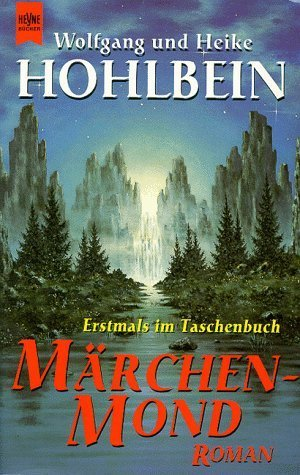} 
\\ 
\textcolor{blue}{\emph{ix.}} NF : (20, 28) & \textcolor{blue}{\emph{x.}}  F : (16, 17, 23, 29) & \textcolor{blue}{\emph{xi.}}  F : (2, 15, 16) & \textcolor{blue}{\emph{xii.}}  F : (9, 14) & 
\textcolor{blue}{\emph{xiii.}}  NF : (2) & \textcolor{blue}{\emph{xiv.}}  F : (29, 23, 27, 17) & \textcolor{blue}{\emph{xv.}}  F : (10, 11, 23) & \textcolor{blue}{\emph{xvi.}} F : (4, 29, 27)  \\ 
\multicolumn{2}{c|}{Non-living element} & \multicolumn{2}{c||}{living element} & \multicolumn{4}{c|}{Scene image}\\
%%%%%%%%%%%%%%%
\hline 
&&& &&&&  \\[\dimexpr-\normalbaselineskip+1.5pt]
\includegraphics[width=0.1\linewidth, height=0.145\linewidth]{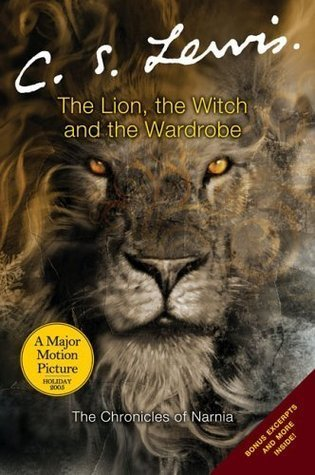} & 
\includegraphics[width=0.1\linewidth, height=0.145\linewidth]{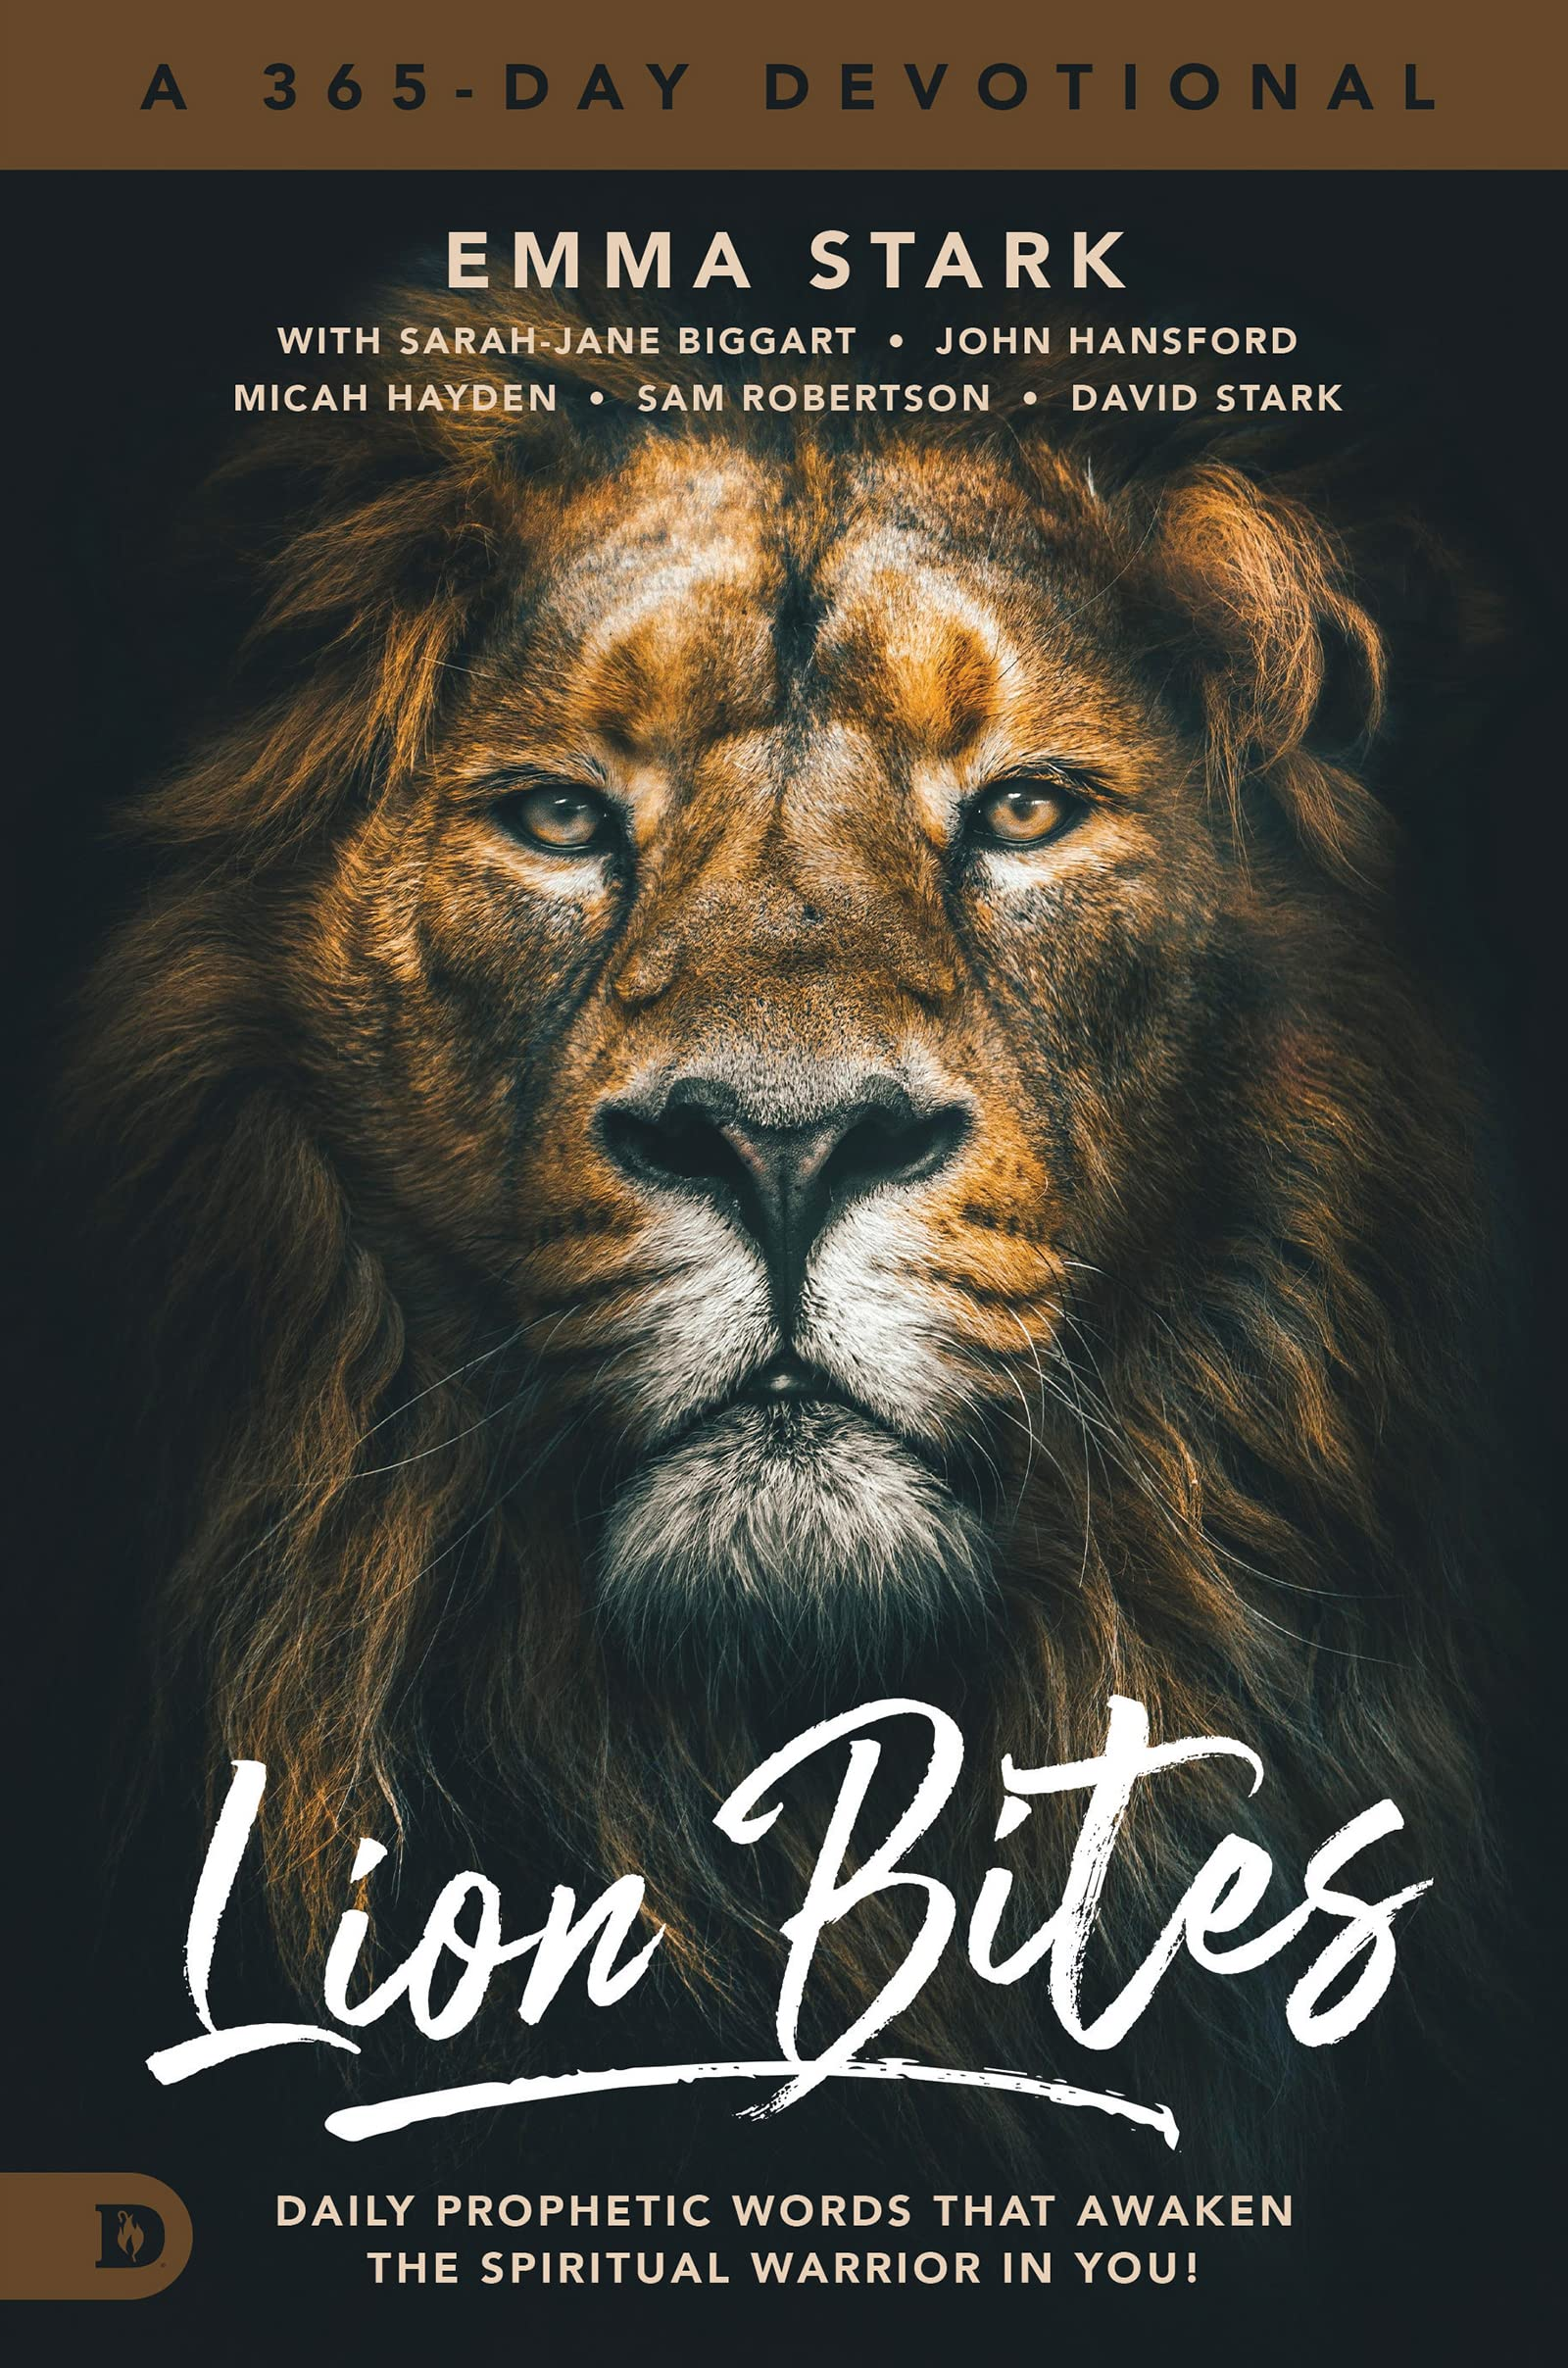} & 
\includegraphics[width=0.1\linewidth, height=0.145\linewidth]{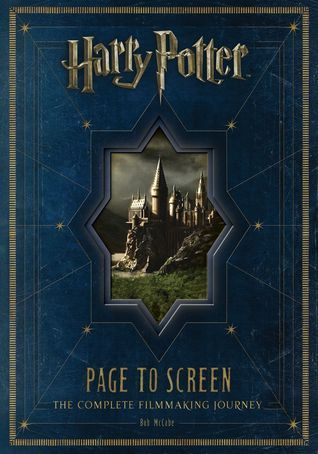} & 
\includegraphics[width=0.1\linewidth, height=0.145\linewidth]{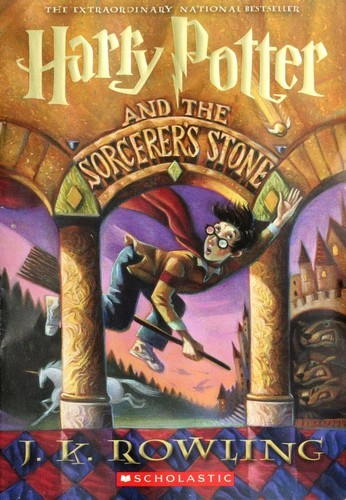} &
\includegraphics[width=0.1\linewidth, height=0.145\linewidth]{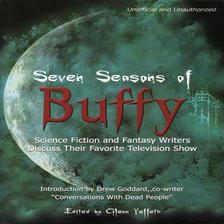} & 
\includegraphics[width=0.1\linewidth, height=0.145\linewidth]{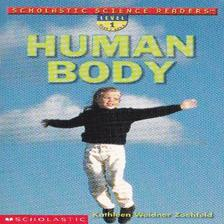} & 
\includegraphics[width=0.1\linewidth, height=0.145\linewidth]{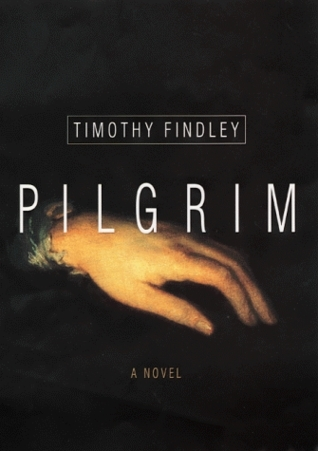} & 
\includegraphics[width=0.1\linewidth, height=0.145\linewidth]{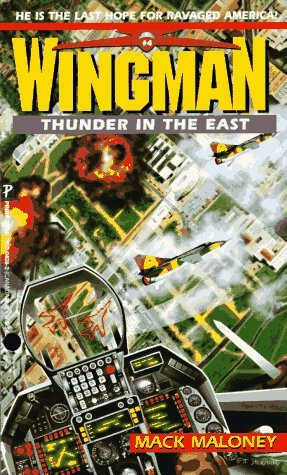} \\ 
\textcolor{blue}{\emph{xvii.}} F : (29, 27, 4) & \textcolor{blue}{\emph{xviii.}}  NF : (20) & \textcolor{blue}{\emph{xix.}}  NF : (22, 19, 27) & \textcolor{blue}{\emph{xx.}}  F : (2, 4, 16, 27) & 
\textcolor{blue}{\emph{xxi.}}  NF : (2, 24) & \textcolor{blue}{\emph{xxii.}}  NF : (2, 24) & \textcolor{blue}{\emph{xxiii.}}  F : (13, 14, 16, 29) & \textcolor{blue}{\emph{xxiv.}}  F : (13, 14, 16, 19)  \\ 
\multicolumn{2}{c|}{Inter-variation} & \multicolumn{2}{c||}{Inter-variation} & \multicolumn{2}{c|}{Intra-variation} & \multicolumn{2}{c}{Intra-variation}\\ 
%%%%%%%%%%%%%%%
\hline 
&&& &&&&  \\[\dimexpr-\normalbaselineskip+1.5pt]
\includegraphics[width=0.1\linewidth, height=0.145\linewidth]{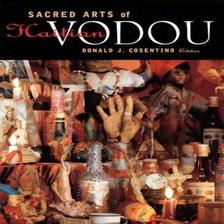} & 
\includegraphics[width=0.1\linewidth, height=0.145\linewidth]{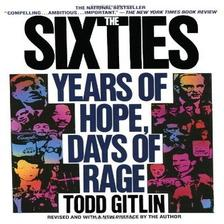} & 
\includegraphics[width=0.1\linewidth, height=0.145\linewidth]{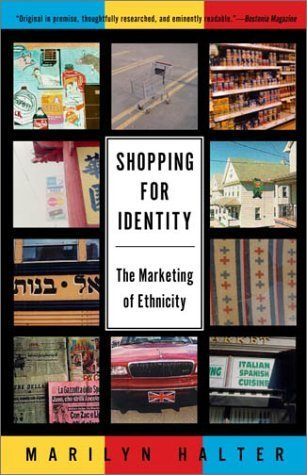} & 
\includegraphics[width=0.1\linewidth, height=0.145\linewidth]{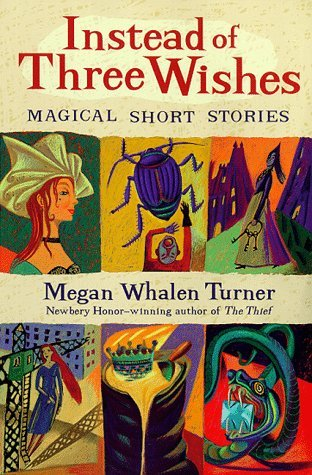} &
\includegraphics[width=0.1\linewidth, height=0.145\linewidth]{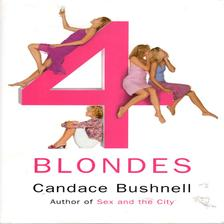} & 
\includegraphics[width=0.1\linewidth, height=0.145\linewidth]{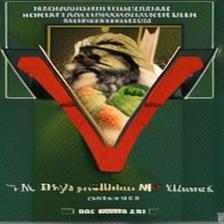} & 
\includegraphics[width=0.1\linewidth, height=0.145\linewidth]{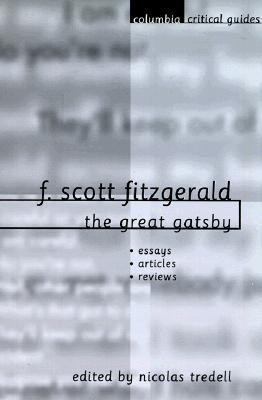} & 
\includegraphics[width=0.1\linewidth, height=0.145\linewidth]{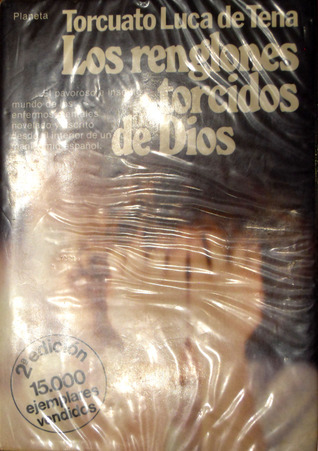} \\ 
\textcolor{blue}{\emph{xxv.}} NF : (2, 13, 20) & \textcolor{blue}{\emph{xxvi.}}  NF : (2, 13, 14) & \textcolor{blue}{\emph{xxvii.}}  NF : (3, 13, 14) & \textcolor{blue}{\emph{xxviii.}}  F : (4, 29, 27) & 
\textcolor{blue}{\emph{xxix.}}  F : (11, 16, 23) & \textcolor{blue}{\emph{xxx.}}  F : (21, 29) & \textcolor{blue}{\emph{xxxi.}} F : (16, 27, 13) & \textcolor{blue}{\emph{xxxii.}}  F : (14, 16, 17) \\ 
\multicolumn{4}{c||}{Collage} & \multicolumn{2}{c|}{Number/ letter as image} & \multicolumn{2}{c}{Unclear image}\\
%%%%%%%%%%%%%%%
\hline
\end{tabular}
\end{adjustbox}
}
\caption{Examples of some challenging book cover images with mentioned issues}
\label{fig:challenge}
\end{figure*}

\begin{figure*}[t]
\centering
\footnotesize
\resizebox{\textwidth}{!}{
\begin{tabular}{c|c|c|c || c|c|c|c}
%%%%%%%%%%%%%%%
\hline 
&&& &&&&  \\[\dimexpr-\normalbaselineskip+1.5pt]
\includegraphics[width=0.1\linewidth, height=0.145\linewidth]{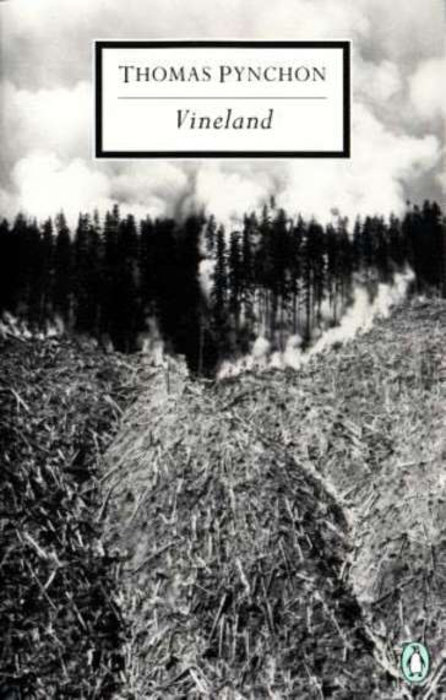} & 
\includegraphics[width=0.1\linewidth, height=0.145\linewidth]{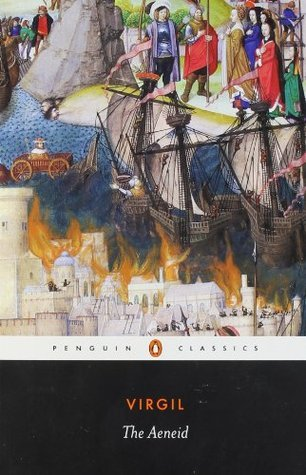} & 
\includegraphics[width=0.1\linewidth, height=0.145\linewidth]{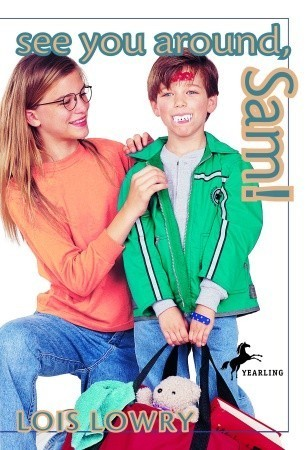} & 
\includegraphics[width=0.1\linewidth, height=0.145\linewidth]{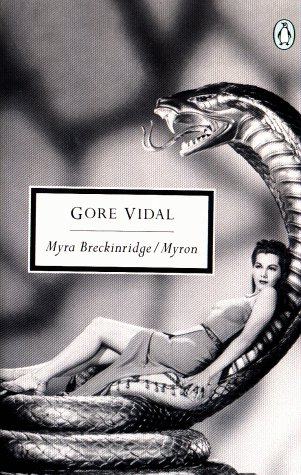} &
\includegraphics[width=0.1\linewidth, height=0.145\linewidth]{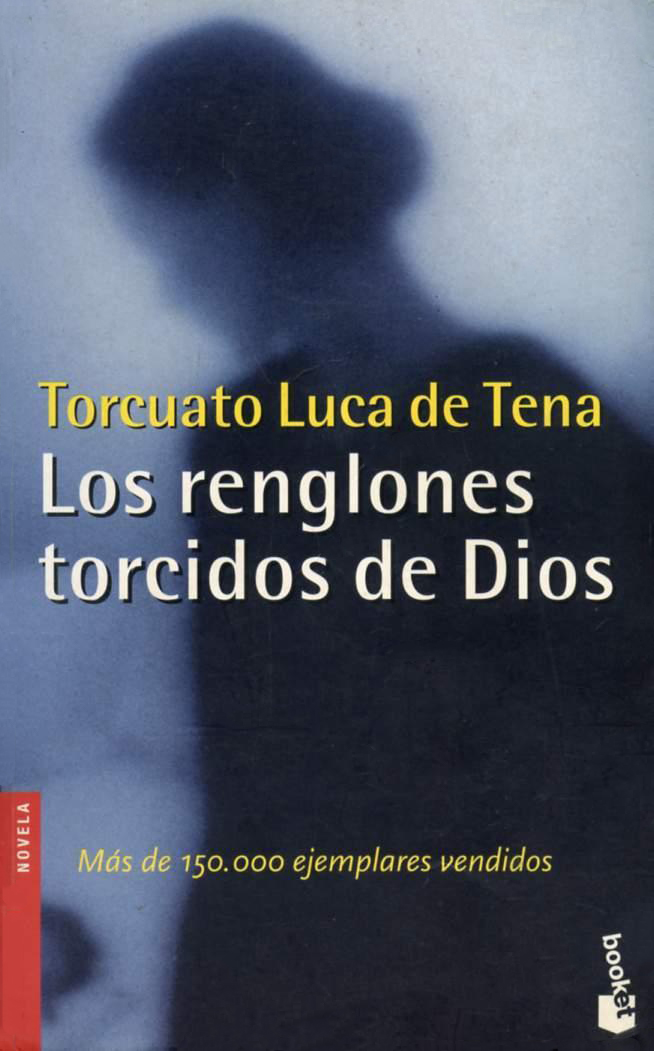} & 
\includegraphics[width=0.1\linewidth, height=0.145\linewidth]{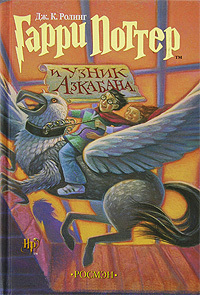} & 
\includegraphics[width=0.1\linewidth, height=0.145\linewidth]{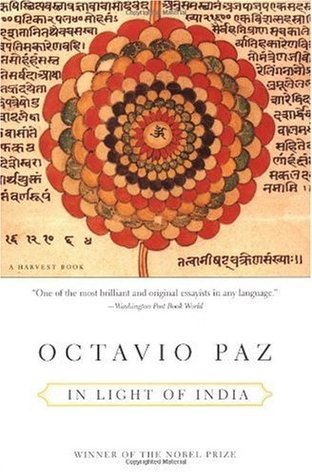} &
\includegraphics[width=0.1\linewidth, height=0.145\linewidth]{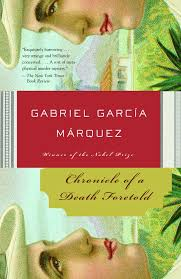}\\
\textcolor{blue}{\emph{i.}} F : (16) & \textcolor{blue}{\emph{ii.}}  F : (16, 20, 29, 27) & \textcolor{blue}{\emph{iii.}}  F : (4, 27) & \textcolor{blue}{\emph{iv.}}  F : (11, 14, 16) & 
\textcolor{blue}{\emph{v.}}  F : (13, 16, 28) & \textcolor{blue}{\emph{vi.}}  F : (2, 4, 29, 27) & \textcolor{blue}{\emph{vii.}} NF : (13, 16, 28) & \textcolor{blue}{\emph{viii.}}  F : (22, 29) \\ 
\multicolumn{4}{c||}{Limited information} & \multicolumn{4}{c}{Non-English cover text}\\
%%%%%%%%%%%%%%%

%%%%%%%%%%%%%%%
\hline 
&&& &&&&  \\[\dimexpr-\normalbaselineskip+1.5pt]
\includegraphics[width=0.1\linewidth, height=0.145\linewidth]{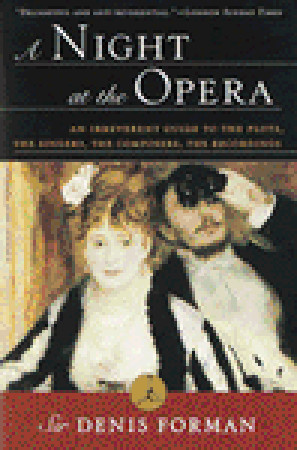} & 
\includegraphics[width=0.1\linewidth, height=0.145\linewidth]{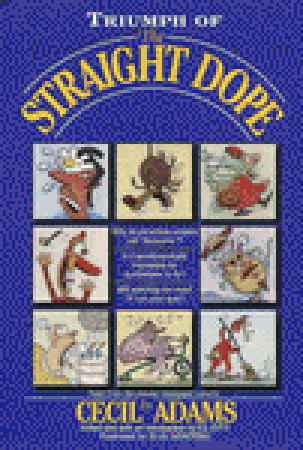} & 
\includegraphics[width=0.1\linewidth, height=0.145\linewidth]{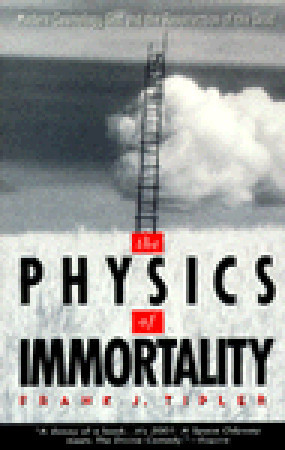} & 
\includegraphics[width=0.1\linewidth, height=0.145\linewidth]{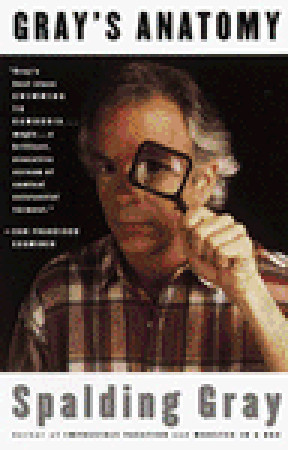} &
\includegraphics[width=0.1\linewidth, height=0.145\linewidth]{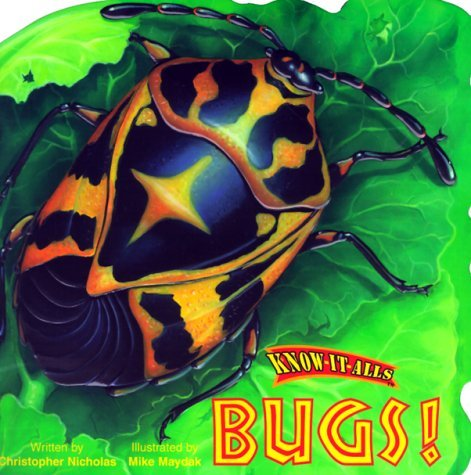} & 
\includegraphics[width=0.1\linewidth, height=0.145\linewidth]{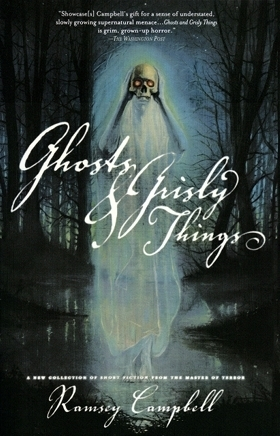} & 
\includegraphics[width=0.1\linewidth, height=0.145\linewidth]{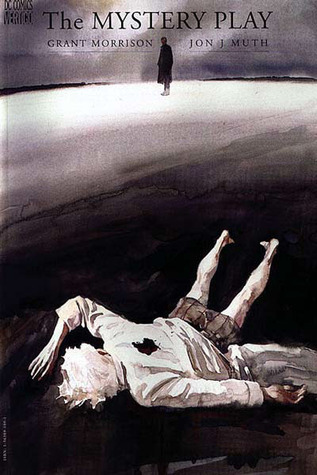} & 
\includegraphics[width=0.1\linewidth, height=0.145\linewidth]{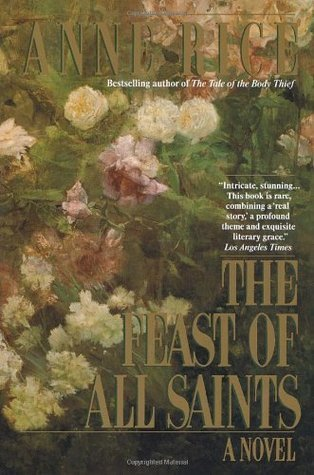}\\ 

\textcolor{blue}{\emph{ix.}} NF : (2, 13, 22) & \textcolor{blue}{\emph{x.}}  NF : (15, 22) & \textcolor{blue}{\emph{xi.}}  NF : (14, 20, 24) & \textcolor{blue}{\emph{xii.}}  NF : (13, 14, 24) & 
\textcolor{blue}{\emph{xiii.}}  NF : (1, 2, 4) & \textcolor{blue}{\emph{xiv.}}  F : (17,24, 29) & \textcolor{blue}{\emph{xv.}} F : (5, 17) & \textcolor{blue}{\emph{xvi.}}  F : (13, 17, 29) \\ 
\multicolumn{4}{c||}{Low resolution cover images} & \multicolumn{4}{c}{Complex background}\\
%%%%%%%%%%%%%%%
\hline
\end{tabular}
}
% \caption{Some challenges of extracting OCR from book cover page}
% \caption{Some challenges of extracted text from cover page}
\caption{Examples of some challenging cases involving text on cover page}
\label{fig:challenge_ocr}
\end{figure*}

% Examples of complex cases involving text elements on book covers.
% involving text on book covers

%%%%
   %%         1->'Animals & Wild life & Pets',
   %%		   2->'Arts & Photography',
   %%	       3->'Business & Money',
   %%	   4->'Childrens Book',
   %%	   5->'Comics & Graphic',
   %%		6->'Computers & Technology',
   %%		7->'Cookbooks & Food & Wine',
   %%		8->'Crafts & Hobbies & Home',
   %%		9->'Environment & Plant',
   %%		10->'Family & Parenting & Relationships',
   %%		11->'Fashion & Lifestyle',
   %%		12->'Health & Fitness & Dieting',
   %%		13->'History',
   %%		14->'Humanities',
   %%		15->'Humor & Entertainment',
   %%		16->'Literature',
   %%		17->'Mystery & Thriller & Suspense & Horror',
   %%		18->'Medical',
   %%		19->'Meta Text', 
   %%		20->'Mythology & Religion & Spirituality',
   %%		21->'Press & Media',
   %%		22->'Reference & Language',
   %%		23->'Romance',
   %%		24->'Science & Math & Mathematics',
   %%		25->'Self-Help & Motivation',
   %%		26->'Sports & Outdoors',
   %%		27->'Teen & Young Adult',
   %%		28->'Travel',
   %%		29->'Science Fiction & Fantasy'

  %%

\noindent
We identified several key challenges within each modality of our dataset, which are outlined below. 

%================================================
\subsection{Challenges in Cover Image}
\noindent
The complexity of book cover images poses challenges in accurately identifying book genres. 

\subsubsection{Background}
Book cover image background plays a crucial role in setting the tone or mood, sparking interest, and assisting readers in determining whether the book aligns with their tastes and preferences.
For instance, \emph{sci-fi \& fantasy} book covers frequently showcase detailed background elements, featuring enchanting landscapes and vivid colors, designed to captivate readers with a sense of wonder and adventure (Fig. \ref{fig:challenge}: \emph{viii}). 
Based on the visual cues available in the background of the cover image, we can group it as follows:

\paragraph{Limited Visual Cues} Sometimes, the cover page provides minimal or no visual information, containing only text in standard fonts, making genre identification challenging (Fig.s \ref{fig:challenge}: \emph{i-ii}).

\paragraph{Moderate Information} 
The cover page often includes moderate visual features to represent some of its genres but may fail to capture others due to the multi-label nature of genres (Fig.s \ref{fig:challenge}: \emph{v-viii}).

\paragraph{Complex Background} In some instances, the background of a book cover image becomes convoluted due to the presence of extensive or composite visual effects or elements (Fig.s \ref{fig:challenge}: \emph{iii-iv}).

%================================================

\subsubsection{Foreground}
The foreground of a book cover image plays a vital role in capturing reader attention. 
However, foreground images on book covers pose challenges for genre identification due to ambiguity, cross-genre similarities, abstract designs, stylistic variations, cultural influences, evolving trends, and marketing-driven misrepresentations. 

\paragraph{Living/ Non-living Element} 
The foreground image can effectively communicate the book theme or atmosphere by strategically placing engaging foreground elements. 
Some non-living elements (e.g., mountain, sea, etc.) are typically associated with genres like \emph{travel}. 
However, in some cases (Fig. \ref{fig:challenge}: \emph{x}), such elements are used to represent genres like 
\emph{literature}, 
\emph{mystery \& thriller \& suspense \& horror \& adventure}, 
\emph{romance}, and
\emph{sci-fi \& fantasy}, 
which creates a disconnect and makes genre identification challenging. 
Similarly, living objects contribute to this ambiguity. 
For example, while an animal on the cover often implies a connection to genres like \emph{animals \& wildlife \& pets}, 
there are instances (Fig. \ref{fig:challenge}: \emph{xi-xii}) 
where this association does not hold, making genre identification more challenging.

\paragraph{Scene Image} 
Scene-based images on book covers further complicate genre prediction due to their intricate visual details, clutter, and lack of a cohesive composition (Fig.s \ref{fig:challenge}: \emph{xiii-xvi}). Unlike single-object covers, scene-based images often contain multiple elements—characters, landscapes, objects, or action sequences—that may belong to different genres. This complexity increases ambiguity, as the dominant visual theme may not be immediately apparent. 
Additionally, certain scenes may be common across multiple genres, making classification more challenging. 
Variations in artistic styles, lighting, and color palettes further contribute to genre ambiguity. 

%================================================

\subsubsection{Inter-Variation}
Sometimes, books from different genres may contain similar visual information (Fig.s  \ref{fig:challenge}: \emph{xvii-xviii}, and Fig.s  \ref{fig:challenge}: \emph{xix-xx}). This may be intentional to challenge reader expectations, create intrigue, or highlight genre blends.
For example, cover image of Fig. \ref{fig:challenge}: \emph{xvii} comprises genres  
\emph{childrens' book}, 
\emph{comics \& graphics}, 
\emph{sci-fi \& fantasy}, 
\emph{teen \& young adult}, but another book's cover image (Fig \ref{fig:challenge}: \emph{xviii}) with similar visual cues belongs to \emph{arts \& photography}.

%================================================

\subsubsection{Intra-Variation}
The visual styles and design elements used in cover images within a specific genre can vary widely. 
This variation is often influenced by the author/artist's unique vision and the intended mood of the book, resulting in diverse interpretations of the same genre. 
Additionally, publishers frequently adhere to specific house styles or branding guidelines, incorporating consistent visual elements or color schemes across their catalog. 
While this ensures some level of uniformity within a publisher's collection, the broader diversity in design choices makes genre identification more challenging 
(Fig.s \ref{fig:challenge}: \emph{xxi-xxii}, and Fig.s \ref{fig:challenge}: \emph{xxiii-xxiv}).

%====================================

\subsubsection{Collage}
In some cases, book covers integrate multiple aforementioned background and foreground elements, forming a collage of numerous smaller images. This visual complexity often leads to information overload, making it challenging to accurately determine the book’s genre (Fig.s \ref{fig:challenge}: \emph{xxv-xxviii}).

%====================================
\subsubsection{Number/ Letter as Image}
Occasionally, book covers feature numbers or letters stylized as visual elements. This artistic choice is often intended to emphasize a theme, establish a distinctive style, or highlight key information related to the book’s content. However, such designs pose a unique challenge for genre identification, as the graphical representation of text or numbers can obscure their intended meaning, making interpretation more difficult (Fig.s \ref{fig:challenge}: \emph{xxix-xxx}).

%====================================
\subsubsection{Unclear Image}
Sometimes, book covers feature images that are blurry, hazy, or of low resolution. Extracting meaningful features from such images becomes difficult, making accurate genre identification challenging (Fig.s \ref{fig:challenge}: \emph{xxxi-xxxii}).

%====================================

%====================================

\subsection{Challenges in Cover Text}
\noindent
We extracted text from book cover images using an OCR (Optical Character Recognition) engine. However, these extracted texts present additional challenges, which we summarize below.

%====================================
\subsubsection{Limited Text}
Some book covers feature only minimal text, such as the author name, or the book title, without supplementary elements like subtitles, or descriptive taglines. These additional details often play a crucial role in genre identification. The absence of such details forces the OCR system to rely solely on sparse information, significantly increasing the risk of misclassification (Fig.s \ref{fig:challenge_ocr}: \emph{i-iv}).

%====================================
\subsubsection{Linguistic Issues}
OCR systems are often designed with a primary focus on specific languages, e.g., English. When book covers feature text in non-English languages, these systems may face difficulties in accurately recognizing and processing the characters. Errors in language detection or character recognition can lead to misinterpretations, further complicating text-based genre classification (Fig. \ref{fig:challenge_ocr}: \emph{v-viii}).

%====================================
\subsubsection{Low Resolution Cover Page}
Low-quality and glossy book covers present significant challenges for accurate text extraction using OCR. Glossy surfaces can create glare and reflections when photographed or scanned, interfering with character recognition. Additionally, low-resolution images often result in blurred text, making it difficult to distinguish individual characters. These factors contribute to errors in text extraction and misinterpretation (Fig.s \ref{fig:challenge_ocr}: \emph{ix-xii}).

%====================================
\subsubsection{Complex background}
Colorful or busy backgrounds on book covers present a significant challenge for OCR systems. These complex backgrounds can interfere with the OCR process in several ways:

        \paragraph{Visual Clutter}
        A busy background with multiple colors, patterns, or images can create visual clutter. This clutter makes it difficult for the OCR system to distinguish the text from the background. The presence of various elements can cause the OCR algorithm to misidentify parts of the background as text or fail to recognize the text altogether (Fig.s \ref{fig:challenge_ocr}: \emph{xiii-xvi}).
        
        \paragraph{Color Contrast}
        Text on colorful backgrounds might not have sufficient contrast. When the text color closely matches the background colors, the OCR system struggles to differentiate between them. High contrast between text and background is crucial for accurate OCR, and colorful backgrounds often fail to provide this (Fig.s \ref{fig:challenge_ocr}: \emph{xiii-xvi}).

%====================================

%====================================
\subsection{Challenges in Blurb}

\noindent
The blurb often contains genre-related textual information. However, there are difficulties in accurately identifying genres based on the blurb text. These challenges are briefly outlined below: 

%====================================
\subsubsection{Insufficient Information}
There are several books containing blurb, often lacked the necessary detail to determine the book’s genre accurately. 
For example: 
The book \emph{Peter Pan} (ISBN-13: \emph{9780881011111}) has the blurb \textquotedblleft Book by J.M. Barrie\textquotedblright. Now, from just the information about the author, it is hard to determine the book genres.

%====================================
\subsubsection{Irrelevant Information}
% \emph {\textbf{(b) Irrelevant information}}: 
We encounter many books containing irrelevant information in the blurb. These blurbs frequently consist of vague or generic statements, contributing little to the genre's understanding, making genre identification difficult. 
For instance:
\begin{itemize}[---]
\item The book titles \emph{Pedagogy of the Oppressed} (ISBN-13: \emph{9780826400475}) has the blurb \textquotedblleft SIGNED COPY BY THE AUTHOR\textquotedblright. This information is very irrelevant to identifying book genres.
\end{itemize}

%====================================
\subsubsection{Multilinguality}
% \emph{\textbf{(c) Multilinguality}}:
Blurb texts are available in various languages, each with its own script and sentence structure. This lack of uniformity makes it difficult to build a framework that can effectively understand and process multiple languages. 
%Each language uses different scripts and sentence structures cause different handling. The lack of uniformity in language led to challenges in building a framework that understands multiple languages.

\begin{itemize}[---]
    \item The book \emph{Michelangelo} (ISBN-13: \emph{9783499222290}) has the blurb in the German -  \textquotedblleft In dem vor Vitalität berstenden Stadtstaat Florenz des 16. Jahrhunderts kämpfte eines der universalen Genies der Menschheitsgeschichte wie ein Titan gegen Kardinäle, Fürsten und Päpste. Rivalitäten mit berühmten Zeitgenossen wie Leonardo da Vinci und Raffael machten ihm das Leben ebenso schwer wie seine eigene dämonische Natur. In den Wirren einer zwischen üppigem Prunk und ständigen Kriegen zerrissenen Zeit schuf Michelangelo, "Gottes eigenes Kind", sein unsterbliches Werk.\textquotedblright
\end{itemize}

%====================================

%====================================
\subsection{Challenges of Metadata}
\noindent
There are several challenges for identifying book genres using book metadata information. We summarized those challenges as follows.

%==========================
\subsubsection{Surface-Level Information}
% \emph{\textbf{(a) Surface-Level Information}}: 
Metadata doesn't reveal a user's deeper interests, reading level, or genre preferences. One author writes books on different genres. So, someone who enjoys a particular author might not like all of their books.

%====================================
%====================================

\subsection{Challenges of Ground-Truthing}
\noindent
Establishing reliable ground-truth genre labels presented significant challenges due to the inherent subjectivity and complexity of the task. 

\subsubsection{Partial Understanding by Human Annotators} 
Since it is often impractical for annotators to read an entire book, the ground-truthing process primarily relied on linguistic experts who assigned genre labels based on limited content—such as publisher blurbs, user reviews (e.g., from Goodreads), and selected excerpts. This partial exposure may lead to a superficial or incomplete understanding of the book’s thematic nuances, thereby impacting the accuracy of genre labeling.

\subsubsection{Subjectivity and Inconsistency in Genre Interpretation} 
Genre classification is often influenced by subjective interpretation. Annotators might interpret the same book differently based on the emphasis placed on particular elements. For instance, a book that blends psychological drama and crime might be labeled as \emph{thriller} by one expert, and as \emph{mystery} or \emph{drama} by another, depending on their reading perspective.

\subsubsection{Fiction vs. Non-fiction Ambiguities}
Differentiating between fiction and non-fiction genres was particularly challenging for works related to well-known fictional universes. For example, while a “\emph{Harry Potter}” novel is clearly fiction, a companion book like "\emph{Harry Potter \--- Page to Screen: The Complete Filmmaking Journey}" is non-fiction, despite sharing the same universe and characters. Such genre-conflicting edge cases complicated the labeling process, requiring careful contextual analysis.

\subsubsection{Multi-Label Overlaps and Unclear Boundaries} 
Many books span multiple genres, making it difficult to determine which labels are most appropriate and at what level of the hierarchy. 
% For example, a book might simultaneously belong to “Fantasy,” “Young Adult,” and “Adventure,” but experts may vary in how broadly or narrowly they assign labels, especially without formal guidelines.

\subsubsection{Lack of Standardized Taxonomy} 
Genre taxonomies vary significantly across publishers, retailers, and literary databases, resulting in inconsistent ground-truth references. Aligning expert annotations with a unified genre hierarchy was non-trivial and often required manual reconciliation.

% Reviewer Bias in Indirect Labeling:
% When annotations were based on user reviews or crowdsourced content, they were susceptible to bias or misinterpretation. Reviewers may focus on personal opinions or plot elements irrelevant to genre classification, leading to noise in genre inference.

%====================================

\subsection{Challenges of Overall Dataset}
\noindent
In preparing a high-quality dataset for hierarchical multi-label book genre classification, several overarching challenges emerged, particularly due to the multi-label nature of the task and the complexity of real-world genre distributions.

\subsubsection{Label Imbalance in Multi-Label Context} 
The dataset exhibits significant class imbalance, with certain genres being highly represented, while others appear far less frequently. However, unlike single-label classification, this imbalance cannot be easily corrected through traditional resampling techniques because books often belong to multiple genres simultaneously. Balancing one under-represented genre could unintentionally disrupt the co-occurrence patterns with more frequent genre.

\subsubsection{Constraints in Data Augmentation} 
Augmentation techniques commonly used to balance datasets pose unique risks in the multi-label setting. When augmenting samples from a genre with few examples, the co-occurring genres in the original sample—many of which may already be overrepresented—also get replicated. This reinforces existing imbalance and biases, making it difficult to selectively boost specific genre classes without inadvertently inflating others.}

\subsubsection{Sparse Label Combinations} 
The multi-label setting also leads to a large number of unique label combinations, many of which appear very infrequently. This sparsity in the label space challenges the model’s ability to generalize well to unseen or rare combinations and limits the effectiveness of frequency-based heuristics.

\subsubsection{Dependency Between Genre Labels} 
Usually genre labels are not mutually independent; the presence of one genre may often influence the likelihood of another. Modeling these dependencies becomes increasingly difficult as the number of labels grows, especially under imbalance and sparsity, and it further complicates synthetic balancing or sampling strategies.

%====================================
% \subsection{Challenges of Multi-Class Labeling}
% \noindent
% Multi-labeling of book genres presents several challenges, including:

% \textbullet~ \emph{Visual ambiguity}: Book covers often contain elements that are relevant to multiple genres, making it difficult to assign distinct labels.

% \textbullet~ \emph{Feature overlap}: Certain visual and textual features may be common across different genres, leading to misclassification.

% \textbullet~\emph{Sparse representation}: Some genres may have limited representation in the dataset, making it harder for models to learn their distinguishing features.

% \textbullet~\emph{Inter-genre dependencies}: Some genres frequently co-occur (e.g., Fantasy and Adventure), requiring models to capture complex relationships between labels.

% \textbullet~\emph{Minimal visual cues}: Some book covers lack strong genre-specific visual elements, relying more on textual information, which may not always be available.

% \textbullet~\emph{Subjective labeling}: Genre classification can be subjective, as the same book may be perceived differently by different annotators.

% \textbullet~ \emph{Scalability issues}: As the number of genres increases, assigning multiple labels accurately becomes more computationally intensive.
