# Supplementary material for: Adaptive Data-Resilient Multi-Modal Hierarchical Multi-Label Book Genre Identification
Source: arXiv:2505.03839 source file (2025-10-18)
Supplement: Supplementary file 5 [file 7appendix_data_processing.tex]

\section{Data Processing}
\label{app:data_processing}

\noindent
Below we discuss data augmentation followed by data preprocessing.

\subsection{{Data Augmentation}} 
\noindent
We observed that some specific genres within both fiction and non-fiction had insufficient samples. While these genres did not have enough samples to be removed, the limited information in these samples hindered the effective training of our models. We utilized data augmentation methods to generate new samples for these genres. We discuss data augmentation methods below in detail:

\subsubsection{Visual Data Augmentation}
% \emph{\textbf{(a) Visual Data Augmentation}}: 
To enhance the diversity of the dataset, we employed \textquoteleft{Stable-diffusion-xl-refiner-1.0'} \cite{stable-diffusion-xl-refiner-1.0} for coverpage data augmentation. The diffusion model generates high-quality synthetic data by progressively adding noise to the original data and then learning to reverse this process.

\subsubsection{Textual Data Augmentation}
% \emph{\textbf{(b) Textual Data Augmentation}}: 
To augment description text, we used GEMINI \cite{gemini} a large language model to generate additional description text from the existing one. Through prompt engineering techniques, we ensured that the generated content accurately retained the contextual meaning and relevance of the original data.

\subsection{{Data Preprocessing}}
\noindent
Data preprocessing is the initial step in data analysis, where raw data is transformed into a suitable format for further analysis. We resized coverpage ${\cal{I}}$ into $3 \times 224 \times 224$. Description text ${\cal{T}}$ and cover text ${\cal{C}}$ went through multiple preprocessing steps. First, we remove stop words of the english language and the articles (a, an, the), then we remove string punctuation from them.
