# Supplementary material for: Adaptive Data-Resilient Multi-Modal Hierarchical Multi-Label Book Genre Identification
Source: arXiv:2505.03839 source file (2025-10-18)
Supplement: Supplementary file 6 [file 7appendix_heatmap.tex]

\section{Heatmap for Correct Classification}

\noindent
Table \ref{tab:heatmap_samples} presents 10 selected data samples, and Fig. \ref{tab:heatmap} provides a qualitative evaluation of IMaGINe performance through heatmap encodings for them. These grayscale heatmaps visualize the ground-truth and IMaGINe-predicted genre labels, with white representing positive and black indicating negative genres.

\begin{table*}[!hbt]
\centering
\caption{Data samples for heatmap}
\begin{adjustbox}{width=0.88\textwidth}
% \begin{adjustbox}{angle=90, height=1\textheight}
% \footnotesize
\begin{tabular}{c|ll}%p{0.9\textwidth}}
% \multicolumn{3}{c}{(a) Samples for heatmap analysis}\\
\hline %\hline
% \multicolumn{1}{c}{} & \multicolumn{1}{c}{} & \\[\dimexpr -\normalbaselineskip+1.5pt]

\rowcolor[HTML]{D9D9D9}
\multicolumn{3}{c}{\textcolor{blue}{\emph{(a)}} \textbf{9780060223595: Bread and Jam for Frances; Author: Russell Hoban; Publisher: HarperCollins Publishers}}\\
\hline %\hline
% & \\ [\dimexpr-\normalbaselineskip+1.5pt]

\multirow{5}{*}{\includegraphics[width=0.04\linewidth, height=0.05\linewidth]{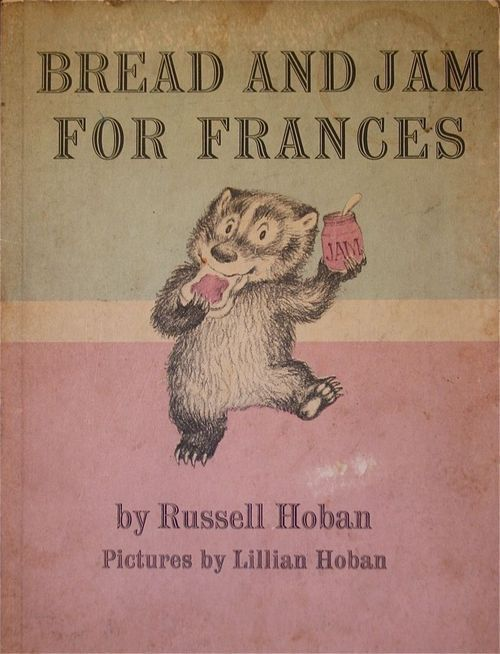}} & \multirow{4}{*}{\textbf{Blurb}:} & The classic funny story about a stubborn little badger with very particular tastes in food. Frances is a fussy eater. In fact, the only thing she likes is bread and jam. She won't  \\
& & touch her squishy soft-boiled egg. She trades away her chicken-salad sandwich at lunch. She turns up her nose at boring veal cutlets. Unless her parents can come up with a \\
& &    plan, Frances just might go on eating bread and jam forever! Join the generations of families that have laughed along as Frances sings "Jam on biscuits, jam on bread,\\
& &   Jam is the thing I like most, Jam is sticky, jam is sweet, Jam is tasty, jam’s a treat—raspberry, strawberry, gooseberry, I’m very FOND…OF…JAM!"\\ \cline{2-3}
% & ${\cal{M}}$ & \{"author":"Russell Hoban","publisher":"HarperCollins Publishers"\}\\ \hline
& \multicolumn{1}{l}{\textbf{Actual Genre}:} & (Fiction, \{Animals \& Wildlife \& Pets, Arts \& Photography, {Childrens\textquoteright} Book, Cookbooks \& Food \& Wine, Family \& Parenting \& Relationships, Literature\})\\ 

\hline \hline

\rowcolor[HTML]{D9D9D9}
\multicolumn{3}{c}{\textcolor{blue}{\emph{(b)}} \textbf{9782723423014: Sailor Moon, tome 14 : Le royaume Elusion; Author: Naoko Takeuchi; Publisher: GLÉNAT}}\\
\hline 

\multirow{3}{*}{\includegraphics[width=0.04\linewidth, height=0.05\linewidth]{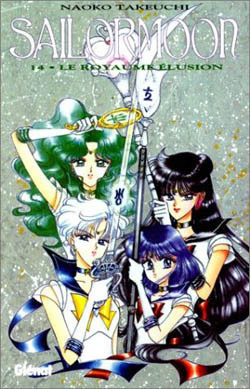}} & \multirow{2}{*}{\textbf{Blurb}:} & A graphic novel offers the continuing adventures of Serena and her friends, who use the power of the moon and the planets, as the superhero Sailor Moon and her comrades, \\
& &  to battle the forces of evil. \\ \cline{2-3}

% & ${\cal{M}}$ & \{"author":"Naoko Takeuchi","publisher":"GLÉNAT"\}\\ \hline
& \multicolumn{1}{l}{\textbf{Actual Genre}:} & (Fiction, \{Comics \& Graphic, Romance, Science Fiction \& Fantasy\})\\

\hline \hline
\rowcolor[HTML]{D9D9D9}
\multicolumn{3}{c}{\textcolor{blue}{\emph{(c)}} \textbf{9780895297273: Prescription for Nutritional Healing: A Practical A-Z Reference to Drug-Free Remedies Using Vitamins, Minerals, Herbs \& Food Supplements;}}\\
\rowcolor[HTML]{D9D9D9}
\multicolumn{3}{c}{ \textbf{
Author: James F. Balch; Publisher: Avery Publishing Group}} \\
\hline 
\multirow{3}{*}{\includegraphics[width=0.04\linewidth, height=0.05\linewidth]{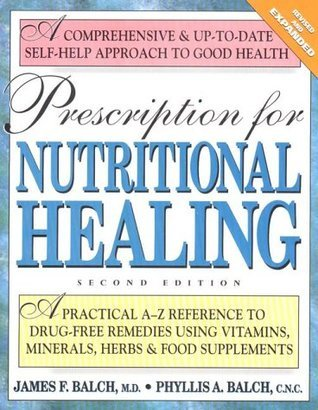}} & \multirow{2}{*}{\textbf{Blurb}:} & An alphabetical encyclopedia of nutritional treatments for a wide range of common ailments explains how to use vitamins, herbs, minerals, and food supplements to promote \\
& &  healing and wellness.\\ \cline{2-3}
% & ${\cal{M}}$ & \{"author":"James F.,Md. Balch","publisher":"Avery Publishing Group"\}\\ \hline
& \multicolumn{1}{l}{\textbf{Actual Genre}:} & (Non-fiction, \{Cookbooks \& Food \& Wine, Health \& Fitness \& Dieting, Medical, Reference \& Language, Self-Help \& Motivation\})\\

\hline \hline
\rowcolor[HTML]{D9D9D9}
\multicolumn{3}{c}{\textcolor{blue}{\emph{(d)}} \textbf{9780060172732: The Dog Who Rescues Cats: The True Story of Ginny; Author: Philip Gonzalez; Publisher: Harpercollins}}\\
\hline 
\multirow{3}{*}{\includegraphics[width=0.04\linewidth, height=0.05\linewidth]{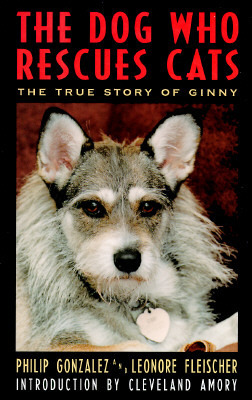}} & \multirow{2}{*}{\textbf{Blurb}:} & The true story of Ginny, an abused dog with an affinity for rescuing cats in trouble, describes Ginny's part in the saving of such handicapped felines as the one-eyed Revlon, \\
& &  deaf Madam, and the paralyzed Topsy. \\ \cline{2-3}

% & ${\cal{M}}$ & \{"author":"Philip Gonzalez","publisher":"Harpercollins"\}\\ \hline
& \multicolumn{1}{l}{\textbf{Actual Genre}:} & (Non-fiction, \{Animals \& Wildlife \& Pets, Biographies \& Memoir\})\\

\hline \hline
\rowcolor[HTML]{D9D9D9}
\multicolumn{3}{c}{\textcolor{blue}{\emph{(e)}} \textbf{9780671668365: MAGIC OF CONFLICT; Author: Thomas Crum; Publisher: Touchstone}}\\
\hline 
\multirow{3}{*}{\includegraphics[width=0.04\linewidth, height=0.05\linewidth]{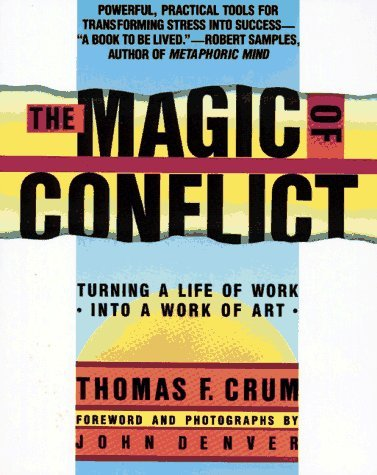}} & \multirow{2}{*}{\textbf{Blurb}:} & Gives techniques for transforming conflict into an opportunity for choice and change and how to grow beyond the striving competitiveness, and pressure of personal and \\
& &  professional life. \\ \cline{2-3}

% & ${\cal{M}}$ & \{"author":"Thomas Crum","publisher":"Touchstone"\}\\
% \hline

& \multicolumn{1}{l}{\textbf{Actual Genre}:} & (Non-fiction, \{Business \& Money, Humanities, Mythology \& Religion \& Spirituality, Self-Help \& Motivation\})\\

\hline \hline
\rowcolor[HTML]{D9D9D9}
\multicolumn{3}{c}{\textcolor{blue}{\emph{(f)}} \textbf{9780963235930: Beyond Backpacking: Ray Jardines Guide to Lightweight Hiking; Author: Ray Jardine; Publisher: Adventurelore Press}}\\
\hline

\multirow{3}{*}{\includegraphics[width=0.04\linewidth, height=0.05\linewidth]{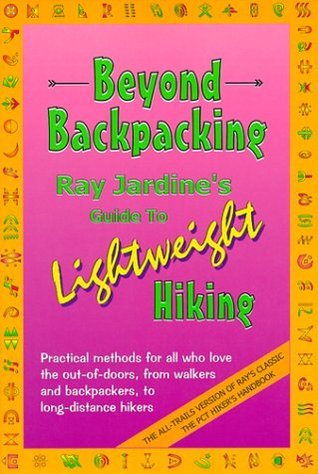}} & \multirow{2}{*}{\textbf{Blurb}:} & Beyond Backpacking has 517 pages of "practical methods for all who love the out-of-doors". Chapters include Equipment, Hiking Considerations, Obstacles, Longer  \\
& & Journeys and Back to Basics.  \\
\cline{2-3}
% & ${\cal{M}}$ & \{"author":"Ray Jardine","publisher":"Adventurelore Press"\}\\
% \hline
& \multicolumn{1}{l}{\textbf{Actual Genre}:} & (Non-fiction, \{Environment \& Plant, Mystery \& Thriller \& Suspense \& Horror, Reference \& Language, Sports \& Outdoors, Travel\})\\

\hline \hline
\rowcolor[HTML]{D9D9D9}
\multicolumn{3}{c}{\textcolor{blue}{\emph{(g)}} \textbf{9780380773527: Dreaming of You; Author: Lisa Kleypas; Publisher: Avon}}\\
\hline 
\multirow{7}{*}{\includegraphics[width=0.04\linewidth, height=0.05\linewidth]{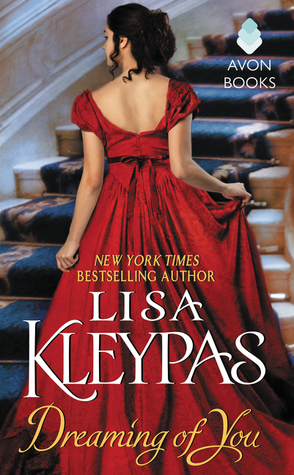}} & \multirow{6}{*}{\textbf{Blurb}:} & She stood at danger's threshold—then love beckoned her in.A prim, well-bred gentlewoman, Sara Fielding is a writer who puts pen to paper to create dreams. But now\\
& &   curiosity is luring her from the shelter of her country cottage into the dangerous world of Derek Craven—handsome, tough, and tenacious—and the most exciting man Sara \\
& &  has ever met. Derek rose from poverty to become the wealthy lord of London’s most exclusive gambling house. And now duty demands that he allow Sara Fielding to \\
& &  enter his perilous realm of ever-shifting fortunes—with her impeccable manners and her infuriating innocence. But there is a hidden strength and sensuality to the lady that\\
& &    captivates him beyond  his better judgment.And in this world, where danger lurks behind every shadow, even a proper “mouse” can be transformed into a breathtaking \\
& &  enchantress—and a cynical gambler can be shaken to his core by the power of passion and the promise of love.\\
\cline{2-3}
& \multicolumn{1}{l}{\textbf{Actual Genre}:} & (Fiction, \{Fashion \& Lifestyle, History, Romance\})\\

\hline \hline

\rowcolor[HTML]{D9D9D9}
\multicolumn{3}{c}{\textbf{{\emph{(h).}} 9780679602613: The Soul of a New Machine; Author: TRACY KIDDER; Publisher: Modern Library}}\\
\hline \hline

\multirow{13}{*}{\includegraphics[width=0.04\linewidth, height=0.05\linewidth]{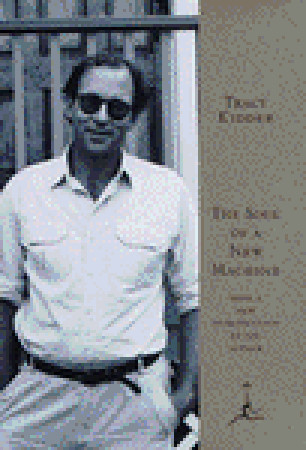}} & \multirow{12}{*}{\textbf{Blurb}:} & Winner of the Pulitzer Prize and the American Book Award, The Soul of a New Machine was a bestseller on its first publication in 1981. With the touch of an expert thriller\\
& &    writer, Tracy Kidder recounts the feverish efforts of a team of Data General researchers to create a new 32-bit superminicomputer. A compelling account of individual sacrifice \\
& &    and human ingenuity, The Soul of a New Machine endures as the classic chronicle of the computer age and the masterminds behind its technological advances. "A superb \\
& &   book," said Robert Pirsig, author of Zen and the Art of Motorcycle Maintenance. "All the incredible complexity and chaos and exploitation and loneliness and strange,\\
& &     half-mad beauty of this field are honestly and correctly drawn." The Washington Post Book World said, "Kidder has created compelling entertainment.  He offers a fast,\\
& &    painless, enjoyable means to an initial understanding of computers, allowing us to understand the complexity of machines  we could only marvel at before, and to appreciate\\

& &   the skills of the people who create them."The Modern Library has played a significant role in American cultural  life for the better part of a century. The series was founded\\
& &   in 1917 by the publishers Boni and Liveright and eight years later acquired by Bennett Cerf and Donald Klopfer. It provided the foundation for their next publishing venture,\\

& &   Random House. The Modern Library has been a staple of the American book trade, providing readers with affordable hardbound editions of important works of literature and \\
& & thought. For the Modern Library's seventy-fifth anniversary, Random House redesigned the series, restoring as its emblem the running torch-bearer created by Lucian Bernhard \\

&  & in 1925 and refurbishing jackets, bindings, and type, as well as inaugurating a new program of selecting titles. The Modern Library continues to provide the world's best \\

& & books, at the best prices. Tracy Kidder has written a new Introduction to this Modern Library edition.\\ \cline{2-3}

 % & ${\cal{M}} $ & \{"author":"TRACY KIDDER","publisher":"Modern Library"\}\\ \hline
& \multicolumn{1}{c}{\textbf{Actual Genre}:} & (Non-fiction, {Business \& Money, Computers \& Technology, History, Science \& Math })\\

\hline \hline
\rowcolor[HTML]{D9D9D9}
\multicolumn{3}{c}{\textcolor{blue}{\emph{(i)}} \textbf{9780803716988: Library Lil; Author: Suzanne Williams; Publisher: Dial Books}}\\
\hline 

\multirow{3}{*}{\includegraphics[width=0.04\linewidth, height=0.05\linewidth]{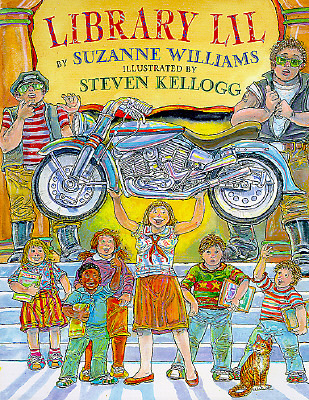}} & \multirow{2}{*}{\textbf{Blurb}:} & A formidable librarian makes readers not only out of the once resistant residents of her small town, but out of a tough-talking, television-watching motorcycle gang as well. \\
& & \\
\cline{2-3}
% & ${\cal{M}}$ & \{"author":"Suzanne Williams","publisher":"Dial Books"\}\\

% \hline
& \multicolumn{1}{l}{\textbf{Actual Genre}:} & (Fiction, \{Arts \& Photography, {Childrens\textquoteright} Book, Humor \& Entertainment, Meta Text, Sci-Fi\})\\

\hline \hline
\rowcolor[HTML]{D9D9D9}
\multicolumn{3}{c}{\textcolor{blue}{\emph{(j)}} \textbf{9780130255792: Understanding Movies; Author: Louis D. Giannetti; Publisher: Prentice Hall}}\\
\hline 
\multirow{5}{*}{\includegraphics[width=0.04\linewidth, height=0.05\linewidth]{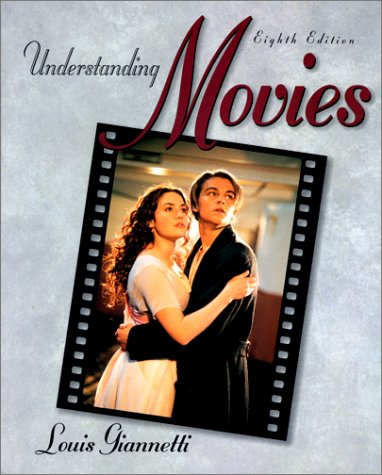}} & \multirow{4}{*}{\textbf{Blurb}:} & Designed to help movie watchers analyze films with precision and technical sophistication, this book focuses on formalism how the forms of the film (e.g., camera work, \\
& &  editing, photography, etc.) create meaning. It sheds light on how television and movies communicate, and the complex network of language systems they use. Chapter topics\\

& &    cover recent developments from all aspects of cinema, contemporary films, personalities in the field, photography, movement, editing, sound, acting, drama, story writing, and   \\ 

& & theory. For movie critics and fans alike.\\
\cline{2-3}

& \multicolumn{1}{l}{\textbf{Actual Genre}:} & (Non-fiction, \{Arts \& Photography, Press \& Media, Reference \& Language, Teen \& Young Adult\}) \\
\hline

\end{tabular}
\end{adjustbox}

\label{tab:heatmap_samples}

\end{table*}
\begin{figure*}[!hbt]
\centering

% \begin{adjustbox}{angle=90, height=1\textheight}
\begin{adjustbox}{width=0.88\textwidth} 
\begin{tabular}{cc|c|c|c|c|c|c|c|c|c|c|c|c|c|c|c|c|c|c|c|c|c|c|c|c|c|c|c|c|c|c|c|c}
\hline

\multicolumn{1}{c}{} & \multicolumn{1}{c|}{} & 
\multicolumn{2}{c|}{Level-1} & \multicolumn{30}{c}{Level-2 Classification} \\
\cline{3-34} 
%%%%%% Actual
\multicolumn{1}{c}{} & \multicolumn{1}{c|}{Class ID}  & NF & F & 1 & 2& 3 & 4& 5& 6 & 7 & 8 & 9 & 10 & 11 & 12 & 13 & 14 & 15 & 16 & 17 & 18 & 19 & 20 & 21 & 22 & 23 & 24 & 25 & 26 & 27 & 28 & 29 & 30 \\ 
% \cline{2-34} 
\hline \hline 

\multirow{10}{*}{\textbf{\rotatebox{90}{\underline{Ground-truth}}}} & \textcolor{blue}{\emph{(a)}} & \cellcolor[gray]{0} & \cellcolor[gray]{1} & \cellcolor[gray]{1.00000} & \cellcolor[gray]{1.00000} & \cellcolor[gray]{0.00000} & \cellcolor[gray]{1.00000} & \cellcolor[gray]{0.00000} & \cellcolor[gray]{0.00000} & \cellcolor[gray]{1.00000} & \cellcolor[gray]{0.00000} & \cellcolor[gray]{0.00000} & \cellcolor[gray]{1.00000} & \cellcolor[gray]{0.00000} & \cellcolor[gray]{0.00000} & \cellcolor[gray]{0.00000} & \cellcolor[gray]{0.00000} & \cellcolor[gray]{0.00000} & \cellcolor[gray]{1.00000} & \cellcolor[gray]{0.00000} & \cellcolor[gray]{0.00000} & \cellcolor[gray]{0.00000} & \cellcolor[gray]{0.00000} & \cellcolor[gray]{0.00000} & \cellcolor[gray]{0.00000} & \cellcolor[gray]{0.00000} & \cellcolor[gray]{0.00000} & \cellcolor[gray]{0.00000} & \cellcolor[gray]{0.00000} & \cellcolor[gray]{0.00000} & \cellcolor[gray]{0.00000} & \cellcolor[gray]{0.00000} & \cellcolor[gray]{0.00000} \\ \cline{2-34} 

 & \textcolor{blue}{\emph{(b)}} & \cellcolor[gray]{0} & \cellcolor[gray]{1} & \cellcolor[gray]{0.00000} & \cellcolor[gray]{0.00000} & \cellcolor[gray]{0.00000} & \cellcolor[gray]{0.00000} & \cellcolor[gray]{1.00000} & \cellcolor[gray]{0.00000} & \cellcolor[gray]{0.00000} & \cellcolor[gray]{0.00000} & \cellcolor[gray]{0.00000} & \cellcolor[gray]{0.00000} & \cellcolor[gray]{0.00000} & \cellcolor[gray]{0.00000} & \cellcolor[gray]{0.00000} & \cellcolor[gray]{0.00000} & \cellcolor[gray]{0.00000} & \cellcolor[gray]{0.00000} & \cellcolor[gray]{0.00000} & \cellcolor[gray]{0.00000} & \cellcolor[gray]{0.00000} & \cellcolor[gray]{0.00000} & \cellcolor[gray]{0.00000} & \cellcolor[gray]{0.00000} & \cellcolor[gray]{1.00000} & \cellcolor[gray]{0.00000} & \cellcolor[gray]{0.00000} & \cellcolor[gray]{0.00000} & \cellcolor[gray]{0.00000} & \cellcolor[gray]{0.00000} & \cellcolor[gray]{1.00000} & \cellcolor[gray]{0.00000} \\ \cline{2-34} 
 
 & \textcolor{blue}{\emph{(c)}} & \cellcolor[gray]{1} & \cellcolor[gray]{0} & \cellcolor[gray]{0.00000} & \cellcolor[gray]{0.00000} & \cellcolor[gray]{0.00000} & \cellcolor[gray]{0.00000} & \cellcolor[gray]{0.00000} & \cellcolor[gray]{0.00000} & \cellcolor[gray]{1.00000} & \cellcolor[gray]{0.00000} & \cellcolor[gray]{0.00000} & \cellcolor[gray]{0.00000} & \cellcolor[gray]{0.00000} & \cellcolor[gray]{1.00000} & \cellcolor[gray]{0.00000} & \cellcolor[gray]{0.00000} & \cellcolor[gray]{0.00000} & \cellcolor[gray]{0.00000} & \cellcolor[gray]{0.00000} & \cellcolor[gray]{1.00000} & \cellcolor[gray]{0.00000} & \cellcolor[gray]{0.00000} & \cellcolor[gray]{0.00000} & \cellcolor[gray]{1.00000} & \cellcolor[gray]{0.00000} & \cellcolor[gray]{0.00000} & \cellcolor[gray]{1.00000} & \cellcolor[gray]{0.00000} & \cellcolor[gray]{0.00000} & \cellcolor[gray]{0.00000} & \cellcolor[gray]{0.00000} & \cellcolor[gray]{0.00000} \\ \cline{2-34} 
 
 & \textcolor{blue}{\emph{(d)}} & \cellcolor[gray]{1} & \cellcolor[gray]{0} & \cellcolor[gray]{1.00000} & \cellcolor[gray]{0.00000} & \cellcolor[gray]{0.00000} & \cellcolor[gray]{0.00000} & \cellcolor[gray]{0.00000} & \cellcolor[gray]{0.00000} & \cellcolor[gray]{0.00000} & \cellcolor[gray]{0.00000} & \cellcolor[gray]{0.00000} & \cellcolor[gray]{0.00000} & \cellcolor[gray]{0.00000} & \cellcolor[gray]{0.00000} & \cellcolor[gray]{0.00000} & \cellcolor[gray]{0.00000} & \cellcolor[gray]{0.00000} & \cellcolor[gray]{0.00000} & \cellcolor[gray]{0.00000} & \cellcolor[gray]{0.00000} & \cellcolor[gray]{0.00000} & \cellcolor[gray]{0.00000} & \cellcolor[gray]{0.00000} & \cellcolor[gray]{0.00000} & \cellcolor[gray]{0.00000} & \cellcolor[gray]{0.00000} & \cellcolor[gray]{0.00000} & \cellcolor[gray]{0.00000} & \cellcolor[gray]{0.00000} & \cellcolor[gray]{0.00000} & \cellcolor[gray]{0.00000} & \cellcolor[gray]{1.00000} \\ \cline{2-34} 
 
 & \textcolor{blue}{\emph{(e)}} & \cellcolor[gray]{1} & \cellcolor[gray]{0} & \cellcolor[gray]{0.00000} & \cellcolor[gray]{0.00000} & \cellcolor[gray]{1.00000} & \cellcolor[gray]{0.00000} & \cellcolor[gray]{0.00000} & \cellcolor[gray]{0.00000} & \cellcolor[gray]{0.00000} & \cellcolor[gray]{0.00000} & \cellcolor[gray]{0.00000} & \cellcolor[gray]{0.00000} & \cellcolor[gray]{0.00000} & \cellcolor[gray]{0.00000} & \cellcolor[gray]{0.00000} & \cellcolor[gray]{1.00000} & \cellcolor[gray]{0.00000} & \cellcolor[gray]{0.00000} & \cellcolor[gray]{0.00000} & \cellcolor[gray]{0.00000} & \cellcolor[gray]{0.00000} & \cellcolor[gray]{1.00000} & \cellcolor[gray]{0.00000} & \cellcolor[gray]{0.00000} & \cellcolor[gray]{0.00000} & \cellcolor[gray]{0.00000} & \cellcolor[gray]{1.00000} & \cellcolor[gray]{0.00000} & \cellcolor[gray]{0.00000} & \cellcolor[gray]{0.00000} & \cellcolor[gray]{0.00000} & \cellcolor[gray]{0.00000} \\ \cline{2-34}
 
 & \textcolor{blue}{\emph{(f)}} & \cellcolor[gray]{1} & \cellcolor[gray]{0} & \cellcolor[gray]{0.00000} & \cellcolor[gray]{0.00000} & \cellcolor[gray]{0.00000} & \cellcolor[gray]{0.00000} & \cellcolor[gray]{0.00000} & \cellcolor[gray]{0.00000} & \cellcolor[gray]{0.00000} & \cellcolor[gray]{0.00000} & \cellcolor[gray]{1.00000} & \cellcolor[gray]{0.00000} & \cellcolor[gray]{0.00000} & \cellcolor[gray]{0.00000} & \cellcolor[gray]{0.00000} & \cellcolor[gray]{0.00000} & \cellcolor[gray]{0.00000} & \cellcolor[gray]{0.00000} & \cellcolor[gray]{1.00000} & \cellcolor[gray]{0.00000} & \cellcolor[gray]{0.00000} & \cellcolor[gray]{0.00000} & \cellcolor[gray]{0.00000} & \cellcolor[gray]{1.00000} & \cellcolor[gray]{0.00000} & \cellcolor[gray]{0.00000} & \cellcolor[gray]{0.00000} & \cellcolor[gray]{1.00000} & \cellcolor[gray]{0.00000} & \cellcolor[gray]{1.00000} & \cellcolor[gray]{0.00000} & \cellcolor[gray]{0.00000} \\ \cline{2-34} 
 
 & \textcolor{blue}{\emph{(g)}} & \cellcolor[gray]{0} & \cellcolor[gray]{1} & \cellcolor[gray]{0.00000} & \cellcolor[gray]{0.00000} & \cellcolor[gray]{0.00000} & \cellcolor[gray]{0.00000} & \cellcolor[gray]{0.00000} & \cellcolor[gray]{0.00000} & \cellcolor[gray]{0.00000} & \cellcolor[gray]{0.00000} & \cellcolor[gray]{0.00000} & \cellcolor[gray]{0.00000} & \cellcolor[gray]{1.00000} & \cellcolor[gray]{0.00000} & \cellcolor[gray]{1.00000} & \cellcolor[gray]{0.00000} & \cellcolor[gray]{0.00000} & \cellcolor[gray]{0.00000} & \cellcolor[gray]{0.00000} & \cellcolor[gray]{0.00000} & \cellcolor[gray]{0.00000} & \cellcolor[gray]{0.00000} & \cellcolor[gray]{0.00000} & \cellcolor[gray]{0.00000} & \cellcolor[gray]{1.00000} & \cellcolor[gray]{0.00000} & \cellcolor[gray]{0.00000} & \cellcolor[gray]{0.00000} & \cellcolor[gray]{0.00000} & \cellcolor[gray]{0.00000} & \cellcolor[gray]{0.00000} & \cellcolor[gray]{0.00000} \\ \cline{2-34} 
 
 &\textcolor{blue}{\emph{(h)}} & \cellcolor[gray]{1} & \cellcolor[gray]{0} & \cellcolor[gray]{0.00000} & \cellcolor[gray]{0.00000} & \cellcolor[gray]{1.00000} & \cellcolor[gray]{0.00000} & \cellcolor[gray]{0.00000} & \cellcolor[gray]{1.00000} & \cellcolor[gray]{0.00000} & \cellcolor[gray]{0.00000} & \cellcolor[gray]{0.00000} & \cellcolor[gray]{0.00000} & \cellcolor[gray]{0.00000} & \cellcolor[gray]{0.00000} & \cellcolor[gray]{1.00000} & \cellcolor[gray]{0.00000} & \cellcolor[gray]{0.00000} & \cellcolor[gray]{0.00000} & \cellcolor[gray]{0.00000} & \cellcolor[gray]{0.00000} & \cellcolor[gray]{0.00000} & \cellcolor[gray]{0.00000} & \cellcolor[gray]{0.00000} & \cellcolor[gray]{0.00000} & \cellcolor[gray]{0.00000} & \cellcolor[gray]{1.00000} & \cellcolor[gray]{0.00000} & \cellcolor[gray]{0.00000} & \cellcolor[gray]{0.00000} & \cellcolor[gray]{0.00000} & \cellcolor[gray]{0.00000} & \cellcolor[gray]{0.00000} \\ \cline{2-34} 
 & \textcolor{blue}{\emph{(i)}} & \cellcolor[gray]{0} & \cellcolor[gray]{1} & \cellcolor[gray]{0.00000} & \cellcolor[gray]{1.00000} & \cellcolor[gray]{0.00000} & \cellcolor[gray]{1.00000} & \cellcolor[gray]{0.00000} & \cellcolor[gray]{0.00000} & \cellcolor[gray]{0.00000} & \cellcolor[gray]{0.00000} & \cellcolor[gray]{0.00000} & \cellcolor[gray]{0.00000} & \cellcolor[gray]{0.00000} & \cellcolor[gray]{0.00000} & \cellcolor[gray]{0.00000} & \cellcolor[gray]{0.00000} & \cellcolor[gray]{1.00000} & \cellcolor[gray]{0.00000} & \cellcolor[gray]{0.00000} & \cellcolor[gray]{0.00000} & \cellcolor[gray]{1.00000} & \cellcolor[gray]{0.00000} & \cellcolor[gray]{0.00000} & \cellcolor[gray]{0.00000} & \cellcolor[gray]{0.00000} & \cellcolor[gray]{0.00000} & \cellcolor[gray]{0.00000} & \cellcolor[gray]{0.00000} & \cellcolor[gray]{0.00000} & \cellcolor[gray]{0.00000} & \cellcolor[gray]{1.00000} & \cellcolor[gray]{0.00000} \\ \cline{2-34} 
 & \textcolor{blue}{\emph{(j)}} & \cellcolor[gray]{1} & \cellcolor[gray]{0} & \cellcolor[gray]{0.00000} & \cellcolor[gray]{1.00000} & \cellcolor[gray]{0.00000} & \cellcolor[gray]{0.00000} & \cellcolor[gray]{0.00000} & \cellcolor[gray]{0.00000} & \cellcolor[gray]{0.00000} & \cellcolor[gray]{0.00000} & \cellcolor[gray]{0.00000} & \cellcolor[gray]{0.00000} & \cellcolor[gray]{0.00000} & \cellcolor[gray]{0.00000} & \cellcolor[gray]{0.00000} & \cellcolor[gray]{0.00000} & \cellcolor[gray]{0.00000} & \cellcolor[gray]{0.00000} & \cellcolor[gray]{0.00000} & \cellcolor[gray]{0.00000} & \cellcolor[gray]{0.00000} & \cellcolor[gray]{0.00000} & \cellcolor[gray]{1.00000} & \cellcolor[gray]{1.00000} & \cellcolor[gray]{0.00000} & \cellcolor[gray]{0.00000} & \cellcolor[gray]{0.00000} & \cellcolor[gray]{0.00000} & \cellcolor[gray]{1.00000} & \cellcolor[gray]{0.00000} & \cellcolor[gray]{0.00000} & \cellcolor[gray]{0.00000} \\ 
 \hline \hline

%%%%%%%% Predicted

\multirow{10}{*}{\textbf{\rotatebox{90}{\underline{Predicted score}}}} & \textcolor{blue}{\emph{(a)}} & \cellcolor[gray]{0.00044} & \cellcolor[gray]{0.99956} & \cellcolor[gray]{0.99476} & \cellcolor[gray]{0.99909} & \cellcolor[gray]{0.00001} & \cellcolor[gray]{0.99997} & \cellcolor[gray]{0.00083} & \cellcolor[gray]{0.00002} & \cellcolor[gray]{0.94047} & \cellcolor[gray]{0.00000} & \cellcolor[gray]{0.00563} & \cellcolor[gray]{0.99830} & \cellcolor[gray]{0.00000} & \cellcolor[gray]{0.00056} & \cellcolor[gray]{0.00066} & \cellcolor[gray]{0.00122} & \cellcolor[gray]{0.03674} & \cellcolor[gray]{0.99246} & \cellcolor[gray]{0.00000} & \cellcolor[gray]{0.00550} & \cellcolor[gray]{0.00044} & \cellcolor[gray]{0.00000} & \cellcolor[gray]{0.00014} & \cellcolor[gray]{0.00006} & \cellcolor[gray]{0.00023} & \cellcolor[gray]{0.00008} & \cellcolor[gray]{0.00006} & \cellcolor[gray]{0.00002} & \cellcolor[gray]{0.00533} & \cellcolor[gray]{0.00015} & \cellcolor[gray]{0.03099} & \cellcolor[gray]{0.00000} \\ \cline{2-34} 

 & \textcolor{blue}{\emph{(b)}} & \cellcolor[gray]{0.00016} & \cellcolor[gray]{0.99984} & \cellcolor[gray]{0.00133} & \cellcolor[gray]{0.01118} & \cellcolor[gray]{0.00027} & \cellcolor[gray]{0.00066} & \cellcolor[gray]{0.99569} & \cellcolor[gray]{0.04551} & \cellcolor[gray]{0.00032} & \cellcolor[gray]{0.00000} & \cellcolor[gray]{0.00000} & \cellcolor[gray]{0.00001} & \cellcolor[gray]{0.00002} & \cellcolor[gray]{0.00000} & \cellcolor[gray]{0.03169} & \cellcolor[gray]{0.00016} & \cellcolor[gray]{0.02745} & \cellcolor[gray]{0.00027} & \cellcolor[gray]{0.00545} & \cellcolor[gray]{0.00022} & \cellcolor[gray]{0.00001} & \cellcolor[gray]{0.00010} & \cellcolor[gray]{0.00255} & \cellcolor[gray]{0.00001} & \cellcolor[gray]{0.99160} & \cellcolor[gray]{0.00353} & \cellcolor[gray]{0.00000} & \cellcolor[gray]{0.00004} & \cellcolor[gray]{0.10041} & \cellcolor[gray]{0.00222} & \cellcolor[gray]{0.97165} & \cellcolor[gray]{0.00000} \\ \cline{2-34} 
 
 & \textcolor{blue}{\emph{(c)}} & \cellcolor[gray]{0.99994} & \cellcolor[gray]{0.00006} & \cellcolor[gray]{0.00007} & \cellcolor[gray]{0.00004} & \cellcolor[gray]{0.00007} & \cellcolor[gray]{0.03481} & \cellcolor[gray]{0.00017} & \cellcolor[gray]{0.00009} & \cellcolor[gray]{0.97895} & \cellcolor[gray]{0.00046} & \cellcolor[gray]{0.00542} & \cellcolor[gray]{0.01889} & \cellcolor[gray]{0.00044} & \cellcolor[gray]{0.99680} & \cellcolor[gray]{0.00002} & \cellcolor[gray]{0.00266} & \cellcolor[gray]{0.00002} & \cellcolor[gray]{0.00476} & \cellcolor[gray]{0.01359} & \cellcolor[gray]{0.82687} & \cellcolor[gray]{0.00702} & \cellcolor[gray]{0.00038} & \cellcolor[gray]{0.00001} & \cellcolor[gray]{0.99791} & \cellcolor[gray]{0.00092} & \cellcolor[gray]{0.00011} & \cellcolor[gray]{0.99844} & \cellcolor[gray]{0.00979} & \cellcolor[gray]{0.00001} & \cellcolor[gray]{0.00032} & \cellcolor[gray]{0.00000} & \cellcolor[gray]{0.00001} \\ \cline{2-34} 
 
 & \textcolor{blue}{\emph{(d)}} & \cellcolor[gray]{0.99635} & \cellcolor[gray]{0.00365} & \cellcolor[gray]{0.99472} & \cellcolor[gray]{0.00016} & \cellcolor[gray]{0.00009} & \cellcolor[gray]{0.00001} & \cellcolor[gray]{0.00002} & \cellcolor[gray]{0.00004} & \cellcolor[gray]{0.00303} & \cellcolor[gray]{0.00000} & \cellcolor[gray]{0.00361} & \cellcolor[gray]{0.00086} & \cellcolor[gray]{0.00008} & \cellcolor[gray]{0.00000} & \cellcolor[gray]{0.00635} & \cellcolor[gray]{0.00004} & \cellcolor[gray]{0.00166} & \cellcolor[gray]{0.00040} & \cellcolor[gray]{0.00005} & \cellcolor[gray]{0.00005} & \cellcolor[gray]{0.01653} & \cellcolor[gray]{0.00047} & \cellcolor[gray]{0.00008} & \cellcolor[gray]{0.00086} & \cellcolor[gray]{0.00274} & \cellcolor[gray]{0.00353} & \cellcolor[gray]{0.00000} & \cellcolor[gray]{0.00002} & \cellcolor[gray]{0.00000} & \cellcolor[gray]{0.00001} & \cellcolor[gray]{0.00000} & \cellcolor[gray]{0.99131} \\ \cline{2-34} 
 
 & \textcolor{blue}{\emph{(e)}} & \cellcolor[gray]{0.99991} & \cellcolor[gray]{0.00009} & \cellcolor[gray]{0.00002} & \cellcolor[gray]{0.00099} & \cellcolor[gray]{0.99969} & \cellcolor[gray]{0.00000} & \cellcolor[gray]{0.00419} & \cellcolor[gray]{0.01303} & \cellcolor[gray]{0.00000} & \cellcolor[gray]{0.00003} & \cellcolor[gray]{0.00002} & \cellcolor[gray]{0.04246} & \cellcolor[gray]{0.00810} & \cellcolor[gray]{0.00004} & \cellcolor[gray]{0.00268} & \cellcolor[gray]{0.98886} & \cellcolor[gray]{0.00000} & \cellcolor[gray]{0.00006} & \cellcolor[gray]{0.00004} & \cellcolor[gray]{0.00378} & \cellcolor[gray]{0.00823} & \cellcolor[gray]{0.90046} & \cellcolor[gray]{0.00000} & \cellcolor[gray]{0.00545} & \cellcolor[gray]{0.00357} & \cellcolor[gray]{0.00013} & \cellcolor[gray]{0.99689} & \cellcolor[gray]{0.00008} & \cellcolor[gray]{0.00005} & \cellcolor[gray]{0.00000} & \cellcolor[gray]{0.00000} & \cellcolor[gray]{0.00358} \\ \cline{2-34} 
 
 & \textcolor{blue}{\emph{(f)}} & \cellcolor[gray]{0.99993} & \cellcolor[gray]{0.00007} & \cellcolor[gray]{0.00021} & \cellcolor[gray]{0.00002} & \cellcolor[gray]{0.00009} & \cellcolor[gray]{0.00027} & \cellcolor[gray]{0.00241} & \cellcolor[gray]{0.00001} & \cellcolor[gray]{0.02858} & \cellcolor[gray]{0.01158} & \cellcolor[gray]{0.93981} & \cellcolor[gray]{0.00048} & \cellcolor[gray]{0.00162} & \cellcolor[gray]{0.03215} & \cellcolor[gray]{0.00400} & \cellcolor[gray]{0.00079} & \cellcolor[gray]{0.00082} & \cellcolor[gray]{0.00392} & \cellcolor[gray]{0.91136} & \cellcolor[gray]{0.00001} & \cellcolor[gray]{0.00181} & \cellcolor[gray]{0.00202} & \cellcolor[gray]{0.00007} & \cellcolor[gray]{0.99415} & \cellcolor[gray]{0.00998} & \cellcolor[gray]{0.00002} & \cellcolor[gray]{0.00505} & \cellcolor[gray]{0.99881} & \cellcolor[gray]{0.01750} & \cellcolor[gray]{0.97146} & \cellcolor[gray]{0.00000} & \cellcolor[gray]{0.11416} \\ \cline{2-34} 
 
 & \textcolor{blue}{\emph{(g)}} & \cellcolor[gray]{0.00008} & \cellcolor[gray]{0.99992} & \cellcolor[gray]{0.00213} & \cellcolor[gray]{0.04993} & \cellcolor[gray]{0.00258} & \cellcolor[gray]{0.00845} & \cellcolor[gray]{0.00705} & \cellcolor[gray]{0.00096} & \cellcolor[gray]{0.00517} & \cellcolor[gray]{0.00225} & \cellcolor[gray]{0.00287} & \cellcolor[gray]{0.42612} & \cellcolor[gray]{0.71277} & \cellcolor[gray]{0.01147} & \cellcolor[gray]{0.92822} & \cellcolor[gray]{0.00258} & \cellcolor[gray]{0.17138} & \cellcolor[gray]{0.07084} & \cellcolor[gray]{0.00624} & \cellcolor[gray]{0.04806} & \cellcolor[gray]{0.03481} & \cellcolor[gray]{0.04279} & \cellcolor[gray]{0.01641} & \cellcolor[gray]{0.00774} & \cellcolor[gray]{0.85877} & \cellcolor[gray]{0.11464} & \cellcolor[gray]{0.00673} & \cellcolor[gray]{0.00154} & \cellcolor[gray]{0.05980} & \cellcolor[gray]{0.00338} & \cellcolor[gray]{0.01469} & \cellcolor[gray]{0.00000} \\ \cline{2-34} 
 & \textcolor{blue}{\emph{(h)}} & \cellcolor[gray]{0.99975} & \cellcolor[gray]{0.00025} & \cellcolor[gray]{0.00133} & \cellcolor[gray]{0.00295} & \cellcolor[gray]{0.92140} & \cellcolor[gray]{0.01267} & \cellcolor[gray]{0.01531} & \cellcolor[gray]{0.87444} & \cellcolor[gray]{0.04635} & \cellcolor[gray]{0.00045} & \cellcolor[gray]{0.00879} & \cellcolor[gray]{0.00264} & \cellcolor[gray]{0.01290} & \cellcolor[gray]{0.00145} & \cellcolor[gray]{0.98127} & \cellcolor[gray]{0.33684} & \cellcolor[gray]{0.00039} & \cellcolor[gray]{0.05179} & \cellcolor[gray]{0.00029} & \cellcolor[gray]{0.05201} & \cellcolor[gray]{0.01190} & \cellcolor[gray]{0.00225} & \cellcolor[gray]{0.06651} & \cellcolor[gray]{0.00788} & \cellcolor[gray]{0.00283} & \cellcolor[gray]{0.82674} & \cellcolor[gray]{0.00126} & \cellcolor[gray]{0.00023} & \cellcolor[gray]{0.24525} & \cellcolor[gray]{0.03039} & \cellcolor[gray]{0.00000} & \cellcolor[gray]{0.18526} \\ \cline{2-34} 
 & \textcolor{blue}{\emph{(i)}} & \cellcolor[gray]{0.00315} & \cellcolor[gray]{0.99685} & \cellcolor[gray]{0.00671} & \cellcolor[gray]{0.80333} & \cellcolor[gray]{0.00000} & \cellcolor[gray]{0.85072} & \cellcolor[gray]{0.00034} & \cellcolor[gray]{0.00014} & \cellcolor[gray]{0.00026} & \cellcolor[gray]{0.00000} & \cellcolor[gray]{0.00001} & \cellcolor[gray]{0.00009} & \cellcolor[gray]{0.00004} & \cellcolor[gray]{0.00500} & \cellcolor[gray]{0.00000} & \cellcolor[gray]{0.00001} & \cellcolor[gray]{0.99992} & \cellcolor[gray]{0.00002} & \cellcolor[gray]{0.03822} & \cellcolor[gray]{0.00001} & \cellcolor[gray]{0.99222} & \cellcolor[gray]{0.00018} & \cellcolor[gray]{0.00008} & \cellcolor[gray]{0.00030} & \cellcolor[gray]{0.00001} & \cellcolor[gray]{0.00000} & \cellcolor[gray]{0.00000} & \cellcolor[gray]{0.01542} & \cellcolor[gray]{0.04668} & \cellcolor[gray]{0.00000} & \cellcolor[gray]{0.99957} & \cellcolor[gray]{0.00000} \\ \cline{2-34} 
 & \textcolor{blue}{\emph{(j)}} & \cellcolor[gray]{0.99802} & \cellcolor[gray]{0.00198} & \cellcolor[gray]{0.01750} & \cellcolor[gray]{0.97278} & \cellcolor[gray]{0.05179} & \cellcolor[gray]{0.17395} & \cellcolor[gray]{0.00997} & \cellcolor[gray]{0.05670} & \cellcolor[gray]{0.00747} & \cellcolor[gray]{0.13790} & \cellcolor[gray]{0.00693} & \cellcolor[gray]{0.00516} & \cellcolor[gray]{0.07648} & \cellcolor[gray]{0.00456} & \cellcolor[gray]{0.07431} & \cellcolor[gray]{0.08559} & \cellcolor[gray]{0.14760} & \cellcolor[gray]{0.01880} & \cellcolor[gray]{0.00740} & \cellcolor[gray]{0.01624} & \cellcolor[gray]{0.01769} & \cellcolor[gray]{0.00190} & \cellcolor[gray]{0.66830} & \cellcolor[gray]{0.96815} & \cellcolor[gray]{0.07242} & \cellcolor[gray]{0.15810} & \cellcolor[gray]{0.13284} & \cellcolor[gray]{0.00079} & \cellcolor[gray]{0.68137} & \cellcolor[gray]{0.00128} & \cellcolor[gray]{0.00000} & \cellcolor[gray]{0.00036} \\ 
 \hline

 \multicolumn{34}{r}{L-1: Level-1 classification, NF: \textit{non-fiction}, F: \textit{fiction}}
\end{tabular}
\end{adjustbox}
\caption{Ground-truth and IMaGINe-predicted confidence score heat-map encodings in gray color code}
\label{tab:heatmap}
\end{figure*}

\clearpage
