# Supplementary material for: Adaptive Data-Resilient Multi-Modal Hierarchical Multi-Label Book Genre Identification
Source: arXiv:2505.03839 source file (2025-10-18)
Supplement: Supplementary file 7 [file 7appendix_misprediction.tex]

\section{Performance Stagnation Analysis of IMAGINE}

\noindent
In this section, we first explore the quantitative analysis for genre indistinguishability and then the qualitative analysis for misprediction by IMAGINE.

\subsection{Qualitative Analysis for Misprediction due to insufficient information on samples:}
\noindent
Our analysis of misprediction indicates that insufficient information on some samples is the one potential cause of these errors. Even human evaluators may find it challenging to determine genres from some samples accurately. Table \ref{tab:misprediction_sample} presents examples of IMAGINE's misprediction.
It is notable that some of the samples can easily misinterpreted in terms of actual genre due to insufficient information on description text and misleading coverage images (e.g., Table \ref{tab:misprediction_sample}: \emph{(a), (b), (c), (d)}).

Based on the above analysis, we recommend providing detailed blurb and redesigning the cover page of these books to better reflect their true genres. These will help to prevent misunderstandings, attract the right audience, and ensure that viewers engage with content that aligns with their interests.

\begin{table}[!hbt]
\centering
\caption{Misprediction due to insufficient information on samples}
\begin{adjustbox}{width=0.5\textwidth}
% \begin{adjustbox}{angle=90, height=1\textheight}
% \footnotesize
\begin{tabular}{c|ll}%p{0.9\textwidth}}
% \multicolumn{3}{c}{(a) Samples for heatmap analysis}\\
\hline \hline

\hline \hline
\rowcolor[HTML]{D9D9D9}
\multicolumn{3}{c}{\textbf{{\emph{(a)}} 9780760705902: The awakening; Author: Kate Chopin; Publisher: Barnes \& Noble Books}}\\
\hline \hline
& \\ [\dimexpr-\normalbaselineskip+1.5pt]

\multirow{6}{*}{\includegraphics[width=0.15\linewidth]{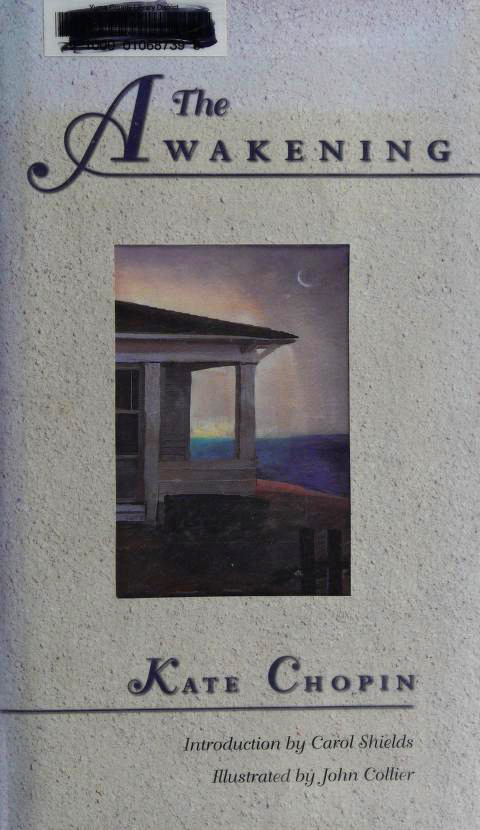}} & \multirow{2}{*}{\textbf{Blurb}:} & \multirow{2}{*}{The Awakening}\\ %\cline{2-3}
& & \\ \cline{2-3}
% & ${\cal{M}}$ & \{"author":"Kate Chopin","publisher":"Barnes \& Noble Books"\}\\ \hline
& \multirow{2}{*}{\textbf{Actual Genre}:} & \multirow{2}{*}{(Fiction, \{History, Humanities, Literature, Teen \& Young Adult\})}\\ %\cline{2-3}
& & \\ \cline{2-3}
& \multirow{2}{*}{\textbf{Predicted Genre}:} & \multirow{2}{*}{(Fiction, \{Arts \& Photography, Environment \& Plant, Literature\})}\\
& & \\

\hline \hline
\rowcolor[HTML]{D9D9D9}
\multicolumn{3}{c}{\textbf{{\emph{(b)}} 9780826400475: Pedagogy of the oppressed; Author: Paulo Freire; Publisher: Continuum}}\\
\hline \hline
& \\ [\dimexpr-\normalbaselineskip+1.5pt]

\multirow{6}{*}{\includegraphics[width=0.15\linewidth]{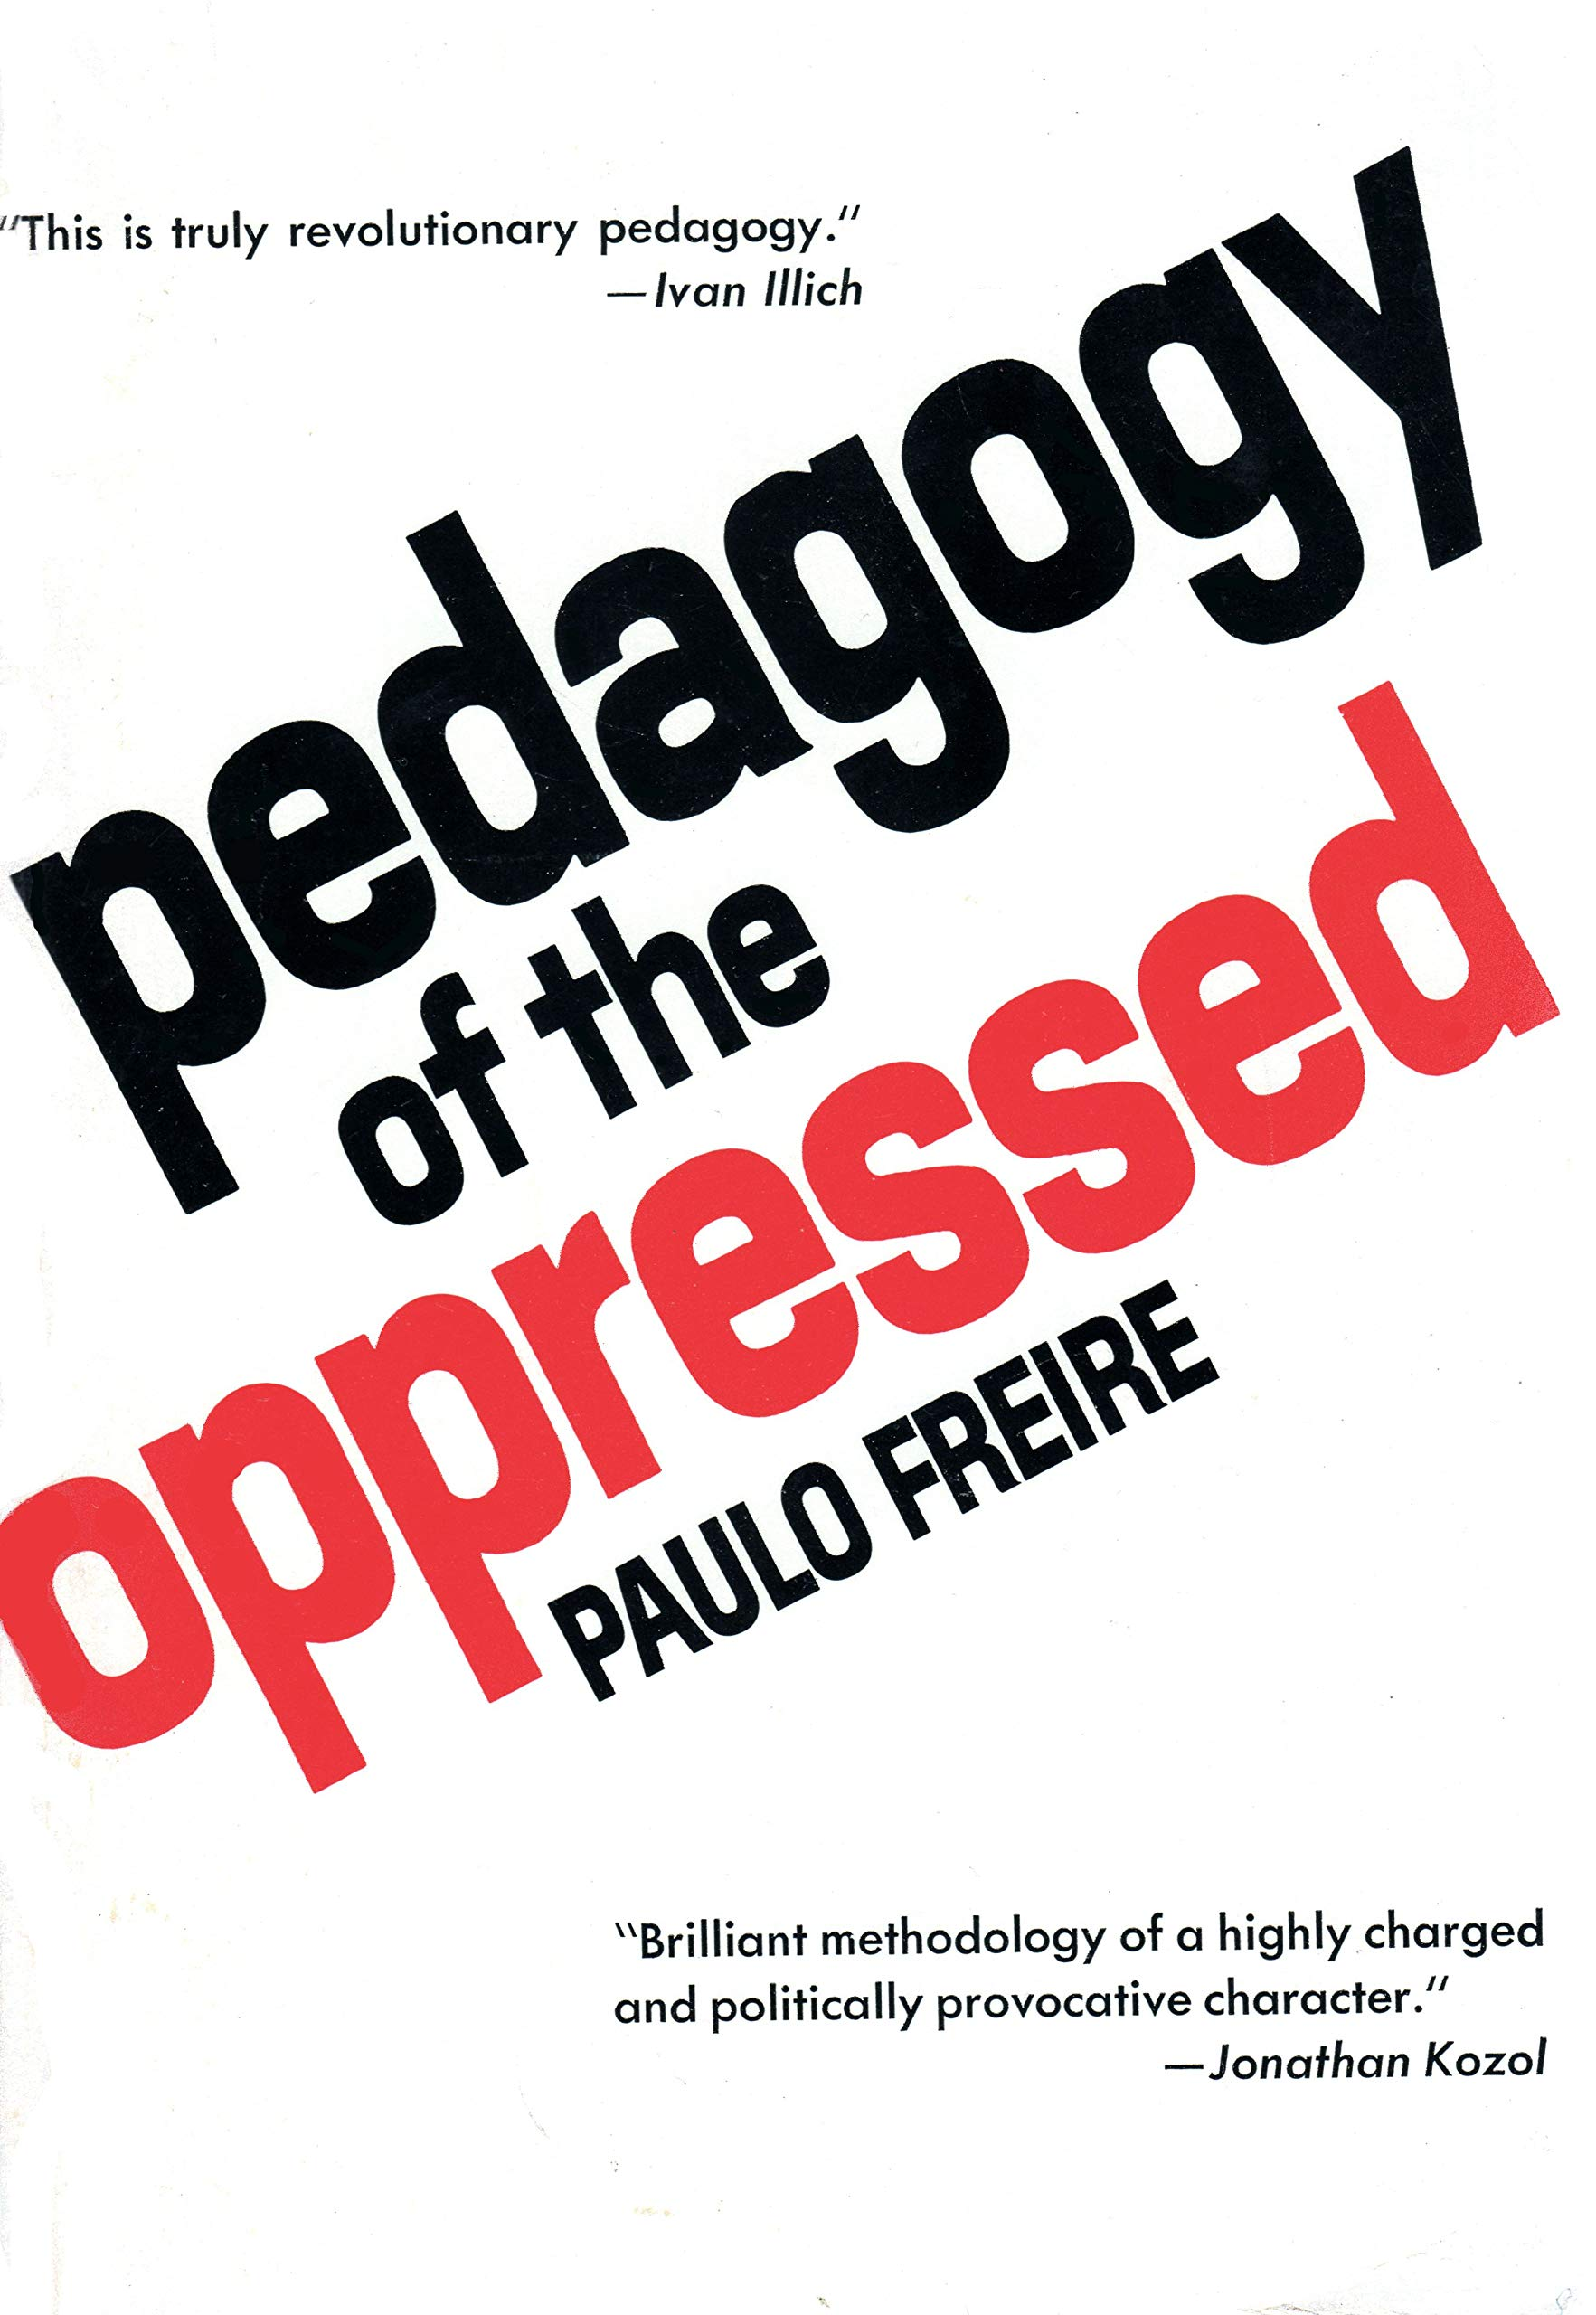}} & \multirow{2}{*}{\textbf{Blurb}:} & \multirow{2}{*}{TSIGNED COPY BY THE AUTHOR} \\ 
& & \\
\cline{2-3}

%& ${\cal{M}}$ & \{"author":"Paulo Freire","publisher":"Continuum"\}\\ \hline
& \multirow{2}{*}{\textbf{Actual Genre}:} & \multirow{2}{*}{(Non-fiction, \{Humanities\})}\\ 
& & \\
\cline{2-3}
& \multirow{2}{*}{\textbf{Predicted Genre}:} & \multirow{2}{*}{(Non-fiction, \{Science \& Math \& Mathematics\})} \\
& & \\

\hline \hline
\rowcolor[HTML]{D9D9D9}
\multicolumn{3}{c}{\textbf{{\emph{(c)}} 9788420478722: LA Caverna De Las Ideas; Author: Jose Carlos Somoza; Publisher: Alfaguara}}\\
\hline \hline

\multirow{6}{*}{\includegraphics[width=0.15\linewidth]{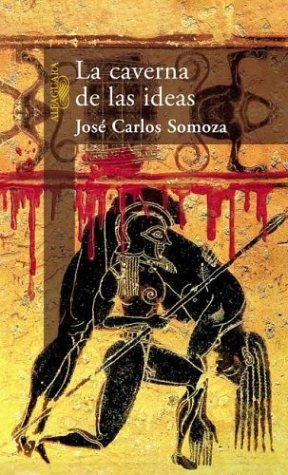}} & \multirow{2}{*}{\textbf{Blurb}:} & \multirow{2}{*}{Book by Jose Carlos Somoza} \\
& &  \\ \cline{2-3}

% & ${\cal{M}}$ & \{"author":"Jose Carlos Somoza","publisher":"Aguilar"\}\\
% \hline

& \multirow{2}{*}{\textbf{Actual Genre}:} & \multirow{2}{*}{(Fiction, \{History, Humanities, Literature, Mystery \& Thriller \& Suspense \& Horror\})}\\
& &  \\ \cline{2-3}
& \multirow{2}{*}{\textbf{Predicted Genre}:} & \multirow{2}{*}{(Fiction, \{Arts \& Photography, Literature, Reference \& Language, Sci-Fi\})} \\
& &  \\

\hline \hline
\rowcolor[HTML]{D9D9D9}
\multicolumn{3}{c}{\textbf{{\emph{(d)}} 9781571740601: Gooberz; Author: Linda Goodman; Publisher: Hampton Roads Publishing Company}}\\
\hline \hline

\multirow{6}{*}{\includegraphics[width=0.15\linewidth]{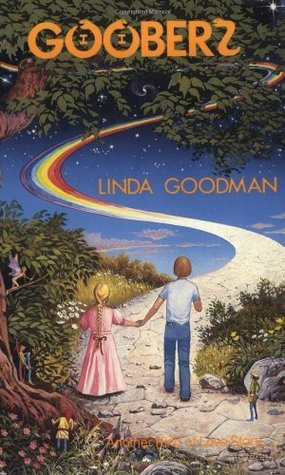}} & \multirow{2}{*}{\textbf{Blurb}:} & \multirow{2}{*}{Paperback} \\
& & \\
\cline{2-3}
% & ${\cal{M}}$ & \{"author":"Linda Goodman","publisher":"Hampton Roads Publishing Company"\}\\
% \hline
& \multirow{2}{*}{\textbf{Actual Genre}:} & \multirow{2}{*}{(Fiction, \{Literature, Mythology \& Religion \& Spirituality\})}\\
& & \\
\cline{2-3}
& \multirow{2}{*}{\textbf{Predicted Genre}:} & \multirow{2}{*}{(Fiction, \{Arts \& Photography, Literature, Sci-Fi\})}\\
& & \\

\hline

% \multicolumn{3}{r}{${\cal{I}}$: Coverpage Image, ${\cal{T}}$: Description Text, ${\cal{M}}$: Metadata}
\end{tabular}
\end{adjustbox}

\label{tab:misprediction_sample}

\end{table}

\begin{table*}[]
\centering
\caption{Fiction genre indistinguishability analysis}

% \begin{adjustbox}{angle=90, height=0.87\textheight}
\begin{adjustbox}{width=1\textwidth} 
\begin{tabular}{c|c|c|c|c|c|c|c|c|c|c|c|c|c|c|c|c|c|c|c|c|c|c|c|c|c|c|c|c|c|c}
\hline
& Class ID $\downarrow\rightarrow$  & 1 & 2 & 3 & 4 & 5 & 6 & 7 & 8 & 9 & 10 & 11 & 12 & 13 & 14 & 15 & 16 & 17 & 18 & 19 & 20 & 21 & 22 & 23 & 24 & 25 & 26 & 27 & 28 & 29 \\

%%%%%%%%%%%%%%%%%%%%%%%%%%%%%%%%%%%%%%%%%%%
% Sample Count
%%%%%%%%%%%%%%%%%%%%%%%%%%%%%%%%%%%%%%%%%%%
\hline \hline
\rowcolor[HTML]{D9D9D9}
\multicolumn{31}{c}{(a) \textbf{Sample Count}}\\
\hline \hline

 \multirow{29}{*}{\rotatebox{90}{Actual Class ID $\downarrow$}} & 1 & 1002 & 539 & 0 & 817 & 23 & 0 & 153 & 0 & 206 & 143 & 0 & 102 & 41 & 38 & 190 & 362 & 38 & 45 & 158 & 52 & 0 & 0 & 16 & 33 & 27 & 0 & 248 & 0 & 304 \\
 & 2 & 539 & 2024 & 12 & 1279 & 32 & 68 & 308 & 44 & 206 & 319 & 24 & 141 & 129 & 54 & 435 & 716 & 46 & 81 & 204 & 137 & 23 & 102 & 154 & 44 & 71 & 53 & 327 & 39 & 882 \\
 & 3 & 0 & 12 & 510 & 0 & 28 & 18 & 0 & 0 & 0 & 0 & 0 & 0 & 154 & 109 & 44 & 160 & 0 & 0 & 213 & 30 & 14 & 0 & 0 & 0 & 106 & 0 & 0 & 14 & 69 \\
 & 4 & 817 & 1279 & 0 & 2575 & 104 & 69 & 291 & 44 & 262 & 387 & 0 & 174 & 273 & 72 & 449 & 997 & 70 & 109 & 484 & 242 & 14 & 51 & 74 & 25 & 83 & 189 & 979 & 19 & 876 \\
 & 5 & 23 & 32 & 28 & 104 & 643 & 19 & 9 & 0 & 0 & 0 & 0 & 0 & 62 & 32 & 270 & 32 & 0 & 0 & 137 & 0 & 9 & 19 & 69 & 17 & 0 & 19 & 56 & 0 & 299 \\
 & 6 & 0 & 68 & 18 & 69 & 19 & 473 & 0 & 0 & 0 & 0 & 0 & 0 & 39 & 18 & 54 & 137 & 0 & 0 & 154 & 0 & 0 & 19 & 16 & 18 & 0 & 179 & 16 & 36 & 419 \\
 & 7 & 153 & 308 & 0 & 291 & 9 & 0 & 646 & 0 & 16 & 62 & 38 & 102 & 24 & 40 & 191 & 306 & 16 & 0 & 133 & 16 & 8 & 0 & 92 & 17 & 0 & 0 & 52 & 32 & 103 \\
 & 8 & 0 & 44 & 0 & 44 & 0 & 0 & 0 & 408 & 0 & 0 & 77 & 0 & 103 & 0 & 0 & 191 & 0 & 0 & 268 & 44 & 0 & 52 & 0 & 52 & 0 & 0 & 52 & 0 & 0 \\
 & 9 & 206 & 206 & 0 & 262 & 0 & 0 & 16 & 0 & 713 & 40 & 26 & 0 & 141 & 104 & 40 & 441 & 0 & 0 & 158 & 84 & 0 & 0 & 36 & 48 & 0 & 50 & 76 & 25 & 184 \\
 & 10 & 143 & 319 & 0 & 387 & 0 & 0 & 62 & 0 & 40 & 638 & 80 & 48 & 130 & 0 & 103 & 371 & 31 & 0 & 20 & 48 & 0 & 0 & 97 & 0 & 36 & 0 & 94 & 8 & 28 \\
 & 11 & 0 & 24 & 0 & 0 & 0 & 0 & 38 & 77 & 26 & 80 & 1128 & 96 & 254 & 139 & 99 & 614 & 89 & 54 & 256 & 151 & 0 & 9 & 376 & 0 & 153 & 0 & 18 & 66 & 159 \\
 & 12 & 102 & 141 & 0 & 174 & 0 & 0 & 102 & 0 & 0 & 48 & 96 & 566 & 30 & 200 & 79 & 365 & 257 & 0 & 84 & 21 & 0 & 0 & 9 & 0 & 0 & 0 & 142 & 0 & 76 \\
 & 13 & 41 & 129 & 154 & 273 & 62 & 39 & 24 & 103 & 141 & 130 & 254 & 30 & 2473 & 138 & 70 & 985 & 108 & 155 & 650 & 382 & 73 & 20 & 574 & 77 & 187 & 65 & 400 & 174 & 506 \\
 & 14 & 38 & 54 & 109 & 72 & 32 & 18 & 40 & 0 & 104 & 0 & 139 & 200 & 138 & 1169 & 85 & 693 & 226 & 40 & 256 & 287 & 0 & 34 & 97 & 8 & 229 & 26 & 146 & 86 & 339 \\
 & 15 & 190 & 435 & 44 & 449 & 270 & 54 & 191 & 0 & 40 & 103 & 99 & 79 & 70 & 85 & 1595 & 604 & 25 & 172 & 271 & 38 & 40 & 42 & 100 & 19 & 34 & 40 & 159 & 83 & 454 \\
 & 16 & 362 & 716 & 160 & 997 & 32 & 137 & 306 & 191 & 441 & 371 & 614 & 365 & 985 & 693 & 604 & 4730 & 378 & 218 & 1044 & 496 & 67 & 216 & 803 & 219 & 277 & 88 & 899 & 425 & 1175 \\
 & 17 & 158 & 204 & 213 & 484 & 137 & 154 & 133 & 268 & 158 & 20 & 256 & 84 & 650 & 256 & 271 & 1044 & 200 & 214 & 3371 & 258 & 168 & 0 & 379 & 158 & 90 & 236 & 471 & 242 & 1184 \\
 & 18 & 38 & 46 & 0 & 70 & 0 & 0 & 16 & 0 & 0 & 31 & 89 & 257 & 108 & 226 & 25 & 378 & 752 & 0 & 200 & 29 & 46 & 0 & 117 & 24 & 0 & 8 & 114 & 0 & 144 \\
 & 19 & 45 & 81 & 0 & 109 & 0 & 0 & 0 & 0 & 0 & 0 & 54 & 0 & 155 & 40 & 172 & 218 & 0 & 598 & 214 & 29 & 0 & 64 & 74 & 16 & 0 & 0 & 85 & 0 & 182 \\
 & 20 & 52 & 137 & 30 & 242 & 0 & 0 & 16 & 44 & 84 & 48 & 151 & 21 & 382 & 287 & 38 & 496 & 29 & 29 & 258 & 1517 & 0 & 73 & 352 & 18 & 615 & 0 & 171 & 56 & 427 \\
 & 21 & 0 & 23 & 14 & 14 & 9 & 0 & 8 & 0 & 0 & 0 & 0 & 0 & 73 & 0 & 40 & 67 & 46 & 0 & 168 & 0 & \textbf{396} & 23 & 0 & 16 & 0 & 0 & 0 & 14 & \textbf{264} \\
 & 22 & 0 & 102 & 0 & 51 & 19 & 19 & 0 & 52 & 0 & 0 & 9 & 0 & 20 & 34 & 42 & 216 & 0 & 64 & 0 & 73 & 23 & 560 & 0 & 118 & 0 & 63 & 76 & 11 & 379 \\
 & 23 & 16 & 154 & 0 & 74 & 69 & 16 & 92 & 0 & 36 & 97 & 376 & 9 & 574 & 97 & 100 & 803 & 117 & 74 & 379 & 352 & 0 & 0 & 1778 & 49 & 193 & 12 & 247 & 67 & 423 \\
 & 24 & 33 & 44 & 0 & 25 & 17 & 18 & 17 & 52 & 48 & 0 & 0 & 0 & 77 & 8 & 19 & 219 & 24 & 16 & 158 & 18 & 16 & 118 & 49 & 580 & 0 & 0 & 92 & 0 & 281 \\
 & 25 & 27 & 71 & 106 & 83 & 0 & 0 & 0 & 0 & 0 & 36 & 153 & 0 & 187 & 229 & 34 & 277 & 0 & 0 & 90 & 615 & 0 & 0 & 193 & 0 & 799 & 0 & 51 & 45 & 81 \\
 & 26 & 0 & 53 & 0 & 189 & 19 & 179 & 0 & 0 & 50 & 0 & 0 & 0 & 65 & 26 & 40 & 88 & 8 & 0 & 236 & 0 & 0 & 63 & 12 & 0 & 0 & 657 & 114 & 0 & 366 \\
 & 27 & 248 & 327 & 0 & 979 & 56 & 16 & 52 & 52 & 76 & 94 & 18 & 142 & 400 & 146 & 159 & 899 & 114 & 85 & 471 & 171 & 0 & 76 & 247 & 92 & 51 & 114 & 1973 & 0 & 766 \\
 & 28 & 0 & 39 & 14 & 19 & 0 & 36 & 32 & 0 & 25 & 8 & 66 & 0 & 174 & 86 & 83 & 425 & 0 & 0 & 242 & 56 & 14 & 11 & 67 & 0 & 45 & 0 & 0 & 603 & 94 \\
 & 29 & 304 & 882 & 69 & 876 & 299 & 419 & 103 & 0 & 184 & 28 & 159 & 76 & 506 & 339 & 454 & 1175 & 144 & 182 & 1184 & 427 & \textbf{264} & 379 & 423 & 281 & 81 & 366 & 766 & 94 & \textbf{3980} \\

%%%%%%%%%%%%%%%%%%%%%%%%%%%%%%%%%%%%%%%%%%%
% Cooccurrence
%%%%%%%%%%%%%%%%%%%%%%%%%%%%%%%%%%%%%%%%%%%
\hline \hline
\rowcolor[HTML]{D9D9D9}
\multicolumn{31}{c}{(b) \textbf{Cooccurrence}}\\
\hline \hline

 \multirow{29}{*}{\rotatebox{90}{Actual Class ID $\downarrow$}} & 1 & 1 & 0.27 & 0 & 0.32 & 0.04 & 0 & 0.24 & 0 & 0.29 & 0.22 & 0 & 0.18 & 0.02 & 0.03 & 0.12 & 0.08 & 0.05 & 0.08 & 0.05 & 0.03 & 0 & 0 & 0.01 & 0.06 & 0.03 & 0 & 0.13 & 0 & 0.08 \\
 & 2 & 0.54 & 1 & 0.02 & 0.50 & 0.05 & 0.14 & 0.48 & 0.11 & 0.29 & 0.50 & 0.02 & 0.25 & 0.05 & 0.05 & 0.27 & 0.15 & 0.06 & 0.14 & 0.06 & 0.09 & 0.06 & 0.18 & 0.09 & 0.08 & 0.09 & 0.08 & 0.17 & 0.06 & 0.22 \\
 & 3 & 0 & 0.01 & 1 & 0 & 0.04 & 0.04 & 0 & 0 & 0 & 0 & 0 & 0 & 0.06 & 0.09 & 0.03 & 0.03 & 0 & 0 & 0.06 & 0.02 & 0.04 & 0 & 0 & 0 & 0.13 & 0 & 0 & 0.02 & 0.02 \\
 & 4 & 0.82 & 0.63 & 0 & 1 & 0.16 & 0.15 & 0.45 & 0.11 & 0.37 & 0.61 & 0 & 0.31 & 0.11 & 0.06 & 0.28 & 0.21 & 0.09 & 0.18 & 0.14 & 0.16 & 0.04 & 0.09 & 0.04 & 0.04 & 0.10 & 0.29 & 0.50 & 0.03 & 0.22 \\
 & 5 & 0.02 & 0.02 & 0.05 & 0.04 & 1 & 0.04 & 0.01 & 0 & 0 & 0 & 0 & 0 & 0.03 & 0.03 & 0.17 & 0.01 & 0 & 0 & 0.04 & 0 & 0.02 & 0.03 & 0.04 & 0.03 & 0 & 0.03 & 0.03 & 0 & 0.08 \\
 & 6 & 0 & 0.03 & 0.04 & 0.03 & 0.03 & 1 & 0 & 0 & 0 & 0 & 0 & 0 & 0.02 & 0.02 & 0.03 & 0.03 & 0 & 0 & 0.05 & 0 & 0 & 0.03 & 0.01 & 0.03 & 0 & 0.27 & 0.01 & 0.06 & 0.11 \\
 & 7 & 0.15 & 0.15 & 0 & 0.11 & 0.01 & 0 & 1 & 0 & 0.02 & 0.10 & 0.03 & 0.18 & 0.01 & 0.03 & 0.12 & 0.06 & 0.02 & 0 & 0.04 & 0.01 & 0.02 & 0 & 0.05 & 0.03 & 0 & 0 & 0.03 & 0.05 & 0.03 \\
 & 8 & 0 & 0.02 & 0 & 0.02 & 0 & 0 & 0 & 1 & 0 & 0 & 0.07 & 0 & 0.04 & 0 & 0 & 0.04 & 0 & 0 & 0.08 & 0.03 & 0 & 0.09 & 0 & 0.09 & 0 & 0 & 0.03 & 0 & 0 \\
 & 9 & 0.21 & 0.10 & 0 & 0.10 & 0 & 0 & 0.02 & 0 & 1 & 0.06 & 0.02 & 0 & 0.06 & 0.09 & 0.03 & 0.09 & 0 & 0 & 0.05 & 0.06 & 0 & 0 & 0.02 & 0.08 & 0 & 0.08 & 0.04 & 0.04 & 0.05 \\
 & 10 & 0.14 & 0.16 & 0 & 0.15 & 0 & 0 & 0.10 & 0 & 0.06 & 1 & 0.07 & 0.08 & 0.05 & 0 & 0.06 & 0.08 & 0.04 & 0 & 0.01 & 0.03 & 0 & 0 & 0.05 & 0 & 0.05 & 0 & 0.05 & 0.01 & 0.01 \\
 & 11 & 0 & 0.01 & 0 & 0 & 0 & 0 & 0.06 & 0.19 & 0.04 & 0.13 & 1 & 0.17 & 0.10 & 0.12 & 0.06 & 0.13 & 0.12 & 0.09 & 0.08 & 0.10 & 0 & 0.02 & 0.21 & 0 & 0.19 & 0 & 0.01 & 0.11 & 0.04 \\
 & 12 & 0.10 & 0.07 & 0 & 0.07 & 0 & 0 & 0.16 & 0 & 0 & 0.08 & 0.09 & 1 & 0.01 & 0.17 & 0.05 & 0.08 & 0.34 & 0 & 0.02 & 0.01 & 0 & 0 & 0.01 & 0 & 0 & 0 & 0.07 & 0 & 0.02 \\
 & 13 & 0.04 & 0.06 & 0.30 & 0.11 & 0.10 & 0.08 & 0.04 & 0.25 & 0.20 & 0.20 & 0.23 & 0.05 & 1 & 0.12 & 0.04 & 0.21 & 0.14 & 0.26 & 0.19 & 0.25 & 0.18 & 0.04 & 0.32 & 0.13 & 0.23 & 0.10 & 0.20 & 0.29 & 0.13 \\
 & 14 & 0.04 & 0.03 & 0.21 & 0.03 & 0.05 & 0.04 & 0.06 & 0 & 0.15 & 0 & 0.12 & 0.35 & 0.06 & 1 & 0.05 & 0.15 & 0.30 & 0.07 & 0.08 & 0.19 & 0 & 0.06 & 0.05 & 0.01 & 0.29 & 0.04 & 0.07 & 0.14 & 0.09 \\
 & 15 & 0.19 & 0.21 & 0.09 & 0.17 & 0.42 & 0.11 & 0.30 & 0 & 0.06 & 0.16 & 0.09 & 0.14 & 0.03 & 0.07 & 1 & 0.13 & 0.03 & 0.29 & 0.08 & 0.03 & 0.10 & 0.08 & 0.06 & 0.03 & 0.04 & 0.06 & 0.08 & 0.14 & 0.11 \\
 & 16 & 0.36 & 0.35 & 0.31 & 0.39 & 0.05 & 0.29 & 0.47 & 0.47 & 0.62 & 0.58 & 0.54 & 0.64 & 0.40 & 0.59 & 0.38 & 1 & 0.50 & 0.36 & 0.31 & 0.33 & 0.17 & 0.39 & 0.45 & 0.38 & 0.35 & 0.13 & 0.46 & 0.70 & 0.30 \\
 & 17 & 0.16 & 0.10 & 0.42 & 0.19 & 0.21 & 0.33 & 0.21 & 0.66 & 0.22 & 0.03 & 0.23 & 0.15 & 0.26 & 0.22 & 0.17 & 0.22 & 0.27 & 0.36 & 1 & 0.17 & 0.42 & 0 & 0.21 & 0.27 & 0.11 & 0.36 & 0.24 & 0.40 & 0.30 \\
 & 18 & 0.04 & 0.02 & 0 & 0.03 & 0 & 0 & 0.02 & 0 & 0 & 0.05 & 0.08 & 0.45 & 0.04 & 0.19 & 0.02 & 0.08 & 1 & 0 & 0.06 & 0.02 & 0.12 & 0 & 0.07 & 0.04 & 0 & 0.01 & 0.06 & 0 & 0.04 \\
 & 19 & 0.04 & 0.04 & 0 & 0.04 & 0 & 0 & 0 & 0 & 0 & 0 & 0.05 & 0 & 0.06 & 0.03 & 0.11 & 0.05 & 0 & 1 & 0.06 & 0.02 & 0 & 0.11 & 0.04 & 0.03 & 0 & 0 & 0.04 & 0 & 0.05 \\
 & 20 & 0.05 & 0.07 & 0.06 & 0.09 & 0 & 0 & 0.02 & 0.11 & 0.12 & 0.08 & 0.13 & 0.04 & 0.15 & 0.25 & 0.02 & 0.10 & 0.04 & 0.05 & 0.08 & 1 & 0 & 0.13 & 0.20 & 0.03 & 0.77 & 0 & 0.09 & 0.09 & 0.11 \\
 & 21 & 0 & 0.01 & 0.03 & 0.01 & 0.01 & 0 & 0.01 & 0 & 0 & 0 & 0 & 0 & 0.03 & 0 & 0.03 & 0.01 & 0.06 & 0 & 0.05 & 0 & 1 & 0.04 & 0 & 0.03 & 0 & 0 & 0 & 0.02 & 0.07 \\
 & 22 & 0 & 0.05 & 0 & 0.02 & 0.03 & 0.04 & 0 & 0.13 & 0 & 0 & 0.01 & 0 & 0.01 & 0.03 & 0.03 & 0.05 & 0 & 0.11 & 0 & 0.05 & 0.06 & 1 & 0 & 0.20 & 0 & 0.10 & 0.04 & 0.02 & 0.10 \\
 & 23 & 0.02 & 0.08 & 0 & 0.03 & 0.11 & 0.03 & 0.14 & 0 & 0.05 & 0.15 & 0.33 & 0.02 & 0.23 & 0.08 & 0.06 & 0.17 & 0.16 & 0.12 & 0.11 & 0.23 & 0 & 0 & 1 & 0.08 & 0.24 & 0.02 & 0.13 & 0.11 & 0.11 \\
 & 24 & 0.03 & 0.02 & 0 & 0.01 & 0.03 & 0.04 & 0.03 & 0.13 & 0.07 & 0 & 0 & 0 & 0.03 & 0.01 & 0.01 & 0.05 & 0.03 & 0.03 & 0.05 & 0.01 & 0.04 & 0.21 & 0.03 & 1 & 0 & 0 & 0.05 & 0 & 0.07 \\
 & 25 & 0.03 & 0.04 & 0.21 & 0.03 & 0 & 0 & 0 & 0 & 0 & 0.06 & 0.14 & 0 & 0.08 & 0.20 & 0.02 & 0.06 & 0 & 0 & 0.03 & 0.41 & 0 & 0 & 0.11 & 0 & 1 & 0 & 0.03 & 0.07 & 0.02 \\
 & 26 & 0 & 0.03 & 0 & 0.07 & 0.03 & 0.38 & 0 & 0 & 0.07 & 0 & 0 & 0 & 0.03 & 0.02 & 0.03 & 0.02 & 0.01 & 0 & 0.07 & 0 & 0 & 0.11 & 0.01 & 0 & 0 & 1 & 0.06 & 0 & 0.09 \\
 & 27 & 0.25 & 0.16 & 0 & 0.38 & 0.09 & 0.03 & 0.08 & 0.13 & 0.11 & 0.15 & 0.02 & 0.25 & 0.16 & 0.12 & 0.10 & 0.19 & 0.15 & 0.14 & 0.14 & 0.11 & 0 & 0.14 & 0.14 & 0.16 & 0.06 & 0.17 & 1 & 0 & 0.19 \\
 & 28 & 0 & 0.02 & 0.03 & 0.01 & 0 & 0.08 & 0.05 & 0 & 0.04 & 0.01 & 0.06 & 0 & 0.07 & 0.07 & 0.05 & 0.09 & 0 & 0 & 0.07 & 0.04 & 0.04 & 0.02 & 0.04 & 0 & 0.06 & 0 & 0 & 1 & 0.02 \\
 & 29 & 0.30 & 0.44 & 0.14 & 0.34 & 0.47 & 0.89 & 0.16 & 0 & 0.26 & 0.04 & 0.14 & 0.13 & 0.20 & 0.29 & 0.28 & 0.25 & 0.19 & 0.30 & 0.35 & 0.28 & \textbf{0.67} & 0.68 & 0.24 & 0.48 & 0.10 & 0.56 & 0.39 & 0.16 & 1 \\

%%%%%%%%%%%%%%%%%%%%%%%%%%%%%%%%%%%%%%%%%%%
% Misprediction
%%%%%%%%%%%%%%%%%%%%%%%%%%%%%%%%%%%%%%%%%%%
\hline \hline
\rowcolor[HTML]{D9D9D9}
\multicolumn{31}{c}{(c) \textbf{Misprediction}}\\
\hline \hline

 \multirow{30}{*}{\rotatebox{90}{Predicted Class ID $\downarrow$}} & 1 & 0 & 0.04 & 0 & 0 & 0.01 & 0 & 0.03 & 0 & 0.01 & 0.03 & 0 & 0.02 & 0.02 & 0.01 & 0.04 & 0.01 & 0.01 & 0.01 & 0.02 & 0.02 & 0 & 0 & 0.02 & 0 & 0 & 0.01 & 0.06 & 0 & 0.02 \\
 & 2 & 0.18 & 0 & 0.02 & 0.03 & 0.13 & 0 & 0.09 & 0 & 0.04 & 0.12 & 0.03 & 0.04 & 0.06 & 0.07 & 0.09 & 0.06 & 0.01 & 0.04 & 0.07 & 0.06 & 0.09 & 0.04 & 0.07 & 0.05 & 0.06 & 0.06 & 0.08 & 0.03 & 0.04 \\
 & 3 & 0.01 & 0 & 0 & 0 & 0.01 & 0 & 0 & 0 & 0 & 0 & 0 & 0 & 0.01 & 0.01 & 0 & 0 & 0 & 0 & 0.01 & 0 & 0 & 0 & 0.01 & 0 & 0.01 & 0 & 0 & 0 & 0 \\
 & 4 & 0.64 & 0.19 & 0.02 & 0 & 0.06 & 0 & 0.09 & 0 & 0.03 & 0.18 & 0.01 & 0.04 & 0.05 & 0.03 & 0.08 & 0.06 & 0.01 & 0.01 & 0.08 & 0.07 & 0.02 & 0 & 0.05 & 0.02 & 0.02 & 0.07 & 0.13 & 0.01 & 0.06 \\
 & 5 & 0 & 0.01 & 0 & 0.01 & 0 & 0 & 0 & 0 & 0 & 0 & 0.01 & 0 & 0.01 & 0 & 0 & 0.01 & 0 & 0 & 0.01 & 0 & 0.02 & 0 & 0 & 0 & 0 & 0 & 0.01 & 0 & 0.01 \\
 & 6 & 0 & 0 & 0 & 0.01 & 0 & 0 & 0 & 0 & 0 & 0 & 0 & 0 & 0 & 0 & 0 & 0 & 0 & 0 & 0.01 & 0.01 & 0.02 & 0.03 & 0 & 0 & 0 & 0.03 & 0 & 0 & 0 \\
 & 7 & 0 & 0 & 0 & 0 & 0.01 & 0 & 0 & 0 & 0 & 0 & 0 & 0.02 & 0 & 0 & 0 & 0 & 0 & 0 & 0.01 & 0 & 0 & 0 & 0 & 0 & 0 & 0 & 0 & 0 & 0 \\
 & 8 & 0 & 0 & 0 & 0 & 0 & 0 & 0 & 0 & 0 & 0 & 0 & 0 & 0 & 0 & 0 & 0 & 0 & 0 & 0 & 0.01 & 0 & 0 & 0 & 0 & 0 & 0 & 0 & 0 & 0 \\
 & 9 & 0.02 & 0.01 & 0 & 0.01 & 0.01 & 0 & 0 & 0 & 0 & 0.01 & 0 & 0 & 0.01 & 0.03 & 0.01 & 0 & 0 & 0 & 0.02 & 0.01 & 0.02 & 0 & 0.02 & 0 & 0 & 0.01 & 0.02 & 0.01 & 0.01 \\
 & 10 & 0.03 & 0.01 & 0 & 0 & 0 & 0 & 0.01 & 0 & 0 & 0 & 0.01 & 0 & 0.02 & 0.01 & 0.02 & 0.01 & 0.01 & 0 & 0 & 0.04 & 0 & 0 & 0.03 & 0 & 0 & 0 & 0.03 & 0 & 0 \\
 & 11 & 0.02 & 0.03 & 0 & 0.01 & 0 & 0 & 0 & 0.02 & 0.01 & 0.03 & 0 & 0.02 & 0.02 & 0.03 & 0.03 & 0.02 & 0.02 & 0 & 0.04 & 0.06 & 0 & 0.02 & 0.03 & 0 & 0.01 & 0 & 0.03 & 0 & 0.01 \\
 & 12 & 0 & 0 & 0 & 0 & 0 & 0 & 0.03 & 0 & 0 & 0 & 0 & 0 & 0 & 0.02 & 0 & 0 & 0 & 0 & 0 & 0.01 & 0 & 0 & 0 & 0 & 0.01 & 0 & 0 & 0 & 0 \\
 & 13 & 0.03 & 0.06 & 0.03 & 0.05 & 0.09 & 0 & 0 & 0.05 & 0.04 & 0 & 0.18 & 0 & 0 & 0.09 & 0.05 & 0.07 & 0 & 0.08 & 0.13 & 0.14 & 0.08 & 0 & 0.09 & 0.05 & 0.03 & 0.05 & 0.08 & 0.08 & 0.08 \\
 & 14 & 0.02 & 0.02 & 0.04 & 0.01 & 0.03 & 0 & 0.01 & 0 & 0 & 0.01 & 0.04 & 0.02 & 0.01 & 0 & 0.02 & 0.02 & 0.03 & 0 & 0.03 & 0.02 & 0.07 & 0 & 0.03 & 0.01 & 0.01 & 0.04 & 0.03 & 0.02 & 0.02 \\
 & 15 & 0.01 & 0.03 & 0 & 0.02 & 0.14 & 0 & 0.05 & 0 & 0 & 0.03 & 0.03 & 0.02 & 0.02 & 0.03 & 0 & 0.03 & 0.02 & 0.02 & 0.04 & 0.01 & 0.10 & 0.02 & 0.03 & 0.03 & 0 & 0.03 & 0.03 & 0 & 0.03 \\
 & 16 & 0.16 & 0.11 & 0.10 & 0.10 & 0.16 & 0 & 0.08 & 0.07 & 0.08 & 0.21 & 0.23 & 0.05 & 0.15 & 0.51 & 0.19 & 0 & 0.04 & 0.13 & 0.17 & 0.17 & 0.15 & 0.08 & 0.17 & 0.23 & 0.08 & 0.06 & 0.26 & 0.26 & 0.10 \\
 & 17 & 0.07 & 0.05 & 0.03 & 0.04 & 0.09 & 0.03 & 0.03 & 0.05 & 0.01 & 0.04 & 0.11 & 0.02 & 0.03 & 0.11 & 0.03 & 0.04 & 0 & 0.07 & 0 & 0.04 & 0.12 & 0 & 0.02 & 0.04 & 0.02 & 0.08 & 0.03 & 0.10 & 0.05 \\
 & 18 & 0 & 0.01 & 0.02 & 0 & 0.01 & 0 & 0.03 & 0 & 0 & 0 & 0.04 & 0 & 0.01 & 0.01 & 0 & 0.01 & 0 & 0 & 0.01 & 0.01 & 0.05 & 0.01 & 0.01 & 0 & 0 & 0 & 0 & 0.01 & 0.01 \\
 & 19 & 0 & 0 & 0 & 0 & 0 & 0 & 0 & 0 & 0 & 0 & 0.01 & 0 & 0 & 0.01 & 0 & 0 & 0 & 0 & 0 & 0.01 & 0 & 0 & 0 & 0 & 0 & 0.01 & 0 & 0 & 0 \\
 & 20 & 0.02 & 0.03 & 0.06 & 0.02 & 0.03 & 0 & 0.01 & 0 & 0.04 & 0.03 & 0.04 & 0 & 0.01 & 0.06 & 0.01 & 0.03 & 0 & 0.01 & 0.05 & 0 & 0 & 0.03 & 0.02 & 0.09 & 0.19 & 0.02 & 0.02 & 0.02 & 0.03 \\
 & 21 & 0 & 0 & 0 & 0 & 0.01 & 0 & 0 & 0 & 0 & 0 & 0 & 0 & 0 & 0 & 0 & 0 & 0 & 0 & 0 & 0 & 0 & 0 & 0 & 0.01 & 0 & 0 & 0 & 0 & 0 \\
 & 22 & 0 & 0 & 0 & 0 & 0.03 & 0 & 0 & 0 & 0 & 0 & 0 & 0 & 0 & 0.01 & 0 & 0 & 0 & 0 & 0 & 0.01 & 0.05 & 0 & 0 & 0 & 0 & 0.01 & 0.02 & 0 & 0.01 \\
 & 23 & 0.02 & 0.04 & 0 & 0.03 & 0.03 & 0 & 0 & 0 & 0.03 & 0.03 & 0.15 & 0 & 0.07 & 0.07 & 0.06 & 0.05 & 0.02 & 0.05 & 0.07 & 0.11 & 0 & 0 & 0 & 0.09 & 0.01 & 0.01 & 0.06 & 0.02 & 0.04 \\
 & 24 & 0.01 & 0 & 0 & 0.01 & 0 & 0 & 0 & 0 & 0 & 0 & 0.01 & 0 & 0 & 0 & 0.01 & 0.01 & 0 & 0 & 0.02 & 0.01 & 0 & 0.04 & 0 & 0 & 0.01 & 0 & 0.02 & 0.01 & 0.02 \\
 & 25 & 0 & 0 & 0.07 & 0 & 0 & 0 & 0 & 0 & 0 & 0 & 0 & 0 & 0 & 0 & 0 & 0 & 0.01 & 0 & 0 & 0.01 & 0 & 0 & 0 & 0 & 0 & 0 & 0 & 0 & 0 \\
 & 26 & 0.01 & 0.01 & 0 & 0.01 & 0.03 & 0.03 & 0 & 0 & 0 & 0.01 & 0 & 0 & 0 & 0 & 0 & 0 & 0 & 0 & 0.01 & 0.01 & 0 & 0 & 0.01 & 0 & 0 & 0 & 0 & 0 & 0.01 \\
 & 27 & 0.09 & 0.08 & 0 & 0.12 & 0.04 & 0.02 & 0.03 & 0 & 0 & 0.03 & 0.05 & 0 & 0.05 & 0.04 & 0.05 & 0.07 & 0 & 0.01 & 0.10 & 0.08 & 0 & 0.04 & 0.09 & 0.04 & 0 & 0 & 0 & 0.01 & 0.06 \\
 & 28 & 0.01 & 0 & 0 & 0 & 0.01 & 0 & 0.01 & 0 & 0 & 0 & 0 & 0 & 0 & 0.03 & 0.01 & 0 & 0 & 0.01 & 0.02 & 0.02 & 0 & 0.02 & 0 & 0 & 0.02 & 0.02 & 0 & 0 & 0.01 \\
 & 29 & 0.13 & 0.16 & 0.04 & 0.07 & 0.38 & 0.17 & 0.03 & 0 & 0.04 & 0.03 & 0.07 & 0.02 & 0.07 & 0.13 & 0.10 & 0.07 & 0.01 & 0.02 & 0.22 & 0.12 & \textbf{0.79} & 0.14 & 0.08 & 0.25 & 0.04 & 0.30 & 0.14 & 0 & 0 \\
 & 30 & 0.01 & 0 & 0 & 0 & 0.03 & 0 & 0 & 0 & 0 & 0 & 0.01 & 0 & 0.01 & 0.01 & 0.01 & 0.01 & 0 & 0.01 & 0.01 & 0.01 & 0.02 & 0 & 0 & 0 & 0 & 0.01 & 0.01 & 0 & 0.01 \\
\hline
\end{tabular}
\end{adjustbox}

\label{tab:misclassification_fiction}
\end{table*}

\begin{table*}[]
\centering
\caption{Non-fiction genre indistinguishability analysis}

% \begin{adjustbox}{angle=90, height=0.87\textheight}
\begin{adjustbox}{width=1\textwidth} 
\begin{tabular}{c|c|c|c|c|c|c|c|c|c|c|c|c|c|c|c|c|c|c|c|c|c|c|c|c|c|c|c|c|c|c}
\hline
& Class ID $\downarrow\rightarrow$  & 1 & 2 & 3 & 4 & 5 & 6 & 7 & 8 & 9 & 10 & 11 & 12 & 13 & 14 & 15 & 16 & 17 & 18 & 19 & 20 & 21 & 22 & 23 & 24 & 25 & 26 & 27 & 28 & 30 \\

%%%%%%%%%%%%%%%%%%%%%%%%%%%%%%%%%%%%%%%%%%%
% Sample Count
%%%%%%%%%%%%%%%%%%%%%%%%%%%%%%%%%%%%%%%%%%%
\hline \hline
\rowcolor[HTML]{D9D9D9}
\multicolumn{31}{c}{(a) \textbf{Sample Count}}\\
\hline \hline

\multirow{29}{*}{\rotatebox{90}{Actual Class ID $\downarrow$}} & 1 & 748 & 169 & 0 & 222 & 41 & 0 & 12 & 0 & 306 & 14 & 0 & 12 & 89 & 52 & 97 & 44 & 14 & 10 & 0 & 16 & 0 & 95 & 0 & 369 & 14 & 0 & 65 & 37 & 157 \\
 & 2 & 169 & 1444 & 9 & 331 & 203 & 42 & 0 & 143 & 53 & 34 & 103 & 12 & 512 & 237 & 165 & 109 & 26 & 57 & 58 & 58 & 270 & 408 & 125 & 236 & 14 & 8 & 162 & 28 & 259 \\
 & 3 & 0 & 9 & 614 & 0 & 46 & 197 & 0 & 0 & 0 & 24 & 0 & 0 & 197 & 303 & 38 & 9 & 0 & 0 & 0 & 34 & 44 & 84 & 0 & 58 & 227 & 0 & 8 & 0 & 107 \\
 & 4 & 222 & 331 & 0 & 878 & 41 & 0 & 8 & 28 & 84 & 170 & 0 & 31 & 214 & 140 & 82 & 52 & 37 & 46 & 0 & 9 & 0 & 152 & 0 & 340 & 61 & 9 & 315 & 0 & 109 \\
 & 5 & 41 & 203 & 46 & 41 & 806 & 0 & 0 & 17 & 19 & 10 & 47 & 17 & 308 & 274 & 298 & 50 & 0 & 25 & 24 & 16 & 8 & 216 & 11 & 176 & 19 & 0 & 19 & 16 & 187 \\
 & 6 & 0 & 42 & 197 & 0 & 0 & 483 & 0 & 0 & 11 & 0 & 0 & 0 & 165 & 183 & 11 & 0 & 8 & 12 & 0 & 0 & 0 & 69 & 0 & 201 & 28 & 9 & 0 & 0 & 73 \\
 & 7 & 12 & 0 & 0 & 8 & 0 & 0 & 494 & 0 & 72 & 0 & 9 & 183 & 38 & 26 & 26 & 38 & 41 & 9 & 0 & 11 & 0 & 185 & 12 & 29 & 89 & 0 & 8 & 104 & 111 \\
 & 8 & 0 & 143 & 0 & 28 & 17 & 0 & 0 & 439 & 45 & 0 & 110 & 8 & 52 & 44 & 8 & 19 & 0 & 34 & 0 & 32 & 0 & 290 & 0 & 0 & 47 & 8 & 0 & 0 & 12 \\
 & 9 & 306 & 53 & 0 & 84 & 19 & 11 & 72 & 45 & 846 & 0 & 0 & 66 & 197 & 132 & 37 & 39 & 11 & 0 & 76 & 17 & 9 & 174 & 0 & 361 & 9 & 55 & 41 & 122 & 196 \\
 & 10 & 14 & 34 & 24 & 170 & 10 & 0 & 0 & 0 & 0 & 889 & 119 & 142 & 16 & 521 & 33 & 25 & 149 & 84 & 0 & 193 & 0 & 222 & 225 & 54 & 506 & 9 & 80 & 0 & 57 \\
 & 11 & 0 & 103 & 0 & 0 & 47 & 0 & 9 & 110 & 0 & 119 & 896 & 0 & 210 & 398 & 85 & 216 & 12 & 68 & 47 & 71 & 33 & 223 & 282 & 39 & 133 & 12 & 0 & 9 & 204 \\
 & 12 & 12 & 12 & 0 & 31 & 17 & 0 & 183 & 8 & 66 & 142 & 0 & 949 & 17 & 381 & 0 & 11 & 456 & 0 & 0 & 92 & 0 & 400 & 11 & 221 & 506 & 16 & 0 & 0 & 84 \\
 & 13 & 89 & 512 & 197 & 214 & 308 & 165 & 38 & 52 & 197 & 16 & 210 & 17 & \textbf{3297} & 1016 & 250 & 556 & 128 & 258 & 383 & 249 & 412 & 478 & 198 & 590 & 9 & 84 & \textbf{266} & 369 & 1198 \\
 & 14 & 52 & 237 & 303 & 140 & 274 & 183 & 26 & 44 & 132 & 521 & 398 & 381 & 1016 & 3417 & 295 & 594 & 353 & 254 & 103 & 532 & 241 & 632 & 369 & 597 & 783 & 24 & 255 & 92 & 581 \\
 & 15 & 97 & 165 & 38 & 82 & 298 & 11 & 26 & 8 & 37 & 33 & 85 & 0 & 250 & 295 & 1112 & 97 & 0 & 37 & 39 & 12 & 104 & 149 & 11 & 77 & 33 & 52 & 40 & 147 & 405 \\
 & 16 & 44 & 109 & 9 & 52 & 50 & 0 & 38 & 19 & 39 & 25 & 216 & 11 & 556 & 594 & 97 & 1448 & 34 & 236 & 93 & 126 & 102 & 207 & 265 & 66 & 17 & 0 & 96 & 204 & 575 \\
 & 17 & 0 & 58 & 0 & 0 & 24 & 0 & 0 & 0 & 76 & 0 & 47 & 0 & 383 & 103 & 39 & 93 & 44 & 41 & 744 & 55 & 126 & 103 & 87 & 58 & 9 & 81 & 0 & 221 & 383 \\
 & 18 & 14 & 26 & 0 & 37 & 0 & 8 & 41 & 0 & 11 & 149 & 12 & 456 & 128 & 353 & 0 & 34 & 886 & 0 & 44 & 143 & 9 & 241 & 20 & 318 & 361 & 0 & 0 & 0 & 179 \\
 & 19 & 10 & 57 & 0 & 46 & 25 & 12 & 9 & 34 & 0 & 84 & 68 & 0 & 258 & 254 & 37 & 236 & 0 & 762 & 41 & 52 & 0 & 315 & 0 & 32 & 27 & 0 & 25 & 37 & 289 \\
 & 20 & 16 & 58 & 34 & 9 & 16 & 0 & 11 & 32 & 17 & 193 & 71 & 92 & 249 & 532 & 12 & 126 & 143 & 52 & 55 & 1122 & 0 & 135 & 205 & 93 & 416 & 12 & 0 & 36 & 147 \\
 & 21 & 0 & 270 & 44 & 0 & 8 & 0 & 0 & 0 & 9 & 0 & 33 & 0 & 412 & 241 & 104 & 102 & 9 & 0 & 126 & 0 & 735 & 104 & 42 & 42 & 0 & 11 & 8 & 67 & 278 \\
 & 22 & 95 & 408 & 84 & 152 & 216 & 69 & 185 & 290 & 174 & 222 & 223 & 400 & 478 & 632 & 149 & 207 & 241 & 315 & 103 & 135 & 104 & 2495 & 171 & 327 & 462 & 129 & 149 & 72 & 107 \\
 & 23 & 0 & 125 & 0 & 0 & 11 & 0 & 12 & 0 & 0 & 225 & 282 & 11 & 198 & 369 & 11 & 265 & 20 & 0 & 87 & 205 & 42 & 171 & 877 & 70 & 273 & 12 & 0 & 43 & 162 \\
 & 24 & 369 & 236 & 58 & 340 & 176 & 201 & 29 & 0 & 361 & 54 & 39 & 221 & 590 & 597 & 77 & 66 & 318 & 32 & 58 & 93 & 42 & 327 & 70 & 1809 & 148 & 0 & 188 & 41 & 207 \\
 & 25 & 14 & 14 & 227 & 61 & 19 & 28 & 89 & 47 & 9 & 506 & 133 & 506 & 9 & 783 & 33 & 17 & 361 & 27 & 9 & 416 & 0 & 462 & 273 & 148 & 1519 & 25 & 16 & 9 & 63 \\
 & 26 & 0 & 8 & 0 & 9 & 0 & 9 & 0 & 8 & 55 & 9 & 12 & 16 & 84 & 24 & 52 & 0 & 0 & 0 & 81 & 12 & 11 & 129 & 12 & 0 & 25 & 424 & 0 & 69 & 185 \\
 & 27 & 65 & 162 & 8 & 315 & 19 & 0 & 8 & 0 & 41 & 80 & 0 & 0 & \textbf{266} & 255 & 40 & 96 & 0 & 25 & 0 & 0 & 8 & 149 & 0 & 188 & 16 & 0 & \textbf{659} & 0 & 151 \\
 & 28 & 37 & 28 & 0 & 0 & 16 & 0 & 104 & 0 & 122 & 0 & 9 & 0 & 369 & 92 & 147 & 204 & 0 & 37 & 221 & 36 & 67 & 72 & 43 & 41 & 9 & 69 & 0 & 888 & 543 \\
 & 30 & 157 & 259 & 107 & 109 & 187 & 73 & 111 & 12 & 196 & 57 & 204 & 84 & 1198 & 581 & 405 & 575 & 179 & 289 & 383 & 147 & 278 & 107 & 162 & 207 & 63 & 185 & 151 & 543 & 2802 \\

%%%%%%%%%%%%%%%%%%%%%%%%%%%%%%%%%%%%%%%%%%%
% Cooccurrence
%%%%%%%%%%%%%%%%%%%%%%%%%%%%%%%%%%%%%%%%%%%
\hline \hline
\rowcolor[HTML]{D9D9D9}
\multicolumn{31}{c}{(b) \textbf{Cooccurrence}}\\
\hline \hline

 \multirow{29}{*}{\rotatebox{90}{Actual Class ID $\downarrow$}} & 1 & 1 & 0.12 & 0 & 0.25 & 0.05 & 0 & 0.02 & 0 & 0.36 & 0.02 & 0 & 0.01 & 0.03 & 0.02 & 0.09 & 0.03 & 0.02 & 0.01 & 0 & 0.01 & 0 & 0.04 & 0 & 0.20 & 0.01 & 0 & 0.10 & 0.04 & 0.06 \\
 & 2 & 0.23 & 1 & 0.01 & 0.38 & 0.25 & 0.09 & 0 & 0.33 & 0.06 & 0.04 & 0.11 & 0.01 & 0.16 & 0.07 & 0.15 & 0.08 & 0.03 & 0.07 & 0.08 & 0.05 & 0.37 & 0.16 & 0.14 & 0.13 & 0.01 & 0.02 & 0.25 & 0.03 & 0.09 \\
 & 3 & 0 & 0.01 & 1 & 0 & 0.06 & 0.41 & 0 & 0 & 0 & 0.03 & 0 & 0 & 0.06 & 0.09 & 0.03 & 0.01 & 0 & 0 & 0 & 0.03 & 0.06 & 0.03 & 0 & 0.03 & 0.15 & 0 & 0.01 & 0 & 0.04 \\
 & 4 & 0.30 & 0.23 & 0 & 1 & 0.05 & 0 & 0.02 & 0.06 & 0.10 & 0.19 & 0 & 0.03 & 0.06 & 0.04 & 0.07 & 0.04 & 0.04 & 0.06 & 0 & 0.01 & 0 & 0.06 & 0 & 0.19 & 0.04 & 0.02 & 0.48 & 0 & 0.04 \\
 & 5 & 0.05 & 0.14 & 0.07 & 0.05 & 1 & 0 & 0 & 0.04 & 0.02 & 0.01 & 0.05 & 0.02 & 0.09 & 0.08 & 0.27 & 0.03 & 0 & 0.03 & 0.03 & 0.01 & 0.01 & 0.09 & 0.01 & 0.10 & 0.01 & 0 & 0.03 & 0.02 & 0.07 \\
 & 6 & 0 & 0.03 & 0.32 & 0 & 0 & 1 & 0 & 0 & 0.01 & 0 & 0 & 0 & 0.05 & 0.05 & 0.01 & 0 & 0.01 & 0.02 & 0 & 0 & 0 & 0.03 & 0 & 0.11 & 0.02 & 0.02 & 0 & 0 & 0.03 \\
 & 7 & 0.02 & 0 & 0 & 0.01 & 0 & 0 & 1 & 0 & 0.09 & 0 & 0.01 & 0.19 & 0.01 & 0.01 & 0.02 & 0.03 & 0.05 & 0.01 & 0 & 0.01 & 0 & 0.07 & 0.01 & 0.02 & 0.06 & 0 & 0.01 & 0.12 & 0.04 \\
 & 8 & 0 & 0.10 & 0 & 0.03 & 0.02 & 0 & 0 & 1 & 0.05 & 0 & 0.12 & 0.01 & 0.02 & 0.01 & 0.01 & 0.01 & 0 & 0.04 & 0 & 0.03 & 0 & 0.12 & 0 & 0 & 0.03 & 0.02 & 0 & 0 & 0 \\
 & 9 & 0.41 & 0.04 & 0 & 0.10 & 0.02 & 0.02 & 0.15 & 0.10 & 1 & 0 & 0 & 0.07 & 0.06 & 0.04 & 0.03 & 0.03 & 0.01 & 0 & 0.10 & 0.02 & 0.01 & 0.07 & 0 & 0.20 & 0.01 & 0.13 & 0.06 & 0.14 & 0.07 \\
 & 10 & 0.02 & 0.02 & 0.04 & 0.19 & 0.01 & 0 & 0 & 0 & 0 & 1 & 0.13 & 0.15 & 0 & 0.15 & 0.03 & 0.02 & 0.17 & 0.11 & 0 & 0.17 & 0 & 0.09 & 0.26 & 0.03 & 0.33 & 0.02 & 0.12 & 0 & 0.02 \\
 & 11 & 0 & 0.07 & 0 & 0 & 0.06 & 0 & 0.02 & 0.25 & 0 & 0.13 & 1 & 0 & 0.06 & 0.12 & 0.08 & 0.15 & 0.01 & 0.09 & 0.06 & 0.06 & 0.04 & 0.09 & 0.32 & 0.02 & 0.09 & 0.03 & 0 & 0.01 & 0.07 \\
 & 12 & 0.02 & 0.01 & 0 & 0.04 & 0.02 & 0 & 0.37 & 0.02 & 0.08 & 0.16 & 0 & 1 & 0.01 & 0.11 & 0 & 0.01 & 0.51 & 0 & 0 & 0.08 & 0 & 0.16 & 0.01 & 0.12 & 0.33 & 0.04 & 0 & 0 & 0.03 \\
 & 13 & 0.12 & 0.35 & 0.32 & 0.24 & 0.38 & 0.34 & 0.08 & 0.12 & 0.23 & 0.02 & 0.23 & 0.02 & 1 & 0.30 & 0.22 & 0.38 & 0.14 & 0.34 & 0.51 & 0.22 & 0.56 & 0.19 & 0.23 & 0.33 & 0.01 & 0.20 & \textbf{0.40} & 0.42 & 0.43 \\
 & 14 & 0.07 & 0.16 & 0.49 & 0.16 & 0.34 & 0.38 & 0.05 & 0.10 & 0.16 & 0.59 & 0.44 & 0.40 & 0.31 & 1 & 0.27 & 0.41 & 0.40 & 0.33 & 0.14 & 0.47 & 0.33 & 0.25 & 0.42 & 0.33 & 0.52 & 0.06 & 0.39 & 0.10 & 0.21 \\
 & 15 & 0.13 & 0.11 & 0.06 & 0.09 & 0.37 & 0.02 & 0.05 & 0.02 & 0.04 & 0.04 & 0.09 & 0 & 0.08 & 0.09 & 1 & 0.07 & 0 & 0.05 & 0.05 & 0.01 & 0.14 & 0.06 & 0.01 & 0.04 & 0.02 & 0.12 & 0.06 & 0.17 & 0.14 \\
 & 16 & 0.06 & 0.08 & 0.01 & 0.06 & 0.06 & 0 & 0.08 & 0.04 & 0.05 & 0.03 & 0.24 & 0.01 & 0.17 & 0.17 & 0.09 & 1 & 0.04 & 0.31 & 0.13 & 0.11 & 0.14 & 0.08 & 0.30 & 0.04 & 0.01 & 0 & 0.15 & 0.23 & 0.21 \\
 & 17 & 0 & 0.04 & 0 & 0 & 0.03 & 0 & 0 & 0 & 0.09 & 0 & 0.05 & 0 & 0.12 & 0.03 & 0.04 & 0.06 & 0.05 & 0.05 & 1 & 0.05 & 0.17 & 0.04 & 0.10 & 0.03 & 0.01 & 0.19 & 0 & 0.25 & 0.14 \\
 & 18 & 0.02 & 0.02 & 0 & 0.04 & 0 & 0.02 & 0.08 & 0 & 0.01 & 0.17 & 0.01 & 0.48 & 0.04 & 0.10 & 0 & 0.02 & 1 & 0 & 0.06 & 0.13 & 0.01 & 0.10 & 0.02 & 0.18 & 0.24 & 0 & 0 & 0 & 0.06 \\
 & 19 & 0.01 & 0.04 & 0 & 0.05 & 0.03 & 0.02 & 0.02 & 0.08 & 0 & 0.09 & 0.08 & 0 & 0.08 & 0.07 & 0.03 & 0.16 & 0 & 1 & 0.06 & 0.05 & 0 & 0.13 & 0 & 0.02 & 0.02 & 0 & 0.04 & 0.04 & 0.10 \\
 & 20 & 0.02 & 0.04 & 0.06 & 0.01 & 0.02 & 0 & 0.02 & 0.07 & 0.02 & 0.22 & 0.08 & 0.10 & 0.08 & 0.16 & 0.01 & 0.09 & 0.16 & 0.07 & 0.07 & 1 & 0 & 0.05 & 0.23 & 0.05 & 0.27 & 0.03 & 0 & 0.04 & 0.05 \\
 & 21 & 0 & 0.19 & 0.07 & 0 & 0.01 & 0 & 0 & 0 & 0.01 & 0 & 0.04 & 0 & 0.12 & 0.07 & 0.09 & 0.07 & 0.01 & 0 & 0.17 & 0 & 1 & 0.04 & 0.05 & 0.02 & 0 & 0.03 & 0.01 & 0.08 & 0.10 \\
 & 22 & 0.13 & 0.28 & 0.14 & 0.17 & 0.27 & 0.14 & 0.37 & 0.66 & 0.21 & 0.25 & 0.25 & 0.42 & 0.14 & 0.18 & 0.13 & 0.14 & 0.27 & 0.41 & 0.14 & 0.12 & 0.14 & 1 & 0.19 & 0.18 & 0.30 & 0.30 & 0.23 & 0.08 & 0.04 \\
 & 23 & 0 & 0.09 & 0 & 0 & 0.01 & 0 & 0.02 & 0 & 0 & 0.25 & 0.31 & 0.01 & 0.06 & 0.11 & 0.01 & 0.18 & 0.02 & 0 & 0.12 & 0.18 & 0.06 & 0.07 & 1 & 0.04 & 0.18 & 0.03 & 0 & 0.05 & 0.06 \\
 & 24 & 0.49 & 0.16 & 0.09 & 0.39 & 0.22 & 0.42 & 0.06 & 0 & 0.43 & 0.06 & 0.04 & 0.23 & 0.18 & 0.17 & 0.07 & 0.05 & 0.36 & 0.04 & 0.08 & 0.08 & 0.06 & 0.13 & 0.08 & 1 & 0.10 & 0 & 0.29 & 0.05 & 0.07 \\
 & 25 & 0.02 & 0.01 & 0.37 & 0.07 & 0.02 & 0.06 & 0.18 & 0.11 & 0.01 & 0.57 & 0.15 & 0.53 & 0 & 0.23 & 0.03 & 0.01 & 0.41 & 0.04 & 0.01 & 0.37 & 0 & 0.19 & 0.31 & 0.08 & 1 & 0.06 & 0.02 & 0.01 & 0.02 \\
 & 26 & 0 & 0.01 & 0 & 0.01 & 0 & 0.02 & 0 & 0.02 & 0.07 & 0.01 & 0.01 & 0.02 & 0.03 & 0.01 & 0.05 & 0 & 0 & 0 & 0.11 & 0.01 & 0.01 & 0.05 & 0.01 & 0 & 0.02 & 1 & 0 & 0.08 & 0.07 \\
 & 27 & 0.09 & 0.11 & 0.01 & 0.36 & 0.02 & 0 & 0.02 & 0 & 0.05 & 0.09 & 0 & 0 & 0.08 & 0.07 & 0.04 & 0.07 & 0 & 0.03 & 0 & 0 & 0.01 & 0.06 & 0 & 0.10 & 0.01 & 0 & 1 & 0 & 0.05 \\
 & 28 & 0.05 & 0.02 & 0 & 0 & 0.02 & 0 & 0.21 & 0 & 0.14 & 0 & 0.01 & 0 & 0.11 & 0.03 & 0.13 & 0.14 & 0 & 0.05 & 0.30 & 0.03 & 0.09 & 0.03 & 0.05 & 0.02 & 0.01 & 0.16 & 0 & 1 & 0.19 \\
 & 30 & 0.21 & 0.18 & 0.17 & 0.12 & 0.23 & 0.15 & 0.22 & 0.03 & 0.23 & 0.06 & 0.23 & 0.09 & 0.36 & 0.17 & 0.36 & 0.40 & 0.20 & 0.38 & 0.51 & 0.13 & 0.38 & 0.04 & 0.18 & 0.11 & 0.04 & 0.44 & 0.23 & 0.61 & 1 \\

%%%%%%%%%%%%%%%%%%%%%%%%%%%%%%%%%%%%%%%%%%%
% Misprediction
%%%%%%%%%%%%%%%%%%%%%%%%%%%%%%%%%%%%%%%%%%%
\hline \hline
\rowcolor[HTML]{D9D9D9}
\multicolumn{31}{c}{(c) \textbf{Misprediction}}\\
\hline \hline

 \multirow{30}{*}{\rotatebox{90}{Predicted Class ID $\downarrow$}}
 & 1 & 0 & 0.03 & 0.01 & 0.03 & 0.01 & 0.02 & 0 & 0 & 0.05 & 0 & 0 & 0 & 0.01 & 0.01 & 0.01 & 0.02 & 0 & 0 & 0.01 & 0.01 & 0.01 & 0.01 & 0 & 0.04 & 0 & 0 & 0.06 & 0 & 0 \\
 & 2 & 0.03 & 0 & 0.03 & 0.06 & 0.03 & 0 & 0.02 & 0.03 & 0 & 0.02 & 0.01 & 0 & 0.04 & 0.01 & 0.01 & 0.03 & 0 & 0.01 & 0.02 & 0.01 & 0.09 & 0.02 & 0 & 0.04 & 0 & 0 & 0.10 & 0.02 & 0.05 \\
 & 3 & 0 & 0.01 & 0 & 0 & 0 & 0 & 0 & 0 & 0 & 0.01 & 0 & 0 & 0 & 0.03 & 0 & 0.01 & 0 & 0 & 0 & 0.02 & 0 & 0.02 & 0 & 0 & 0.02 & 0 & 0 & 0 & 0 \\
 & 4 & 0.03 & 0.03 & 0 & 0 & 0 & 0 & 0 & 0 & 0.01 & 0.04 & 0 & 0 & 0.01 & 0.01 & 0.02 & 0.01 & 0.01 & 0 & 0.01 & 0.01 & 0.01 & 0.01 & 0.01 & 0.04 & 0.01 & 0 & 0.17 & 0.01 & 0.01 \\
 & 5 & 0.01 & 0 & 0 & 0 & 0 & 0 & 0 & 0 & 0 & 0 & 0 & 0.01 & 0 & 0 & 0 & 0.01 & 0 & 0 & 0.04 & 0 & 0 & 0 & 0 & 0.01 & 0 & 0 & 0.04 & 0 & 0 \\
 & 6 & 0 & 0.01 & 0.06 & 0.01 & 0 & 0 & 0 & 0 & 0 & 0 & 0.01 & 0 & 0.01 & 0.01 & 0.01 & 0.01 & 0.01 & 0 & 0 & 0 & 0 & 0 & 0 & 0.01 & 0.01 & 0 & 0 & 0 & 0.01 \\
 & 7 & 0 & 0 & 0 & 0 & 0 & 0 & 0 & 0 & 0.01 & 0 & 0 & 0.01 & 0.01 & 0 & 0 & 0.01 & 0.01 & 0 & 0 & 0 & 0 & 0.01 & 0 & 0 & 0 & 0 & 0 & 0.01 & 0.01 \\
 & 8 & 0 & 0 & 0 & 0 & 0 & 0 & 0 & 0 & 0 & 0 & 0.01 & 0 & 0 & 0 & 0 & 0 & 0 & 0.01 & 0 & 0 & 0 & 0.01 & 0 & 0 & 0.01 & 0 & 0 & 0 & 0 \\
 & 9 & 0.07 & 0.02 & 0 & 0.04 & 0 & 0 & 0 & 0 & 0 & 0 & 0 & 0.01 & 0.01 & 0.02 & 0.02 & 0.02 & 0 & 0 & 0 & 0.01 & 0.02 & 0 & 0 & 0.02 & 0.01 & 0 & 0.05 & 0.03 & 0.02 \\
 & 10 & 0 & 0.01 & 0 & 0 & 0 & 0 & 0 & 0 & 0 & 0 & 0 & 0.02 & 0 & 0.03 & 0.01 & 0.01 & 0.01 & 0 & 0 & 0.04 & 0.01 & 0 & 0.01 & 0 & 0.06 & 0 & 0.03 & 0.01 & 0.01 \\
 & 11 & 0.02 & 0.01 & 0 & 0 & 0.01 & 0 & 0.02 & 0 & 0 & 0 & 0 & 0.01 & 0.01 & 0.01 & 0.01 & 0.03 & 0.04 & 0 & 0 & 0.01 & 0.01 & 0 & 0 & 0 & 0.02 & 0 & 0.01 & 0.02 & 0.03 \\
 & 12 & 0.01 & 0 & 0 & 0 & 0 & 0 & 0.09 & 0 & 0 & 0.02 & 0 & 0 & 0 & 0.01 & 0 & 0 & 0 & 0 & 0 & 0.02 & 0 & 0.02 & 0 & 0.02 & 0.01 & 0 & 0 & 0 & 0 \\
 & 13 & 0.03 & 0.06 & 0.16 & 0.09 & 0.10 & 0.03 & 0.02 & 0 & 0.03 & 0 & 0.09 & 0 & 0 & 0.06 & 0.09 & 0.16 & 0.04 & 0.03 & 0.23 & 0.04 & 0.11 & 0.02 & 0.01 & 0.04 & 0.01 & 0.03 & \textbf{0.43} & 0.24 & 0.16 \\
 & 14 & 0 & 0.06 & 0.08 & 0 & 0.05 & 0 & 0 & 0.07 & 0.01 & 0.10 & 0.05 & 0.04 & 0 & 0 & 0.07 & 0.09 & 0.07 & 0.03 & 0.07 & 0.15 & 0.11 & 0.02 & 0.02 & 0.07 & 0.09 & 0.02 & 0.25 & 0.07 & 0.05 \\
 & 15 & 0.03 & 0.01 & 0 & 0.02 & 0.05 & 0 & 0 & 0 & 0 & 0.01 & 0 & 0 & 0.01 & 0 & 0 & 0.02 & 0 & 0.01 & 0.02 & 0 & 0.04 & 0 & 0 & 0.01 & 0 & 0 & 0.05 & 0.05 & 0.02 \\
 & 16 & 0.02 & 0.01 & 0.01 & 0.01 & 0.03 & 0 & 0.02 & 0.02 & 0 & 0.02 & 0.03 & 0.01 & 0.04 & 0.04 & 0 & 0 & 0.02 & 0.09 & 0.04 & 0.04 & 0.01 & 0.01 & 0 & 0.01 & 0.01 & 0.02 & 0.10 & 0.14 & 0.11 \\
 & 17 & 0.01 & 0 & 0.03 & 0 & 0 & 0 & 0 & 0 & 0.01 & 0 & 0.03 & 0 & 0.02 & 0.02 & 0 & 0 & 0.03 & 0.01 & 0 & 0 & 0 & 0.01 & 0 & 0.01 & 0 & 0.02 & 0.03 & 0.07 & 0.04 \\
 & 18 & 0.01 & 0 & 0 & 0 & 0 & 0 & 0.04 & 0 & 0 & 0.02 & 0 & 0 & 0 & 0.01 & 0.02 & 0 & 0 & 0 & 0 & 0.02 & 0 & 0 & 0 & 0.01 & 0.01 & 0 & 0 & 0 & 0 \\
 & 19 & 0 & 0.01 & 0 & 0.01 & 0 & 0 & 0 & 0.06 & 0 & 0.01 & 0.01 & 0 & 0 & 0.01 & 0 & 0.01 & 0 & 0 & 0 & 0.02 & 0 & 0.01 & 0 & 0 & 0 & 0 & 0.01 & 0.01 & 0.01 \\
 & 20 & 0.01 & 0.04 & 0 & 0.02 & 0.02 & 0 & 0 & 0 & 0 & 0.01 & 0.01 & 0.01 & 0.03 & 0.01 & 0 & 0.03 & 0.05 & 0.01 & 0 & 0 & 0.01 & 0.01 & 0 & 0.01 & 0.03 & 0 & 0.04 & 0.02 & 0.03 \\
 & 21 & 0 & 0.01 & 0.07 & 0 & 0 & 0 & 0 & 0 & 0 & 0 & 0.01 & 0 & 0.01 & 0 & 0 & 0 & 0 & 0 & 0.03 & 0 & 0 & 0 & 0 & 0 & 0 & 0 & 0.01 & 0.04 & 0.02 \\
 & 22 & 0.03 & 0.01 & 0.02 & 0.04 & 0.03 & 0.04 & 0.06 & 0.24 & 0.04 & 0.07 & 0 & 0.05 & 0.03 & 0.04 & 0.06 & 0.02 & 0.01 & 0 & 0 & 0.04 & 0 & 0 & 0 & 0.03 & 0.02 & 0.03 & 0.08 & 0.02 & 0.01 \\
 & 23 & 0.02 & 0 & 0 & 0 & 0.02 & 0 & 0 & 0 & 0 & 0 & 0.01 & 0 & 0 & 0.01 & 0.01 & 0.02 & 0.01 & 0 & 0.01 & 0.04 & 0 & 0 & 0 & 0.01 & 0.01 & 0.02 & 0 & 0.02 & 0.03 \\
 & 24 & 0.07 & 0.04 & 0.01 & 0.08 & 0.03 & 0.03 & 0.04 & 0 & 0.06 & 0.03 & 0.01 & 0.03 & 0.02 & 0.03 & 0.03 & 0.03 & 0.08 & 0 & 0.01 & 0.02 & 0.01 & 0.01 & 0 & 0 & 0.03 & 0 & 0.08 & 0 & 0 \\
 & 25 & 0.01 & 0.01 & 0.02 & 0 & 0.02 & 0 & 0.04 & 0.04 & 0.01 & 0.05 & 0.01 & 0.06 & 0.01 & 0.05 & 0.02 & 0.02 & 0.07 & 0 & 0.01 & 0.09 & 0.02 & 0.02 & 0.02 & 0 & 0 & 0 & 0.01 & 0 & 0.01 \\
 & 26 & 0.01 & 0.01 & 0 & 0.01 & 0.01 & 0.02 & 0 & 0 & 0.01 & 0 & 0.01 & 0.01 & 0.01 & 0.01 & 0.03 & 0 & 0 & 0.02 & 0 & 0.02 & 0.01 & 0.01 & 0 & 0 & 0 & 0 & 0.01 & 0.02 & 0.01 \\
 & 27 & 0 & 0.01 & 0 & 0.02 & 0 & 0 & 0 & 0 & 0 & 0.03 & 0 & 0 & 0.01 & 0.01 & 0.02 & 0 & 0 & 0.01 & 0.01 & 0 & 0 & 0 & 0 & 0 & 0.01 & 0 & 0 & 0.01 & 0.02 \\
 & 28 & 0 & 0 & 0.01 & 0 & 0.01 & 0.04 & 0 & 0 & 0.01 & 0 & 0.01 & 0 & 0.01 & 0.02 & 0.02 & 0.01 & 0 & 0 & 0.05 & 0.02 & 0.03 & 0.01 & 0 & 0.02 & 0.01 & 0 & 0 & 0 & 0.01 \\
 & 29 & 0 & 0.01 & 0 & 0.02 & 0.01 & 0 & 0.02 & 0 & 0 & 0 & 0 & 0 & 0.01 & 0.01 & 0.01 & 0.01 & 0 & 0 & 0.01 & 0.02 & 0 & 0.01 & 0 & 0.01 & 0 & 0 & 0 & 0 & 0.02 \\
 & 30 & 0.06 & 0.05 & 0.10 & 0.06 & 0.01 & 0 & 0 & 0 & 0.01 & 0.04 & 0.12 & 0.03 & 0.10 & 0.07 & 0.09 & 0.14 & 0.12 & 0.07 & 0.17 & 0.08 & 0.13 & 0.03 & 0.03 & 0.05 & 0.04 & 0.07 & 0.23 & 0.23 & 0 \\
 \hline
\end{tabular}
\end{adjustbox}
\label{tab:misclassification_non_fiction}
\end{table*}

\begin{table*}[hbt]
\centering
\caption{Example of misclassified data samples due to genre indistinguishability.}
\begin{adjustbox}{width=0.95\textwidth}
% \begin{adjustbox}{angle=90, height=1\textheight}
% \footnotesize
\begin{tabular}{c|ll}%p{0.9\textwidth}}

\hline \hline

\rowcolor[HTML]{D9D9D9}
\multicolumn{3}{c}{\textbf{\emph{(a)} 9780671501075: Dragon's Honor (Star Trek: The Next Generation, No. 38); Author: Kij Johnson; Publisher: Star Trek}}\\
\hline \hline
& \\ [\dimexpr-\normalbaselineskip+1.5pt]

\multirow{8}{*}{\includegraphics[width=0.08\linewidth]{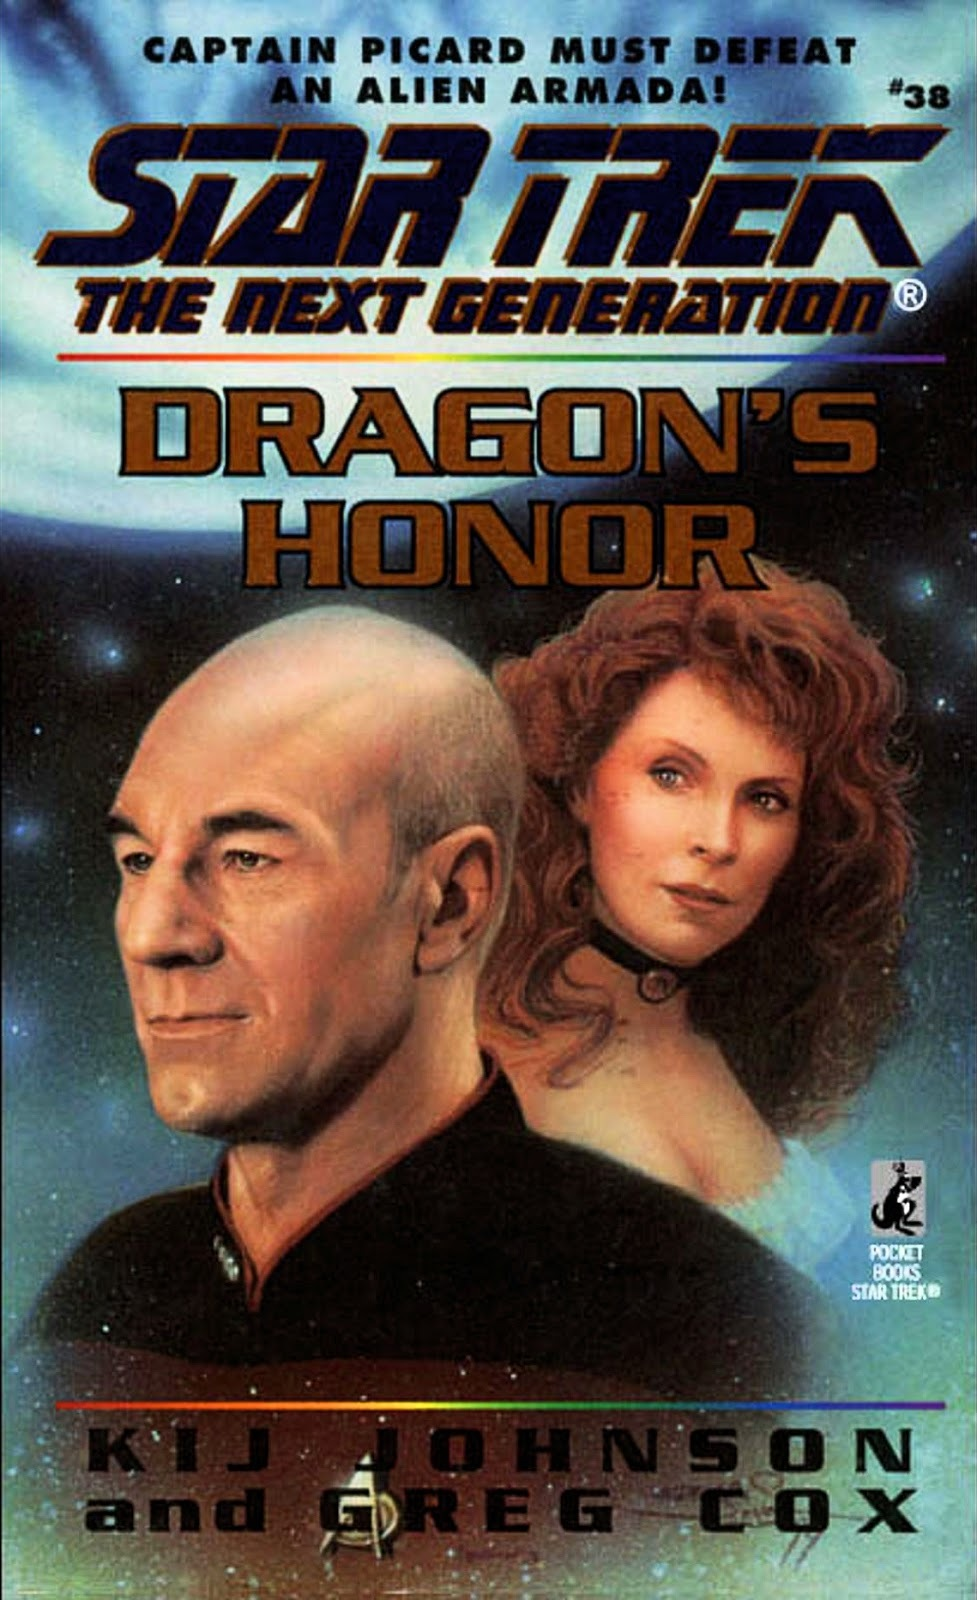}} & \multirow{5}{*}{\textbf{Blurb}:} & Isolated for centuries, the exotic Dragon Empire is finally ready to join the United Federation of Planets. But first the emperor's eldest son must marry the only   \\
 &  & daughter of his oldest enemy, bringing to an end decades of civil war. Without the wedding, there can be no peace -- and no treaty with the Federation.As honored \\
 & & guests of  the  Dragon Empire, Captain Picard and the crew of the "Starship Enterprise" TM must ensure that the royal wedding occurs on schedule, despite the  \\
 & & Empire's complicated and difficult codes of honor. And Dr. Beverly Crusher finds her loyalties torn when she wins the confidence of the unusually reluctant  \\
 & & bride-to-be.  More than just of the Federation. Picard a treaty is at stake, for a vicious race of alien conquerors will stop at nothing, from assassination to invasion,\\
 & &   to keep the Empire out must use all  his skills to save the Empire, and preserve the Dragon's Honor.\\
\cline{2-3}
% & ${\cal{M}}$ & \{"author":"Kij Johnson","publisher":"Star Trek"\}\\ \hline

& \multicolumn{1}{l}{\textbf{Actual Genre}:} & (Fiction, \{Press \& Media, Sci-Fi\})\\ \cline{2-3} %\hline

& \multicolumn{1}{l}{\textbf{Predicted Genre}:} & (Fiction, \{Sci-Fi\})\\

\hline \hline

\rowcolor[HTML]{D9D9D9}
\multicolumn{3}{c}{\textbf{\emph{(b)} 9780380808175: T2: Rising Storm (T2); Author: S.M. Stirling; Publisher: HarperEntertainment}}\\
\hline \hline
& \\ [\dimexpr-\normalbaselineskip+1.5pt]

\multirow{6}{*}{\includegraphics[width=0.08\linewidth]{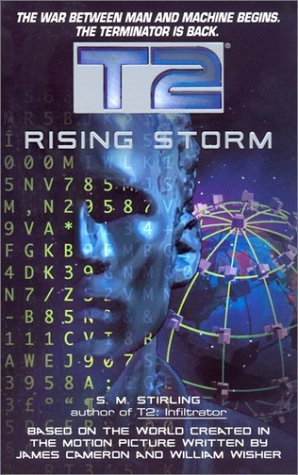}} & \multirow{4}{*}{\textbf{Blurb}:} & \multirow{4}{*}{The war is far from over ... Those who fight for the future face the ultimate challenge ... As the electronic brain behind humanity's destruction comes alive.} \\
 &  & \\
  &  & \\
  &  & \\
\cline{2-3}
% & ${\cal{M}}$ & \{"author":"S.M. Stirling","publisher":"HarperEntertainment"\}\\ \hline

& \multicolumn{1}{l}{\textbf{Actual Genre}:} & (Fiction, \{Mystery \& Thriller \& Suspense \& Horror, Press \& Media, Sci-Fi\})\\ \cline{2-3} %\hline

& \multicolumn{1}{l}{\textbf{Predicted Genre}:} & (Fiction, \{Humanities, Mystery \& Thriller \& Suspense \& Horror, Medical, Sci-Fi\})\\

\hline \hline

\rowcolor[HTML]{D9D9D9}
\multicolumn{3}{c}{\textbf{\emph{(c)} 9781569711293: Star Wars: Battle of the Bounty Hunters; Author: Ryder Windham; Publisher: Dark Horse Comics}}\\
\hline \hline
& \\ [\dimexpr-\normalbaselineskip+1.5pt]

\multirow{6}{*}{\includegraphics[width=0.08\linewidth]{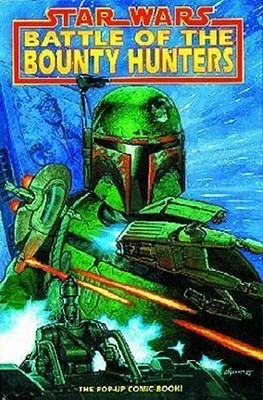}} & \multirow{4}{*}{\textbf{Blurb}:} &  \\
 & & Battle of the Bounty Hunters was a pop-up comic and part of the Star Wars: Shadows of the Empire multimedia campaign. It showed the space battle between \\
 &  &  Boba Fett and IG-88D.\\
 &  &  \\
\cline{2-3}
% & ${\cal{M}}$ & \{"author":"Ryder Windham","publisher":"Dark Horse Comics"\}\\ \hline

& \multicolumn{1}{l}{\textbf{Actual Genre}:} & (Fiction, \{Comics \& Graphic, Press \& Media, Sci-Fi\})\\ \cline{2-3} %\hline

& \multicolumn{1}{l}{\textbf{Predicted Genre}:} & (Fiction, \{Comics \& Graphic, Sci-Fi\})\\ 

\hline \hline

\rowcolor[HTML]{D9D9D9}
\multicolumn{3}{c}{\textbf{\emph{(d)} 9780425051849: 
 Dance of the Tiger; Author: Bjorn Kurten; Publisher: Berkley Publishing Group}}\\
\hline \hline
& \\ [\dimexpr-\normalbaselineskip+1.5pt]

\multirow{6}{*}{\includegraphics[width=0.08\linewidth]{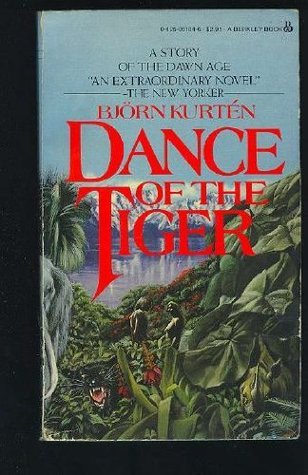}} & \multirow{4}{*}{\textbf{Blurb}:} & \multirow{2}{*}{Björn Kurtén's compelling novel gives the reader a detailed picture of life 35,000 years ago in Western Europe. One of the world's leading scholars of Ice Age}   \\
& & \multirow{2}{*}{fauna, Kurtén fuses extraordinary knowledge and imagination in this vivid evocation of our deepest past. This novel illuminates the lives of the humans who left}    \\ 
& & \multirow{2}{*}{us magnificent paintings in the caves of France and Spain.} \\ 
& & \\ \cline{2-3}

% & ${\cal{M}}$ & \{"author":"Bjorn Kurten","publisher":"Berkley Publishing Group"\}\\ \hline
& \multicolumn{1}{l}{\textbf{Actual Genre}:} & (Fiction, \{History, Humanities, Sci-Fi\})\\ \cline{2-3} %\hline

& \multicolumn{1}{l}{\textbf{Predicted Genre}:} & (Fiction, \{Environment \& Plant, History, Literature, Travel, Sci-Fi\})\\

\hline \hline

\rowcolor[HTML]{D9D9D9}
\multicolumn{3}{c}{\textbf{\emph{(e)} 9780789425225: Voices in the Park; Author: Anthony Browne; Publisher: Dorling Kindersley Publishing}}\\
\hline \hline
& \\ [\dimexpr-\normalbaselineskip+1.5pt]

\multirow{5}{*}{\includegraphics[width=0.08\linewidth]{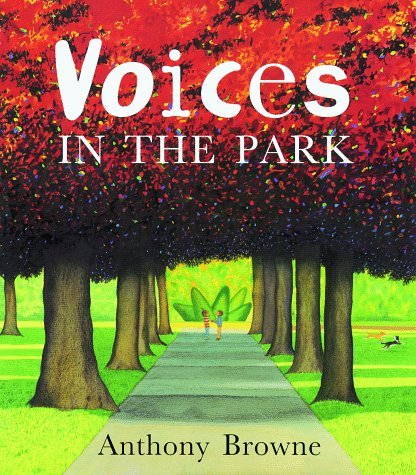}} & \multirow{3}{*}{\textbf{Blurb}:} & \multirow{2}{*}{Four people enter a park and through their eyes young readers see different visions, from the bossy woman and the sad man to the lonely boy and the warm young} \\

 &  &  \multirow{2}{*}{girl, moving from one voice to another and shifting landscapes and seasons.} \\

  &  & \\

\cline{2-3}
% & ${\cal{M}}$ & \{"author":"Anthony Browne","publisher":"Dorling Kindersley Publishing"\}\\ \hline
& \multicolumn{1}{l}{\textbf{Actual Genre}:} & (Fiction, \{Animals \& Wildlife \& Pets, Arts \& Photography, {Childrens\textquoteright} Book, Family \& Parenting \& Relationships, Teen \& Young Adult\})\\ \cline{2-3} %\hline

& \multicolumn{1}{l}{\textbf{Predicted Genre}:} & (Fiction, \{Arts \& Photography, {Childrens\textquoteright} Book, Family \& Parenting \& Relationships, Teen \& Young Adult\})\\ %\hline

\hline \hline

\rowcolor[HTML]{D9D9D9}
\multicolumn{3}{c}{\textbf{\emph{(f)} 9780894712661: The Classic Tale of Velveteen Rabbit or How Toys Become Real; Author: Margery Williams; Publisher: Running Press}}\\
\hline \hline
& \\ [\dimexpr-\normalbaselineskip+1.5pt]

\multirow{5}{*}{\includegraphics[width=0.08\linewidth]{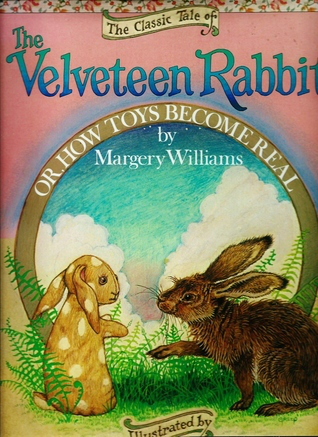}} & \multirow{3}{*}{\textbf{Blurb}:} & \multirow{2}{*}{A beautiful large-format edition of this timeless children's tale, replete with enchanting full-color illustrations. A charming fable with the moral that love can make} \\
& & \multirow{2}{*}{all things real and beautiful. 10" x 13".}\\ 
& & \\ \cline{2-3}

% & ${\cal{M}}$ & \{"author":"Margery Williams","publisher":"Courage Books"\}\\ \hline
& \multicolumn{1}{l}{\textbf{Actual Genre}:} & (Fiction, \{Animals \& Wildlife \& Pets, Arts \& Photography, {Childrens\textquoteright} Book, Literature, Sci-Fi, Teen \& Young Adult\})\\ \cline{2-3} %\hline

& \multicolumn{1}{l}{\textbf{Predicted Genre}:} & (Fiction, \{Arts \& Photography, {Childrens\textquoteright} Book, Literature, Mythology \& Religion \& Spirituality, Teen \& Young Adult, Sci-Fi\})\\
% \hline

\hline \hline

\rowcolor[HTML]{D9D9D9}
\multicolumn{3}{c}{\textbf{\emph{(g)} 9780440436836: Homesick: My Own Story; Author: Jean Fritz; Publisher: Yearling Books}}\\
\hline \hline
& \\ [\dimexpr-\normalbaselineskip+1.5pt]

\multirow{8}{*}{\includegraphics[width=0.08\linewidth]{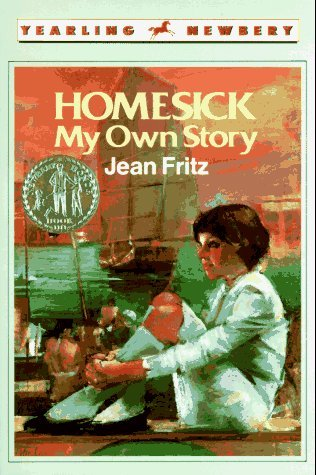}} & \multirow{6}{*}{\textbf{Blurb}:} & Jean Fritz was born in China and lived there until 1927, when she was twelve. Young Jean had spent her entire life in China, but her parents' memories of home  \\
 &  & and letters from relatives in  Pennsylvania made her feel that she was American--and homesick for a place she'd never seen!Family photographs and illustrations   \\
 & &  by Margot Tomes show us the real people behind Jean's vivid and unforgettable stories--memories of picnics on the Great Wall, pranks, holidays in the foreign \\
 & &  compound, rebellious moments at her British school. close ties to Chinese friends, and how it felt to be called a "foreign devil" and spat upon in the streets of \\
 & &  a turbulent China on the eve of revolution. When her family embarks upon its long journey home, Jean is thrilled, but she When she arrives in America at last,  \\
  & & will she fit in after growing up on "the wrong side of the world?" \\
 
\cline{2-3}
% & ${\cal{M}}$ & \{"author":"Jean Fritz","publisher":"Yearling Books"\}\\ \hline
& \multicolumn{1}{l}{\textbf{Actual Genre}:} & (Non-fiction, \{Biographies \& Memoir, {Childrens\textquoteright} Book, History, Teen \& Young Adult\})\\ \cline{2-3} %\hline

& \multicolumn{1}{l}{\textbf{Predicted Genre}:} & (Non-fiction, \{{Childrens\textquoteright} Book, History, Biographies \& Memoir\})\\ %\hline

\hline \hline

\rowcolor[HTML]{D9D9D9}
\multicolumn{3}{c}{\textbf{\emph{(h)} 9780345291363: Elephant Man; Author: Christine Sparks; Publisher: Ballantine Books}}\\
\hline \hline
& \\ [\dimexpr-\normalbaselineskip+1.5pt]

\multirow{7}{*}{\includegraphics[width=0.08\linewidth]{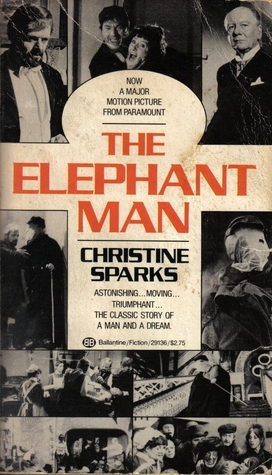}} & \multirow{5}{*}{\textbf{Blurb}:} &  \\
& & John Merrick had lived for more than twenty years imprisoned in a body that condemned him to a miserable life in the workhouse and to humiliation as a circus   \\
 &  & sideshow freak. But beneath  that tragic exterior, within that enormous and deformed head, thrived the soul of a poet, the heart of a dreamer, the longings of a    \\
 & &  man. Based on the extraordinary motion picture that captured the heart of America.\\
  & & \\
 
\cline{2-3}
% & ${\cal{M}}$ & \{"author":"Christine Sparks","publisher":"Ballantine Books"\}\\ \hline
& \multicolumn{1}{l}{\textbf{Actual Genre}:} & (Non-fiction, \{Biographies \& Memoir, History, Literature, Teen \& Young Adult\})\\ \cline{2-3} %\hline

& \multicolumn{1}{l}{\textbf{Predicted Genre}:} & (Non-fiction, \{History, Literature, Biographies \& Memoir\})\\ \hline

\end{tabular}
\end{adjustbox}

\label{tab:indistinguish_sample}

\end{table*}

\begin{table*}[!hbt]
\centering
\caption{Misprediction due to Level-1 classification}
\begin{adjustbox}{width=0.95\textwidth}
% \begin{adjustbox}{angle=90, height=1\textheight}
% \footnotesize
\begin{tabular}{c|ll}%p{0.9\textwidth}}
% \multicolumn{3}{c}{(a) Samples for heatmap analysis}\\

\hline \hline
\rowcolor[HTML]{D9D9D9}
\multicolumn{3}{c}{\textbf{{\emph{(a)}} 9780312266820: Dead Egotistical Morons: A Paul Turner Mystery; Author: Mark Richard Zubro; Publisher: St. Martin's Press}}\\
\hline \hline

\multirow{11}{*}{\includegraphics[width=0.1\linewidth]{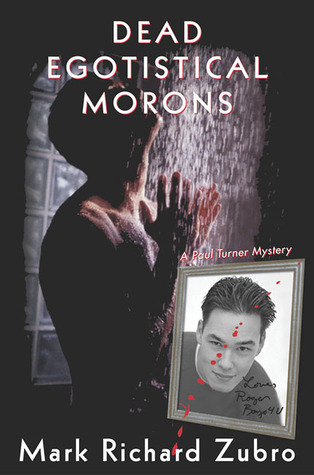}} & \multirow{8}{*}{\textbf{Blurb}:} & Boys4U is the world's most popular singing group - at least among teenaged girls - and they have closed out their sold-out world tour with a series of shows \\
& &   in Chicago's brand new arena. The premier group of the inexplicably popular "boy band" trend, they've just finished their very last concert of the tour. While  \\
& & hundreds of tour members, well-wishers, executives, and various hangers on wait to celebrate another wildly successful tour, the lead singer is found murdered  \\
& &   - shot in the back of the head at close range - in the shower all times, the only other people back there were the other members of the band, and  none of the \\
& &   dozens of people in the next room report having heard a shot. While the international press is engaged of the backstage dressing area. To make matters more    \\
& & distressing, the crime itself was almost impossible - there was tight security on the shower area at in an unprecedented feeding frenzy over the sensationalistic \\
& & murder, Chicago Police Detectives Paul Turner and his partner Buck Fenwick have pulled the unenviable task of investigating the murder But even the initial \\
& &  appearances are deceiving and as they dig deeper into the case, they uncover more disturbing truths beneath the wholesome façade of Boys4U. Now they have \\
& &  untangle an increasingly complex web if they are to stop a determined killer before more victims are claimed. \\
\cline{2-3}

% & ${\cal{M}}$ & \{"author":"Mark Richard Zubro","publisher":"St. Martin's Press"\}\\ \hline

& \multicolumn{1}{l}{\textbf{Actaul Genre}:} & (Fiction, \{Fashion \& Lifestyle, Mystery \& Thriller \& Suspense \& Horror\})\\ \cline{2-3} %\hline
& \multicolumn{1}{l}{\textbf{Predicted Genre}:} & (Non-fiction, \{Arts \& Photography\}) \\

\hline \hline
\rowcolor[HTML]{D9D9D9}
\multicolumn{3}{c}{\textbf{{\emph{(b)}} 9780312979256: Mafia Marriage; Author: Rosalie Bonanno; Publisher: St. Martin's Paperbacks}}\\
\hline \hline

\multirow{9}{*}{\includegraphics[width=0.08\linewidth]{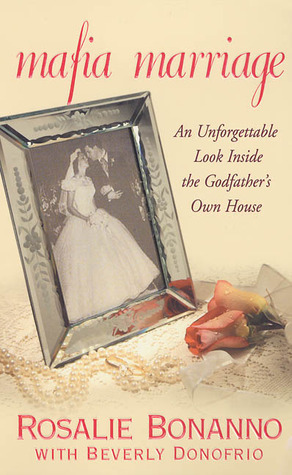}} & \multirow{6}{*}{\textbf{Blurb}:} & An Unforgettable Look Inside the Godfather's Own HouseShe Was A Profaci. He Was A BonannoRosalie Profaci was a Mafia princess. Salvatore "Bill" \\
& &   Bonanno, oldest son of   Mafia Don Joe Bonanno, the real-life model for The Godfather, was organized crime's crown prince. And Bill, deeply involved in his \\
& &   father's "business" of mob schemes thought  pretty Rosalie knew what it meant to be a "Mafia wife." But the convent-raised, deeply devout Rosalie, whose \\
& &   innocence was protected by her doting father, had no idea...Their  Marriage United Two Mafia Dynasties...Mafia Marriage is Rosalie Bonanno's intimate \\
& &  account of life inside the secretive world of the Mafia. Naming names and providing shocking details, she writes about the wild spending sprees, the \\
& &   mysterious absences of her husband, the other women in his-their running from the law, the abductions, and shootings. Above all, Rosalie reveals the passion\\
& &  that kept her virtually a prisoner to love...and her heartbreaking journey of discovering the truth and trying to break free. \\

\cline{2-3}

% & ${\cal{M}}$ & \{"author":"Rosalie Bonanno","publisher":"St. Martin's Paperbacks"\}\\ \hline

& \multicolumn{1}{l}{\textbf{Actaul Genre}:} & (Non-fiction, \{Biographies \& Memoir, Mystery \& Thriller \& Suspense \& Horror\})\\ \cline{2-3} %\hline
& \multicolumn{1}{l}{\textbf{Predicted Genre}:} & (Fiction, \{History, Romance, Teen \& Young Adult\}) \\

\hline

% \multicolumn{3}{r}{${\cal{I}}$: Coverpage Image, ${\cal{T}}$: Description Text, ${\cal{M}}$: Metadata}
\end{tabular}
\end{adjustbox}

\label{tab:model_limitation}

\end{table*}

% \clearpage

\subsection{Quantitative and Qualitative Analysis for Genre Indistinguishability}
\noindent
Our investigation into misclassification suggests that the genre co-occurrence might be a contributing factor. Table \ref{tab:misclassification_fiction}: (a) and \ref{tab:misclassification_non_fiction}: (a) present pair-wise genre sample count for \textit{fiction} and \textit{non-fiction} genre in ${\cal{D}}_{train}$. Each cell in the table represents the number of samples belonging to both the row and column genre class ids. Table \ref{tab:misclassification_fiction}: (b) and \ref{tab:misclassification_non_fiction}: (b) illustrates the co-occurrence ratio between row class ID $i$ in association with column class ID $j$ for \textit{fiction} and \textit{non-fiction} genres respectively. Each cell contains the ratio of samples belonging to both class ids $i$ and $j$ to the total number of training samples associated with class ID $j$. Table \ref{tab:misclassification_fiction}: (c) and \ref{tab:misclassification_non_fiction}: (c) reports the misclassification rate by IMAGINE for \textit{fiction} and \textit{non-fiction} genres, respectively. Here, each cell corresponding to row class ID $i$ and column class ID $j$ represents the ratio between the number of testing samples associated with class ID $j$ but wrongly identified as class ID $i$ and the total number of testing samples associated with class ID $j$ that have been misclassified.

Our analysis of Table \ref{tab:misclassification_fiction} and \ref{tab:misclassification_non_fiction} suggest that the high co-occurrence of the two genres,  coupled with a significant imbalance in the number of training samples associated with one genre without the other, potentially causes the high misclassification rate. For instance, in Table \ref{tab:misclassification_fiction}, 264 out of 396 \textit{Press \& Media} (class ID 21) books are associated with \textit{Sci-Fi} (class ID 29) genre (refer to Table \ref{tab:misclassification_fiction}: (a)). This leaves only 132 samples that are not categorized as \textit{Sci-Fi}. Conversely, there are 3716 \textit{Sci-Fi} books that do not belong to the \textit{Press \& Media} genre, creating imbalance between non-Sci-Fi \textit{Press \& Media} and non-Press \& Media
\textit{Sci-Fi} samples. This leads to \textit{Press \& Media} genre being misclassified as \textit{Sci-Fi} with the misclassification rate of 0.79. Standard data augmentation methods are limited in their ability to address this imbalance issue, as increasing in the number of samples for \textit{Press \& Media} genre, also increases the \textit{Sci-Fi} samples due to inter-genre relation. We observe similar issue between \textit{Humanities} (class ID 14) and \textit{Literature} (class ID 16) (refer Table \ref{tab:misclassification_fiction}),  \textit{Animals \& Wildlife \& Pets} (class ID 1) and \textit{{Childrens\textquoteright} Book} (class ID 4) (refer Table \ref{tab:misclassification_fiction}), and \textit{non-fiction} genres \textit{Teen \& Young Adult} (class ID 27) and \textit{History} (class ID 13) (refer Table \ref{tab:misclassification_non_fiction}). As a result, relatively lower ${\cal{BA}}$ than other genre was observed for \textit{Press \& Media}, \textit{Humanities}, \textit{Animals \& Wildlife \& Pets} in Table \ref{tab:genrewise_analysis}: (a) and \textit{Teen \& Young Adult} in Table \ref{tab:genrewise_analysis}: (b). 

Table \ref{tab:indistinguish_sample} showcases the example of misclassified data samples due to genre indistinguishability. Here, samples [Table \ref{tab:misclassification_fiction}: \emph{(a)-(c)}] contains \textit{Press \& Media} and \textit{Sci-Fi} as actual genre but IMAGINE can only predict \textit{Sci-Fi }. As mentioned above, it is caused by a high imbalance between non-Sci-Fi \textit{Press \& Media} and non-Press \& Media \textit{Sci-Fi}. Similarly, [\ref{tab:misclassification_fiction}: \emph{(d)}], [\ref{tab:misclassification_fiction}: \emph{(e), (f)}] and [\ref{tab:misclassification_fiction}: \emph{(g), (h)}] show the imbalance between [non-Humanities \textit{Literature} and non-Literature \textit{Humanities}], [non-Animals \& Wildlife \& Pets \textit{{Childrens\textquoteright} Book} and non-{Childrens\textquoteright} Book  \textit{Animals \& Wildlife \& Pets}], respectively.

% \emph{(ii) Qualitative Analysis for Genre Indistinguishability:} Table \ref{tab:indistinguish_sample} showcases the example of misclassified data samples due to genre indistinguishability. As mentioned in appendix \ref{app:analysis_misprediction}.\emph{(i)} and Table \ref{tab:misclassification_fiction},   

\subsection{Qualitative Analysis of Model Limitation:} 
Another significant reason for IMAGINE's mispredictions is the inherent limitations of the model. From Table \ref{tab:model_limitation}, we observe genre misprediction in Level-2 classification due to misclassification in Level-1 classification for some samples (e.g., Table \ref{tab:model_limitation}:  \emph{(a)}). This analysis shows the area of improvement in Level-1 classification to enhance the overall performance of the model.
