# Supplementary material for: Adaptive Data-Resilient Multi-Modal Hierarchical Multi-Label Book Genre Identification
Source: arXiv:2505.03839 source file (2025-10-18)
Supplement: Supplementary file 8 [file 7appendix_stats_info.tex]

\section{Statistical Information}

%Hierarchical Genrewise

%Visual (Resolution, Size)

%Description (word count, processed w/o stopwords)
%\begin{enumerate}

In Table \ref{tab:dataset_table}, we present the hierarchical analysis of book counts by genre. The dataset includes 30 genres. This table provides counts for fiction and nonfiction books separately within each genre. In the table, we can observe overlapping counts across genres due to some books are associated with multiple genres.
The dataset was split up into training (${\cal{D}}_{train}$), validation (${\cal{D}}_{val}$), and testing (${\cal{D}}_{test}$) disjoint sets with an approximate ratio of 8:1:1 considering the presence of all genres in each set equivalently.
Additionally, we employ data augmentation techniques for the cover page images and descriptions to enhance the number of available samples. 
%Before data augmentation, training, validation, and testing sets contained 8972, 1152, and 1178 samples. After data augmentation, training, validation, and testing sets contained 22340, 2804, and 2809 samples.  

Table \ref{tab:all_stats} presents the statistical analysis of each modality before and after augmentation. We have used minimum, maximum, mean ($\mu$), median, and standard deviation ($\sigma$) for statistical analysis. We are measuring the dataset based on the image area for the cover page image, the number of words for the description text and cover text, and the number of books written/published by the author/publisher for metadata.

We also provide the distribution of each modality before and after augmentation. Table \ref{tab:stats_coverpage} shows the area-wise distribution of cover page images. In Fig. \ref{tab:stats_description}, we demonstrate word count-wise distribution of description text. Fig. \ref{tab:stats_cover_text} presents word count-wise distribution of cover text and Fig. \ref{tab:stats_metadata} provides a breakdown of the number of books authored within specific
ranges and the corresponding count of authors who fall into that range, similarly the number of books published within ranges and the number of publishers associated with that range. This analysis provides valuable insights into the dataset.

\begin{table}[!hbt]
 \centering
 \caption{Statistical analysis}
 %\vspace{1em} % Adjust the vertical space here
 \begin{adjustbox}{width=0.47\textwidth}
 \begin{tabular}{c|c|c|c|c|c|c}
\hline
   \textbf{Input} & 
   
& \textbf{Minimum} & \textbf{Maximum} & \textbf{Mean ($\mu$)} & \textbf{Median} & \textbf{SD ($\sigma$)}\\ \hline

& Image area before & \multirow{2}{*}{20460} & \multirow{2}{*}{16301712} & \multirow{2}{*}{435282.41} & \multirow{2}{*}{146775} & \multirow{2}{*}{1125224.73}\\

\textbf{Cover page} & augmentation & & & & & \\
\cline{2-7}
\textbf{images} & Image area after & \multirow{2}{*}{20460} & \multirow{2}{*}{16301712} & \multirow{2}{*}{325205.84} & \multirow{2}{*}{135850} & \multirow{2}{*}{980565.34}\\ 
& augmentation & & & & & \\
\hline

& No. of words before & \multirow{2}{*}{0} & \multirow{2}{*}{1786} & \multirow{2}{*}{120.52} & \multirow{2}{*}{98} & \multirow{2}{*}{102.37}\\ 
   
\textbf{Description} & augmentation & & & & & \\
\cline{2-7}

\textbf{text} & No. of words after & \multirow{2}{*}{0} & \multirow{2}{*}{1953} & \multirow{2}{*}{110.01} & \multirow{2}{*}{96} & \multirow{2}{*}{80.89}\\ 

& augmentation & & & & & \\
\hline

\multirow{4}{*}{\textbf{Cover text}} & No. of words  & \multirow{3}{*}{1} & \multirow{3}{*}{944} & \multirow{3}{*}{20.67} & \multirow{3}{*}{15} & \multirow{3}{*}{27.69}\\

& before augmentation & & & & & \\ \cline{2-7}

 & No. of words  & \multirow{3}{*}{1} & \multirow{3}{*}{944} & \multirow{3}{*}{21.61} & \multirow{3}{*}{16} & \multirow{3}{*}{25.89}\\
& after augmentation & & & & & \\
   
\hline

& No. of books  & \multirow{2}{*}{1} & \multirow{2}{*}{43} & \multirow{2}{*}{1.57} & \multirow{2}{*}{1} & \multirow{2}{*}{1.91}\\ 

\textbf{Metadata} & written by an author & & & & & \\

\cline{2-7}
& No. of books  & \multirow{2}{*}{1} & \multirow{2}{*}{268} & \multirow{2}{*}{5.80} & \multirow{2}{*}{1} & \multirow{2}{*}{16.64}\\ 
   
& published by a publisher & & & & & \\

\hline

   \multicolumn{7}{r}{SD: Standard Deviation}
 \end{tabular}
\end{adjustbox}
\label{tab:all_stats}
 \end{table}

\begin{table}[!hbt]
\centering  
% \footnotesize
% \caption{ Image area-wise distribution  before and after augmentation} 
% \caption{Statistics analysis of cover page images}
\caption{Image area-wise distribution of cover page}
\begin{adjustbox}{width=0.47\textwidth}
\begin{tabular}{c|c|c}%{p{2.5cm}|p{2.5cm}|p{2.5cm}}
\hline
Image area range  & Number of samples before & Number of samples after\\
(10000 pixel$^2$) & augmentation & augmentation \\
\hline 
< 5 & 20 & 50\\
5 \--- 10 & 264 & 9847\\
10 \--- 15 & 7039 & 11104\\
15 \--- 20 & 2194 & 3895\\
20 \--- 25 & 275 & 574\\
25 \--- 30 & 120 & 243\\
30 \--- 35 & 51 & 86\\
35 \--- 40 & 41 & 63\\
> 40 & 1298 & 2091\\
 \hline
\end{tabular}
\end{adjustbox}
\label{tab:stats_coverpage}
\end{table}

\begin{figure}[!hbt]
    \centering
    \begin{subfigure}{0.24\textwidth}
        \begin{tikzpicture}[scale=0.48]
        \begin{axis}[
        ybar,
        ymin=0,
        ymax=7000,
        ylabel={No. of samples},
        xlabel={Word count range},
        symbolic x coords={0 -- 100,101 -- 200,201 -- 300,301 -- 400,>400},
        xtick=data,
        ytick={1000,2000,3000,4000,5000,6000},
        nodes near coords,
        every node near coord/.append style={font=\large, yshift=5pt, color=black},
        tick label style={font=\large},
        label style={font=\Large},
        enlarge x limits=0.15,
        ymajorgrids=true,
        xmajorgrids=false,
        xticklabel style={rotate=90, anchor=east},
        ]
        \addplot+[fill=red, color=red]  coordinates {(0 -- 100,5788) (101 -- 200,3524) (201 -- 300,1370) (301 -- 400,422) (>400,187)};
        \end{axis}
    \end{tikzpicture}
    \caption{before augmentation}
    \end{subfigure}
    \hfill
     \begin{subfigure}{0.24\textwidth}
        \begin{tikzpicture}[scale=0.48]
        \begin{axis}[
        ybar,
        ymin=0,
        ymax=17500,
        ylabel={No. of samples},
        xlabel={Word count range},
        symbolic x coords={0 -- 100,101 -- 200,201 -- 300,301 -- 400,>400},
        xtick=data,
        ytick={2500,5000,7500,10000,12500,15000},
        nodes near coords,
        every node near coord/.append style={font=\large, yshift=5pt, color=black},
        tick label style={font=\large},
        label style={font=\Large},
        enlarge x limits=0.15,
        ymajorgrids=true,
        xmajorgrids=false,
        xticklabel style={rotate=90, anchor=east},
        ]
        \addplot+[fill=blue, color=blue]  coordinates {(0 -- 100,14710) (101 -- 200,10222) (201 -- 300,2257) (301 -- 400,553) (>400,200)};
        \end{axis}
    \end{tikzpicture}
    \caption{after augmentation}
    \end{subfigure}
    \caption{(a)  Word count-wise distribution of description across sample}
    \label{tab:stats_description}
\end{figure}

\begin{figure}[!hbt]
    \centering
    \begin{subfigure}{0.24\textwidth}
        \begin{tikzpicture}[scale=0.48]
        \begin{axis}[
        ybar,
        ymin=0,
        ymax=8400,
        ylabel={No. of samples},
        xlabel={Word count range},
        symbolic x coords={0 -- 20,21 -- 40,41 -- 60,61 -- 80,81 -- 100,>100},
        xtick=data,
        ytick={1200,2400,3600,4800,6000,7200},
        nodes near coords,
        every node near coord/.append style={font=\large, yshift=5pt, color=black},
        tick label style={font=\large},
        label style={font=\Large},
        enlarge x limits=0.15,
        ymajorgrids=true,
        xmajorgrids=false,
        xticklabel style={rotate=90, anchor=east},
        ]
        \addplot+[fill=red, color=red]  coordinates {(0 -- 20,7421) (21 -- 40,2880) (41 -- 60,740) (61 -- 80,146) (81 -- 100,38) (>100,74) };
        \end{axis}
    \end{tikzpicture}
    \caption{before augmentation}
    \end{subfigure}
    % \hfill
     \begin{subfigure}{0.24\textwidth}
        \begin{tikzpicture}[scale=0.48]
        \begin{axis}[
        ybar,
        ymin=0,
        ymax=21000,
        ylabel={No. of samples},
        xlabel={Word count range},
        symbolic x coords={0 -- 20,21 -- 40,41 -- 60,61 -- 80,81 -- 100,>100},
        xtick=data,
        ytick={3000,6000,9000,12000,15000,18000},
        nodes near coords,
        every node near coord/.append style={font=\large, yshift=5pt, color=black},
        tick label style={font=\large},
        label style={font=\Large},
        enlarge x limits=0.15,
        ymajorgrids=true,
        xmajorgrids=false,
        xticklabel style={rotate=90, anchor=east},
        ]
        \addplot+[fill=blue, color=blue]  coordinates {(0 -- 20,17646) (21 -- 40,7476) (41 -- 60,2013) (61 -- 80,491) (81 -- 100,128)  (>100,199)};
        \end{axis}
    \end{tikzpicture}
    \caption{after augmentation}
    \end{subfigure}
    \caption{(a)  Word count-wise distribution of cover text across sample}
    \label{tab:stats_cover_text}
\end{figure}

\begin{figure}[!hbt]
    \centering
    % \begin{subfigure}{0.24\textwidth}
        \begin{tikzpicture}[scale=0.55]
        \begin{axis}[
        ybar,
        ymin=0,
        ymax=8000,
        ylabel={No. of authors},
        xlabel={No. of samples},
        symbolic x coords={0 -- 10,11 -- 20,21 -- 30,31 -- 40, >40},
        xtick=data,
        ytick={1000,2000,3000,4000,5000,6000, 7000},
        nodes near coords,
        every node near coord/.append style={font=\large, yshift=5pt, color=black},
        tick label style={font=\large},
        label style={font=\Large},
        enlarge x limits=0.15,
        ymajorgrids=true,
        xmajorgrids=false,
        xticklabel style={rotate=90, anchor=east},
        ]
        \addplot+[fill=red, color=red]  coordinates {(0 -- 10,7122) (11 -- 20,42) (21 -- 30,6) (31 -- 40,5) (>40,1)};
        \end{axis}
    \end{tikzpicture}
    % \caption{\footnotesize}
    % \end{subfigure}
    % \hfill
    %  \begin{subfigure}{0.24\textwidth}
    %     \begin{tikzpicture}[scale=0.48]
    %     \begin{axis}[
    %     ybar,
    %     ymin=0,
    %     ymax=2000,
    %     ylabel={No. of publisher},
    %     xlabel={No. of samples},
    %     symbolic x coords={0 -- 10,11 -- 20,21 -- 30,31 -- 40,41 -- 50, >50},
    %     xtick=data,
    %     ytick={250,500,750,1000,1250,1500, 1750},
    %     nodes near coords,
    %     every node near coord/.append style={font=\large, yshift=5pt, color=black},
    %     tick label style={font=\large},
    %     label style={font=\Large},
    %     enlarge x limits=0.15,
    %     ymajorgrids=true,
    %     xmajorgrids=false,
    %     xticklabel style={rotate=90, anchor=east},
    %     ]
    %     \addplot+[fill=blue, color=blue]  coordinates {(0 -- 10,1735) (11 -- 20,99) (21 -- 30,34) (31 -- 40,28) (41 -- 50,15) (>50,35)};
    %     \end{axis}
    % \end{tikzpicture}
    % \caption{\footnotesize No. of samples-wise distribution of publishers}
    % \end{subfigure}
    \caption{No. of samples-wise distribution of authors}
    \label{tab:stats_metadata}
\end{figure}
