# Supplementary material for: Adaptive Data-Resilient Multi-Modal Hierarchical Multi-Label Book Genre Identification
Source: arXiv:2505.03839 source file (2025-10-18)
Supplement: Supplementary file 9 [file all_stats.tex]

\begin{table}[!hbt]
 \centering
 \caption{Statistical analysis}
 %\vspace{1em} % Adjust the vertical space here
 \begin{adjustbox}{width=0.47\textwidth}
 \begin{tabular}{c|c|c|c|c|c|c}
\hline
   \textbf{Input} & 
   
& \textbf{Minimum} & \textbf{Maximum} & \textbf{Mean ($\mu$)} & \textbf{Median} & \textbf{SD ($\sigma$)}\\ \hline

& Image area before & \multirow{2}{*}{20460} & \multirow{2}{*}{16301712} & \multirow{2}{*}{435282.41} & \multirow{2}{*}{146775} & \multirow{2}{*}{1125224.73}\\

\textbf{Cover page} & augmentation & & & & & \\
\cline{2-7}
\textbf{images} & Image area after & \multirow{2}{*}{20460} & \multirow{2}{*}{16301712} & \multirow{2}{*}{325205.84} & \multirow{2}{*}{135850} & \multirow{2}{*}{980565.34}\\ 
& augmentation & & & & & \\
\hline

& No. of words before & \multirow{2}{*}{0} & \multirow{2}{*}{1786} & \multirow{2}{*}{120.52} & \multirow{2}{*}{98} & \multirow{2}{*}{102.37}\\ 
   
\textbf{Description} & augmentation & & & & & \\
\cline{2-7}

\textbf{text} & No. of words after & \multirow{2}{*}{0} & \multirow{2}{*}{1953} & \multirow{2}{*}{110.01} & \multirow{2}{*}{96} & \multirow{2}{*}{80.89}\\ 

& augmentation & & & & & \\
\hline

\multirow{4}{*}{\textbf{Cover text}} & No. of words  & \multirow{3}{*}{1} & \multirow{3}{*}{944} & \multirow{3}{*}{20.67} & \multirow{3}{*}{15} & \multirow{3}{*}{27.69}\\

& before augmentation & & & & & \\ \cline{2-7}

 & No. of words  & \multirow{3}{*}{1} & \multirow{3}{*}{944} & \multirow{3}{*}{21.61} & \multirow{3}{*}{16} & \multirow{3}{*}{25.89}\\
& after augmentation & & & & & \\
   
\hline

& No. of books  & \multirow{2}{*}{1} & \multirow{2}{*}{43} & \multirow{2}{*}{1.57} & \multirow{2}{*}{1} & \multirow{2}{*}{1.91}\\ 

\textbf{Metadata} & written by an author & & & & & \\

\cline{2-7}
& No. of books  & \multirow{2}{*}{1} & \multirow{2}{*}{268} & \multirow{2}{*}{5.80} & \multirow{2}{*}{1} & \multirow{2}{*}{16.64}\\ 
   
& published by a publisher & & & & & \\

\hline

   \multicolumn{7}{r}{SD: Standard Deviation}
 \end{tabular}
\end{adjustbox}
\label{tab:all_stats}
 \end{table}
