# Supplementary material for: Adaptive Data-Resilient Multi-Modal Hierarchical Multi-Label Book Genre Identification
Source: arXiv:2505.03839 source file (2025-10-18)
Supplement: Supplementary file 10 [file stat_measure_word.tex]

% \begin{table}[h]
%     \centering
%         \caption{\textcolor{red}{Statistical Measure of words}}
%         \label{tab:word-distribution}
%         \begin{adjustbox}{width=0.48\textwidth}
%         % \begin{tabular}{|p{2.5cm}|p{1.6cm}|p{1.6cm}|p{1.7cm}|}
% \begin{tabular}{c|c|c|c}
%         \hline
%         \textbf{Dataset type} & \textbf{Mean of Words} & \textbf{Standard Deviation} & \textbf{Mean $\pm$ Stddev (approx.)}\\
%         \hline

%         \multirow{1}{*}{Train dataset} & 97.400224 & 34.857362 & 62-132 \\
%         \hline
%         \multirow{1}{*}{Test dataset} & 97.599857 & 49.066968 & 49-147 \\
%         \hline
%         \multirow{1}{*}{Validation dataset} & 96.888017 & 47.016818 & 50-144 \\
%         \hline
%         \end{tabular}
%         \end{adjustbox}

%         \end{table}

\begin{table}[!hbt]
\centering
\caption{\textcolor{red}{Statistical Measure of words}}
\label{tab:word-distribution}
\begin{adjustbox}{width=0.35\textwidth}

\begin{tabular}{c|c|c|c}
\cline{2-4}
& \multicolumn{3}{c}{Dataset Distribution} \\
\cline{2-4}
& ${\cal{D}}_{train}$ & ${\cal{D}}_{val}$ &  ${\cal{D}}_{test}$\\
\hline

Mean ($\mu$) & 97.4002 & 96.8880 & 97.5996 \\
\hline

SD ($\sigma$) & 34.8574 & 49.0670 & 47.0168\\
\hline
$\mu \pm \sigma$ & 62 - 132& 49 - 147& 50 - 144\\

\hline
\multicolumn{4}{r}{SD: Standard Deviation}
\end{tabular}
\end{adjustbox}

\end{table}
