# Supplementary material for: Adaptive Data-Resilient Multi-Modal Hierarchical Multi-Label Book Genre Identification
Source: arXiv:2505.03839 source file (2025-10-18)
Supplement: Supplementary file 11 [file stats_cover_text.tex]

\begin{figure}[!hbt]
    \centering
    \begin{subfigure}{0.24\textwidth}
        \begin{tikzpicture}[scale=0.48]
        \begin{axis}[
        ybar,
        ymin=0,
        ymax=8400,
        ylabel={No. of samples},
        xlabel={Word count range},
        symbolic x coords={0 -- 20,21 -- 40,41 -- 60,61 -- 80,81 -- 100,>100},
        xtick=data,
        ytick={1200,2400,3600,4800,6000,7200},
        nodes near coords,
        every node near coord/.append style={font=\large, yshift=5pt, color=black},
        tick label style={font=\large},
        label style={font=\Large},
        enlarge x limits=0.15,
        ymajorgrids=true,
        xmajorgrids=false,
        xticklabel style={rotate=90, anchor=east},
        ]
        \addplot+[fill=red, color=red]  coordinates {(0 -- 20,7421) (21 -- 40,2880) (41 -- 60,740) (61 -- 80,146) (81 -- 100,38) (>100,74) };
        \end{axis}
    \end{tikzpicture}
    \caption{before augmentation}
    \end{subfigure}
    % \hfill
     \begin{subfigure}{0.24\textwidth}
        \begin{tikzpicture}[scale=0.48]
        \begin{axis}[
        ybar,
        ymin=0,
        ymax=21000,
        ylabel={No. of samples},
        xlabel={Word count range},
        symbolic x coords={0 -- 20,21 -- 40,41 -- 60,61 -- 80,81 -- 100,>100},
        xtick=data,
        ytick={3000,6000,9000,12000,15000,18000},
        nodes near coords,
        every node near coord/.append style={font=\large, yshift=5pt, color=black},
        tick label style={font=\large},
        label style={font=\Large},
        enlarge x limits=0.15,
        ymajorgrids=true,
        xmajorgrids=false,
        xticklabel style={rotate=90, anchor=east},
        ]
        \addplot+[fill=blue, color=blue]  coordinates {(0 -- 20,17646) (21 -- 40,7476) (41 -- 60,2013) (61 -- 80,491) (81 -- 100,128)  (>100,199)};
        \end{axis}
    \end{tikzpicture}
    \caption{after augmentation}
    \end{subfigure}
    \caption{(a)  Word count-wise distribution of cover text across sample}
    \label{tab:stats_cover_text}
\end{figure}
