# Supplementary material for: Adaptive Data-Resilient Multi-Modal Hierarchical Multi-Label Book Genre Identification
Source: arXiv:2505.03839 source file (2025-10-18)
Supplement: Supplementary file 12 [file stats_coverpage.tex]

\begin{table}[!hbt]
\centering  
% \footnotesize
% \caption{ Image area-wise distribution  before and after augmentation} 
% \caption{Statistics analysis of cover page images}
\caption{Image area-wise distribution of cover page}
\begin{adjustbox}{width=0.47\textwidth}
\begin{tabular}{c|c|c}%{p{2.5cm}|p{2.5cm}|p{2.5cm}}
\hline
Image area range  & Number of samples before & Number of samples after\\
(10000 pixel$^2$) & augmentation & augmentation \\
\hline 
< 5 & 20 & 50\\
5 \--- 10 & 264 & 9847\\
10 \--- 15 & 7039 & 11104\\
15 \--- 20 & 2194 & 3895\\
20 \--- 25 & 275 & 574\\
25 \--- 30 & 120 & 243\\
30 \--- 35 & 51 & 86\\
35 \--- 40 & 41 & 63\\
> 40 & 1298 & 2091\\
 \hline
\end{tabular}
\end{adjustbox}
\label{tab:stats_coverpage}
\end{table}
