# Supplementary material for: Adaptive Data-Resilient Multi-Modal Hierarchical Multi-Label Book Genre Identification
Source: arXiv:2505.03839 source file (2025-10-18)
Supplement: Supplementary file 13 [file stats_description.tex]

\begin{figure}[!hbt]
    \centering
    \begin{subfigure}{0.24\textwidth}
        \begin{tikzpicture}[scale=0.48]
        \begin{axis}[
        ybar,
        ymin=0,
        ymax=7000,
        ylabel={No. of samples},
        xlabel={Word count range},
        symbolic x coords={0 -- 100,101 -- 200,201 -- 300,301 -- 400,>400},
        xtick=data,
        ytick={1000,2000,3000,4000,5000,6000},
        nodes near coords,
        every node near coord/.append style={font=\large, yshift=5pt, color=black},
        tick label style={font=\large},
        label style={font=\Large},
        enlarge x limits=0.15,
        ymajorgrids=true,
        xmajorgrids=false,
        xticklabel style={rotate=90, anchor=east},
        ]
        \addplot+[fill=red, color=red]  coordinates {(0 -- 100,5788) (101 -- 200,3524) (201 -- 300,1370) (301 -- 400,422) (>400,187)};
        \end{axis}
    \end{tikzpicture}
    \caption{before augmentation}
    \end{subfigure}
    \hfill
     \begin{subfigure}{0.24\textwidth}
        \begin{tikzpicture}[scale=0.48]
        \begin{axis}[
        ybar,
        ymin=0,
        ymax=17500,
        ylabel={No. of samples},
        xlabel={Word count range},
        symbolic x coords={0 -- 100,101 -- 200,201 -- 300,301 -- 400,>400},
        xtick=data,
        ytick={2500,5000,7500,10000,12500,15000},
        nodes near coords,
        every node near coord/.append style={font=\large, yshift=5pt, color=black},
        tick label style={font=\large},
        label style={font=\Large},
        enlarge x limits=0.15,
        ymajorgrids=true,
        xmajorgrids=false,
        xticklabel style={rotate=90, anchor=east},
        ]
        \addplot+[fill=blue, color=blue]  coordinates {(0 -- 100,14710) (101 -- 200,10222) (201 -- 300,2257) (301 -- 400,553) (>400,200)};
        \end{axis}
    \end{tikzpicture}
    \caption{after augmentation}
    \end{subfigure}
    \caption{(a)  Word count-wise distribution of description across sample}
    \label{tab:stats_description}
\end{figure}

% \begin{tikzpicture}
% \begin{axis}[
%     ybar,
%     bar width=25pt,
%     width=13cm,
%     height=8cm,
%     ymin=0,
%     ymax=7000,
%     ylabel={No. of samples},
%     xlabel={Word count range},
%     symbolic x coords={0-100,101-200,201-300,301-400,400<},
%     xtick=data,
%     nodes near coords,
%     nodes near coords align={vertical},
%     every node near coord/.append style={font=\large, yshift=5pt},
%     tick label style={font=\large},
%     label style={font=\large},
%     enlarge x limits=0.15,
%     grid=major,
% ]
% \addplot coordinates {(0-100,5788) (101-200,3524) (201-300,1370) (301-400,422) (400<,187)};
% \end{axis}
% \end{tikzpicture}
