# Supplementary material for: Adaptive Data-Resilient Multi-Modal Hierarchical Multi-Label Book Genre Identification
Source: arXiv:2505.03839 source file (2025-10-18)
Supplement: Supplementary file 14 [file stats_metadata.tex]

\begin{figure}[!hbt]
    \centering
    % \begin{subfigure}{0.24\textwidth}
        \begin{tikzpicture}[scale=0.55]
        \begin{axis}[
        ybar,
        ymin=0,
        ymax=8000,
        ylabel={No. of authors},
        xlabel={No. of samples},
        symbolic x coords={0 -- 10,11 -- 20,21 -- 30,31 -- 40, >40},
        xtick=data,
        ytick={1000,2000,3000,4000,5000,6000, 7000},
        nodes near coords,
        every node near coord/.append style={font=\large, yshift=5pt, color=black},
        tick label style={font=\large},
        label style={font=\Large},
        enlarge x limits=0.15,
        ymajorgrids=true,
        xmajorgrids=false,
        xticklabel style={rotate=90, anchor=east},
        ]
        \addplot+[fill=red, color=red]  coordinates {(0 -- 10,7122) (11 -- 20,42) (21 -- 30,6) (31 -- 40,5) (>40,1)};
        \end{axis}
    \end{tikzpicture}
    % \caption{\footnotesize}
    % \end{subfigure}
    % \hfill
    %  \begin{subfigure}{0.24\textwidth}
    %     \begin{tikzpicture}[scale=0.48]
    %     \begin{axis}[
    %     ybar,
    %     ymin=0,
    %     ymax=2000,
    %     ylabel={No. of publisher},
    %     xlabel={No. of samples},
    %     symbolic x coords={0 -- 10,11 -- 20,21 -- 30,31 -- 40,41 -- 50, >50},
    %     xtick=data,
    %     ytick={250,500,750,1000,1250,1500, 1750},
    %     nodes near coords,
    %     every node near coord/.append style={font=\large, yshift=5pt, color=black},
    %     tick label style={font=\large},
    %     label style={font=\Large},
    %     enlarge x limits=0.15,
    %     ymajorgrids=true,
    %     xmajorgrids=false,
    %     xticklabel style={rotate=90, anchor=east},
    %     ]
    %     \addplot+[fill=blue, color=blue]  coordinates {(0 -- 10,1735) (11 -- 20,99) (21 -- 30,34) (31 -- 40,28) (41 -- 50,15) (>50,35)};
    %     \end{axis}
    % \end{tikzpicture}
    % \caption{\footnotesize No. of samples-wise distribution of publishers}
    % \end{subfigure}
    \caption{No. of samples-wise distribution of authors}
    \label{tab:stats_metadata}
\end{figure}
