# Supplementary material for: Adaptive Data-Resilient Multi-Modal Hierarchical Multi-Label Book Genre Identification
Source: arXiv:2505.03839 source file (2025-10-18)
Supplement: Supplementary file 15 [file word_distribution.tex]

% \begin{table}[h]
%         \centering
%         \caption{\textcolor{red}{Distribution of words in the dataset}}
%         \begin{adjustbox}{width=0.47\textwidth}
%         \begin{tabular}{c|c|c}
%         \hline
%         & \textbf{Word} & \textbf{Frequency} \\
%          & \textbf{Count} & \\
%          & \textbf{Range}& \\
%         \hline
%         \multirow{5}{*}{${\cal{D}}_{train}$} & 0-10 & 520 \\
%         & 10-20 & 803 \\
%         & 20-30 & 1290 \\
%         & 30-40 & 1747 \\
%         & 40-50 & 1753 \\
%         \hline
%         \multirow{5}{*}{${\cal{D}}_{test}$} & 0-10 & 65 \\
%         & 10-20 & 85 \\
%         & 20-30 & 163 \\
%         & 30-40 & 220 \\
%         & 40-50 & 211 \\
%         \hline
%         \multirow{2}{*}{${\cal{D}}_{val}$} & 0-10 & 64 \\
%         & 10-20 & 84 \\
%         & 20-30 & 152 \\
%         & 30-40 & 232 \\
%         & 40-50 & 234 \\
%         \hline
%         \end{tabular}
%         \end{adjustbox}
%         \label{tab:word-distribution}
%         \end{table}

\begin{table}[!hbt]
\centering
\caption{\textcolor{red}{Distribution of words in the dataset}}
\begin{adjustbox}{width=0.25\textwidth}
\begin{tabular}{c|c|c|c}
\hline
\textbf{Word} & & & \\
\textbf{Count} & ${\cal{D}}_{train}$& ${\cal{D}}_{val}$ & ${\cal{D}}_{test}$ \\
\textbf{Range} & & & \\
\hline

0-10 & 520 & 64 & 65 \\ \hline
10-20 & 803 & 84 & 85 \\ \hline
20-30 & 1290 & 152 & 163 \\ \hline
30-40 & 1747 & 232 & 220  \\ \hline
40-50 & 1753 & 234 & 211 \\ \hline
\end{tabular}
\end{adjustbox}
\label{tab:word-distribution}
\end{table}
